# Supplementary material for: A Note on Target Q-learning For Solving Finite MDPs with A Generative Oracle
Source: arXiv:2203.11489 source file (2022-03-22)
Supplement: Supplementary file 1 [file discussion.tex]

\section{Discussion}
\label{appendix:discussion}

In this section, we discuss some theoretical results in the main paper. 

\subsection{Non-convexity of VAIL}
\label{appendix:vail_objective_is_non_convex}

In this part, we give an example to show that \textsf{VAIL}'s objective in \eqref{eq:ail} is non-convex. Our construction is based on the example in \citep{agarwal2020pg}, in which the authors showed that policy optimization for infinite-horizon tabular MDPs is a non-convex problem.

\begin{claim}   \label{claim:vail_non_convex}
For tabular and episodic MDPs, there exists an instance such that the objective of VAIL in \eqref{eq:ail} is non-convex. 
\end{claim}

\begin{figure}[htbp]
    \centering
    \includegraphics[width=0.6\linewidth]{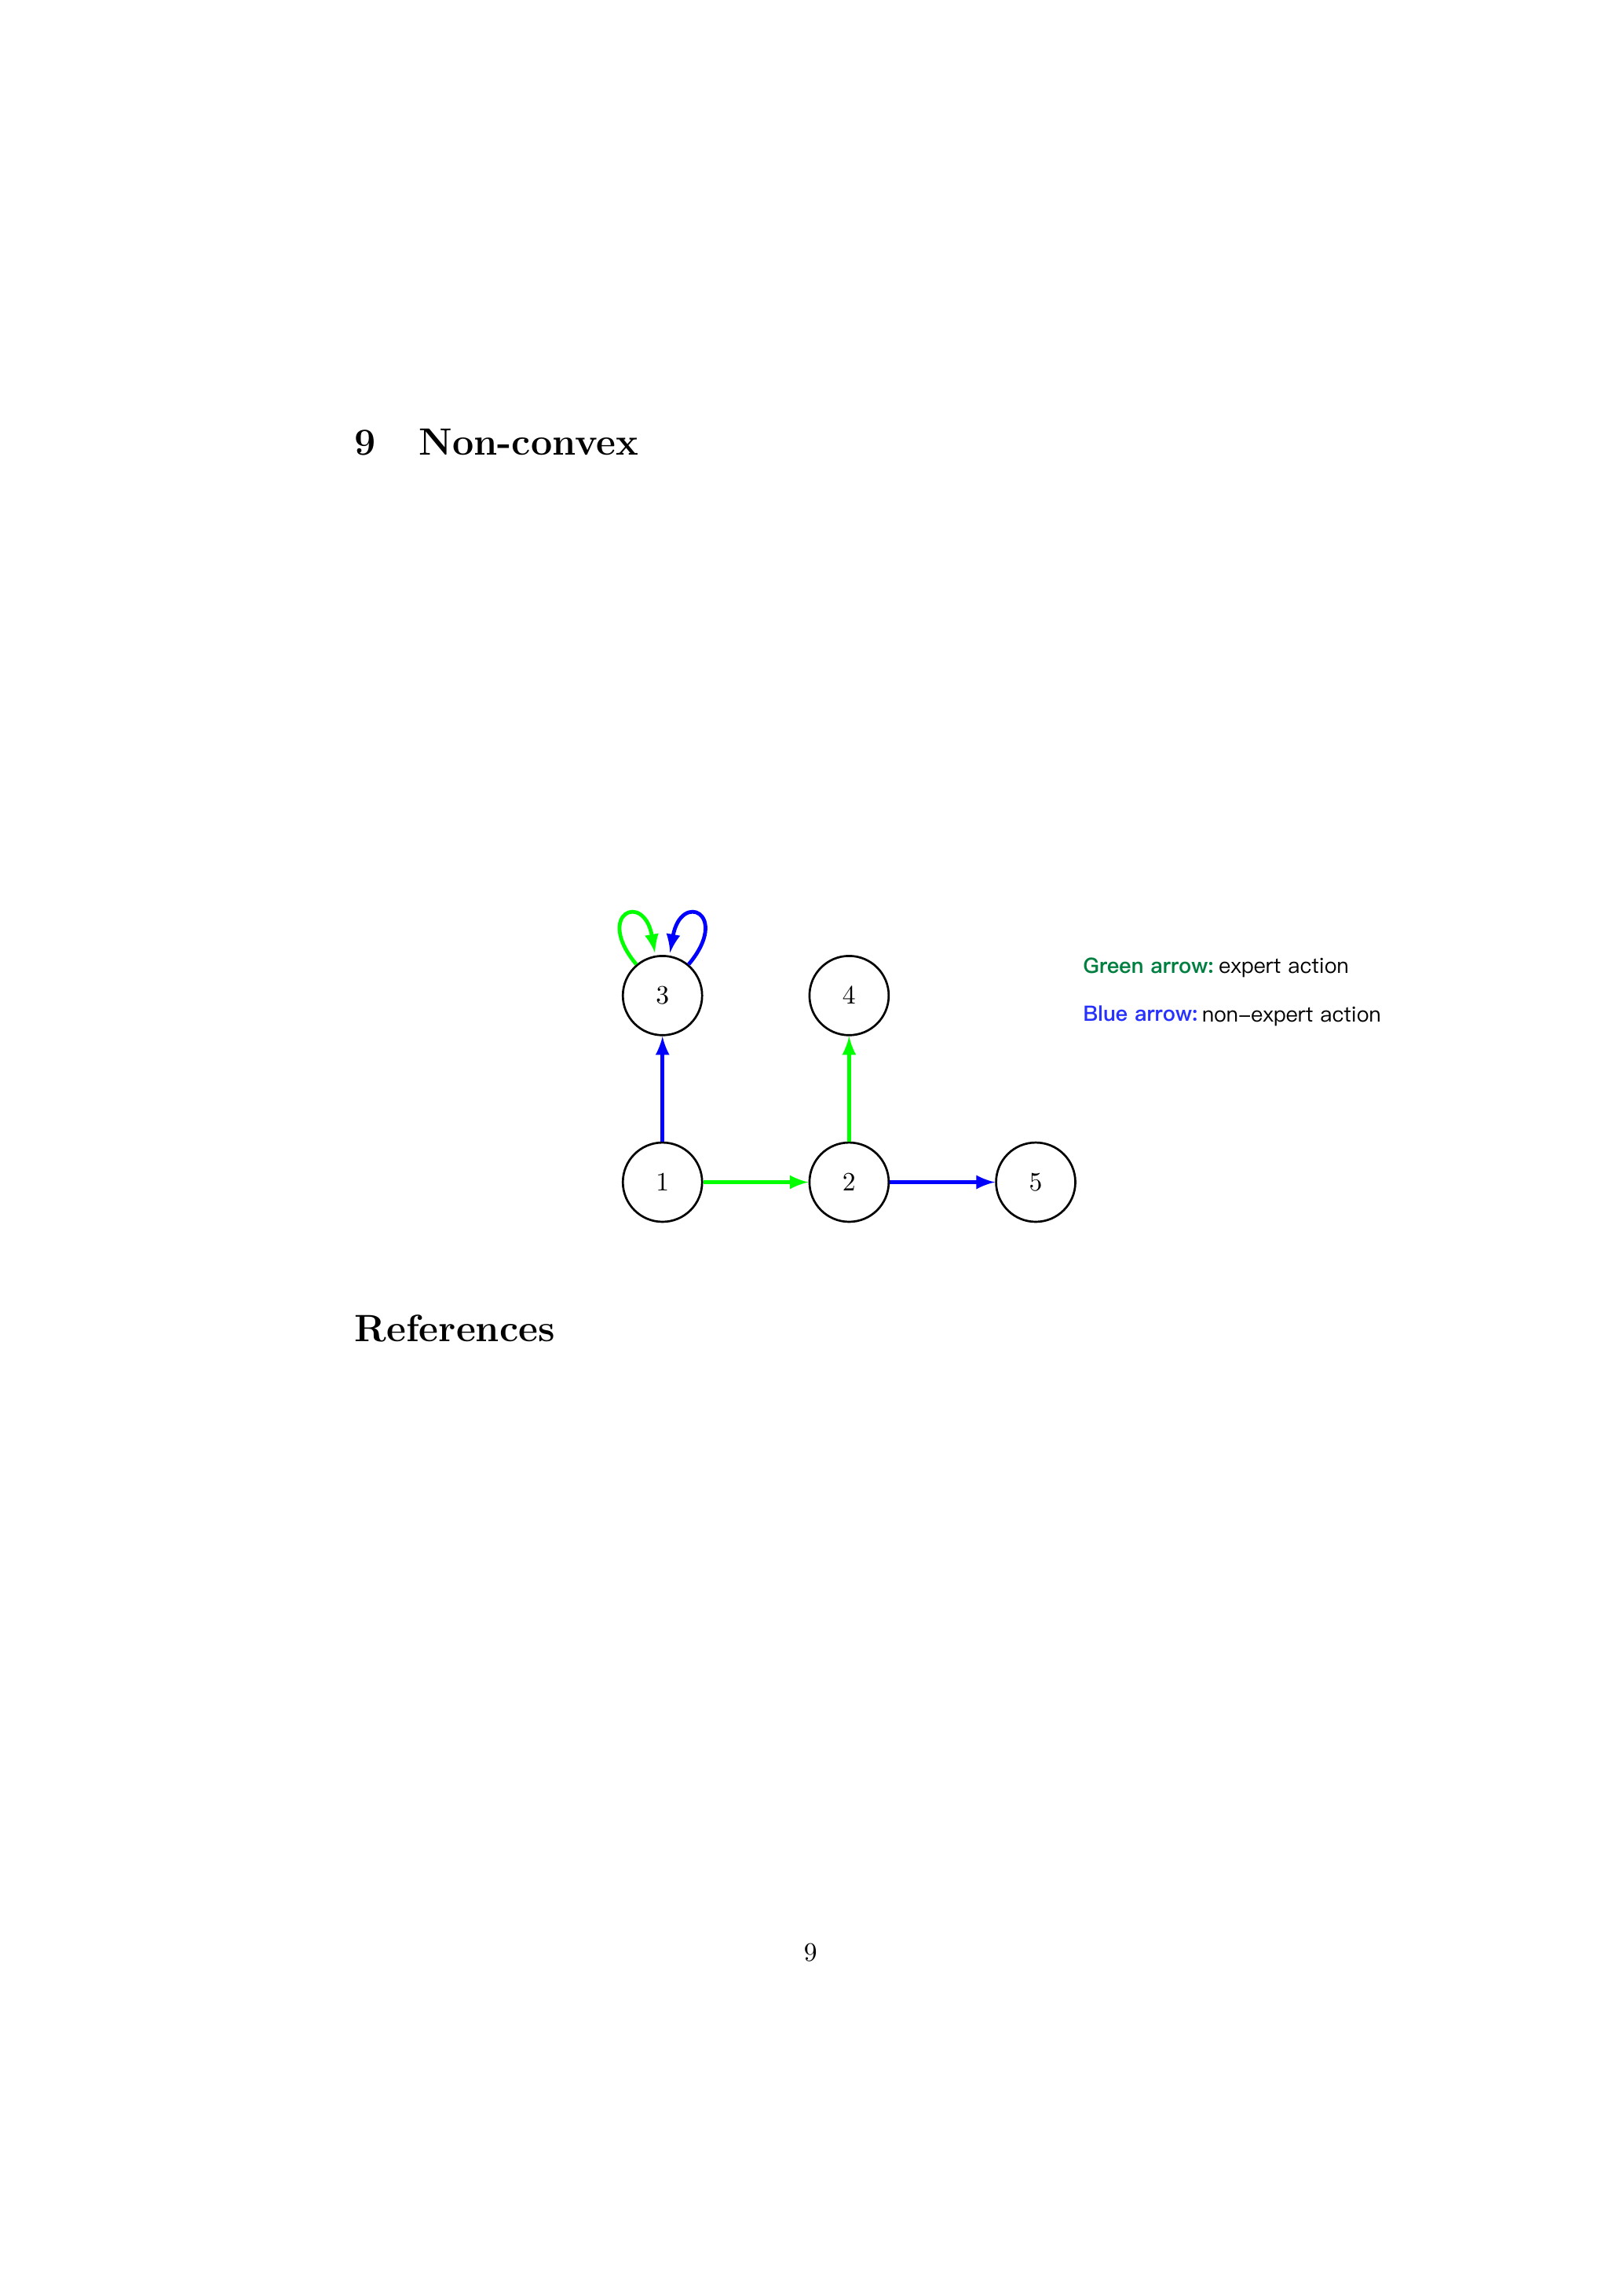}
    \caption{A simple example to show that \textsf{VAIL}'s objective in \eqref{eq:ail} is non-convex.}
    \label{fig:non_convex}
\end{figure}

\begin{proof}[Proof of \cref{claim:vail_non_convex}]
Our construction is shown in \cref{fig:non_convex}. In particular, there are 5 states $(s^{1}, s^{2}, s^{3}, s^{4}, s^{5})$ and two actions $(a^{1}, a^{2})$. Each arrow shows a deterministic transition. The initial state is $s^1$ and the planning horizon is $2$. Assume  $a^{1}$ is the expert action and there is only one expert trajectory: $(s^{1}, a^{1}) \rar (s^{2}, a^{1})$. We can calculate the empirical distribution:
\begin{align*}
    \widehat{P}^{\piE}_{1}(s^{1}, a^{1}) = 1.0, \quad  \widehat{P}^{\piE}_{2}(s^{2}, a^{1}) = 1.0
\end{align*}
Let us use the following notations: $x := \pi_1(a^{1} | s^{1})$ and $y := \pi_2(a^{1} | s^{2})$. In time step $h=1$, we have 
\begin{align*}
    \ell_1 &= \sum_{(s, a)} \labs P^{\pi}_1(s, a) - \widehat{P}^{\piE}_1(s, a) \rabs \\
    &= \labs P^{\pi}_{1}(s^{1}, a^{1}) - \widehat{P}^{\piE}_{1} (s^{1}, a^{1}) \rabs + \labs P^{\pi}_{1} (s^{1}, a^{2}) - \widehat{P}^{\piE}_{1}(s^{1}, a^{2}) \rabs \\
    &= \labs x - 1 \rabs + \labs 1-x - 0 \rabs = 2(1 - x).
\end{align*}
In time step $h=2$, we have 
\begin{align*}
    \ell_2 &= \sum_{(s, a)} \labs P^{\pi}_2(s, a) - \widehat{P}^{\piE}_2(s, a) \rabs \\
    &= \labs P^{\pi}_{2}(s^{2}, a^{1}) - \widehat{P}^{\piE}_2(s^{2}, a^{1}) \rabs +  \labs P^{\pi}_{2}(s^{2}, a^{2}) - \widehat{P}^{\piE}_2(s^{2}, a^{2}) \rabs \\
    &\quad + \labs P^{\pi}_{2}(s^{3}, a^{1}) - \widehat{P}^{\piE}_2(s^{3}, a^{1}) \rabs + \labs P^{\pi}_{2}(s^{3}, a^{2}) - \widehat{P}^{\piE}_2(s^{3}, a^{2}) \rabs \\
    &= \labs xy - 1 \rabs + \labs x(1-y) - 0 \rabs + (1-x)  \\
    &= 1 - xy + x - xy + 1 - x = 2(1 - xy).
\end{align*}
Thus, we have that 
\begin{align*}
    f(x, y) = \ell_1 + \ell_2 = 2 \lp 2 - x - xy \rp.
\end{align*}
Furthermore, we can compute that 
\begin{align*}
    \nabla f(x, y) = \bvec{-2 - 2y \\ -2x}, \\
    \nabla^2 f(x, y) = \bvec{0 & -2 \\ -2 & 0}.
\end{align*}
Since $\nabla^2 f(x, y)$ is not a PSD, we claim that $f(x, y)$ is non-convex w.r.t. $(x, y)$.

\end{proof}

\subsection{VAIL with Subsampled Trajectories}
\label{appendix:further_discssuion_of_example_success_subsampling}

In this part, we discuss the generalization of \textsf{VAIL} with \emph{subsampled} expert trajectories. Before discussion, we point out that VAIL cannot recover the expert policy with any subsampled trajectories even on Reset Cliff. What really matters for VAIL is the state-action pairs with large time steps. If these state-action pairs are masked, we cannot expect VAIL to generalize well. This claim can be easily verified on Gym MuJoCo locomotion tasks. Hence, we mainly focus on the following example to illustrate the key idea under the subsampling case. 

\begin{example}  \label{example:subsample_trajectory}
Consider an example similar to \cref{example:ail_success}. We consider the same state space, action space, initial state distribution and transition function as in \cref{example:ail_success}. Different from \cref{example:ail_success}, we consider the horizon length $H=3$. The agent is provided only 2 expert trajectories $\tr_1 = (s^{1}, a^{1}) \rar (s^{1}, a^{1}) \rar (s^{1}, a^{1}) $ and $\tr_2 = (s^{1}, a^{1}) \rar (s^{2}, a^{1}) \rar (s^{2}, a^{1})$. We subsample expert trajectories so that \emph{the data in the time step $h=1$ is masked (i.e., missing)}. This operation is similar to the subsampling procedure in \citep{ho2016gail, Kostrikov19dac}. 
\end{example}

\begin{claim} \label{claim:ail_reset_cliff_subsample}
Consider the MDP and expert demonstrations in \cref{example:subsample_trajectory}. Suppose that $\piail$ is the optimal solution of \eqref{eq:ail}, then for each time step $h \in [3]$, $\piail_{h} (a^{1}|s) = \piE_h (a^{1}|s) = 1, \forall s \in \{s^{1}, s^{2} \}$.  
\end{claim}

\begin{rem}
\cref{claim:ail_reset_cliff_subsample} indicates that if the expert trajectories are properly subsampled, VAIL can still recover the expert policy. We remark that this conclusion does not hold for the case where the horizon is 2 and we mask the state-action pair in the first time step. This is because the objective in the second time step is too weak to provide effective guidance for the policy optimization in the first time step. Instead, the conclusion holds for the case where the horizon is 3 considered in \cref{example:subsample_trajectory}. This implies that to retain good performance with subsampled trajectories, we must post constraints on the subsampling rate and subsampling interval.
\end{rem}

Before proving \cref{claim:ail_reset_cliff_subsample}, we first prove a useful claim which is similar to \cref{lem:condition_for_ail_optimal_solution}.

\begin{claim}
\label{claim:condition_for_ail_optimal_solution}
Consider the MDP and expert demonstrations in \cref{example:subsample_trajectory}. Suppose that $\piail$ is the optimal solution of \eqref{eq:ail}, then for each time step $h \in [3]$, $\exists s \in \goodS, \piail_h (a^{1}|s) > 0$. 
\end{claim}

\begin{proof}
The empirical state-action distribution with subsampled expert demonstrations are formulated as follows. Note that the data in time step $h=1$ is masked and thus the corresponding empirical distribution is uniform distribution.
\begin{align*}
    \widehat{P}^{\piE}_{1}(s^{1}, a^{1}) = \frac{1}{6}, \widehat{P}^{\piE}_{1}(s^{2}, a^{1}) = \frac{1}{6}, \widehat{P}^{\piE}_{1}(s^{3}, a^{1}) = \frac{1}{6}, \\
    \widehat{P}^{\piE}_{1}(s^{1}, a^{2}) = \frac{1}{6}, \widehat{P}^{\piE}_{1}(s^{2}, a^{2}) = \frac{1}{6}, \widehat{P}^{\piE}_{1}(s^{3}, a^{2}) = \frac{1}{6}, \\
    \widehat{P}^{\piE}_{2}(s^{1}, a^{1}) = \RED{0.5}, \widehat{P}^{\piE}_{2}(s^{2}, a^{1}) = \RED{0.5}, \widehat{P}^{\piE}_{2}(s^{3}, a^{1}) = 0.0, \\
    \widehat{P}^{\piE}_{2}(s^{1}, a^{2}) = 0.0, \widehat{P}^{\piE}_{2}(s^{2}, a^{2}) = 0.0, \widehat{P}^{\piE}_{2}(s^{3}, a^{2}) = 0.0, \\
    \widehat{P}^{\piE}_{3}(s^{1}, a^{1}) = \RED{0.5}, \widehat{P}^{\piE}_{3}(s^{2}, a^{1}) = \RED{0.5}, \widehat{P}^{\piE}_{3}(s^{3}, a^{1}) = 0.0, \\
    \widehat{P}^{\piE}_{3}(s^{1}, a^{2}) = 0.0, \widehat{P}^{\piE}_{3}(s^{2}, a^{2}) = 0.0, \widehat{P}^{\piE}_{3}(s^{3}, a^{2}) = 0.0.
\end{align*}
We first prove that for the first time step, $\exists s \in \goodS, \piail_1 (a^{1}|s) > 0$. The proof is based on contradiction.

We assume that the original statement is false and $\forall s \in \goodS$, $\piail_1 (a^{1}|s) = 0$. We construct another policy $\widetilde{\pi}^{\ail}$. In time steps $h=1$ and $h=2$, $\forall s \in \goodS, \widetilde{\pi}^{\ail}_h (a^{1}|s) = 1$. We compare \textsf{VAIL}'s objectives under $\piail$ and $\widetilde{\pi}^{\ail}$. We first consider $\piail$. It is easy to compute the state-action distribution induced by $\piail$.
\begin{align*}
    &P^{\piail}_{1}(s^{1}, a^{1}) = 0.0, P^{\piail}_{1}(s^{2}, a^{1}) = 0.0, P^{\piail}_{1}(s^{3}) = 0.0, \\
    &P^{\piail}_{1}(s^{1}, a^{2}) = 0.5, P^{\piail}_{1}(s^{2}, a^{2}) = 0.5, \\
    &P^{\piail}_{2}(s^{1}) = 0.0, P^{\piail}_{2}(s^{2}) = 0.0, P^{\piail}_{2}(s^{3}) = 1.0, \\
    &P^{\piail}_{3}(s^{1}) = 0.0, P^{\piail}_{3}(s^{2}) = 0.0, P^{\piail}_{3}(s^{3}) = 1.0.
\end{align*}
Recall the definition of the single-stage loss function in time step $h$.
\begin{align*}
    \text{Loss}_h (\pi) = \sum_{(s, a) \in \gS \times \gA} \labs P^{\pi}_h(s, a)  - \widehat{P}^{\piE}_h(s, a) \rabs .
\end{align*}
It is direct to compute that $\text{Loss}_1 (\piail) = 4/3, \text{Loss}_2 (\piail) = \text{Loss}_3 (\piail) = 2$.

Second, we consider \textsf{VAIL}'s objective of $\widetilde{\pi}^{\ail}$.
\begin{align*}
     &P^{\widetilde{\pi}^{\ail}}_{1}(s^{1}, a^{1}) = 0.5, P^{\widetilde{\pi}^{\ail}}_{1}(s^{2}, a^{1}) = 0.5, P^{\widetilde{\pi}^{\ail}}_{1}(s^{3}) = 0.0, \\
    &P^{\widetilde{\pi}^{\ail}}_{1}(s^{1}, a^{2}) = 0.0, P^{\widetilde{\pi}^{\ail}}_{1}(s^{2}, a^{2}) = 0.0.
\end{align*}
Similarly, we have $\text{Loss}_1 (\widetilde{\pi}^{\ail}) = 4/3$. We proceed to consider time step $h=2$. By \dquote{transition flow equation}, it holds that
\begin{align*}
    &P^{\widetilde{\pi}^{\ail}}_{2}(s^{1}) = P^{\widetilde{\pi}^{\ail}}_{1}(s^{1}, a^{1}) P_1 (s^{1}|s^{1}, a^{1}) +  P^{\widetilde{\pi}^{\ail}}_{1}(s^{2}, a^{1}) P_1 (s^{1}|s^{2}, a^{1}) = 0.5,
    \\
    &P^{\widetilde{\pi}^{\ail}}_{2}(s^{2}) = P^{\widetilde{\pi}^{\ail}}_{1}(s^{1}, a^{1}) P_1 (s^{2}|s^{1}, a^{1}) +  P^{\widetilde{\pi}^{\ail}}_{1}(s^{2}, a^{1}) P_1 (s^{2}|s^{2}, a^{1}) = 0.5,
    \\
    & P^{\widetilde{\pi}^{\ail}}_{2}(s^{3}) = 0. 
\end{align*}
Then we can calculate that
\begin{align*}
    \text{Loss}_2 (\widetilde{\pi}^{\ail}) &= \labs 0.5 - P^{\widetilde{\pi}^{\ail}}_{2}(s^{1}) \widetilde{\pi}^{\ail}_2( a^{1}|s^{1})  \rabs + P^{\widetilde{\pi}^{\ail}}_{2}(s^{1})  \widetilde{\pi}^{\ail}_2 (a^{2}|s^{1})
    \\
    &\quad + \labs 0.5 - P^{\widetilde{\pi}^{\ail}}_{2}(s^{2}) \widetilde{\pi}^{\ail}_{2} (a^{1}|s^{2})  \rabs + P^{\widetilde{\pi}^{\ail}}_{2}(s^{2})  \widetilde{\pi}^{\ail}_{2} (a^{2}|s^{2})
    \\
    &= \labs 0.5 - 0.5 \widetilde{\pi}^{\ail}_2( a^{1}|s^{1})  \rabs + 0.5 - 0.5  \widetilde{\pi}^{\ail}_2 (a^{1}|s^{1})
    \\
    &\quad + \labs 0.5 - 0.5 \widetilde{\pi}^{\ail}_{2} (a^{1}|s^{2})  \rabs + 0.5 - 0.5 \widetilde{\pi}^{\ail}_{2} (a^{1}|s^{2})
    \\
    &= 2 - \widetilde{\pi}^{\ail}_2 (a^{1}|s^{1}) - \widetilde{\pi}^{\ail}_{2} (a^{1}|s^{2}) = 0.  
\end{align*}
Therefore, we have that $\text{Loss}_2 (\widetilde{\pi}^{\ail}) < 2 = \text{Loss}_2 (\pi^{\ail})$. For time step $h=3$, note that $2$ is the maximal value of the single-stage loss function and $\text{Loss}_3 (\widetilde{\pi}^{\ail}) \leq 2 = \text{Loss}_3 (\pi^{\ail})$. In a word, we construct policy $\widetilde{\pi}^{\ail}$ whose \textsf{VAIL}'s objective is strictly smaller than that of $\piail$. This contradicts with the fact that $\piail$ is the optimal solution of \eqref{eq:ail} and thus the original statement is true. That is, $\exists s \in \goodS$, $\piail_1 (a^{1}|s) > 0$.

We continue to consider time steps $h=2$. With \cref{lem:n_vars_opt_greedy_structure}, fixing $\piail_1$, $\piail_2$ and $\piail_3$ is also optimal solution w.r.t \textsf{VAIL}'s objective. Formally,
\begin{align}
    (\piail_2, \piail_3) &\in \argmin_{\pi_2, \pi_3} \text{Loss}_1 (\piail_1) + \text{Loss}_2 (\piail_1, \pi_2) + \text{Loss}_3 (\piail_1, \pi_2, \pi_3) \nonumber
    \\
    &= \argmin_{\pi_2, \pi_3} \text{Loss}_2 (\piail_1, \pi_2) + \text{Loss}_3 (\piail_1, \pi_2, \pi_3). \label{eq:piail_2_and_piail_3_are_optimal}  
\end{align}
The proof is also based on contradiction. We assume that $\forall s \in \goodS$, $\piail_2 (a^{1}|s) = 0$. We construct another policy $(\widetilde{\pi}^{\ail}_2, \piail_3)$: $\forall s \in \goodS$, $\widetilde{\pi}^{\ail}_2 (a^{1}|s) = 1$. On the one hand,
\begin{align*}
    \text{Loss}_2 (\piail_1, \piail_2) = 2, \text{Loss}_3 (\piail_1, \piail_2, \piail_3) = 2.
\end{align*}
On the other hand,
\begin{align*}
    \text{Loss}_2 (\piail_1, \widetilde{\pi}^{\ail}_2) &= \labs 0.5 - P^{\piail}_{2}(s^{1}) \widetilde{\pi}^{\ail}_2( a^{1}|s^{1})  \rabs + P^{\piail}_{2}(s^{1})  \widetilde{\pi}^{\ail}_2 (a^{2}|s^{1})
    \\
    &+ \labs 0.5 - P^{\piail}_{2}(s^{2}) \widetilde{\pi}^{\ail}_{2} (a^{1}|s^{2})  \rabs + P^{\piail}_{2}(s^{2})  \widetilde{\pi}^{\ail}_{2} (a^{2}|s^{2}) + P^{\piail}_{2}(s^{3})
    \\
    &= \labs 0.5 - P^{\piail}_{2}(s^{1}) \rabs + \labs 0.5 - P^{\piail}_{2}(s^{2}) \rabs + P^{\piail}_{2}(s^{3})
    \\
    &= 2 - 2 \lp P^{\piail}_{2}(s^{1}) + P^{\piail}_{2}(s^{2})  \rp.
\end{align*}
We have proved for time step $h=1$, $\exists s \in \goodS$, $\piail_1 (a^{1}|s) > 0$. Therefore, it holds that $P^{\piail}_{2}(s^{1}) > 0, P^{\piail}_{2}(s^{2}) > 0$ and $\text{Loss}_2 (\piail_1, \widetilde{\pi}^{\ail}_2) < \text{Loss}_2 (\piail_1, \piail_2)$. Besides, it is obvious that $\text{Loss}_3 (\piail_1, \widetilde{\pi}^{\ail}_2, \piail_3) \leq \text{Loss}_3 (\piail_1, \piail_2, \piail_3) = 2$. In a word, we construct another policy $(\widetilde{\pi}^{\ail}_2, \piail_3)$ such that
\begin{align*}
    \text{Loss}_2 (\piail_1, \widetilde{\pi}^{\ail}_2) + \text{Loss}_3 (\piail_1, \widetilde{\pi}^{\ail}_2, \piail_3) < \text{Loss}_2 (\piail_1, \piail_2) + \text{Loss}_3 (\piail_1, \piail_2, \piail_3),
\end{align*}
which contradicts with the fact in \eqref{eq:piail_2_and_piail_3_are_optimal}. Hence, the original statement is true and $\exists s \in \goodS$, $\piail_2 (a^{1}|s) > 0$.

Finally, we consider the last time step. Similarly, we have that
\begin{align*}
    \piail_3 &\in \argmin_{\pi_3} \text{Loss}_3 (\piail_1, \piail_2, \pi_3)
    \\
    &= \argmin_{\pi_3} \labs 0.5 - P^{\piail}_{3}(s^{1}) \pi_3 ( a^{1}|s^{1})  \rabs + P^{\piail}_{3}(s^{1})  \pi_3 (a^{2}|s^{1})
    \\
    &\quad + \labs 0.5 - P^{\piail}_{3}(s^{2}) \pi_{3} (a^{1}|s^{2})  \rabs + P^{\piail}_{3}(s^{2})  \pi_3 (a^{2}|s^{2}) + P^{\piail}_{3}(s^{3})
    \\
    &=\argmin_{\pi_3} \labs 0.5 - P^{\piail}_{3}(s^{1}) \pi_3 ( a^{1}|s^{1})  \rabs - P^{\piail}_{3}(s^{1})  \pi_3 (a^{1}|s^{1})
    \\
    &\quad + \labs 0.5 - P^{\piail}_{3}(s^{2}) \pi_{3} (a^{1}|s^{2})  \rabs - P^{\piail}_{3}(s^{2})  \pi_3 (a^{1}|s^{2}).
\end{align*}
We have proved that for time steps $h=1$ and $h=2$, $\exists s \in \goodS$, $\piail_h (a^{1}|s) > 0$. Hence $P^{\piail}_{3}(s^{1}) > 0$ and $P^{\piail}_{3}(s^{2}) > 0$. With \cref{lem:single_variable_opt_condition}, we have that $\piail_3 (a^{1}|s^1) > 0$ and $\piail_3 (a^{1}|s^2) > 0$. We finish the whole proof. 
\end{proof}

\begin{proof}[Proof of \cref{claim:ail_reset_cliff_subsample}]
We first compute the empirical state-action distribution with subsampled expert demonstrations. Note that the data in time step $h=1$ is masked and thus the corresponding empirical distribution is uniform distribution.
\begin{align*}
    \widehat{P}^{\piE}_{1}(s^{1}, a^{1}) = \frac{1}{6}, \widehat{P}^{\piE}_{1}(s^{2}, a^{1}) = \frac{1}{6}, \widehat{P}^{\piE}_{1}(s^{3}, a^{1}) = \frac{1}{6}, \\
    \widehat{P}^{\piE}_{1}(s^{1}, a^{2}) = \frac{1}{6}, \widehat{P}^{\piE}_{1}(s^{2}, a^{2}) = \frac{1}{6}, \widehat{P}^{\piE}_{1}(s^{3}, a^{2}) = \frac{1}{6}, \\
    \widehat{P}^{\piE}_{2}(s^{1}, a^{1}) = \RED{0.5}, \widehat{P}^{\piE}_{2}(s^{2}, a^{1}) = \RED{0.5}, \widehat{P}^{\piE}_{2}(s^{3}, a^{1}) = 0.0, \\
    \widehat{P}^{\piE}_{2}(s^{1}, a^{2}) = 0.0, \widehat{P}^{\piE}_{2}(s^{2}, a^{2}) = 0.0, \widehat{P}^{\piE}_{2}(s^{3}, a^{2}) = 0.0, \\
    \widehat{P}^{\piE}_{3}(s^{1}, a^{1}) = \RED{0.5}, \widehat{P}^{\piE}_{3}(s^{2}, a^{1}) = \RED{0.5}, \widehat{P}^{\piE}_{3}(s^{3}, a^{1}) = 0.0, \\
    \widehat{P}^{\piE}_{3}(s^{1}, a^{2}) = 0.0, \widehat{P}^{\piE}_{3}(s^{2}, a^{2}) = 0.0, \widehat{P}^{\piE}_{3}(s^{3}, a^{2}) = 0.0.
\end{align*}

Recall the definition of the single-stage loss function $\text{Loss}_h (\pi)$ and the \dquote{cost-to-go} function $\ell_h (\pi)$ in time step $h$ 
\begin{align*}
    &\text{Loss}_h (\pi) = \sum_{(s, a) \in \gS \times \gA} \labs P^{\pi}_h(s, a)  - \widehat{P}^{\piE}_h(s, a) \rabs,
    \\
    &\ell_h (\pi) = \sum_{t=h}^{H} \text{Loss}_t (\pi)  = \sum_{t=h}^{H} \sum_{(s, a) \in \gS \times \gA} \labs P^{\pi}_t(s, a)  - \widehat{P}^{\piE}_t(s, a) \rabs .
\end{align*}

We perform a similar analysis to that in \cref{example:ail_success}. As $\piail = (\piail_1, \piail_2, \piail_3)$ is the optimal solution of \eqref{eq:ail}, with \cref{lem:n_vars_opt_greedy_structure}, fixing $(\piail_1, \piail_2)$, $\piail_3$ is optimal w.r.t to VAIL's objective. Notice that $P^{\piail}_1$ and $P^{\piail}_2$ are independent of $\piail_3$, so we have that
\begin{align*}
    \piail_3 &\in \argmin_{\pi_3} \text{Loss}_3 (\pi_3)
    \\
    &= \argmin_{\pi_3} \sum_{(s, a) \in \gS \times \gA} \labs P^{\pi}_3(s, a)  - \widehat{P}^{\piE}_3(s, a) \rabs  
    \\
    &= \argmin_{\pi_3}  \labs P^{\pi}_3 (s^{1}) \pi_3 (a^{1} | s^{1}) - 0.5 \rabs +  \labs P^{\pi}_3(s^{2}) \pi_3(a^{1}|s^{2}) - 0.5 \rabs + P^{\pi}_3(s^{3})  \\
    &\quad +  P^{\pi}_3(s^{1}) (1 - \pi_3(a^{1} | s^{1}))  + P^{\pi}_3(s^{2}) (1 - \pi_3(a^{1} | s^{2}))
\end{align*}

With a slight abuse of notation, we use $P^{\pi}_3$ denote the distribution induce by $(\piail_1, \piail_2, \pi_3)$ for any optimization variable $\pi_3$. Note that $\pi_3$ is the optimization variable for $\text{Loss}_3 (\pi_3)$ while $P_3^{\pi}(s^{1}) = P_3^{\piail}(s^{1})$, and $P_3^{\pi}(s^{2}) = P_3^{\piail}(s^{2}), P_3^{\pi}(s^{3}) = P_3^{\piail}(s^{3})$ are independent of $\pi_3$. We obtain
\begin{align*}
    \piail_3 &\in \argmin_{\pi_3} \labs P_3^{\piail}(s^{1}) \pi_3(a^{1} | s^{1}) - 0.5 \rabs - P^{\piail}_3(s^{1}) \pi_3(a^{1} | s^{1})  +  \labs P_3^{\piail}(s^{2}) \pi_3(a^{1}|s^{2}) - 0.5 \rabs \\
    &\quad - P^{\piail}_3(s^{2})  \pi_3(a^{1} | s^{2}).
\end{align*}
We only have two free optimization variables: $\pi_3(a^{1}|s^{1})$ and $\pi_3(a^{1}|s^{2})$ and they are independent. Then we obtain
\begin{align*}
    & \piail_3 (a^1|s^1) \in \argmin_{\pi_3 (a^1|s^1) \in [0, 1]} \labs P_3^{\piail}(s^{1}) \pi_3(a^{1} | s^{1}) - 0.5 \rabs - P^{\piail}_3(s^{1}) \pi_3(a^{1} | s^{1}),
    \\
    &\piail_3 (a^1|s^2) \in \argmin_{\pi_3 (a^1|s^2) \in [0, 1]} \labs P_3^{\piail}(s^{2}) \pi_3(a^{1}|s^{2}) - 0.5 \rabs - P^{\piail}_3(s^{2})  \pi_3(a^{1} | s^{2}).
\end{align*}
With \cref{claim:condition_for_ail_optimal_solution} and $\rho (s_1) = \rho (s_2) > 0$, it holds that $P_3^{\piail}(s^{1}) > 0$ and $P_3^{\piail}(s^{2}) > 0$. With \cref{lem:mn_variables_opt_unique}, we have that $\piail_3 (a^1|s^1) = 1$ and $\piail_3 (a^1|s^2) = 1$ are the unique optimal solutions of the above two problems, respectively. This finishes the proof in time step $h=3$.

Then we consider the policy optimization in time step $h=2$. With \cref{lem:single_variable_opt_condition}, we have that fixing $(\piail_1, \piail_3)$, $\piail_2$ is optimal w.r.t \textsf{VAIL}'s objective. Note that \textsf{VAIL}'s objective in time step $h=1$ is fixed, so we have 
\begin{align*}
    \piail_2 \in \argmin_{\pi_2} \ell_1 (\pi_2) = \argmin_{\pi_2} \text{Loss}_1 (\pi_2) + \text{Loss}_2 (\pi_2) +  \text{Loss}_3 (\pi_2) = \argmin_{\pi_2} \text{Loss}_2 (\pi_2) +  \text{Loss}_3 (\pi_2). 
\end{align*}
We have proved that $\piail_3 (a^1|s^1) = \piail_3 (a^1|s^2) = 1$ and plug it into $\text{Loss}_3 (\pi_2)$.
\begin{align*}
    \text{Loss}_3 (\pi_2) &= \labs P^{\pi}_3(s^{1}) - 0.5 \rabs + \labs P^{\pi}_3(s^{2})  - 0.5 \rabs + P^{\pi}_3(s^{3}) = 2.0 - \pi_2 (a^{1} | s^{1}) - \pi_2 (a^{1} | s^{2}),
\end{align*}
which has a unique globally optimal solution at $\pi_2 (a^{1} | s^{1}) = 1.0$ and $\pi_2 (a^{1} | s^{2}) = 1.0$. For $\text{Loss}_2 (\pi_2)$, we have
\begin{align*}
    \piail_2 &\in \argmin_{\pi_2} \text{Loss}_2 (\pi_2)
    \\
    &= \argmin_{\pi_2} \sum_{(s, a) \in \gS \times \gA} \labs P^{\pi}_2(s, a)  - \widehat{P}^{\piE}_2(s, a) \rabs  
    \\
    &= \argmin_{\pi_2}  \labs P^{\pi}_2 (s^{1}) \pi_2 (a^{1} | s^{1}) - 0.5 \rabs +  \labs P^{\pi}_2(s^{2}) \pi_2(a^{1}|s^{2}) - 0.5 \rabs + P^{\pi}_2(s^{3})  \\
    &\quad +  P^{\pi}_2(s^{1}) (1 - \pi_2(a^{1} | s^{1}))  + P^{\pi}_2(s^{2}) (1 - \pi_2(a^{1} | s^{2})).
\end{align*}
Here we use $P^{\pi}_2(s, a)$ and $P^{\pi}_2(s)$ to denote the distributions induced by $(\piail_1, \pi_2)$. Note that $\pi_2$ is the optimization variable for $\text{Loss}_2 (\pi_2)$ while $P_2^{\pi}(s^{1}) = P_2^{\piail}(s^{1}), P_2^{\pi}(s^{2}) = P_2^{\piail}(s^{2})$, and $P_2^{\pi}(s^{3}) = P_2^{\piail}(s^{3})$ are independent of $\pi_2$. Then we have that
\begin{align*}
    \piail_2 &\in \argmin_{\pi_2} \labs P_2^{\piail}(s^{1}) \pi_2(a^{1} | s^{1}) - 0.5 \rabs - P^{\piail}_2(s^{1}) \pi_2(a^{1} | s^{1})  +  \labs P_2^{\piail}(s^{2}) \pi_2(a^{1}|s^{2}) - 0.5 \rabs \\
    &\quad - P^{\piail}_2(s^{2})  \pi_2(a^{1} | s^{2}).
\end{align*}
With \cref{lem:single_variable_opt}, we have that $\piail_2 (a^1|s^1) = 1, \piail_2 (a^1|s^2) = 1$ is the optimal solution of $\text{Loss}_2 (\pi_2)$. Thus, $\piail_2 (a^1|s^1) = 1, \piail_2 (a^1|s^2) = 1$ is the unique optimal solution of optimization problem $\argmin_{\pi_2} \text{Loss}_2 (\pi_2) +  \text{Loss}_3 (\pi_2)$. We finish the proof in time step $h=2$.

Finally, we consider the policy optimization in time step $h=1$. With \cref{lem:single_variable_opt_condition}, we have that fixing $(\piail_2, \piail_3)$, $\piail_1$ is optimal w.r.t \textsf{VAIL}'s objective. 
\begin{align*}
    \piail_1 \in \argmin_{\pi_1} \ell_1 (\pi_1) = \argmin_{\pi_1} \text{Loss}_1 (\pi_1) + \text{Loss}_2 (\pi_1) +  \text{Loss}_3 (\pi_1) . 
\end{align*}
Note that we have proved that $\piail_2 (a^1|s^1) = \piail_2 (a^1|s^2) = \piail_3 (a^1|s^1) = \piail_3 (a^1|s^2) = 1$ and plug it into the above equation. We use $P^{\pi}$ to denote the distribution induced by $(\pi_1, \piail_2, \piail_3)$.
\begin{align*}
    \text{Loss}_1 (\pi_1) &= \labs P^{\pi}_1(s^{1}, a^{1}) - \frac{1}{6}  \rabs + \labs P^{\pi}_1(s^{1}, a^{2}) - \frac{1}{6}  \rabs + \labs P^{\pi}_1(s^{2}, a^{1}) - \frac{1}{6}  \rabs + \labs P^{\pi}_1(s^{2}, a^{2}) - \frac{1}{6}  \rabs + \frac{1}{3}
    \\
    &= \labs \frac{1}{2} \pi_1 (a^{1}|s^{1}) - \frac{1}{6} \rabs + \labs \frac{1}{2} \pi_1 (a^{1}|s^{1}) - \frac{1}{3} \rabs + \labs \frac{1}{2} \pi_1 (a^{1}|s^{2}) - \frac{1}{6} \rabs + \labs \frac{1}{2} \pi_1 (a^{1}|s^{2}) - \frac{1}{3} \rabs + \frac{1}{3},  
    \\
    \text{Loss}_2 (\pi_1) &= \labs P^{\pi}_2(s^{1}) - 0.5 \rabs + \labs P^{\pi}_2(s^{2})  - 0.5 \rabs + P^{\pi}_2(s^{3})
    \\
    &= \labs \frac{1}{4} \lp \pi_1 (a^{1}|s^{1}) + \pi_1 (a^{1}|s^{2}) \rp - 0.5 \rabs + \labs \frac{1}{4} \lp \pi_1 (a^{1}|s^{1}) + \pi_1 (a^{1}|s^{2}) \rp - 0.5 \rabs \\
    &\quad +\frac{1}{2} \lp 2 - \pi_1 (a^{1}|s^{1}) - \pi_1 (a^{1}|s^{2})   \rp,
    \\
    &= 2 - \pi_1 (a^1|s^1) - \pi_1 (a^1|s^2),  
    \\
    \text{Loss}_3 (\pi_1) &= \labs P^{\pi}_3(s^{1}) - 0.5 \rabs + \labs P^{\pi}_3(s^{2})  - 0.5 \rabs + P^{\pi}_3(s^{3})
    \\
    &= \labs \frac{1}{2} \lp P^{\pi}_2 (s^{1}) + P^{\pi}_2 (s^{1}) \rp - 0.5 \rabs + \labs  \frac{1}{2} \lp P^{\pi}_2 (s^{1}) + P^{\pi}_2 (s^{1}) \rp  - 0.5 \rabs + P^{\pi}_2(s^{3})
    \\
    &= \labs \frac{1}{4} \lp \pi_1 (a^{1}|s^{1}) + \pi_1 (a^{1}|s^{2}) \rp - 0.5 \rabs + \labs \frac{1}{4} \lp \pi_1 (a^{1}|s^{1}) + \pi_1 (a^{1}|s^{2}) \rp - 0.5 \rabs \\
    &\quad +
    \frac{1}{2} \lp 2 - \pi_1 (a^{1}|s^{1}) - \pi_1 (a^{1}|s^{2})   \rp
    \\
    &= 2 - \pi_1 (a^1|s^1) - \pi_1 (a^1|s^2). 
\end{align*}
Combining the above three equations yields that
\begin{align*}
     &\quad \argmin_{\pi_1} \text{Loss}_1 (\pi_1) + \text{Loss}_2 (\pi_1) +  \text{Loss}_3 (\pi_1)
     \\
     &= \argmin_{\pi_1} \labs \frac{1}{2} \pi_1 (a^{1}|s^{1}) - \frac{1}{6} \rabs + \labs \frac{1}{2} \pi_1 (a^{1}|s^{1}) - \frac{1}{3} \rabs + \labs \frac{1}{2} \pi_1 (a^{1}|s^{2}) - \frac{1}{6} \rabs + \labs \frac{1}{2} \pi_1 (a^{1}|s^{2}) - \frac{1}{3} \rabs
     \\
     &\quad - 2\pi_1 (a^1|s^1) - 2\pi_1 (a^1|s^2).
\end{align*}
Note that $\pi_1 (a^1|s^1)$ and $\pi_1 (a^1|s^2)$ are independent and we can view the optimization problem individually.
\begin{align*}
    \argmin_{\pi_1 (a^{1}|s^{1}) \in [0, 1]} \labs \frac{1}{2} \pi_1 (a^{1}|s^{1}) - \frac{1}{6} \rabs + \labs \frac{1}{2} \pi_1 (a^{1}|s^{1}) - \frac{1}{3} \rabs - 2\pi_1 (a^1|s^1).  
\end{align*}
This is a piece-wise linear function and it is direct to see that $\piail_1 (a^1|s^1)=1$ is the unique optimal solution. In the same way, we can also prove that $\piail_1 (a^1|s^2)=1$ is the unique optimal solution. Therefore, we finish the proof in the step $h=1$. 

\end{proof}

\subsection{VAIL with Approximately Optimal Solutions}
\label{appendix:proof_of_the_approximate_solution_in_VAIL}

Here we consider the generalization of an approximately optimal solution of \textsf{VAIL}'s objective instead of the exactly optimal solution discussed in \cref{sec:generalization_of_ail}. In particular, for a policy $\pi$, given estimation $\widehat{P}^{\piE}_h(s, a)$, \textsf{VAIL}'s objective is formulated as
\begin{align*}
    \min_{\pi \in \Pi} f(\pi) := \sum_{h=1}^H \text{Loss}_h (\pi) =  \sum_{h=1}^{H} \sum_{(s, a) \in \gS \times \gA} | P^{\pi}_h(s, a) - \widehat{P}^{\piE}_h(s, a) |.
\end{align*}
Here $\text{Loss}_h (\pi) = \sum_{(s, a) \in \gS \times \gA} | P^{\pi}_h(s, a) - \widehat{P}^{\piE}_h(s, a) |$. Suppose that we can get an $\varepsilon_{\ail}$-approximately optimal solution $\widebar{\pi}$ instead of the exact optimal solution $\piail$. More specifically, it holds that
\begin{align*}
    f (\widebar{\pi}) \leq \min_{\pi \in \Pi} f(\pi) + \varepsilon_{\ail} = f(\piail) + \varepsilon_{\ail} .  
\end{align*}
We consider the generalization of $\widebar{\pi}$ on Standard Imitation and Reset Cliff. Note that the analysis of the approximately optimal solution on Standard Imitation is straightforward. To see this, through the reduction analysis, we can directly plug the optimization error into the final policy value gap.  
\begin{align*}
    V^{\piE} - V^{\widebar{\pi}} &= \sum_{h=1}^{H} \sum_{(s, a) \in \gS \times \gA} \lp P^{\piE}_h(s, a) - P^{\widebar{\pi}}_h(s, a) \rp r_h(s, a)
    \\
    &\leq \sum_{h=1}^{H} \lnorm P^{\piE}_h(\cdot, \cdot) - P^{\widebar{\pi}}_h(\cdot, \cdot)  \rnorm_{1}
    \\
    &\leq  \sum_{h=1}^{H} \lnorm P^{\piE}_h(\cdot, \cdot) - \widehat{P}^{\piE}_h(\cdot, \cdot)  \rnorm_{1} +  \sum_{h=1}^{H} \lnorm \widehat{P}^{\piE}_h(\cdot, \cdot) - P^{\widebar{\pi}}_h(\cdot, \cdot)  \rnorm_{1}
    \\
    &\leq \sum_{h=1}^{H} \lnorm P^{\piE}_h(\cdot, \cdot) - \widehat{P}^{\piE}_h(\cdot, \cdot)  \rnorm_{1} +  \min_{\pi \in \Pi} \sum_{h=1}^{H} \lnorm \widehat{P}^{\piE}_h(\cdot, \cdot) - P^{\pi}_h(\cdot, \cdot)  \rnorm_{1} + \varepsilon_{\ail}
    \\
    &\leq 2\sum_{h=1}^{H} \lnorm P^{\piE}_h(\cdot, \cdot) - \widehat{P}^{\piE}_h(\cdot, \cdot)  \rnorm_{1} + \varepsilon_{\ail}. 
\end{align*}

Thus, it is straightforward to obtain the following theoretical guarantee. 
\begin{thm}[Sample Complexity of Approximate VAIL]  \label{theorem:sample_complexity_approximate_vail}
For any tabular and episodic MDP, assume $\widebar{\pi}$ is an $\varepsilon_{\ail}$-approximately optimal solution of \eqref{eq:ail}. To obtain an $\varepsilon$-optimal policy (i.e., $V^{\piE} - \expect[V^{\widebar{\pi}}] \leq \varepsilon$), in expectation, when $\varepsilon_{\ail} \leq \varepsilon/2$, VAIL requires at most $\gO(|\gS| H^2/\varepsilon^2)$ expert trajectories. 
\end{thm}

However, the analysis of the approximately optimal solution on Reset Cliff is non-trivial. On Reset Cliff, we hope to obtain a tight horizon-free sample complexity as in \cref{theorem:ail_reset_cliff} and thus we cannot apply the reduction analysis. Here we briefly discuss the proof idea. To achieve a horizon-free sample complexity, we first develop a sharp analysis to measure the distance between the approximately optimal solution and the exactly optimal solution in \cref{prop:ail_general_reset_cliff_approximate_solution}. With \cref{prop:ail_general_reset_cliff_approximate_solution}, we can upper bound the policy value gap of the approximately optimal solution and obtain the corresponding sample complexity.

First, we present a useful property of \textsf{VAIL}'s objective on Reset Cliff.

\begin{lem}
\label{lemma:ail_policy_ail_objective_equals_expert_policy_ail_objective}
Consider the Reset Cliff MDP satisfying \cref{asmp:reset_cliff}. Suppose that $\piail$ is the optimal solution of \eqref{eq:ail}, then we have that $f(\piail) = f(\piE)$.
\end{lem}
Refer to \cref{appendix:proof_lemma:ail_policy_ail_objective_equals_expert_policy_ail_objective} for the proof. The following proposition demonstrates that the distance between the approximately optimal solution and the exactly optimal solution can be upper bounded by the optimization error. 

\begin{prop}
\label{prop:ail_general_reset_cliff_approximate_solution}
Consider any tabular and episodic MDP satisfying \cref{asmp:reset_cliff}. The candidate policy set is defined as $\Pi^{\text{opt}} = \{ \pi \in \Pi: \forall h \in [H], \exists s \in \goodS, \pi_h (a^{1}|s) > 0 \}$. Given expert state-action distribution estimation $\widehat{P}^{\piE}_{H}$, suppose that $\widebar{\pi} \in \Pi^{\text{opt}}$ is an $\varepsilon_{\ail}$-approximately optimal solution of \eqref{eq:ail}, when $\vert \gD \vert \geq 1$, we have the following approximate optimality condition almost surely:
\begin{align*}
    c (\widebar{\pi}) \lp \sum_{h=1}^{H} \sum_{\ell=1}^{h-1} \sum_{s \in \goodS} P^{\widebar{\pi}}_{\ell} (s) \lp 1 - \widebar{\pi}_{\ell} (a^{1}|s)  \rp + \sum_{s \in  \gS^{\widebar{\pi}}_H}  P^{\widebar{\pi}}_{H} (s) \lp \min\{1,  \widehat{P}^{\piE}_{H} (s) / P^{\piE}_H (s)\} -  
    \widebar{\pi}_H (a^1|s)  \rp  \rp \leq \varepsilon_{\ail},
\end{align*}
where $c (\pi) := \min_{1 \leq \ell < h \leq H, s, s^\prime \in \goodS} \{ \sP^{\pi} \lp s_{h} = s |s_{\ell} = s^\prime, a_{\ell} = a^{1} \rp \}$ and $\gS^{\pi}_H  = \{s \in \goodS, \pi_H (a^1|s) \leq \min \{1,  \widehat{P}^{\piE}_{H} (s) / P^{\piE}_H (s) \}  \}$. Note that $c(\pi) > 0$ for any $\pi \in \Pi^{\text{opt}}$.
\end{prop}

This proof is rather technical and is deferred to \cref{appendix:proof_prop:ail_general_reset_cliff_approximate_solution}. We explain \cref{prop:ail_general_reset_cliff_approximate_solution} by connecting it with \cref{prop:ail_general_reset_cliff}. In particular, if $\varepsilon_{\ail} = 0$, we can show that the optimality condition in  \cref{prop:ail_general_reset_cliff_approximate_solution} reduces to the one in \cref{prop:ail_general_reset_cliff}. To see this, for each $h \in [H-1]$ and $s \in \goodS$, since $c(\widebar{\pi}) > 0$ and $P^{\widebar{\pi}}_h (s) > 0$, we must have $\widebar{\pi}_{h}(a^{1} | s) = 1$ for all $h \in [H-1]$ while there exists many optimal solutions in the last step policy optimization.

Equipped with \cref{prop:ail_general_reset_cliff} and \cref{prop:ail_general_reset_cliff_approximate_solution}, we can obtain the horizon-free sample complexity for the approximately optimal solution of \textsf{VAIL} in \cref{theorem:ail_approximate_reset_cliff}.

\begin{thm}[Horizon-free Sample Complexity of Approximate \textsf{VAIL} on \textsf{Reset Cliff}]
\label{theorem:ail_approximate_reset_cliff}
For each tabular and episodic MDP satisfying \cref{asmp:reset_cliff}, the candidate policy set is defined as $\Pi^{\text{opt}} = \{ \pi \in \Pi: \forall h \in [H], \exists s \in \goodS, \pi_h (a^{1}|s) > 0 \}$. Suppose that $\widebar{\pi} \in \Pi^{\text{opt}} $ is an $\varepsilon_{\ail}$-approximately optimal solution of \eqref{eq:ail}, to obtain an $\varepsilon$-optimal policy (i.e., $V^{\piE} - \expect[V^{\widebar{\pi}}] \leq \varepsilon$), in expectation, when $\varepsilon_{\ail}  \leq \varepsilon/8 \cdot  c(\widebar{\pi})$, \textsf{VAIL} requires at most ${\gO}(|\gS|/\varepsilon^2)$ expert trajectories. Here
$c (\pi) := \min_{1 \leq \ell < h \leq H, s, s^\prime \in \goodS} \{ \sP^{\pi} \lp s_{h} = s |s_{\ell} = s^\prime, a_{\ell} = a^{1} \rp \}$.
\end{thm}

\begin{thm}[High Probability Version of \cref{theorem:ail_approximate_reset_cliff}]
\label{theorem:ail_approximate_high_prob_reset_cliff}
For each tabular and episodic MDP satisfying \cref{asmp:reset_cliff}, the candidate policy set is defined as $\Pi^{\text{opt}} = \{ \pi \in \Pi: \forall h \in [H], \exists s \in \goodS, \pi_h (a^{1}|s) > 0 \}$. Suppose that $\widebar{\pi} \in \Pi^{\text{opt}} $ is an $\varepsilon_{\ail}$-approximately optimal solution of \eqref{eq:ail}, with probability at least $1-\delta$, to obtain an $\varepsilon$-optimal policy (i.e., $V^{\piE} - V^{\widebar{\pi}} \leq \varepsilon$), when $ \varepsilon_{\ail}  \leq \varepsilon/8 \cdot  c(\widebar{\pi})$, \textsf{VAIL} requires at most ${\widetilde{\gO}}(|\gS|/\varepsilon^2)$ expert trajectories.
\end{thm}

\begin{proof}[Proof of \cref{theorem:ail_approximate_reset_cliff} and \cref{theorem:ail_approximate_high_prob_reset_cliff}]
With a fixed estimation, we consider \textsf{VAIL}'s objective.
\begin{align*}
    \min_{\pi \in \Pi} \sum_{h=1}^{H} \sum_{(s, a) \in \gS \times \gA} | P^{\pi}_h(s, a) - \widehat{P}^{\piE}_h(s, a) |.
\end{align*}
Suppose that $\widebar{\pi}$ is $\varepsilon_{\ail}$-optimal w.r.t the above objective. We construct an optimal solution $\piail$ in the following way.

\begin{itemize}
    \item By \cref{prop:ail_general_reset_cliff}, we have $\forall h \in [H-1], s \in \goodS, \piail_{h} (a^{1}|s) = \piE_{h} (a^{1}|s)$.
    
    \item For the last time step $H$, we defined a set of states $\gS_H^1 := \{s \in \goodS: \widehat{P}^{\piE}_H (s) < P^{\piE}_H (s)   \}$. The policy in the last time step is defined as $\forall s \in \gS_H^1$, $\piail_{H} (a^{1}|s) = \widehat{P}^{\piE}_H (s) / P^{\piE}_H (s)$ and $\forall s \in \goodS \setminus \gS_H^1$, $\piail_{H} (a^{1}|s) = 1$. In a word, $\forall s \in \goodS$, $\piail_{H} (a^{1}|s) = \min \{\widehat{P}^{\piE}_H (s) / P^{\piE}_H (s),1  \}$.
    
    \item For simplicity of analysis, we also define the policy on bad states although $\piail$ never visit bad states. $\forall h \in [H], s \in \badS, \piail_{h} (\cdot|s) = \widebar{\pi}_{h} (\cdot|s)$.   
\end{itemize}

We first verify that $\piail$ is the optimal solution of \eqref{eq:ail}. With \cref{prop:ail_general_reset_cliff}, we have that $\forall h \in [H-1], s \in \goodS, \piail_{h} (a^{1}|s) = \piE_{h} (a^{1}|s)$ is the \emph{unique} optimal solution of \eqref{eq:ail}. Furthermore, with fixed $ \piail_{h} (a^{1}|s) = \piE_{h} (a^{1}|s), \forall h \in [H-1], s \in \goodS$, \textsf{VAIL}'s objective from time step $1$ to $H-1$ is fixed. Therefore, it suffices to verify that with fixed $ \piail_{h} (a^{1}|s) = \piE_{h} (a^{1}|s), \forall h \in [H-1], s \in \goodS$, $\piail_{H}$ is optimal w.r.t the \textsf{VAIL}'s objective in the last time step. Thus, we take the policy in the last time step as optimization variables and consider \textsf{VAIL}'s objective in the last time step.
\begin{align*}
    & \quad \min_{\pi_H} \sum_{(s, a) \in \gS \times \gA} | P^{\piail}_H (s) \pi_H (a|s) - \widehat{P}^{\piE}_H (s, a) |
    \\
    &=  \min_{\pi_H} \sum_{(s, a) \in \gS \times \gA} | P^{\piE}_H (s) \pi_H (a|s) - \widehat{P}^{\piE}_H (s, a) |
    \\
    &=  \min_{\pi_H} \sum_{s \in \goodS } \lp  | P^{\piE}_H (s) \pi_H (a^{1}|s) - \widehat{P}^{\piE}_H (s) | + P^{\piE}_H (s) \lp 1- \pi_H (a^{1}|s) \rp  \rp
    \\
    &= \min_{\pi_H} \sum_{s \in \goodS } \lp  | P^{\piE}_H (s) \pi_H (a^{1}|s) - \widehat{P}^{\piE}_H (s) | - P^{\piE}_H (s)  \pi_H (a^{1}|s)  \rp .
\end{align*}
We can view the optimization problem for each $s \in \goodS$ individually.
\begin{align*}
    \forall s \in \goodS, \min_{\pi_H (a^{1}|s) \in [0, 1]}   | P^{\piE}_H (s) \pi_H (a^{1}|s) - \widehat{P}^{\piE}_H (s) | - P^{\piE}_H (s)  \pi_H (a^{1}|s) .
\end{align*}
For $s \in \gS_H^1$, by \cref{lem:single_variable_opt_condition}, we have that $ \piail_{H} (a^{1}|s) = \widehat{P}^{\piE}_H (s) / P^{\piE}_H (s)$ is the optimal solution. For $s \in \goodS \setminus \gS_H^1$, by \cref{lem:single_variable_opt}, we have that $ \piail_{H} (a^{1}|s) =1$ is the optimal solution. Therefore, we show that $\piail_{H}$ is also optimal w.r.t the \textsf{VAIL}'s objective in the last time step and hence $\piail$ is the optimal solution of \eqref{eq:ail}.

Now we consider the policy value gap of $\widebar{\pi}$.
\begin{align}
\label{eq:value_gap_decomposition_approximate_solution}
    V^{\piE} - V^{\widebar{\pi}} = V^{\piE} - V^{\piail} + V^{\piail} -  V^{\widebar{\pi}}. 
\end{align}
By \eqref{eq:value_gap_ail_policy} in the proof of \cref{theorem:ail_reset_cliff}, we have that
\begin{align}
\label{eq:ail_policy_piE_value_gap}
    V^{\piE} - V^{\piail} \leq 2 \sum_{s \in \gS} \labs \widehat{P}^{\piE}_H (s) - P^{\piE}_H (s)  \rabs.
\end{align}
Then we consider the policy value gap between $\piail$ and $\widebar{\pi}$. With the dual representation of policy value, we get that
\begin{align*}
    V^{\piail} -  V^{\widebar{\pi}} &= \sum_{h=1}^{H-1} \sum_{(s, a) \in \gS \times \gA} \lp P^{\piail}_h (s, a) - P^{\widebar{\pi}}_h (s, a)  \rp r_h (s, a) + \sum_{(s, a) \in \gS \times \gA} \lp P^{\piail}_H (s, a) - P^{\widebar{\pi}}_H (s, a)  \rp r_H (s, a)
    \\
    &\leq \sum_{h=1}^{H-1} \lnorm P^{\piail}_h (\cdot, \cdot) - P^{\widebar{\pi}}_h (\cdot, \cdot) \rnorm_{1} + \sum_{(s, a) \in \gS \times \gA} \lp P^{\piail}_H (s, a) - P^{\widebar{\pi}}_H (s, a)  \rp r_H (s, a), 
\end{align*}
where we use $P^{\pi}_h (\cdot, \cdot)$ denote the state-action distribution induced by $\pi$. Recall the definition of $\gS^{\pi}_H  = \{s \in \goodS, \pi_H (a^1|s) \leq \min \{1,  \widehat{P}^{\piE}_{H} (s) / P^{\piE}_H (s) \}  \}$ introduced in \cref{prop:ail_general_reset_cliff_approximate_solution}. For the second term in RHS, we have
\begin{align*}
    &\quad \sum_{(s, a) \in \gS \times \gA} \lp P^{\piail}_H (s, a) - P^{\widebar{\pi}}_H (s, a)  \rp r_H (s, a)
    \\
    &= \sum_{s \in \goodS}  \lp P^{\piail}_H (s, a^{1}) - P^{\widebar{\pi}}_H (s, a^{1})  \rp
    \\
    &= \sum_{s \in \goodS}  \lp P^{\piail}_H (s) \piail_{H} \lp a^{1}|s \rp - P^{\widebar{\pi}}_H (s) \widebar{\pi}_H (a^{1}|s)  \rp
    \\
    &=  \sum_{s \in \goodS}   \lp P^{\piail}_H (s) - P^{\widebar{\pi}}_H (s) \rp  \piail_{H} \lp a^{1}|s \rp + \sum_{s \in \goodS} P^{\widebar{\pi}}_H (s) \lp \piail_{H} \lp a^{1}|s \rp -   \widebar{\pi}_H (a^{1}|s) \rp
    \\
    &\leq \lnorm P^{\piail}_H (\cdot) - P^{\widebar{\pi}}_H (\cdot) \rnorm_1 + \sum_{s: s \in \goodS, \piail_{H} \lp a^{1}|s \rp \geq   \widebar{\pi}_H (a^{1}|s)} P^{\widebar{\pi}}_H (s) \lp \piail_{H} \lp a^{1}|s \rp -   \widebar{\pi}_H (a^{1}|s) \rp
    \\
    &= \lnorm P^{\piail}_H (\cdot) - P^{\widebar{\pi}}_H (\cdot) \rnorm_1 + \sum_{s \in \gS^{\widebar{\pi}}_H} P^{\widebar{\pi}}_H (s) \lp \piail_{H} \lp a^{1}|s \rp -   \widebar{\pi}_H (a^{1}|s) \rp,
\end{align*}
where we use $P^{\pi}_h (\cdot)$ to denote the state distribution induced by $\pi$. Plugging the above inequality into the policy value gap yields
\begin{align*}
    V^{\piail} -  V^{\widebar{\pi}} &\leq \sum_{h=1}^{H-1} \lnorm P^{\piail}_h (\cdot, \cdot) - P^{\widebar{\pi}}_h (\cdot, \cdot) \rnorm_{1} + \lnorm P^{\piail}_H (\cdot) - P^{\widebar{\pi}}_H (\cdot) \rnorm_1  + \sum_{s \in \gS^{\widebar{\pi}}_H} P^{\widebar{\pi}}_H (s) \lp \piail_{H} \lp a^{1}|s \rp -   \widebar{\pi}_H (a^{1}|s) \rp.
\end{align*}
With \cref{lemma:state_dist_discrepancy}, we have that
\begin{align*}
    &\quad \sum_{h=1}^{H-1} \lnorm P^{\piail}_h (\cdot, \cdot) - P^{\widebar{\pi}}_h (\cdot, \cdot) \rnorm_{1} + \lnorm P^{\piail}_H (\cdot) - P^{\widebar{\pi}}_H (\cdot) \rnorm_1 
    \\
    &\leq \sum_{h=1}^{H-1} \lnorm P^{\piail}_h (\cdot) - P^{\widebar{\pi}}_h (\cdot) \rnorm_{1} + \sum_{h=1}^{H-1} \expect_{s \sim P^{\widebar{\pi}}_h (\cdot)} \ls \lnorm \piail_h (\cdot|s) - \widebar{\pi}_h (\cdot|s) \rnorm_1 \rs + \lnorm P^{\piail}_H (\cdot) - P^{\widebar{\pi}}_H (\cdot) \rnorm_1
    \\
    &= \sum_{h=1}^{H} \lnorm P^{\piail}_h (\cdot) - P^{\widebar{\pi}}_h (\cdot) \rnorm_{1} + \sum_{h=1}^{H-1} \expect_{s \sim P^{\widebar{\pi}}_h (\cdot)} \ls \lnorm \piail_h (\cdot|s) - \widebar{\pi}_h (\cdot|s) \rnorm_1 \rs
    \\
    &= \sum_{h=1}^{H} \sum_{\ell=1}^{h-1} \expect_{s \sim P^{\widebar{\pi}}_\ell (\cdot)} \ls \lnorm \piail_\ell (\cdot|s) - \widebar{\pi}_\ell (\cdot|s) \rnorm_1 \rs + \sum_{h=1}^{H-1} \expect_{s \sim P^{\widebar{\pi}}_h (\cdot)} \ls \lnorm \piail_h (\cdot|s) - \widebar{\pi}_h (\cdot|s) \rnorm_1 \rs
    \\
    &\leq 2  \sum_{h=1}^{H} \sum_{\ell=1}^{h-1} \expect_{s \sim P^{\widebar{\pi}}_\ell (\cdot)} \ls \lnorm \piail_\ell (\cdot|s) - \widebar{\pi}_\ell (\cdot|s) \rnorm_1 \rs.
\end{align*}
Then we have that
\begin{align*}
    V^{\piail} -  V^{\widebar{\pi}} &\leq 2  \sum_{h=1}^{H} \sum_{\ell=1}^{h-1} \expect_{s \sim P^{\widebar{\pi}}_\ell (\cdot)} \ls \lnorm \piail_\ell (\cdot|s) - \widebar{\pi}_\ell (\cdot|s) \rnorm_1 \rs +  \sum_{s \in \gS^{\widebar{\pi}}_H} P^{\widebar{\pi}}_H (s) \lp \piail_{H} \lp a^{1}|s \rp -   \widebar{\pi}_H (a^{1}|s) \rp.
\end{align*}

Notice that $\piail$ agrees with $\widebar{\pi}$ on bad states and we obtain
\begin{align*}
     \expect_{s \sim P^{\widebar{\pi}}_{\ell} (\cdot)} \ls \lnorm \piail_{\ell} (\cdot|s) - \widebar{\pi}_{\ell} (\cdot|s) \rnorm_1 \rs &= \sum_{s \in \goodS } P^{\widebar{\pi}}_{\ell} (s)    \lnorm \piail_{\ell} (\cdot|s) - \widebar{\pi}_{\ell} (\cdot|s) \rnorm_1
    \\
    &=  \sum_{s \in \goodS } P^{\widebar{\pi}}_{\ell} (s) \lp \labs \piail_{\ell} (a^{1}|s) - \widebar{\pi}_{\ell} (a^{1}|s)  \rabs + \sum_{a \in \gA \setminus \{a^{1}\}} \widebar{\pi}_{\ell} (a|s)  \rp
    \\
    &= 2 \sum_{s \in \goodS } P^{\widebar{\pi}}_{\ell} (s)    \lp 1 - \widebar{\pi}_{\ell} (a^{1}|s) \rp.
\end{align*}
In the penultimate inequality, we use the fact that $\forall \ell \in [H-1], s \in \goodS, \piail_{\ell} (a^{1}|s) = 1$. Then we have that
\begin{align*}
    V^{\piail} -  V^{\widebar{\pi}} &\leq 4  \sum_{h=1}^{H} \sum_{\ell=1}^{h-1} \sum_{s \in \goodS } P^{\widebar{\pi}}_{\ell} (s)    \lp 1 - \widebar{\pi}_{\ell} (a^{1}|s) \rp +  \sum_{s \in \gS^{\widebar{\pi}}_H} P^{\widebar{\pi}}_H (s) \lp \piail_{H} \lp a^{1}|s \rp -   \widebar{\pi}_H (a^{1}|s) \rp.
\end{align*}
Then we consider the second term in RHS. For the last time step $H$, notice that $\piail_{H} (a^{1}|s)  = \min\{ \widehat{P}^{\piE}_H (s) / P^{\piE}_H (s), 1  \}$. Then we have
\begin{align*}
    \sum_{s \in \gS^{\widebar{\pi}}_H} P^{\widebar{\pi}}_H (s) \lp \piail_{H} \lp a^{1}|s \rp -   \widebar{\pi}_H (a^{1}|s) \rp \leq \sum_{s \in \gS^{\widebar{\pi}}_H} P^{\widebar{\pi}}_H (s) \lp \min\lb \frac{\widehat{P}^{\piE}_H (s)}{P^{\piE}_H (s)},  1  \rb -   \widebar{\pi}_H (a^{1}|s) \rp. 
\end{align*}
Combing the above inequality with $V^{\piail} -  V^{\widebar{\pi}}$ yields that
\begin{align*}
    V^{\piail} -  V^{\widebar{\pi}} &\leq 4  \sum_{h=1}^{H} \sum_{\ell=1}^{h-1} \sum_{s \in \goodS } P^{\widebar{\pi}}_{\ell} (s)    \lp 1 - \widebar{\pi}_{\ell} (a^{1}|s) \rp + \sum_{s \in \gS^{\widebar{\pi}}_H} P^{\widebar{\pi}}_H (s) \lp \min\lb \frac{\widehat{P}^{\piE}_H (s)}{P^{\piE}_H (s)},  1  \rb -   \widebar{\pi}_H (a^{1}|s) \rp.
\end{align*}
We apply \cref{prop:ail_general_reset_cliff_approximate_solution} and get that
\begin{align*}
    V^{\piail} -  V^{\widebar{\pi}} &\leq 4 \lp \sum_{h=1}^{H} \sum_{\ell=1}^{h-1} \sum_{s \in \goodS } P^{\widebar{\pi}}_{\ell} (s)    \lp 1 - \widebar{\pi}_{\ell} (a^{1}|s) \rp + \sum_{s \in \gS^{\widebar{\pi}}_H} P^{\widebar{\pi}}_H (s) \lp \min\lb \frac{\widehat{P}^{\piE}_H (s)}{P^{\piE}_H (s)},  1  \rb -   \widebar{\pi}_H (a^{1}|s) \rp \rp
    \\
    &\leq \frac{4}{c (\widebar{\pi})} \varepsilon_{\ail}.
\end{align*}

We first consider the sample complexity required to achieve a small policy value gap with high probability. With \eqref{eq:value_gap_decomposition_approximate_solution} and \eqref{eq:ail_policy_piE_value_gap}, we have
\begin{align*}
    V^{\piE} - V^{\widebar{\pi}} &= V^{\piE} - V^{\piail} + V^{\piail} -  V^{\widebar{\pi}}
    \\
    &\leq 2 \sum_{s \in \gS} \labs \widehat{P}^{\piE}_H (s) - P^{\piE}_H (s)  \rabs + \frac{4}{c (\widebar{\pi})} \varepsilon_{\ail}
    \\
    &=  2 \lnorm \widehat{P}^{\piE}_H (\cdot) - P^{\piE}_H (\cdot) \rnorm_{1} + \frac{4}{c (\widebar{\pi})} \varepsilon_{\ail}. 
\end{align*}
By $\ell_1$-norm concentration inequality in \cref{lemma:l1_concentration}, with probability at least $1-\delta$, we have 
\begin{align*}
    V^{\piE} - V^{\widebar{\pi}} \leq 2\sqrt{\frac{2 \vert \gS \vert \ln (1/\delta)}{m}} + \frac{4}{c (\widebar{\pi})} \varepsilon_{\ail}. 
\end{align*}
To achieve an $\varepsilon$-optimal policy, when $4 \varepsilon_{\ail} / c(\widebar{\pi}) \leq \varepsilon/2$, we need a sample complexity of $\widetilde{\gO} (|\gS|/\varepsilon^2)$ at most.

We proceed to upper bound the expected policy value gap between $\widebar{\pi}$ and $\piE$ in expectation, with \eqref{eq:value_gap_decomposition_approximate_solution} and \eqref{eq:ail_policy_piE_value_gap}, we have 
\begin{align*}
    \expect \ls V^{\piE} - V^{\widebar{\pi}} \rs &=  \expect \ls V^{\piE} - V^{\piail} \rs + \expect \ls V^{\piail} -  V^{\widebar{\pi}} \rs
    \\
    &\leq 2 \expect \ls \sum_{s \in \gS} \labs \widehat{P}^{\piE}_H (s) - P^{\piE}_H (s)  \rabs \rs + \frac{4}{c (\widebar{\pi})} \varepsilon_{\ail}
    \\
    &= 2 \expect \ls  \lnorm \widehat{P}^{\piE}_H (\cdot) - P^{\piE}_H (\cdot) \rnorm_{1}  \rs + \frac{4}{c (\widebar{\pi})} \varepsilon_{\ail}, 
\end{align*}
where the expectation is taken w.r.t the randomness of expert demonstrations. We apply the upper bound of the expected $\ell_1$ risk of empirical distribution \citep[Theorem 1]{han2015minimax} and obtain
\begin{align*}
    \expect \ls V^{\piE} - V^{\widebar{\pi}} \rs \leq 2 \sqrt{ \frac{|\gS| - 1}{m}} + \frac{4}{c (\widebar{\pi})} \varepsilon_{\ail}.
\end{align*}
To achieve an $\varepsilon$-optimal policy (i.e., $\expect[V^{\piE} - V^{\piail}] \leq \varepsilon$), when $4 \varepsilon_{\ail} / c(\widebar{\pi}) \leq \varepsilon/2$, we need a sample complexity of $\gO(|\gS|/\varepsilon^2)$ at most.
\end{proof}

\subsection{Horizon-free Sample Complexity of MIMIC-MD on Reset Cliff}
\label{appendix:horizon_free_complexity_of_mimic_md}

Here we show the horizon-free sample complexity of MIMIC-MD \citep{rajaraman2020fundamental} on Reset Cliff. With the estimator $\widetilde{P}_h^{\piE}$ in \eqref{eq:new_estimator}, MIMIC-MD performs the state-action distribution matching like VAIL.
\begin{align*}
    \min_{\pi \in \Pi_{\text{BC}} \lp \gD_1 \rp} \sum_{h=1}^{H} \sum_{(s, a) \in \gS \times \gA} | P^{\pi}_h(s, a) - \widetilde{P}^{\piE}_h(s, a) |,
\end{align*}
where $\Pi_{\text{BC}} (\gD_1) = \{ \pi \in \Pi: \pi_h (s) = \piE_h (s), \forall h \in [H], s \in \gS_h (\gD_1) \}$ is the set of BC policies on $\gD_1$.

\begin{thm}[High Probability Version of \cref{theorem:ail_mimic_md}]     \label{theorem:ail_mimic_md_high_prob}
For each tabular and episodic MDP satisfying \cref{asmp:reset_cliff}, suppose that $\piail$ is the optimal solution of the above problem and $\vert \gD \vert \geq 2$, with probability at least $1-\delta$, to obtain an $\varepsilon$-optimal policy (i.e., $V^{\piE} - V^{\piail} \leq \varepsilon$), MIMIC-MD requires at most $\min\{ {\widetilde{\gO}}(|\gS|/\varepsilon^2),  {\widetilde{\gO}}(|\gS| \sqrt{H}/\varepsilon)\}$ expert trajectories.
\end{thm}

\begin{proof}[Proof of \cref{theorem:ail_mimic_md} and \cref{theorem:ail_mimic_md_high_prob}]

The proof is mainly based on \cref{prop:ail_general_reset_cliff} and \cref{theorem:ail_reset_cliff}. We apply \cref{prop:ail_general_reset_cliff} with the unbiased estimation in \eqref{eq:new_estimator}. Therefore, with \cref{prop:ail_general_reset_cliff}, we obtain that $\piail$ agrees with the expert policy on good states in the first $H-1$ time steps. Then the policy value gap of $\piail$ only arises from the decision errors in the last time step. Notice that MIMIC-MD and VAIL both perform the state-action distribution. Following the same proof strategy as in \cref{theorem:ail_reset_cliff}, with \eqref{eq:vail_reset_cliff_value_gap_last_step_estimation_error}, we have that
\begin{align*}
    \labs  V^{\piE} - V^{\piail} \rabs \leq 2\sum_{s \in \gS} \labs \widetilde{P}^{\piE}_H (s) - P^{\piE}_H (s)  \rabs = 2\sum_{s \in \gS} \labs \widetilde{P}^{\piE}_H (s, a^{1}) - P^{\piE}_H (s, a^{1})  \rabs.
\end{align*}
Recall that $\Tr_H^{\gD_1} = \lb \tr_H: \tr_H (s_\ell) \in \gS_{\ell} (\gD), \forall \ell \in [H] \rb$ is the set of trajectories along which each state has been visited in $\gD_1$ up to time step $H$. With \eqref{eq:new_estimation_probability_error}, we have
\begin{align*}
    &\quad \labs \widetilde{P}_H^{\pi_E}(s, a^{1}) - P_H^{\piE}(s, a^{1}) \rabs
    \\
    &= \labs \frac{  \sum_{\tr_H \in \gD_1^c}  \indict\{ \tr_H (s_H, a_H) = (s, a^{1}), \tr_H \not\in \Tr_H^{\gD_1}  \} }{|\gD_1^c|} - \sum_{\tr_H \notin \Tr_H^{\gD_1}} \sP^{\piE}(\tr_H) \indict\lb  \tr_H (s_H, a_H) = (s, a^{1})  \rb  \rabs. 
\end{align*}

For a trajectory $\tr_H$, let $E_H^{s}$ be the event that $\tr_H$ agrees with expert policy at state $s$ in the last time step $H$ but is not in $\Tr_H^{\gD_1}$, that is, 
\begin{align*}
    E_H^{s} = \indict\{\tr_H (s_H, a_H) = (s, a^{1}) \, \cap \, \tr_H \notin {\Tr}_H^{\gD_1}\}.
\end{align*}
We consider $E_{H}^{s}$ is measured by the stochastic process induced by the expert policy $\piE$. Accordingly, its probability is denoted as $\sP^{\piE}(E_{H}^{s})$. In fact, we see that $\sP^{\piE}(E^{s}_H)$ is equal to the second term in the RHS of above equation. Moreover, the first term in the RHS of above equation is an empirical estimation for $\sP^{\piE}(E^{s}_H)$. More specifically, let $X (\tr_{H})$ denote the Bernoulli random variable of $\indict\{ \tr_H (s_H, a_H) = (s, a^{1}), \tr_H \not\in \Tr_H^{\gD_1}  \}$. We have that 
\begin{align*}
    \expect_{\gD_1^c} \ls \frac{\sum_{\tr_H \in \gD_1^c} X (\tr_{H}) }{|\gD_1^c|} \rs = \sP^{\piE}(E^{s}_H),
\end{align*}
where the expectation is taken w.r.t the randomness of $\gD_1^c$. We first prove the sample complexity required to obtain a small policy value gap in expectation. We take expectation w.r.t the randomness of $\gD_1^c$ on both sides.
\begin{align*}
    \expect_{\gD_1^c} \ls \labs \widetilde{P}_H^{\pi_E}(s, a^{1}) - P_H^{\piE}(s, a^{1}) \rabs \rs &= \expect_{\gD_1^c} \ls \labs \frac{  \sum_{\tr_H \in \gD_1^c} X (\tr_{H}) }{|\gD_1^c|} - \sP^{\piE}(E_{H}^{s})   \rabs \rs
    \\
    &\leq \sqrt{ \expect_{\gD_1^c} \ls \lp \frac{  \sum_{\tr_H \in \gD_1^c}  X (\tr_{H}) }{|\gD_1^c|} - \sP^{\piE}(E_{H}^{s})   \rp^2 \rs }, 
\end{align*}
where the last inequality follows the Jensen's inequality. Furthermore, we obtain
\begin{align*}
    \expect_{\gD_1^c} \ls \labs \widetilde{P}_H^{\pi_E}(s, a^{1}) - P_H^{\piE}(s, a^{1}) \rabs \rs &\leq \sqrt{ \Var \ls \frac{  \sum_{\tr_H \in \gD_1^c}  X (\tr_{H}) }{|\gD_1^c|}     \rs } = \sqrt{ \frac{\Var \ls X (\tr_{H})      \rs}{|\gD_1^c|}  } \leq \sqrt{ \frac{\sP^{\piE}(E_{H}^{s})}{|\gD_1^c|}  }.    
\end{align*}
The last inequality follows that for $X \sim \text{Ber} (p)$, $\Var \ls X \rs = p (1-p) \leq p$. Then we have that
\begin{align*}
    \expect_{\gD_1^c} \ls \sum_{s \in \gS} \labs \widetilde{P}_H^{\pi_E}(s, a^{1}) - P_H^{\piE}(s, a^{1}) \rabs \rs \leq \sum_{s \in \gS} \sqrt{ \frac{\sP^{\piE}(E_{H}^{s})}{|\gD_1^c|}  } \leq \sqrt{ \frac{\sum_{s \in \gS} \sP^{\piE}(E_{H}^{s}) \vert \gS \vert}{|\gD_1^c|}  }.  
\end{align*}
The last inequality follows the Cauchy-Schwarz inequality. It remains to upper bound $\sum_{s \in \gS}  \sP^{\piE}(E_{H}^{s})$. To this end, we define the event $G_H^{\gD_1}$: the expert policy $\piE$ visits certain states that are uncovered in $\gD_1$ up to time step $H$. Formally, $G_H^{\gD_1} = \indict\{ \exists h^{\prime} \leq H,  s_{h^{\prime}} \notin \gS_{h^{\prime}} (\gD_1) \}$, where $\gS_{h}(\gD_1)$ is the set of states in $\gD_1$ in time step $h$. Then we have 
\begin{align}
\label{eq:probability_equation}
    \sum_{s \in \gS} \sP^{\piE} \lp E_H^{s}  \rp = \sP (G_H^{\gD_1}),
\end{align}
where the equality is true because $\cup_{s} E_H^{s}$ corresponds to the event that $\piE$ does not visit any trajectory fully covered in $\gD_1$. On the one hand, we have that $\expect_{\gD_1} \ls \sP (G_H^{\gD_1}) \rs \leq 1$. On the other hand, it holds that
\begin{align*}
    \expect_{\gD_1} \ls \sP (G_H^{\gD_1}) \rs &\leq \expect_{\gD_1} \ls \sum_{h=1}^{H} \sum_{s \in \gS} P^{\piE}_h(s) \indict\lb s \notin \gS_h(\gD_1)  \rb \rs
    \\
    &= \sum_{h=1}^{H} \sum_{s \in \gS} P^{\piE}_h(s) \sP \lp s \notin \gS_h(\gD_1)  \rp
    \\
    &= \sum_{h=1}^{H} \sum_{s \in \gS} P^{\piE}_h(s) \lp 1 - P^{\piE}_h(s)  \rp^{m/2}
    \\
    &\leq \frac{2 \vert \gS \vert H}{em},
\end{align*}
where the last inequality follows \eqref{eq:expected_missing_mass_upper_bound}. In a word, we have that $\expect_{\gD_1} \ls \sP (G_H^{\gD_1}) \rs \leq \min \{1,  (2 \vert \gS \vert H) / (em) \}$.

Then we have that
\begin{align*}
    V^{\piE} - \expect \ls V^{\piail} \rs &\leq 2 \expect \ls \sum_{s \in \gS} \labs \widetilde{P}_H^{\pi_E}(s, a^{1}) - P_H^{\piE}(s, a^{1}) \rabs \rs
    \\
    &= 2 \expect_{\gD_1} \ls  \sqrt{ \frac{ \sP (G_H^{\gD_1}) \vert \gS \vert}{|\gD_1^c|}  } \rs
    \\
    &\leq 2 \sqrt{ \frac{ \expect_{\gD_1} \ls \sP (G_H^{\gD_1}) \rs \vert \gS \vert}{|\gD_1^c|}  }
    \\
    &\leq \min \lb 2 \sqrt{\frac{2 \vert \gS \vert}{m}}, 4 \sqrt{\frac{\vert \gS \vert H}{e m^2}} \rb.
\end{align*}
which translates into sample complexity of $\min \{ \gO \lp \vert \gS \vert / \varepsilon^2  \rp, \gO ( \vert \gS \vert \sqrt{H} / \varepsilon  )  \}$.

Second, we prove the sample complexity required to achieve a small policy value gap with high probability. Notice that $\sum_{\tr_H \in \gD_1^c} X (\tr_{H}) / |\gD_1^c|$ is an empirical estimation of $\sP^{\piE}(E_{H}^{s})$. By Chernoff's bound in \cref{lemma:chernoff_bound}, with probability at least $1 - \delta/(2|\gS|)$ with $\delta \in (0, 1)$ (over the randomness of the dataset $\gD_1^c$), for each $s \in \gS$,
\begin{align*}
    &\quad \labs \frac{  \sum_{\tr_H \in \gD_1^c}  \indict\{ \tr_H (s_H, a_H) = (s, a^{1}), \tr_H \not\in \Tr_H^{\gD_1}  \} }{|\gD_1^c|} - \sum_{\tr_H \notin \Tr_H^{\gD_1}} \sP^{\piE}(\tr_H) \indict\lb  \tr_H (s_H, a_H) = (s, a^{1})  \rb  \rabs
    \\
    &\leq \sqrt{\sP^{\piE}(E_{H}^{s})  \frac{3 \log (4 |\gS| /\delta)}{m}}.
\end{align*}
By union bound, with probability at least $1-\delta/2$, we have
\begin{align*}
    \labs  V^{\piE} - V^{\piail} \rabs &\leq 2\sum_{s \in \gS} \labs \widetilde{P}^{\piE}_H (s, a^{1}) - P^{\piE}_H (s, a^{1})  \rabs
    \\
    &\leq  2\sum_{s \in \gS} \sqrt{\sP^{\piE}(E_{H}^{s})  \frac{3 \log (4 |\gS| /\delta)}{m}}
    \\
    &\leq 2 \sqrt{ \lp \sum_{s \in \gS} \sP^{\piE}(E_{H}^{s}) \rp  \frac{3 |\gS| \log (4 |\gS| /\delta)}{m}},
\end{align*}
where the last inequality follows the Cauchy–Schwarz inequality. With \eqref{eq:probability_equation}, with probability at least $1-\delta/2$ (over the randomness of $\gD_1^c$), we have
\begin{align*}
    \labs  V^{\piE} - V^{\piail} \rabs \leq 2 \sqrt{ \sP (G_H^{\gD_1})  \frac{3 |\gS| \log (4 |\gS| /\delta)}{m}} .
\end{align*}
On the one hand, with probability of 1, $\sP (G_H^{\gD_1}) \leq 1$. On the other hand, notice that
\begin{align*}
    \sP (G_H^{\gD_1}) \leq \sum_{h=1}^{H} \sum_{s \in \gS} P^{\piE}_h(s) \indict\lb s \notin \gS_h(\gD_1)  \rb.
\end{align*}
Furthermore, by \cref{lemma:missing_mass_one_step}, with probability at least $1-\delta/2$,
\begin{align*}
    \sum_{h=1}^{H} \sum_{s \in \gS} P^{\piE}_h(s) \indict\lb s \notin \gS_h(\gD_1)  \rb \leq \frac{8|\gS| H}{9m} + \frac{6 \sqrt{|\gS|} H \log(2H/\delta)}{m}.
\end{align*}
In a word, with probability at least $1-\delta/2$ (over the randomness of $\gD_1$), it holds that
\begin{align*}
    \sP (G_H^{\gD_1}) \leq \min \lb 1,  \frac{8|\gS| H}{9m} + \frac{6 \sqrt{|\gS|} H \log(2H/\delta)}{m} \rb.
\end{align*}
By union bound, with probability at least $1-\delta$, we have 
\begin{align*}
    \labs  V^{\piE} - V^{\piail} \rabs &\leq 2\sqrt{ \min \lb 1, \frac{8|\gS| H}{9m} + \frac{6 \sqrt{|\gS|} H \log(2H/\delta)}{m}  \rb \frac{3 |\gS| \log (4 |\gS| H/\delta)}{m}}
    \\
    &\leq 2\min \lb \sqrt{\frac{3 |\gS| \log (4 |\gS| H/\delta)}{m}}, \frac{ |\gS| \sqrt{H}}{m} \log^{1/2}\lp \frac{4|\gS| H}{\delta}  \rp \sqrt{ \frac{8}{3} + 18 \log (2H/\delta)  } \rb,
\end{align*}
which translates to sample complexity of $\min \{ \widetilde{\gO} \lp \vert \gS \vert / \varepsilon^2  \rp, \widetilde{\gO} ( \vert \gS \vert \sqrt{H} / \varepsilon  )  \}$.
\end{proof}

\subsection{Application of FEM with Proposition \ref{prop:connection}}
\label{appendix:discussion_of_prop:connection}

Note the metric (e.g., $\ell_1$-norm) used in the estimation problem (assumption $(b)$) and the optimization problem (assumption $(c)$) is not unique in \cref{prop:connection}. For instance, FEM \citep{pieter04apprentice} uses the $\ell_2$-norm metric in its algorithm but FEM can be also applied under this framework. As a result, the policy value gap becomes $\gO ( \sqrt{\vert \gS \vert \vert \gA \vert} ( \varepsilon_{\text{EST}} + \varepsilon_{\text{RFE}} + H \varepsilon_{\text{AIL}} ) )$.

\begin{claim}
If we apply FEM \citep{pieter04apprentice} and RF-Express \citep{menard20fast-active-learning} in \cref{algo:framework}, the corresponding policy value gap in \cref{prop:connection} is $\gO ( \sqrt{\vert \gS \vert \vert \gA \vert} ( \varepsilon_{\text{EST}} + \varepsilon_{\text{RFE}} + H \varepsilon_{\text{AIL}} ) )$.
\end{claim}

\begin{proof}
To apply FEM under our framework in Algorithm \ref{algo:framework}, the assumption $(b)$ becomes: with probability at least $1-\delta_{\text{EST}}$, 
\begin{align*}
    \sum_{h=1}^H \lnorm \widetilde{P}^{\piE}_h - P^{\piE}_h \rnorm_2 \leq \varepsilon_{\text{EST}}.
\end{align*}
Besides, the assumption $(c)$ becomes: with estimation $\widetilde{P}_h^{\piE} (s, a)$ and transition model $\widehat{\gP}$, the policy $\widebar{\pi}$ output by FEM satisfies
\begin{align*}
    \frac{1}{H} \sum_{h=1}^H \lnorm \widetilde{P}^{\piE}_h - P^{\widebar{\pi}, \widehat{\gP}}_h   \rnorm_2 \leq \min_{\pi \in \Pi} \frac{1}{H} \sum_{h=1}^H \lnorm \widetilde{P}^{\piE}_h - P^{\pi, \widehat{\gP}}_h   \rnorm_2 + \varepsilon_{\mathrm{AIL}}.
\end{align*}
Following the same idea in the proof of Proposition \ref{prop:connection}, we can get that
\begin{align*}
    \left\vert V^{\piE, \gP} - V^{\widebar{\pi}, \gP} \right\vert &\leq \left\vert V^{\piE, \gP} - V^{\widebar{\pi}, \widehat{\gP}} \right\vert + \varepsilon_{\text{RFE}} 
    \\
    &\leq \sum_{h=1}^H \lnorm P^{\piE, \gP}_h  - P^{\widebar{\pi}, \widehat{\gP}}_h  \rnorm_1 + \varepsilon_{\text{RFE}}
    \\
    &\leq \sum_{h=1}^H \lnorm P^{\piE, \gP}_h  - \widetilde{P}^{\piE}_h  \rnorm_1 + \sum_{h=1}^H \lnorm \widetilde{P}^{\piE}_h  - P^{\widebar{\pi}, \widehat{\gP}}_h  \rnorm_1 + \varepsilon_{\text{RFE}}.
\end{align*}
For an arbitrary vector $x \in \reals^n$, we have that $\lnorm x \rnorm_2 \leq \lnorm x \rnorm_1 \leq \sqrt{n} \lnorm x \rnorm_2$. Then we show that
\begin{align*}
    \lnorm P^{\piE, \gP}_h  - \widetilde{P}^{\piE}_h  \rnorm_1 \leq \sqrt{\vert \gS \vert \vert \gA \vert} \lnorm P^{\piE, \gP}_h  - \widetilde{P}^{\piE}_h  \rnorm_2 \leq \sqrt{\vert \gS \vert \vert \gA \vert} \varepsilon_{\text{EST}}.
\end{align*}
Then we continue to consider the policy value gap.
\begin{align*}
    \left\vert V^{\piE, \gP} - V^{\widebar{\pi}, \gP} \right\vert &\leq \sum_{h=1}^H \lnorm \widetilde{P}^{\piE}_h  - P^{\widebar{\pi}, \widehat{\gP}}_h  \rnorm_1 + \sqrt{\vert \gS \vert \vert \gA \vert} \varepsilon_{\text{EST}} + \varepsilon_{\text{RFE}}
    \\
    &\leq \sqrt{\vert \gS \vert \vert \gA \vert} \sum_{h=1}^H \lnorm \widetilde{P}^{\piE}_h  - P^{\widebar{\pi}, \widehat{\gP}}_h  \rnorm_2 + \sqrt{\vert \gS \vert \vert \gA \vert} \varepsilon_{\text{EST}} + \varepsilon_{\text{RFE}}
    \\
    &\leq \sqrt{\vert \gS \vert \vert \gA \vert} \lp \min_{\pi \in \Pi} \sum_{h=1}^H \lnorm \widetilde{P}^{\piE}_h  - P^{\pi, \widehat{\gP}}_h  \rnorm_2 + H \varepsilon_{\text{AIL}} \rp + \sqrt{\vert \gS \vert \vert \gA \vert} \varepsilon_{\text{EST}} + \varepsilon_{\text{RFE}}.
\end{align*}
The last inequality holds since that FEM performs $\ell_2$-norm projection with $\widetilde{P}^{\piE}_h (s, a)$ and $\widehat{\gP}$ up to an error of $\varepsilon_{\text{AIL}}$. Then we have that
\begin{align*}
    &\quad \left\vert V^{\piE, \gP} - V^{\widebar{\pi}, \gP} \right\vert \\
    &\leq \sqrt{\vert \gS \vert \vert \gA \vert} \sum_{h=1}^H \lnorm \widetilde{P}^{\piE}_h  - P^{\piE, \widehat{\gP}}_h  \rnorm_2 + \sqrt{\vert \gS \vert \vert \gA \vert} \lp H \varepsilon_{\text{AIL}} +  \varepsilon_{\text{EST}} \rp + \varepsilon_{\text{RFE}}
    \\
    &\leq \sqrt{\vert \gS \vert \vert \gA \vert} \lp \sum_{h=1}^H \lnorm \widetilde{P}^{\piE}_h  - P^{\piE, \gP}_h  \rnorm_2 + \sum_{h=1}^H \lnorm P^{\piE, \gP}_h  - P^{\piE, \widehat{\gP}}_h  \rnorm_2  \rp + \sqrt{\vert \gS \vert \vert \gA \vert} \lp H \varepsilon_{\text{AIL}} +  \varepsilon_{\text{EST}} \rp + \varepsilon_{\text{RFE}}
    \\
    &\leq \sqrt{\vert \gS \vert \vert \gA \vert} \lp \varepsilon_{\mathrm{EST}} + \sum_{h=1}^H \lnorm P^{\piE, \gP}_h  - P^{\piE, \widehat{\gP}}_h  \rnorm_2  \rp + \sqrt{\vert \gS \vert \vert \gA \vert} \lp H \varepsilon_{\text{AIL}} +  \varepsilon_{\text{EST}} \rp + \varepsilon_{\text{RFE}}
    \\
    &\leq \sqrt{\vert \gS \vert \vert \gA \vert} \sum_{h=1}^H \lnorm P^{\piE, \gP}_h  - P^{\piE, \widehat{\gP}}_h  \rnorm_1 + \sqrt{\vert \gS \vert \vert \gA \vert} \lp H \varepsilon_{\text{AIL}} +  2 \varepsilon_{\text{EST}} \rp + \varepsilon_{\text{RFE}}
    \\
    &\leq \sqrt{\vert \gS \vert \vert \gA \vert} \lp H \varepsilon_{\text{AIL}} +  2 \varepsilon_{\text{EST}} + \varepsilon_{\text{RFE}} \rp + \varepsilon_{\text{RFE}}.
\end{align*}
In the last inequality, we use the dual representation of $\ell_1$-norm and policy value. Furthermore, $\widehat{\gP}$ satisfies that for any policy $\pi \in \Pi$ and reward $r \in \gS \times \gA \rar [0, 1]$, $\vert V^{\pi, \gP, r} - V^{\pi, \widehat{\gP}, r} \vert \leq \varepsilon_{\text{RFE}}$. 

\end{proof}

\begin{rem}
Note that the additional factor $\sqrt{|\gS||\gA|}$ is partially caused by the $\ell_2$-norm. In particular, the original assumption in FEM \citep{pieter04apprentice} is that there exists some $w_h$ such that $r_h(s, a) = w_h^{\top} \phi_h(s, a)$. When $\phi_h(s, a)$ is the one-hot feature used in the tabular MDP in this paper, $w_h(s, a) = r_h(s, a)$. According to our assumption that $r_h(s, a) \in [0, 1]$, such an $w_h$ satisfies $\Vert w_h \Vert_2 \leq \sqrt{|\gS| |\gA|}$, which is different from the assumption $\Vert w_h \Vert_2 \leq 1$ in \citep{pieter04apprentice}. However, this mismatch may not be a big issue since the concentration rate for $\ell_2$-norm metric is faster than $\ell_1$-norm when the estimation error is small.
\end{rem}

\subsection{From Regret Guarantee to Sample Complexity Guarantee}
\label{appendix:from_regret_to_pac}

\citet{shani21online-al} proved a regret guarantee for their OAL algorithm. In particular, \citet{shani21online-al} showed that with probability at least $1 - \delta^\prime$, we have 
\begin{align}   \label{eq:oal_regret}
     \sum_{k=1}^{K}  V^{\piE} - V^{\pi_k}  \leq  \widetilde{\gO}\lp \sqrt{H^4 |\gS|^2 |\gA|K} + \sqrt{H^3 |\gS| |\gA| K^2 /m} \rp,
\end{align}
where $\pi^{k}$ is the policy obtained at episode $k$, $K$ is the number of interaction episodes, and $m$ is the number of expert trajectories. We would like to comment that the second term in \eqref{eq:oal_regret} involves the statistical estimation error about the expert policy. Furthermore, this term reduces to $\widetilde{\gO}(\sqrt{H^2 |\gS| K^2 /m})$ under the assumption that the expert policy is deterministic.

To further convert this regret guarantee to the sample complexity guarantee considered in this paper, we can apply Markov's inequality as suggested by \citep{jin18qlearning}. Concretely, let $\widebar{\pi}$ be the policy that randomly chosen from $\{\pi^{1}, \pi^{2}, \cdots, \pi^{K}\}$ with equal probability, then we have 
\begin{align*}
    \sP \lp V^{\piE} - V^{\widebar{\pi}} \geq \varepsilon \rp \leq \frac{1}{\varepsilon} \expect \ls \frac{1}{K} \sum_{k=1}^{K}  V^{\piE} - V^{\pi_k} \rs \leq \frac{1}{\varepsilon} \lp \widetilde{\gO} \lp \sqrt{ \frac{H^4 |\gS|^2 |\gA|}{K} } + \sqrt{H^2 |\gS| /m}\rp + \delta^\prime H  \rp,
\end{align*}
Therefore, if we set $\delta^{\prime} = \varepsilon \delta / (3H)$, and
\begin{align*}
    K = \widetilde{\gO} \lp \frac{H^4 |\gS|^2 |\gA|}{\varepsilon^2 \delta^2} \rp, \quad m = \widetilde{\gO} \lp \frac{H^2 |\gS|}{\varepsilon^2} \rp,
\end{align*}
we obtain that $\sP ( V^{\piE} - V^{\widebar{\pi}} \geq \varepsilon ) \leq \delta $. As commented in \citep{menard20fast-active-learning}, this transformation leads to a worse dependence on failure probability $\delta$, but the sample complexity dependence on other terms does not change.

\subsection{VAIL with State Abstraction}
\label{appendix:discussion_of_function_approximation}

Notice that the upper bounds of sample complexity discussed in this paper depend on the state space size $\vert \gS \vert$. Besides, the lower bounds \citep[Theorem 6.1, 6.2]{rajaraman2020fundamental} imply that the dependence of $\vert \gS \vert$ is inevitable for all imitation learning algorithms if no additional information is provided. In this part, we discuss that if provided with a set of state abstractions \citep{li2006towards}, how to avoid the dependence of $\vert \gS \vert$ on sample complexity. In particular, state abstractions correspond to the function approximation with a series of piecewise constant functions \citep{chen2019information}.

To be more specific, assume we have access to a set of state abstractions $\{ \phi_h \}_{h=1}^H$, where $\phi_h: \gS \rightarrow \Phi$ for each $h \in [H]$ and $\Phi$ is abstract state space. The size of abstract state space is much smaller than that of original state space, i.e., $|\Phi| \ll |\gS|$. We assume that the state abstractions satisfy the following reward-irrelevant condition \citep{li2006towards}.

\begin{asmp}[Reward-irrelevant]
\label{asmp:reward_irrelevant}
Consider the set of state abstractions $\{ \phi_h \}_{h=1}^H$. For each $h \in [H]$, for any $s^{1}, s^{2} \in \gS$ such that $\phi_h (s^{1}) = \phi_h (s^{2})$, $\forall a \in \gA$, $r_h (s^{1}, a) = r_h (s^{2}, a)$. 
\end{asmp}

We highlight that the reward-irrelevant condition is important for AIL to avoid the dependence on $\vert \gS \vert$; see also \citep{pieter04apprentice, syed07game, liu2021provably}. In particular, the bottleneck of the sample complexity of AIL methods is the estimation of $P^{\piE}_h(s, a)$.  With the set of state abstractions, we can calculate the expert policy value as
\begin{align*}
    V^{\piE} = \sum_{h=1}^H \sum_{(s, a) \in \gS \times \gA} r_h (s, a)  P^{\piE}_h (s, a) = \sum_{h=1}^H \sum_{(x, a) \in \Phi \times \gA} r^{\phi}_h (x, a) P^{\piE, \phi}_h (x, a), 
\end{align*}
where $P^{\pi, \phi}_h$ is the \dquote{abstract state-action distribution}: $P^{\pi, \phi}_h (x, a) = \sP^{\piE} (\phi_h (s_h) = x, a_h = a) = \sum_{s \in \phi_h^{-1} (x)} P^{\pi}_h (s, a)$. With the above formulation, to estimate the expert policy value, we can estimate the \emph{abstract} state-action distribution rather than the original state-action distribution. This may remove the dependence on $\vert \gS \vert$. We present our conjecture as follows.

\begin{conj}[Sample Complexity of \textsf{VAIL} with State Abstraction]
\label{theorem:worst_case_sample_complexity_of_vail_state_abstraction}
For any tabular and episodic MDP, suppose that there exists a set of known state abstractions $\{ \phi_h: \gS \rightarrow \Phi \}_{h=1}^H$ satisfying \cref{asmp:reward_irrelevant}. To obtain an $\varepsilon$-optimal policy (i.e., $V^{\piE} - \expect[ V^{\piail}] \leq \varepsilon$), in expectation,  \textsf{VAIL} requires at most $\gO(|\Phi |H^2/\varepsilon^2)$ expert trajectories. 
\end{conj}
