# Supplementary material for: A Note on Target Q-learning For Solving Finite MDPs with A Generative Oracle
Source: arXiv:2203.11489 source file (2022-03-22)
Supplement: Supplementary file 2 [file experiment.tex]

\section{Experiments}
\label{appendix:experiments}

In this section, we present experiment results to help verify and understand our theoretical claims.

\subsection{Baselines}

We consider the following baselines on two MDPs: \emph{Standard Imitation} and \emph{Reset Cliff} introduced in \cref{sec:generalization_of_ail}. 
\begin{itemize}
    \item Behavioral Cloning (BC) \citep{Pomerleau91bc}. 
    \item Feature Expectation Matching (FEM) \citep{pieter04apprentice}.
    \item Game-theoretic Apprenticeship Learning (GTAL) \citep{syed07game}. 
    \item Vanilla Adversarial Imitation Learning (VAIL) (refer to \eqref{eq:ail}).
    \item Transition-aware Adversarial Imitation Learning (TAIL) (refer to \cref{algo:main_aglorithm}) .
    \item Model-based Transition-aware Adversarial Imitation Learning (MB-TAIL) (refer to \cref{algo:mbtail-abstract}).
    \item Online apprenticeship learning (OAL) \citep{shani21online-al}. 
\end{itemize}

Algorithm configurations are given in \cref{subsection:experiment_details}. We do not involve MIMIC-MD \citep{rajaraman2020fundamental} because its LP formulation in \citep{nived2021provably}  runs out of memory on a machine with $128$GB RAM when $H \geq 100$.  GAIL is not considered as it does not have a formal convergent algorithm. Furthermore, GAIL differs from \textsf{VAIL} in terms of the discrepancy metric, which does not matter under tabular MDPs. For completeness, we provide a variant of GAIL \citep{ho2016gail} and investigate its performance in Appendix \ref{subsection:additional_results_gail}.

\subsection{Known Transition Setting}
\label{appendix:experiment_known_transition}

We aim to study the dependence on $H$ and $\varepsilon$ appeared in the sample complexity. To achieve this goal, figures have used \emph{logarithmic} scales so that we can read the order dependence from slopes of curves. Specifically, a worst-case sample complexity $m \succsim |\gS| H^{\alpha}/\varepsilon^{\beta}$ implies the policy value gap $ V^{\piE} - V^{\pi} \precsim |\gS|^{1/\beta} H^{\alpha/\beta} /m^{1 / \beta}$. Then,
\begin{align*}
\log(V^{\piE} - V^{\pi}) \precsim & (\alpha/\beta) \log (H) - 1/\beta \log (m) +1/\beta \log (|\gS|).
\end{align*}
For example, the sample complexity ${\gO}(|\gS| H^2/\varepsilon)$ of \textsf{VAIL} similarly suggests slope $1$ w.r.t. $\log(H)$ and slope $-1/2$ w.r.t. $\log(m)$ for its $\log$ policy value gap. It is worth mentioning that these implications are true only on the worst instances.

\begin{figure}[htbp]
     \centering
     \begin{subfigure}[b]{0.45\textwidth}
         \centering
         \includegraphics[width=\textwidth]{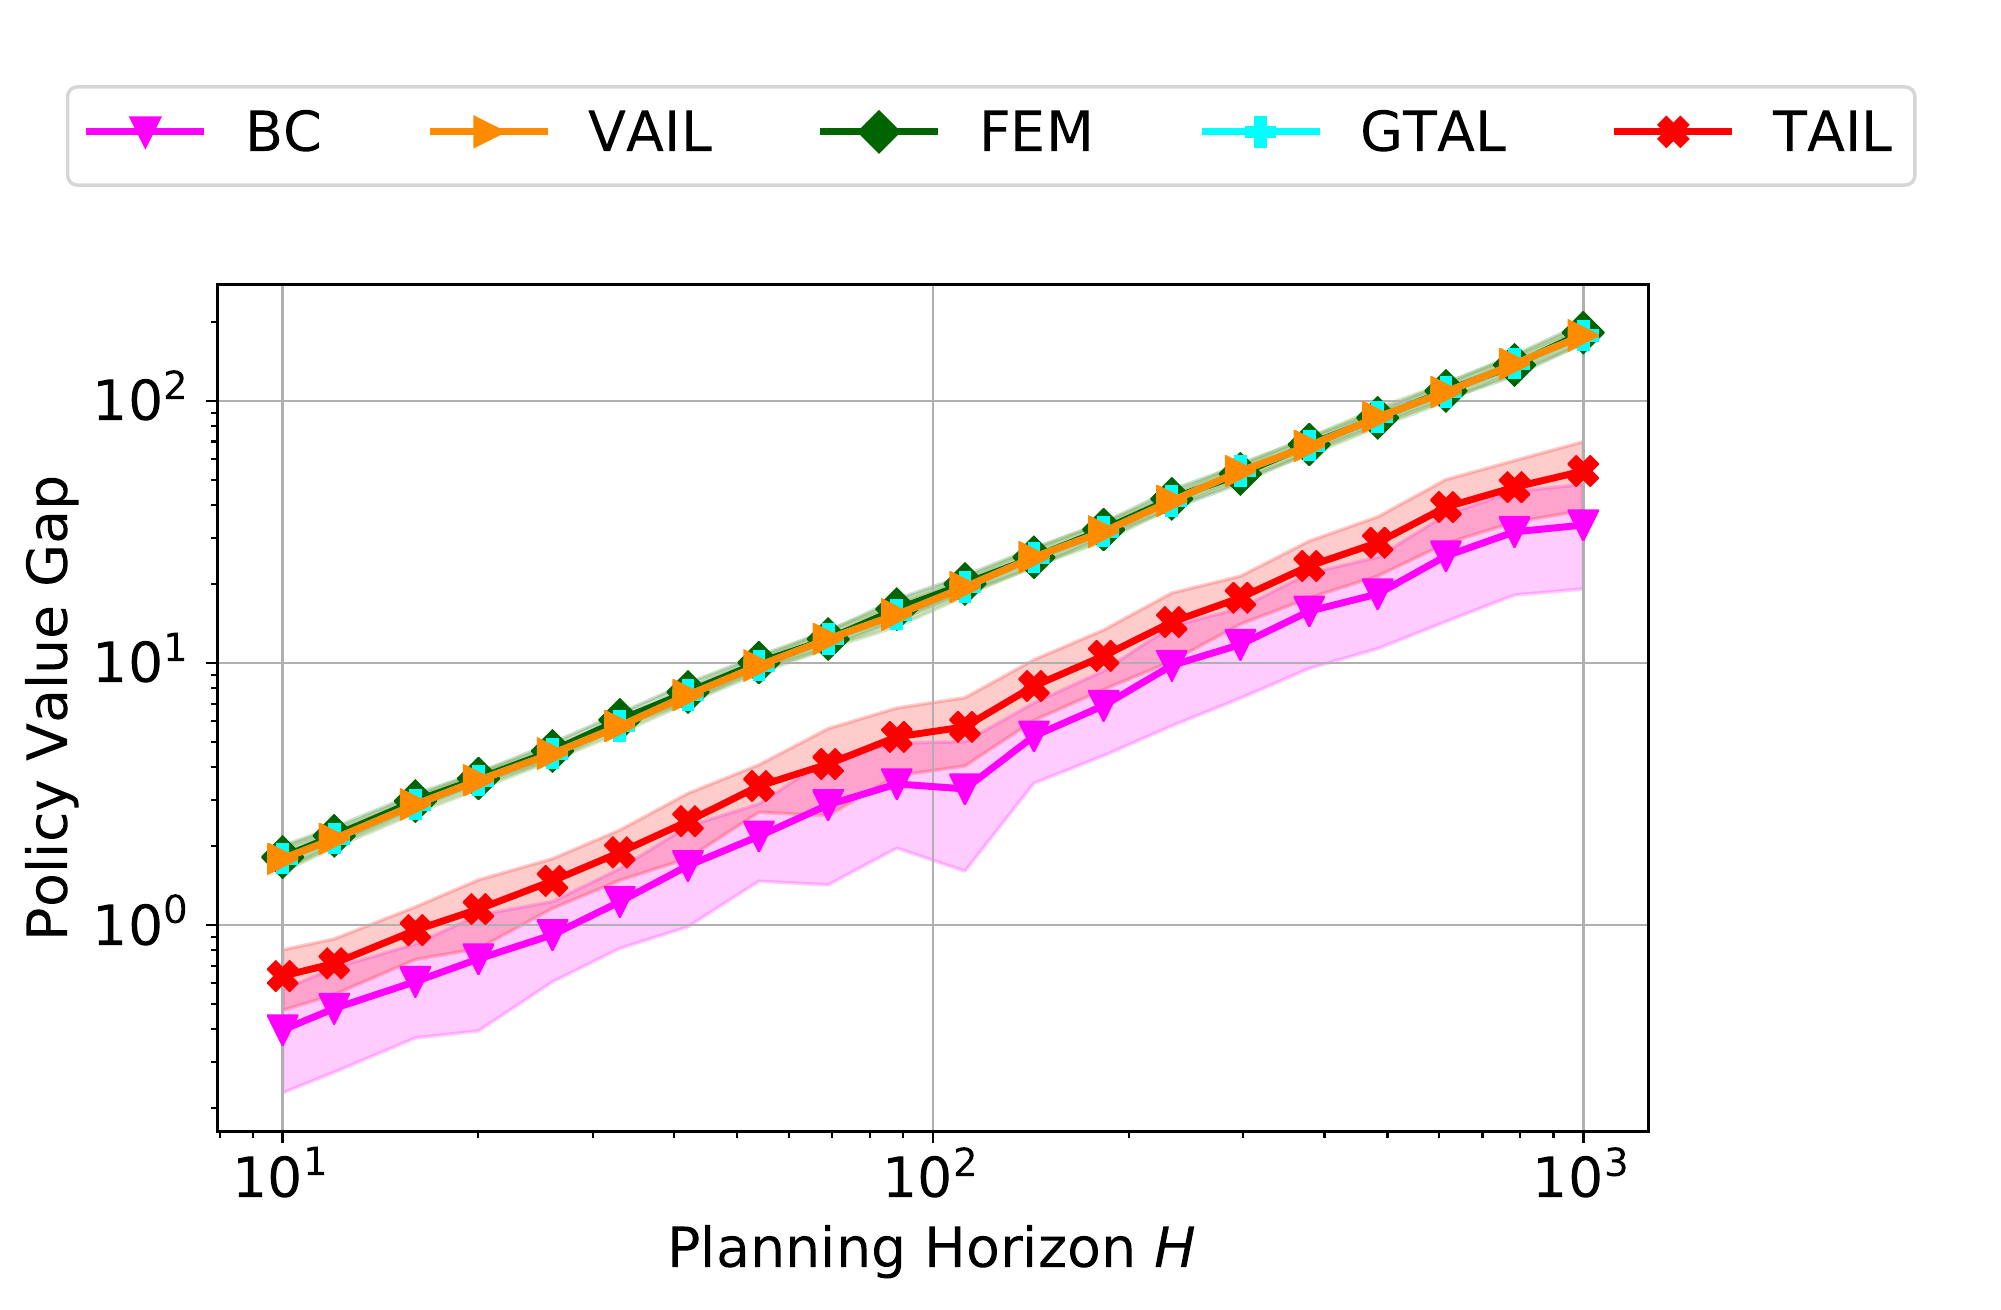}
         \caption{On the planning horizon on Standard Imitation.}
         \label{fig:bandit_h_log_result}
     \end{subfigure}
     \hfill
     \begin{subfigure}[b]{0.45\textwidth}
         \centering
         \includegraphics[width=\textwidth]{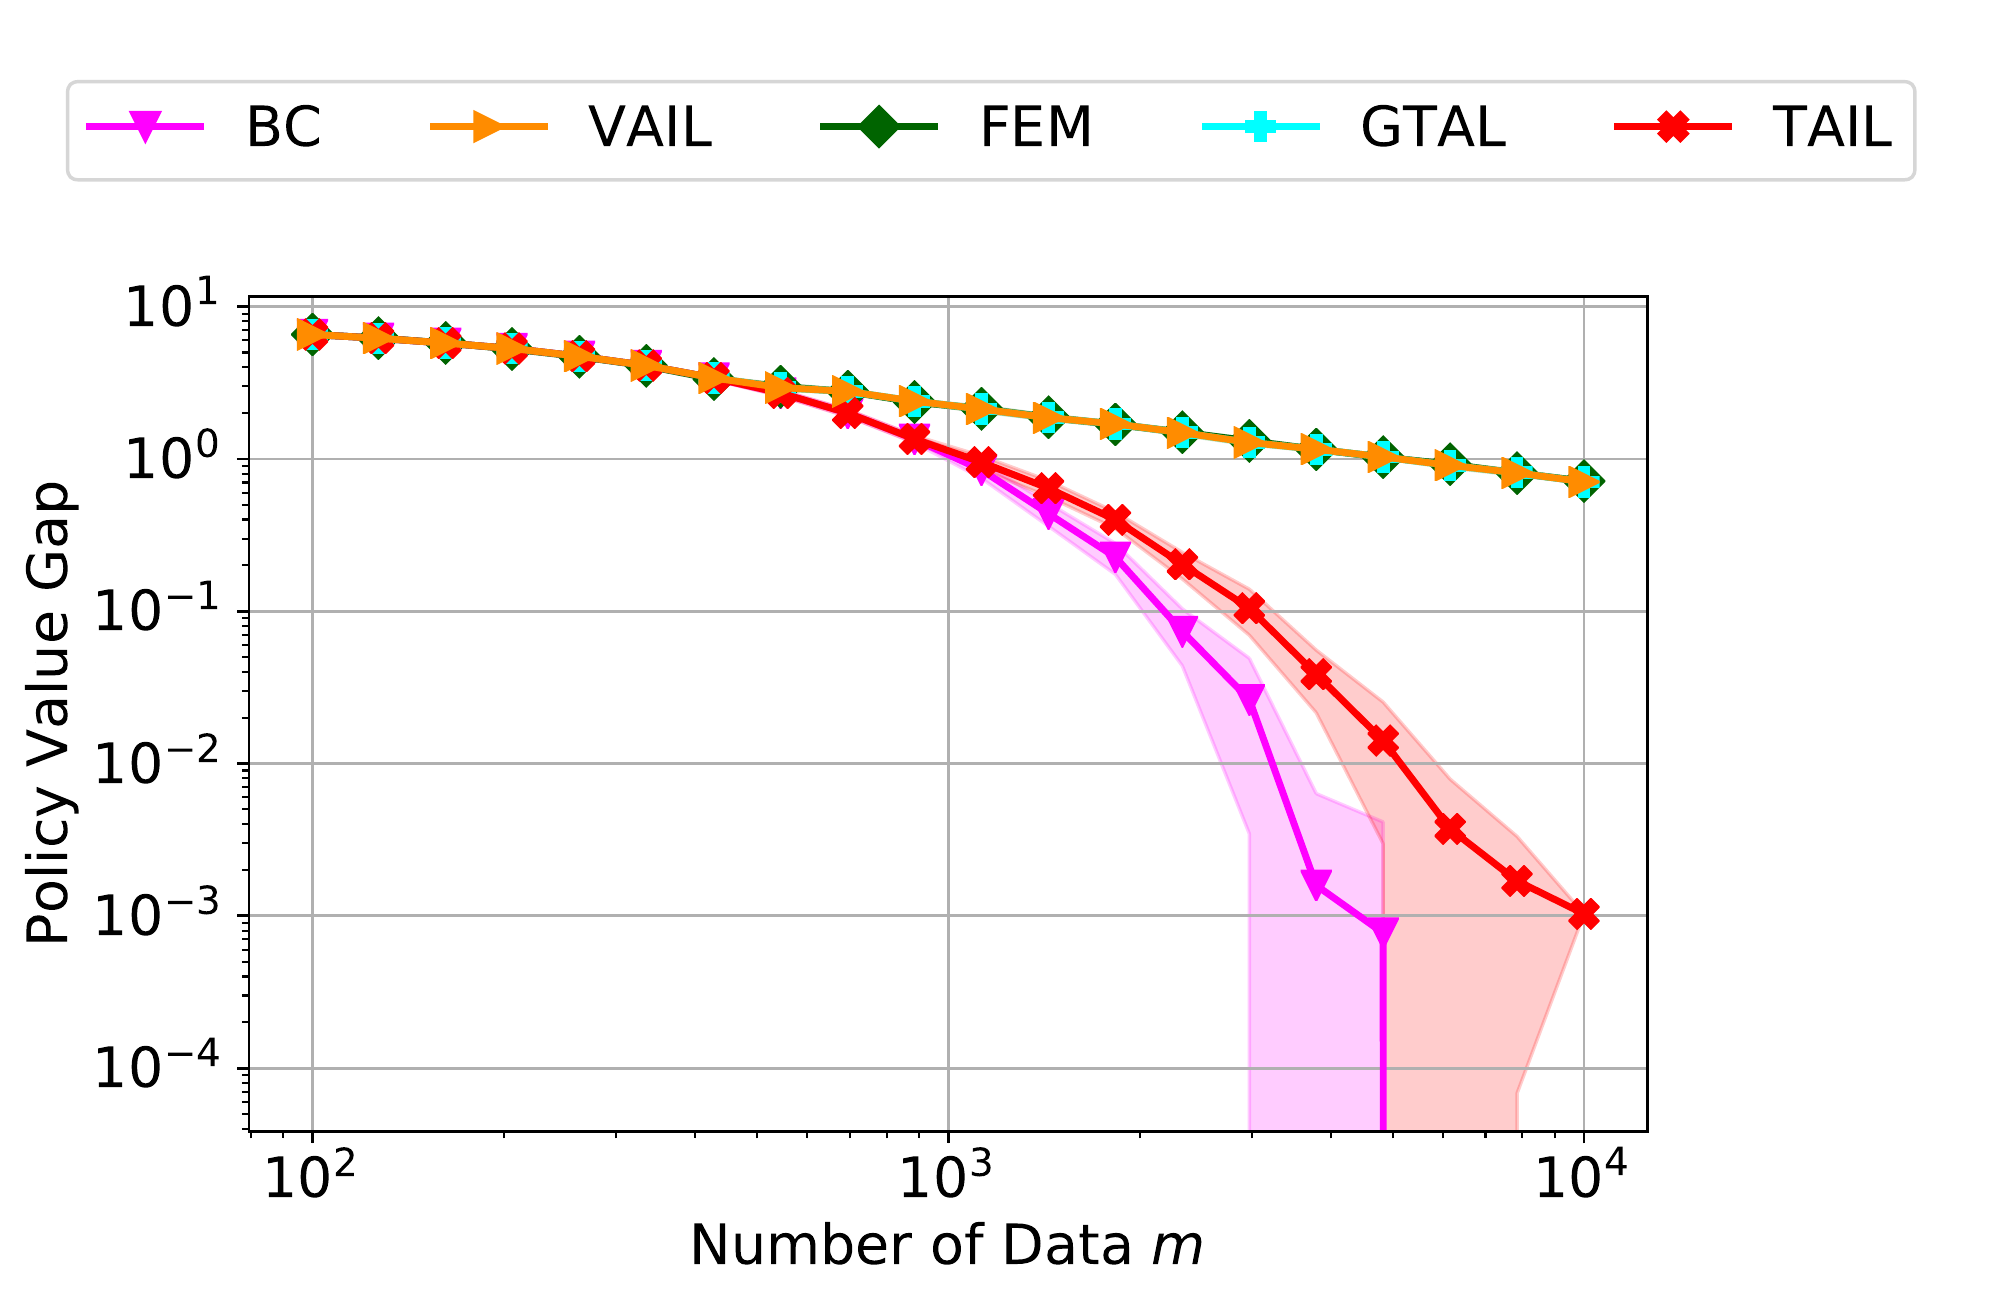}
         \caption{On the expert sample size on Standard Imitation.}
         \label{fig:bandit_m_log_result}
     \end{subfigure}
     \hfill
     \vskip\baselineskip
     \begin{subfigure}[b]{0.45\textwidth}
         \centering
         \includegraphics[width=\textwidth]{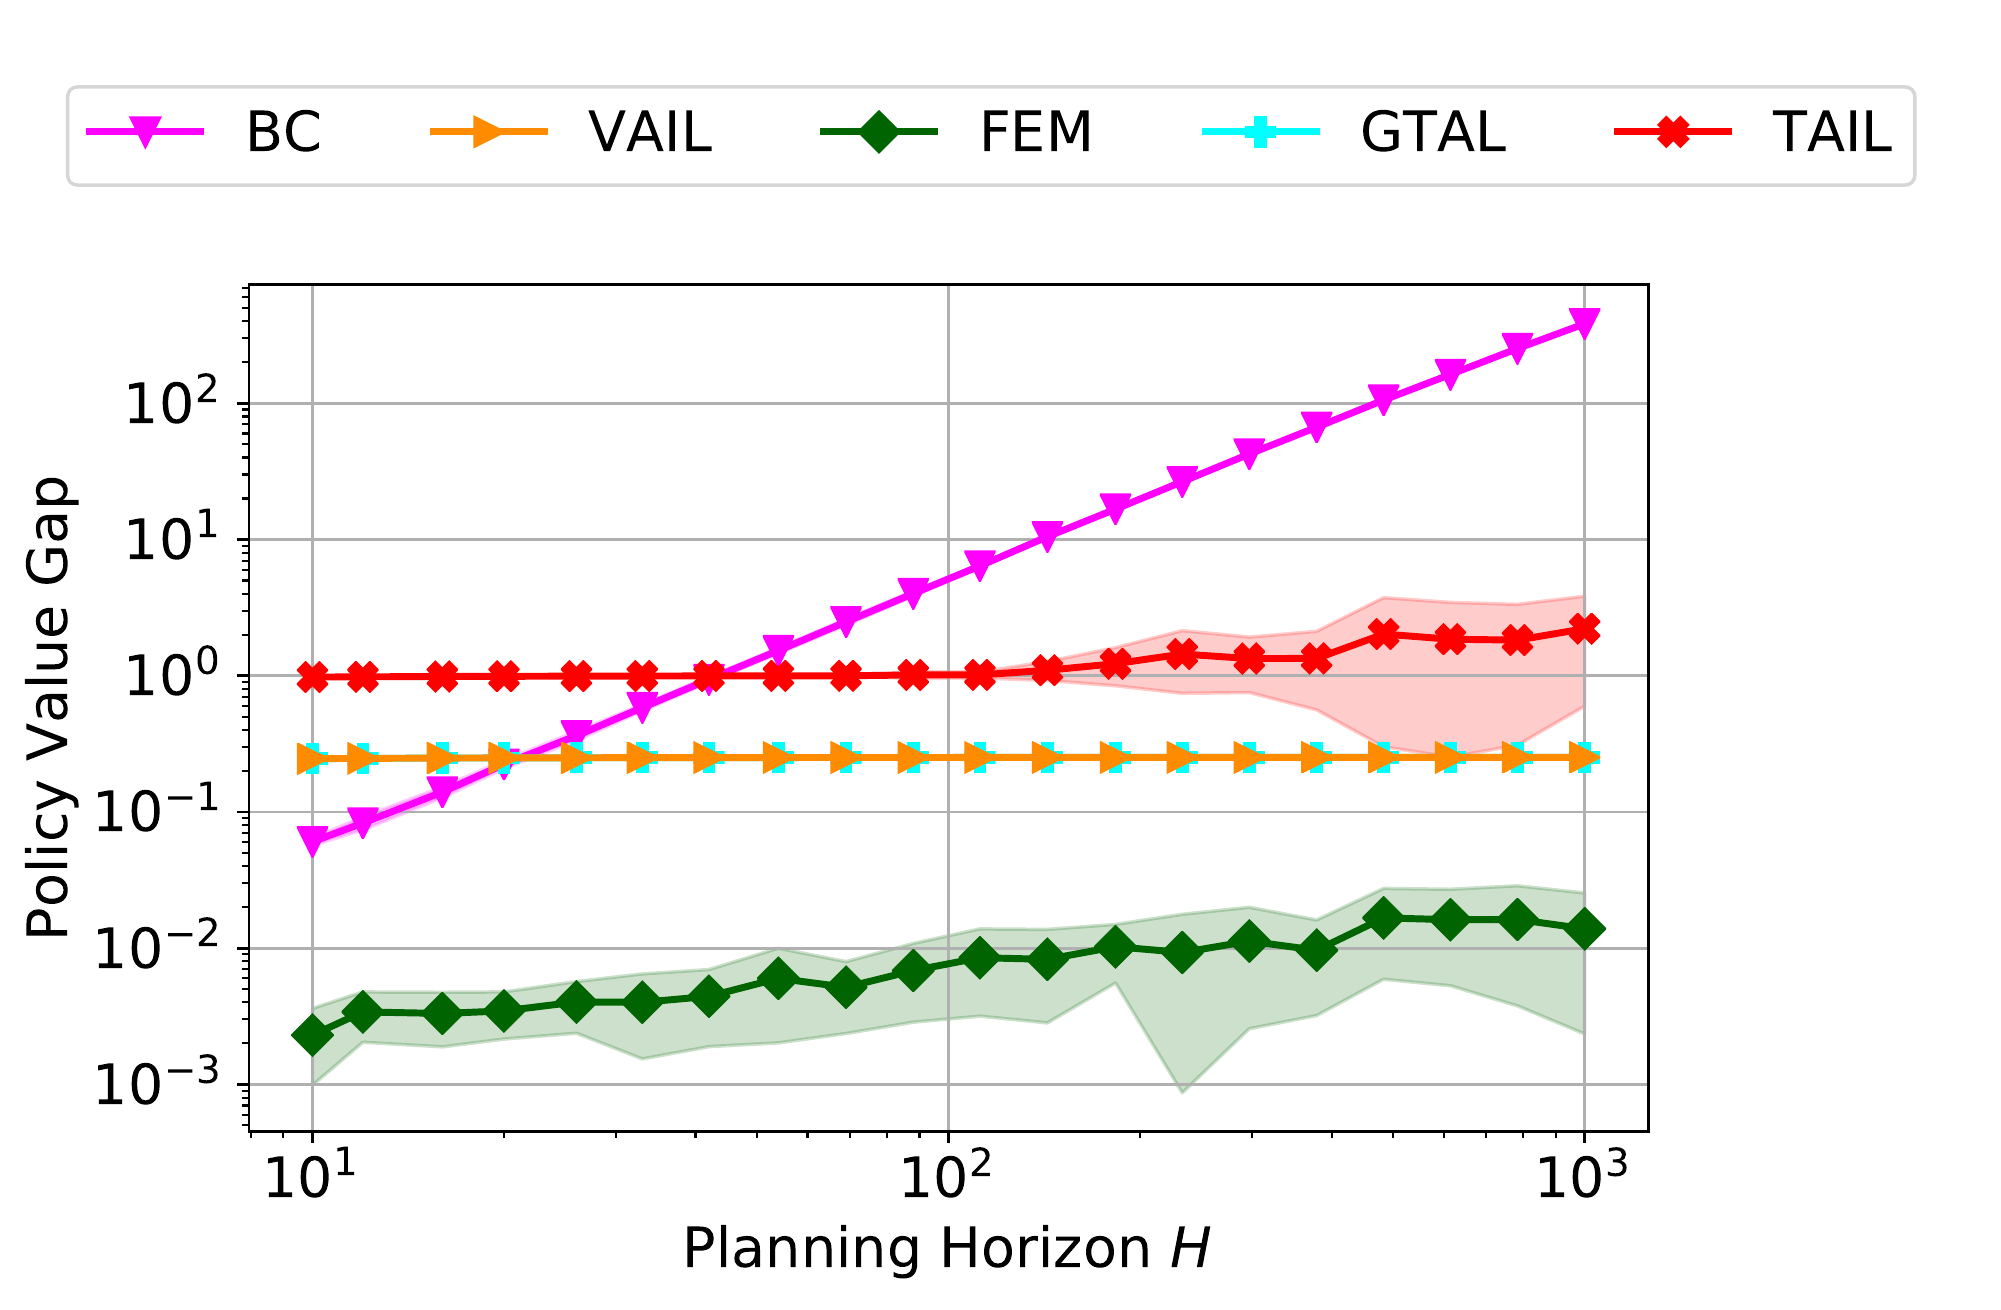}
         \caption{On the planning horizon on Reset Cliff.}
         \label{fig:cliffwalking_h_log_result}
     \end{subfigure}
     \hfill
    \begin{subfigure}[b]{0.45\textwidth}
      \centering
      \includegraphics[width=\textwidth]{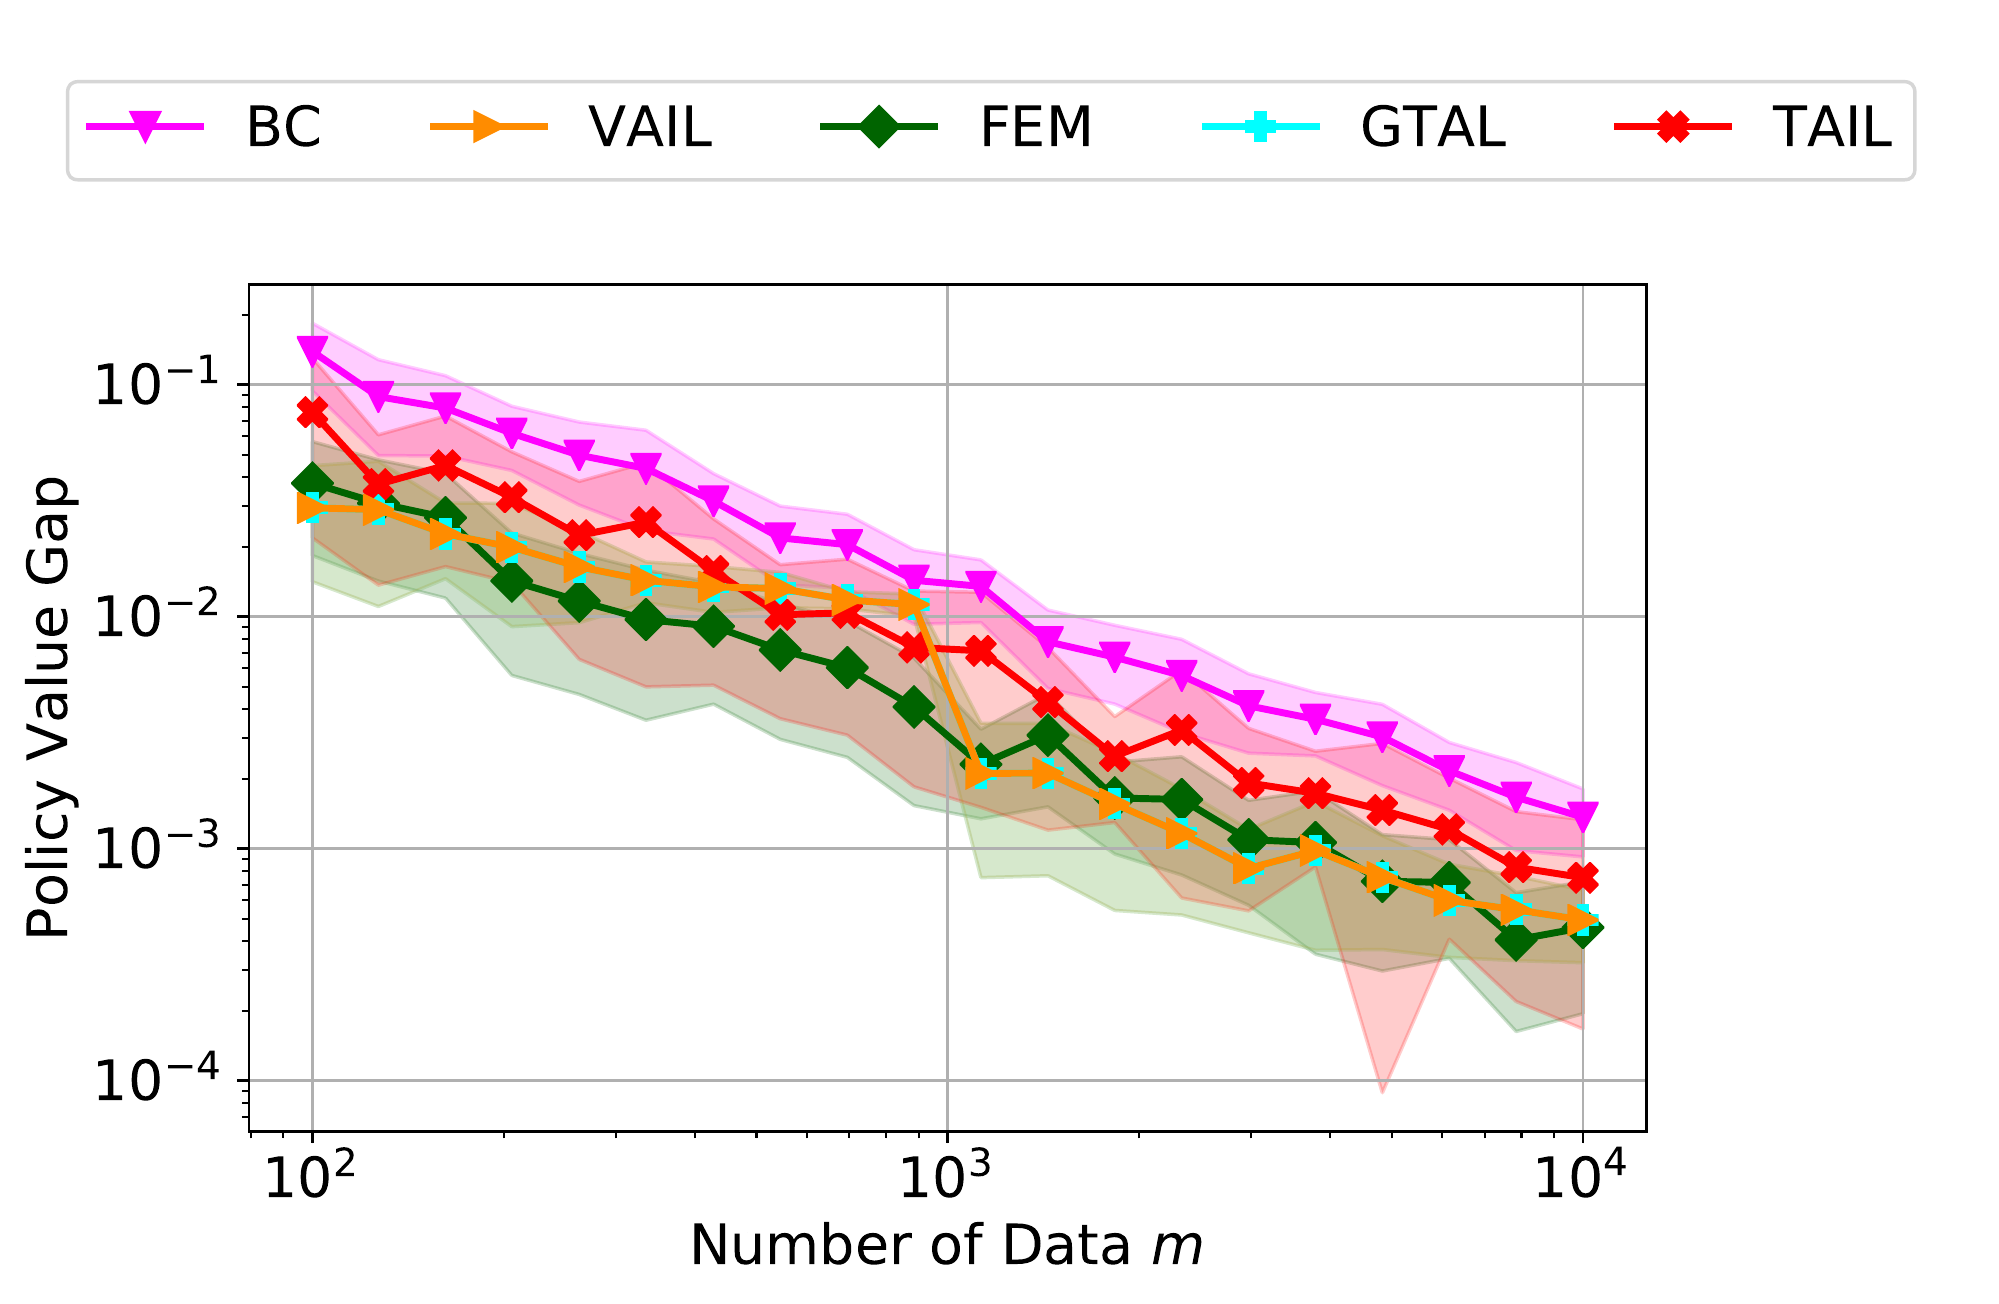}
      \caption{On the expert sample size on Reset Cliff.}
      \label{fig:cliffwalking_m_log_result}
    \end{subfigure}

     \caption{The policy value gap (i.e., $V^{\piE} - V^{\pi}$) on Standard Imitation and Reset Cliff. The solid lines are mean of results and the shaded region corresponds to the standard deviation over $20$ random seeds (same with the following figure). \dquote{sample size} refers to the number of expert trajectories. }
     \label{figure:main_results}
\end{figure}

\textbf{Case Study on Standard Imitation.} For Standard Imitation (Figure \ref{fig:bandit}), each state is absorbing and the agent gets $+1$ reward only by taking the expert action (shown in green). Different from \citep{rajaraman2020fundamental}, the initial state distribution $\rho$ is $({1}/{|\gS|}, \cdots, {1}/{|\gS|})$ to better disclose the sample barrier issue of AIL methods discussed in Section \ref{sec:generalization_of_ail}.

First, we focus on the planning horizon dependence issue; see the result in Figure~\ref{fig:bandit_h_log_result}. In particular, the numerical result shows that the policy value gap of all methods grows linearly with respect to the planning horizon. This is reasonable since each state on Standard Imitation is absorbing. As suggested in \cref{theorem:bc_deterministic}, Standard Imitation is not the worst-case MDP for BC due to its absorbing structure. However, Standard Imitation is challenging for conventional AIL approaches (VAIL, FEM, and GTAL) and thus can be used to validate the tightness of their sample complexity.

Second, we display the result regarding the number of expert demonstrations in Figure~\ref{fig:bandit_m_log_result}. Under Standard Imitation, the state distribution of every policy is a uniform distribution at every time step, which raises a statistical estimation challenge for conventional AIL. Specifically, the $\ell_1$-norm estimation error of maximum likelihood estimation is highest at uniform distribution (refer to the discussion below \citep[Lemma 8]{kamath2015learning}). From Figure~\ref{fig:bandit_m_log_result}, we clearly see that the slopes of VAIL, FEM and GTAL with respect to $\log \lp m \rp$ are around $-1/2$. This can be explained by their sample complexity ${\gO}( |\gS| H^2/\varepsilon^2)$, which implies $\log(V^{\piE} - V^{\pi}) \precsim -1/2 \log(m) + \text{constant}$. This empirical result demonstrates the sample barrier issue of VAIL discussed in \cref{subsec:when_does_vail_generalize_poorly}. Combined with the observation on the horizon dependence, these results verify the sample complexity lower bound of VAIL in \cref{prop:lower_bound_vail} and further indicate that its worst-case sample complexity in \cref{theorem:worst_case_sample_complexity_of_vail} is tight. As for TAIL, as shown in Figure~\ref{fig:bandit_m_log_result}, the policy value gap of TAIL diminishes substantially faster than VAIL, FEM, and GTAL, which verifies the sample efficiency of TAIL. The fast diminishing rate of BC is due to the quick concentration rate of missing mass; see \citep{rajaraman2020fundamental} for more explanation.

\textbf{Case Study on Reset Cliff.} Next, we consider the Reset Cliff MDP (\cref{fig:reset_cliff}) with 1 bad absorbing state and 19 good states. For Reset Cliff, the agent gets $+1$ reward by taking the expert action (shown in green) on states except the bad state $b$, then the next state is renewed according to the initial state distribution $\rho$. Here, $\rho = ( {1}/({m+1}), \cdots, {1}/({m+1}), 1 - {(\vert \mathcal{S} \vert -2)}/{(m+1)}, 0 )$ \citep{rajaraman2020fundamental}. Once taking a non-expert action (shown in blue), the agent goes to the absorbing state $b$ and gets $0$ reward.

On the one hand, Reset Cliff highlights the compounding errors issue and recovers the key characteristics of many practical tasks. Take the Gym MuJoCo locomotion task as an example, once the robot takes a wrong action, it would go to the terminate state and obtain $0$ reward forever. The numerical result about the planning horizon is given in Figure \ref{fig:cliffwalking_h_log_result}. From \cref{fig:cliffwalking_h_log_result}, we clearly see that the slope of BC w.r.t $\log (H)$ is around $2$, indicating the compounding errors issue of BC. As for conventional AIL methods, especially VAIL, their policy value gaps almost keep constant as the planning horizon increases. This result validates the horizon-free sample complexity of AIL approaches on Reset Cliff.

On the other hand, we consider the dependence on the number of expert demonstrations; the corresponding numerical result is shown in Figure \ref{fig:cliffwalking_m_log_result}. From Figure \ref{fig:cliffwalking_m_log_result}, we see that the slopes of all methods are around $-1$. Combined with the quadratic horizon dependency of BC, we empirically validate that the sample complexity analysis of BC is tight. Notice that we do not empirically observe the sample barrier issue of VAIL on Reset Cliff. The reason is that there is no statistical difficulty in estimating the state distribution of the expert policy on Reset Cliff. More specifically, instead of the uniform distribution on Standard Imitation, the state distribution of the expert policy on Reset Cliff is $( {1}/({m+1}), \cdots, {1}/({m+1}), 1 - {(\vert \mathcal{S} \vert -2)}/{(m+1)}, 0)$ in each step. When $m$ is large, this distribution assigns all probability mass on the 
penultimate state and thus the estimation problem is easy. We empirically validate this claim. In particular, the $\ell_1$-norm estimation error of maximum likelihood estimation is illustrated in \cref{fig:estimation_result}. We see that the slope on Standard Imitation is about $-1/2$ while the slope on Reset Cliff is about $-1$. This result is consistent with the policy value gap of VAIL on Standard Imitation (\cref{fig:bandit_m_log_result}) and Reset Cliff (\cref{fig:cliffwalking_m_log_result}).

\begin{figure}[htbp]
\begin{subfigure}{.42\textwidth}
  \centering
  \includegraphics[width=0.8\textwidth]{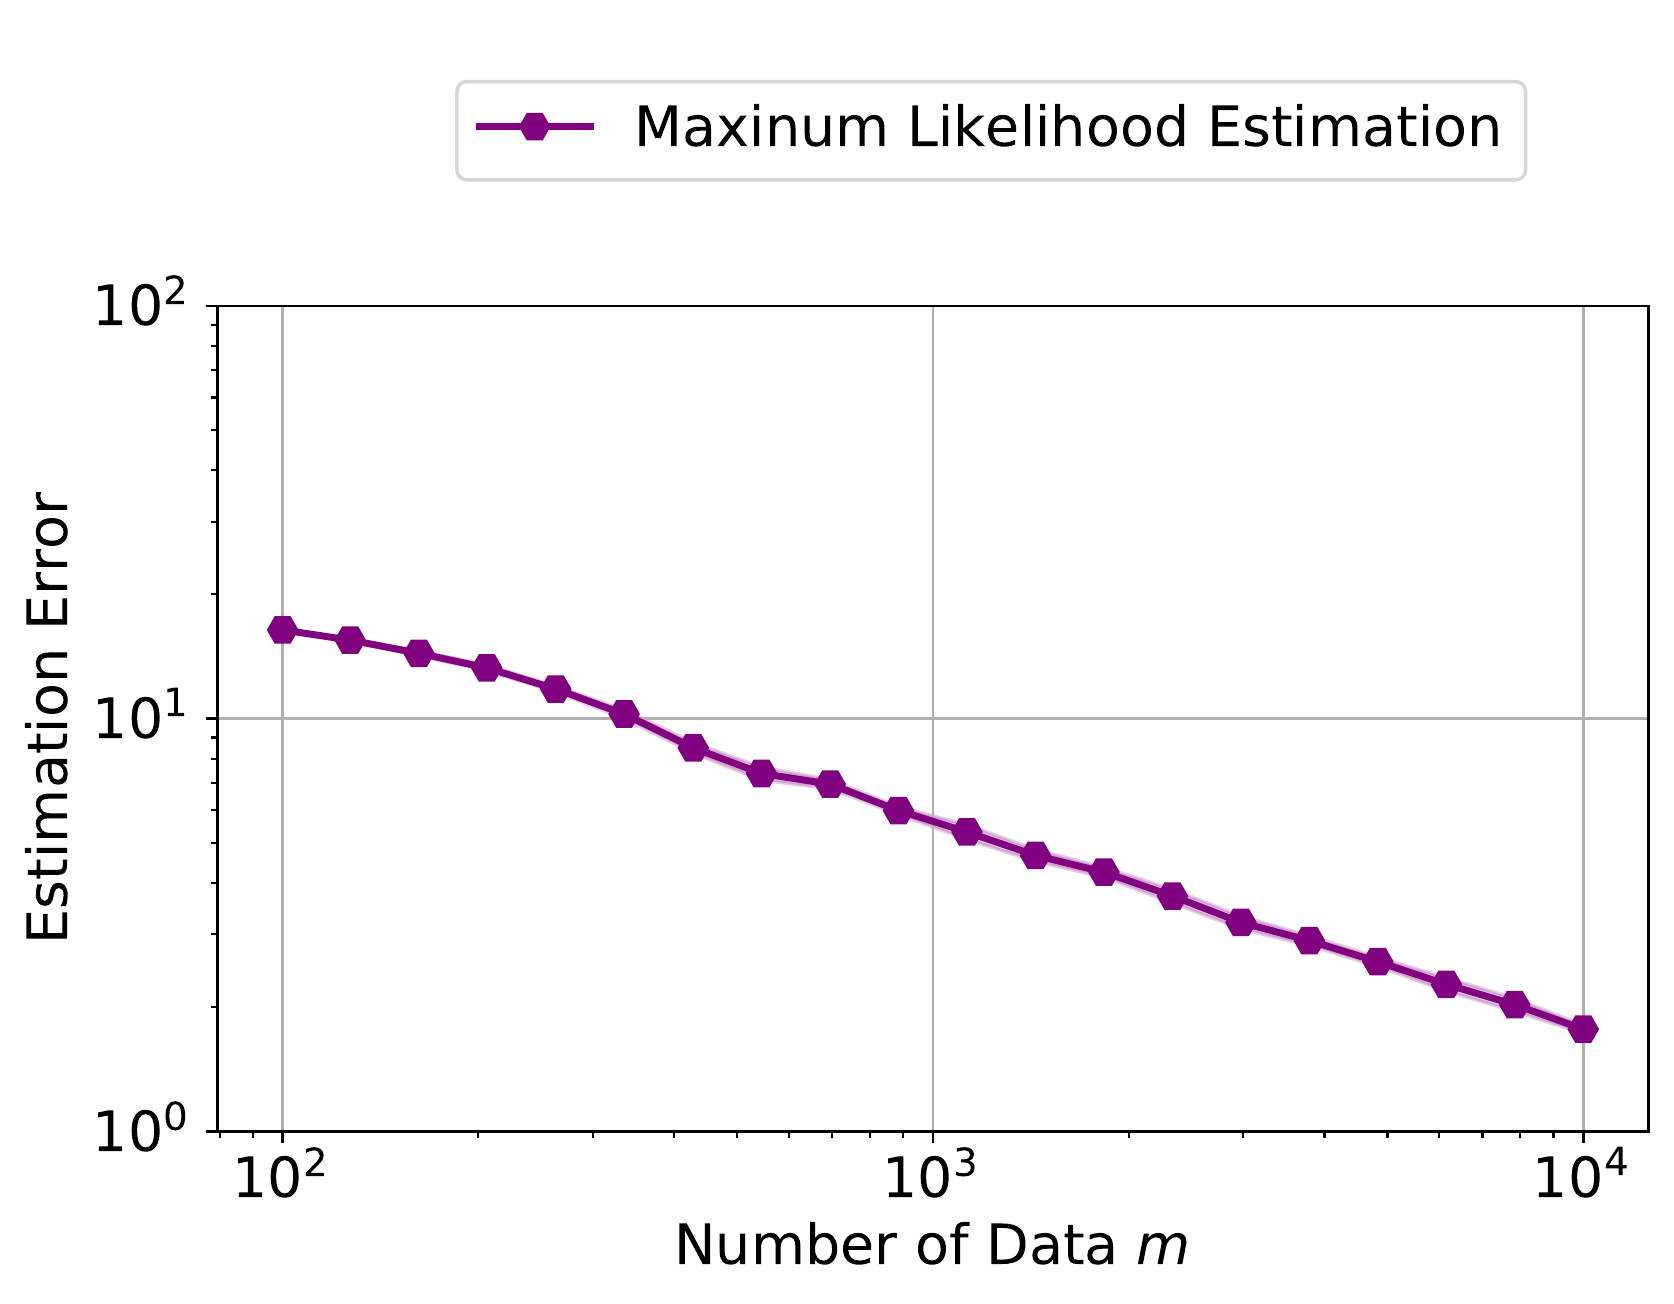}
  \caption{The $\ell_1$-norm estimation error on Standard Imitation.}
  \label{fig:mle_estimation_error_bandit}
\end{subfigure}
\hfill
\begin{subfigure}{.42\textwidth}
  \centering
  \includegraphics[width=0.8\textwidth]{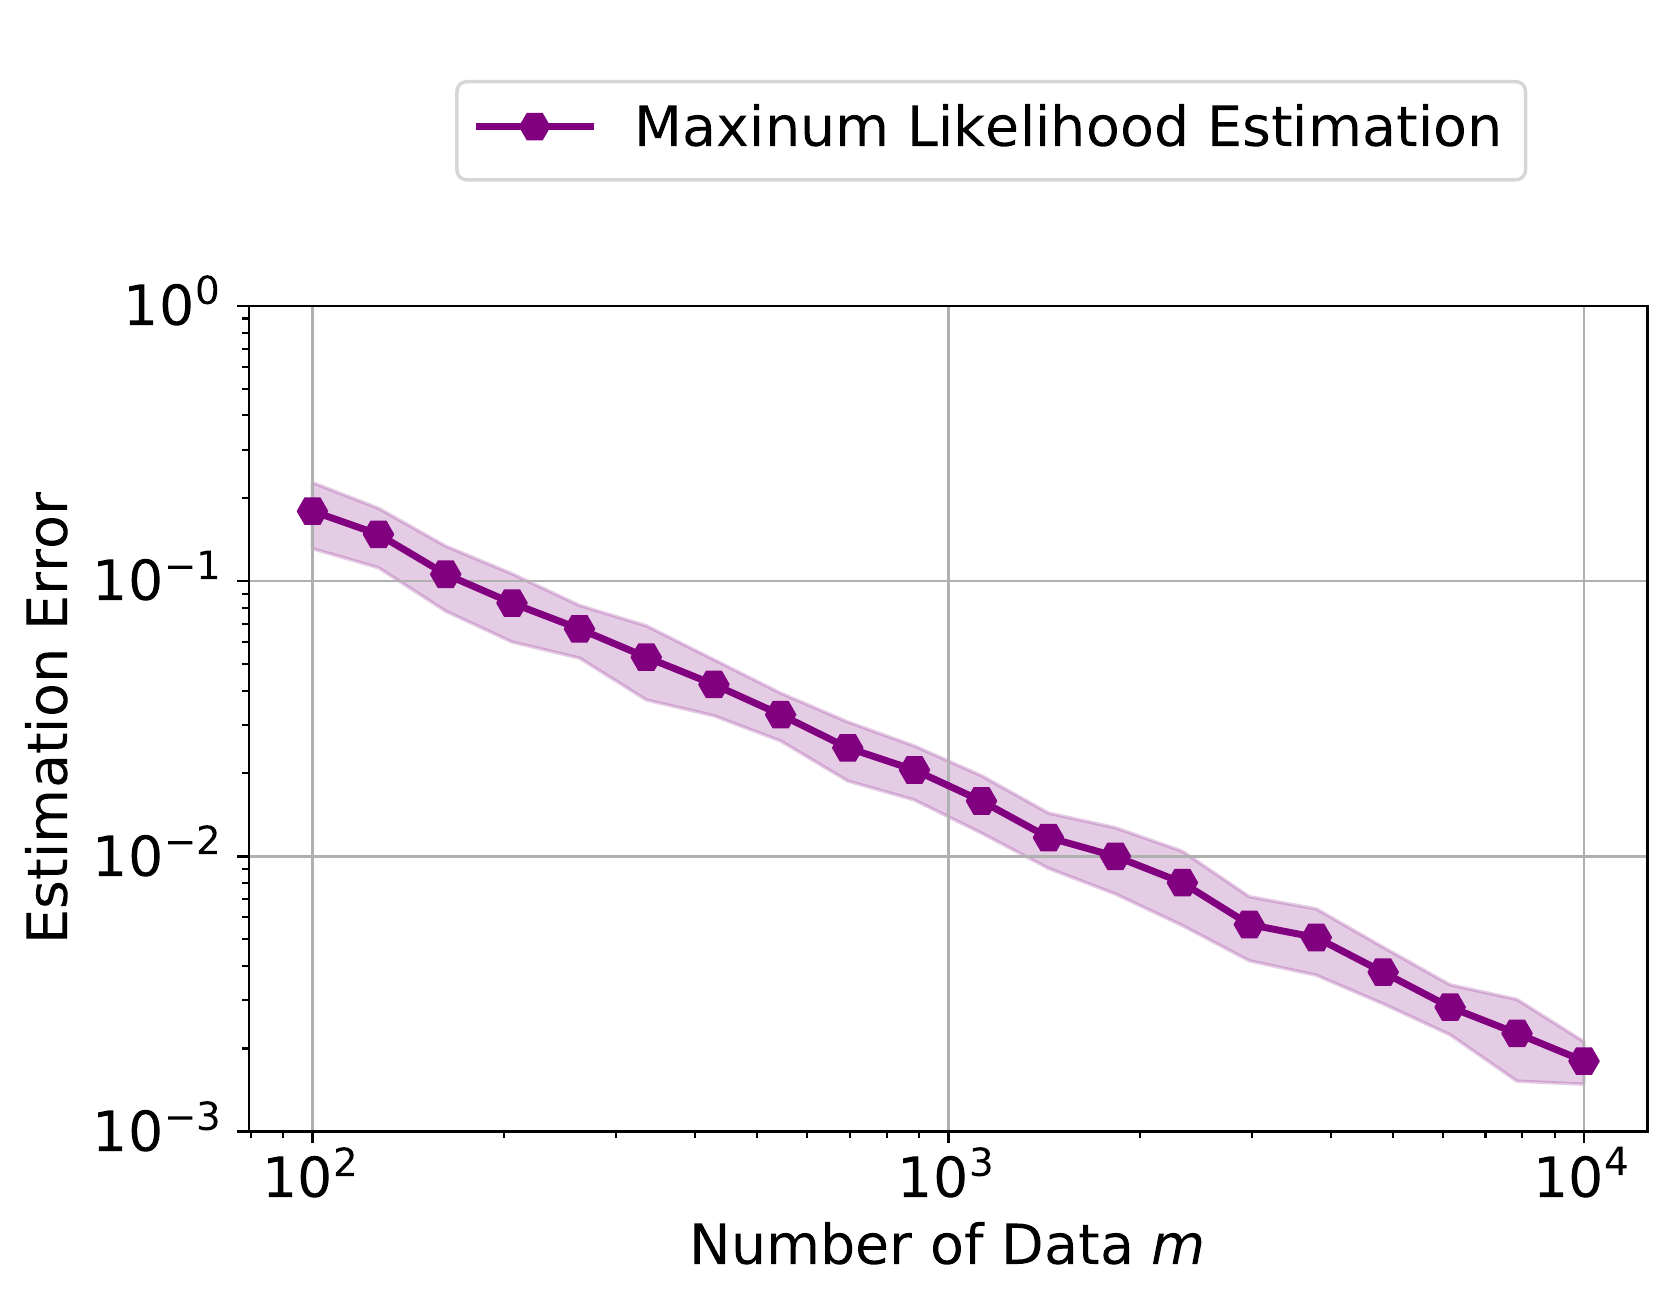}
  \caption{The $\ell_1$-norm estimation error on Reset Cliff.}
  \label{fig:mle_estimation_error_cliffwalking}
\end{subfigure}
\caption{The $\ell_1$-norm estimation error of maximum likelihood estimation $\sum_{h=1}^{H} \Vert P^{\piE}_h - \widehat{P}_h^{\piE} \Vert_1$ on Standard Imitation and Reset Cliff with different number of expert demonstrations.}
\label{fig:estimation_result}
\end{figure}

\subsection{Unknown Transitions Setting}
\label{appendix:experiment_unknown_transition}

In this part, we study the interaction complexity under the unknown transition setting. We still use the above two MDPs, but they may not be hard instances. Hence, we do not verify the tightness of order dependency. The comparison involves BC~\citep{Pomerleau91bc}, OAL~\citep{shani21online-al} and MB-TAIL (see Algorithm \ref{algo:mbtail-abstract}). All algorithms are provided with the same expert demonstrations.

Empirical results are displayed in Figure~\ref{fig:unknown_transition_result}. Note that BC does not need interaction. Similar to the results shown in Figure \ref{figure:main_results}, BC performs worse than MB-TAIL on Reset Cliff while BC could be better than MB-TAIL on Standard Imitation. Moreover, we see that MB-TAIL outperforms OAL provided with the same number of interactions.

\begin{figure}[htbp]
\begin{subfigure}{.42\textwidth}
  \centering
  \includegraphics[width=0.8\textwidth]{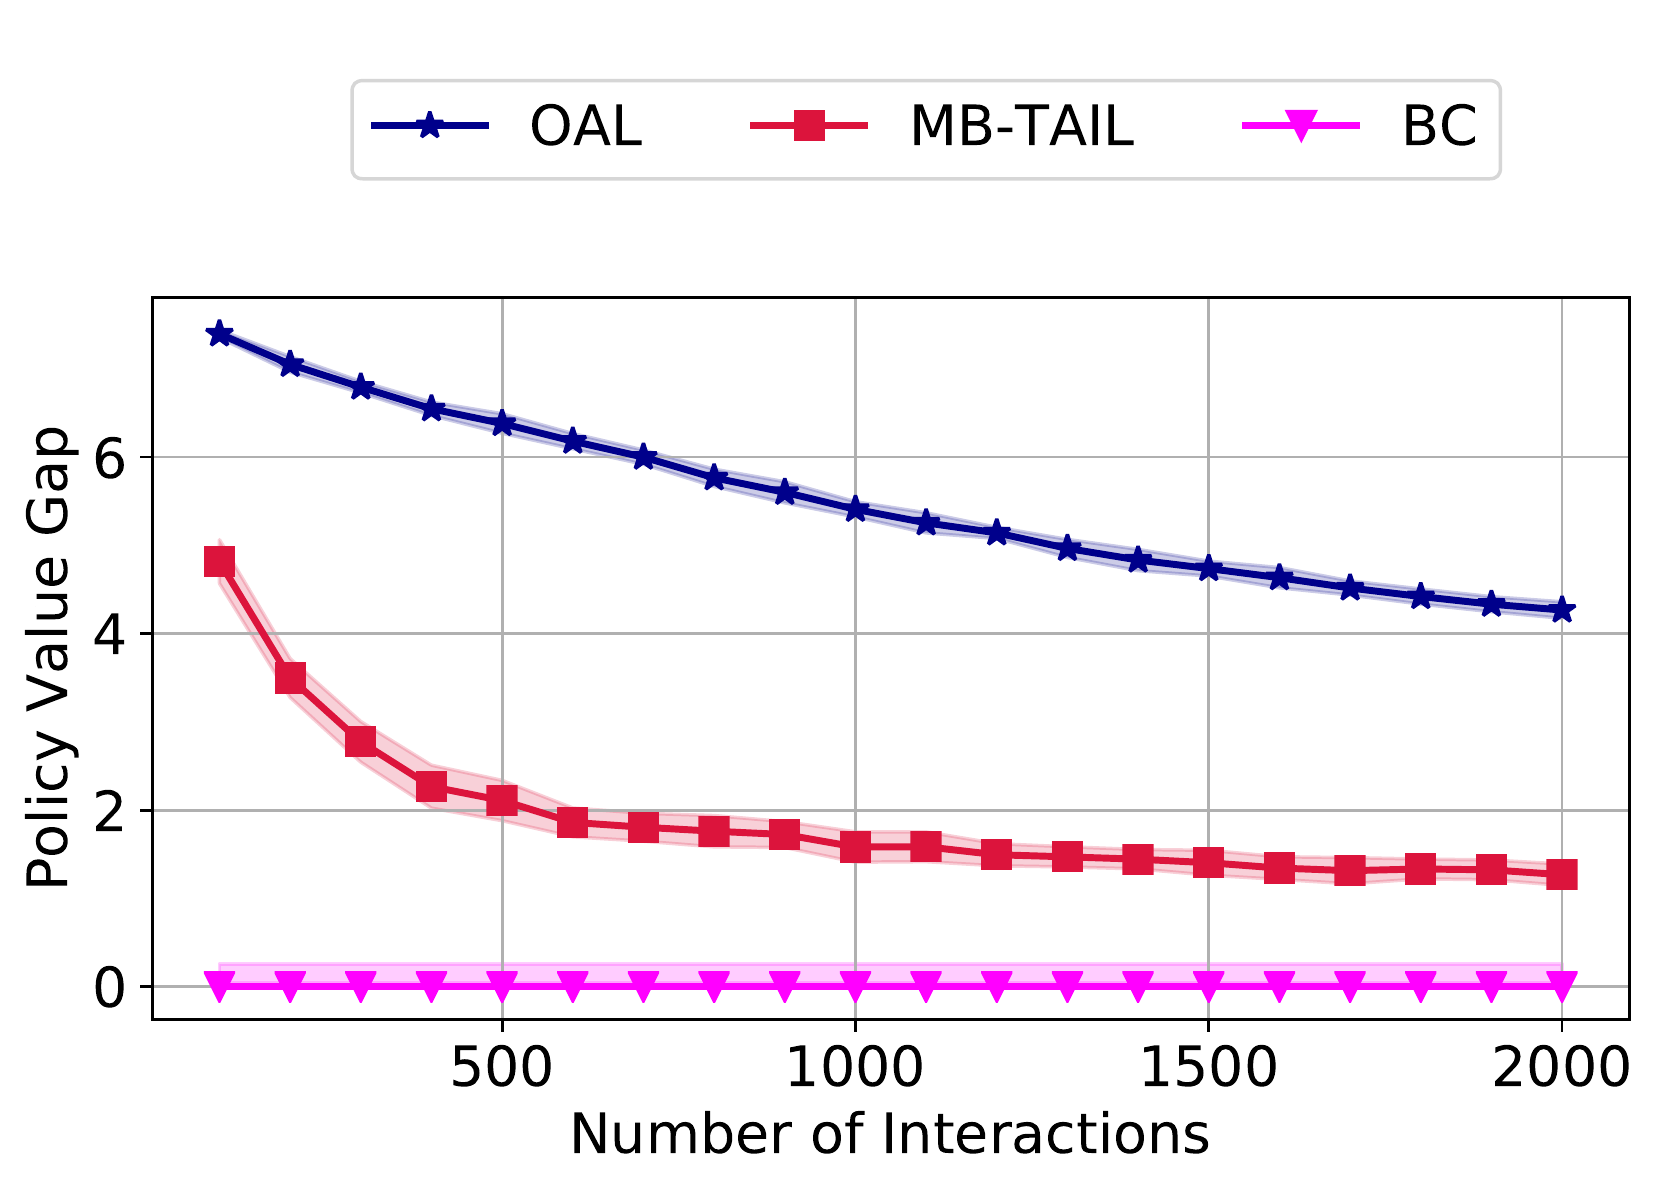}
  \caption{The policy value gap on Standard Imitation.}
  \label{fig:unknown_transition_bandit}
\end{subfigure}
\hfill
\begin{subfigure}{.42\textwidth}
  \centering
  \includegraphics[width=0.8\textwidth]{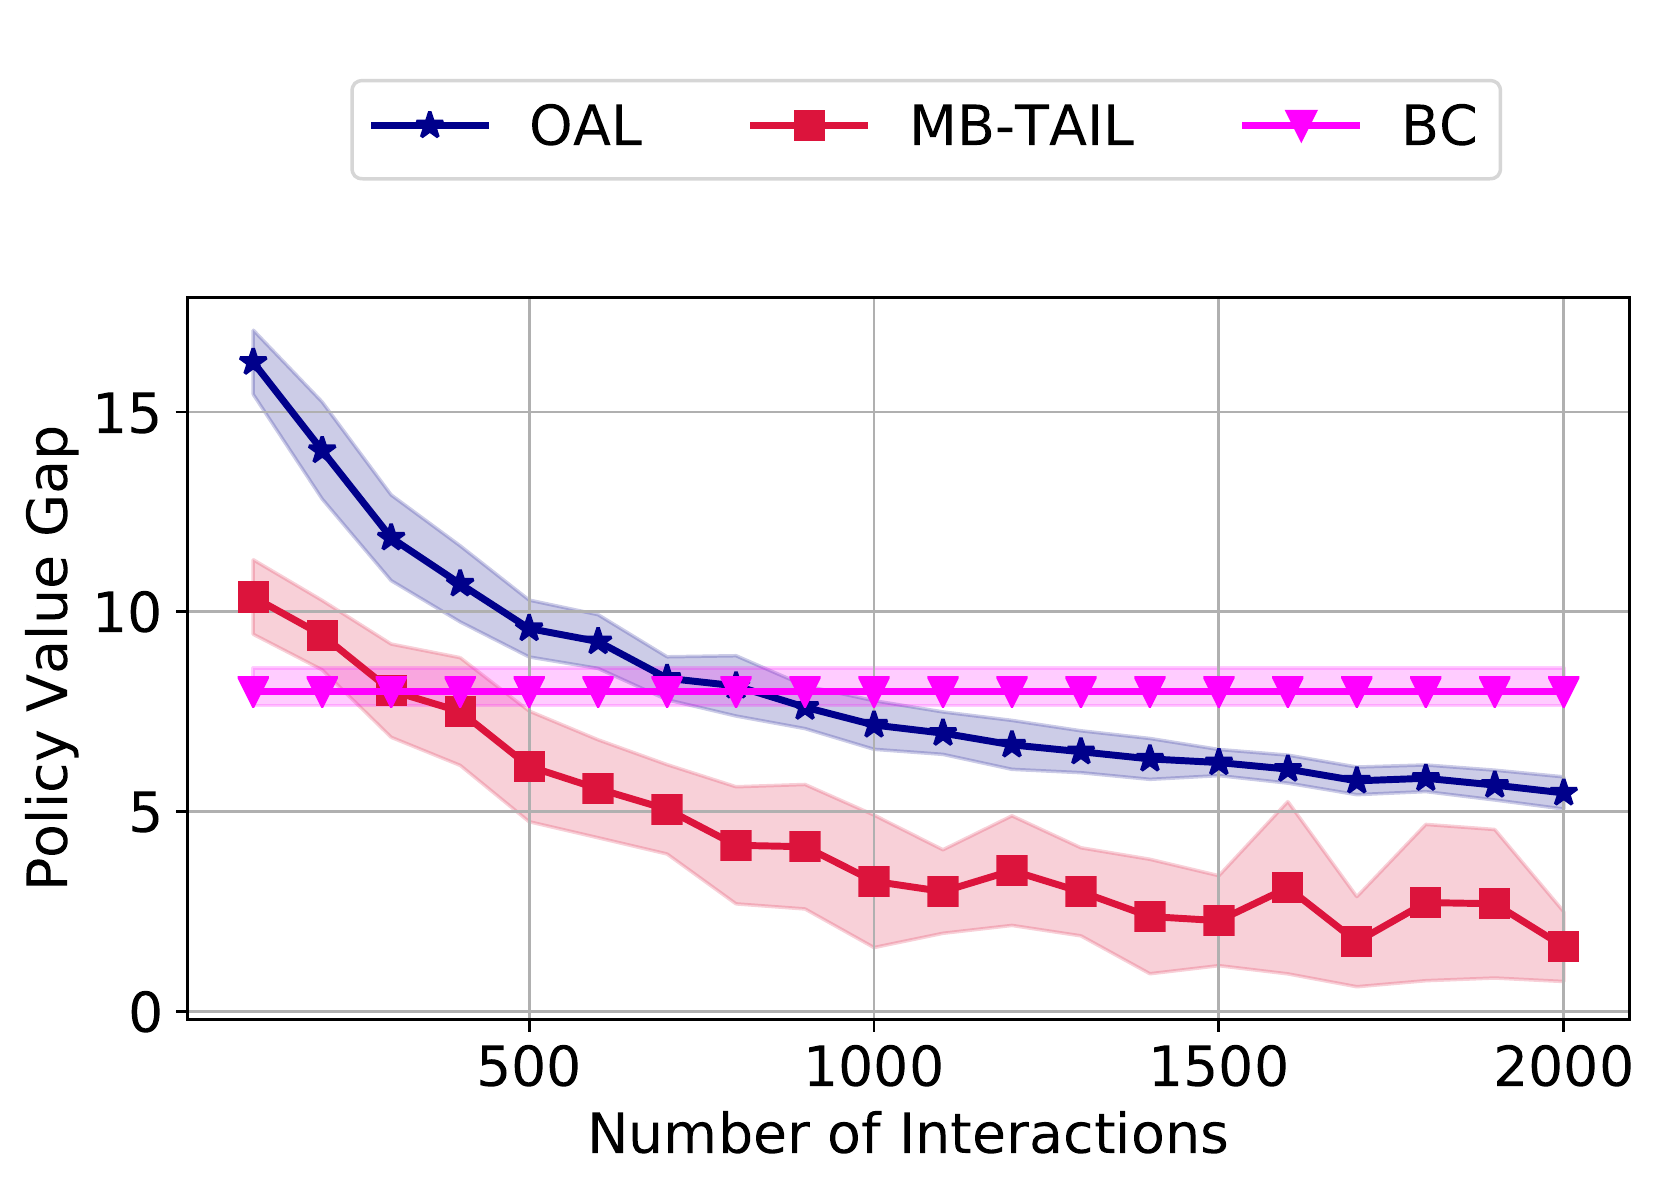}
  \caption{The policy value gap on Reset Cliff.}
  \label{fig:unknown_transition_cliffwalking}
\end{subfigure}
\caption{The policy value gap (i.e., $V^{\piE} - V^{\pi}$) on Standard Imitation and Reset Cliff with different number of interactions.}
\label{fig:unknown_transition_result}
\end{figure}

\subsection{Experiment Details}
\label{subsection:experiment_details}
\subsubsection{Known Transition Setting}

All experiments are run with $20$ random seeds. The detailed information on tasks is listed in Table \ref{table:task_information}. All experiments  are run on the machine with $32$ CPU cores, $128$ GB RAM and NVIDIA GeForce RTX $2080$ Ti.

BC directly estimates the expert policy from expert demonstrations. The information on the number of optimization iterations of VAIL, FEM, GTAL and TAIL is summarized in Table \ref{table:num_iterations}. In each iteration, with the recovered reward function, all conventional AIL methods utilize value iteration to solve the optimal policy. As discussed in ~\citep{Zahavy20al_via_frank-wolfe}, the optimization problem of FEM can be solved by Frank Wolfe (FW) algorithm ~\citep{frank1956algorithm}. In particular, the step size of FW is determined by line search. GTAL uses multiplicative weights to solve the outer problem in \eqref{eq:new_algo_max_min}. VAIL and our algorithm TAIL utilize online gradient descent to update the reward function. To utilize the optimization structure, an adaptive step size~\citep{Orabona19a_modern_introduction_to_ol} is implemented for GTAL, VAIL and our algorithm TAIL\footnote{Conclusions about the sample complexity and computational complexity do not change by this adaptive step size.}: 
\begin{align*}
    \eta_{t} = \frac{D}{ \sqrt{\sum_{i=1}^t \lnorm \nabla_{w} f^{(i)} \lp w^{(i)} \rp \rnorm_2^2}},
\end{align*}
where $D = \sqrt{2H |\gS| |\gA|}$ is the diameter of the set $\gW$. After the training process, we evaluate the policy value via exact Bellman update.

\begin{table}[htbp]
\caption{Information about tasks under known transition setting.}
\label{table:task_information}
\centering
{ \small
\begin{tabular}{@{}lllll@{}}
\toprule
Tasks           & Number of states & Number of actions & Horizon & Number of expert trajectories \\ \midrule

Standard Imitation (Figure \ref{fig:bandit_h_log_result})   & 500             & 5 & $10^{1} \to 10^{3}$ & 300 \\ 
\midrule
Standard Imitation (Figure \ref{fig:bandit_m_log_result}) & 500 & 5 &  $10$ &$10^{2} \to 10^{4}$         \\
\midrule
Reset Cliff (Figure \ref{fig:cliffwalking_h_log_result})          & 20              & 5      & $10^{1} \to 10^{3}$          & 5000           \\
\midrule
Reset Cliff (Figure \ref{fig:cliffwalking_m_log_result}) & 5 & 5 & $5$ & $10^2 \to 10^4$
\\
\bottomrule
\end{tabular}%
}
\end{table}

\begin{table}[htbp]
\caption{The number of optimization iterations of different algorithms on Standard Imitation and Reset Cliff.}
\label{table:num_iterations}
\centering
{ \small
\begin{tabular}{@{}lllll@{}}
\toprule
Tasks          & VAIL & FEM & GTAL  &TAIL \\ \midrule
Standard Imitation (Figure \ref{fig:bandit_h_log_result}) & $500$ & $500$ & $500$ & $500$
\\
\midrule
Standard Imitation (Figure \ref{fig:bandit_m_log_result}) & $8000$ & $8000$ & $8000$ & $8000$ \\ 
\midrule
Reset Cliff (Figure \ref{fig:cliffwalking_h_log_result})                      & $4H$ & $300$      & $4H$            & $H$                    \\ \midrule
Reset Cliff (Figure \ref{fig:cliffwalking_m_log_result}) & $20000$ & $20000$ & $20000$ & $20000$
\\ \bottomrule
\end{tabular}%
}
\end{table}

\subsubsection{Unknown Transition Setting}

All experiments are run with $20$ random seeds. Table \ref{table:task_information_unknown_transition_setting} summaries the detailed information on tasks under the unknown transition setting.

In particular, OAL is a model-based method and uses mirror descent (MD)~\citep{beck2003mirror} to optimize policy and reward. The step sizes of MD are set by the results in the theoretical analysis of~\citep{shani21online-al}. During the interaction, OAL maintains an empirical transition model to estimate Q-function for policy optimization. To encourage exploration, OAL adds a bonus function to the Q-function. The bonus used in the theoretical analysis of~\citep{shani21online-al} is too 
large in experiments and hence, OAL requires too many interactions to reach a good and stable performance. Therefore, we simplify their bonus function from $b_{h}^k (s, a)=\sqrt{ \frac{4  |\gS| H^{2} \log \lp 3  |\gS| |\gA| H^{2} n / \delta \rp}{ n_{h}^{k}(s, a) \vee 1}}$ to  $b_{h}^k (s, a)=\sqrt{\frac{ \log \lp  |\gS| |\gA| H n / \delta \rp}{n_{h}^{k}(s, a) \vee 1}}$, where $n$ is the total number of interactions, $\delta$ is the failure probability and $n^{k}_h (s, a)$ is the number of times visiting $(s, a)$ in time step $h$ until episode $k$.

MB-TAIL first establishes the estimator in \eqref{eq:new_estimator_unknown_transition} with half of the environment interactions and learns an empirical transition model by invoking RF-Express~\citep{menard20fast-active-learning} to collect the other half of trajectories. Subsequently, MB-TAIL performs policy and reward optimization with the recovered transition model. In MB-TAIL, the policy and reward optimization steps are the same as TAIL.

\begin{table}[htbp]
\caption{Information about tasks under unknown transition setting.}
\label{table:task_information_unknown_transition_setting}
\centering
{ \small
\begin{tabular}{@{}lllll@{}}
\toprule
Tasks           & Number of states & Number of actions & Horizon & Number of expert trajectories \\ \midrule
Reset Cliff          & 20              & 5      &  20          & 100           \\
\midrule 
Standard Imitation   & 100             & 5 & 10  & 400          \\ \bottomrule
\end{tabular}%
}
\end{table}

\subsection{GAIL}
\label{subsection:additional_results_gail}

\begin{figure*}[htbp]
     \centering
     \begin{subfigure}[b]{0.23\textwidth}
         \centering
         \includegraphics[width=\textwidth]{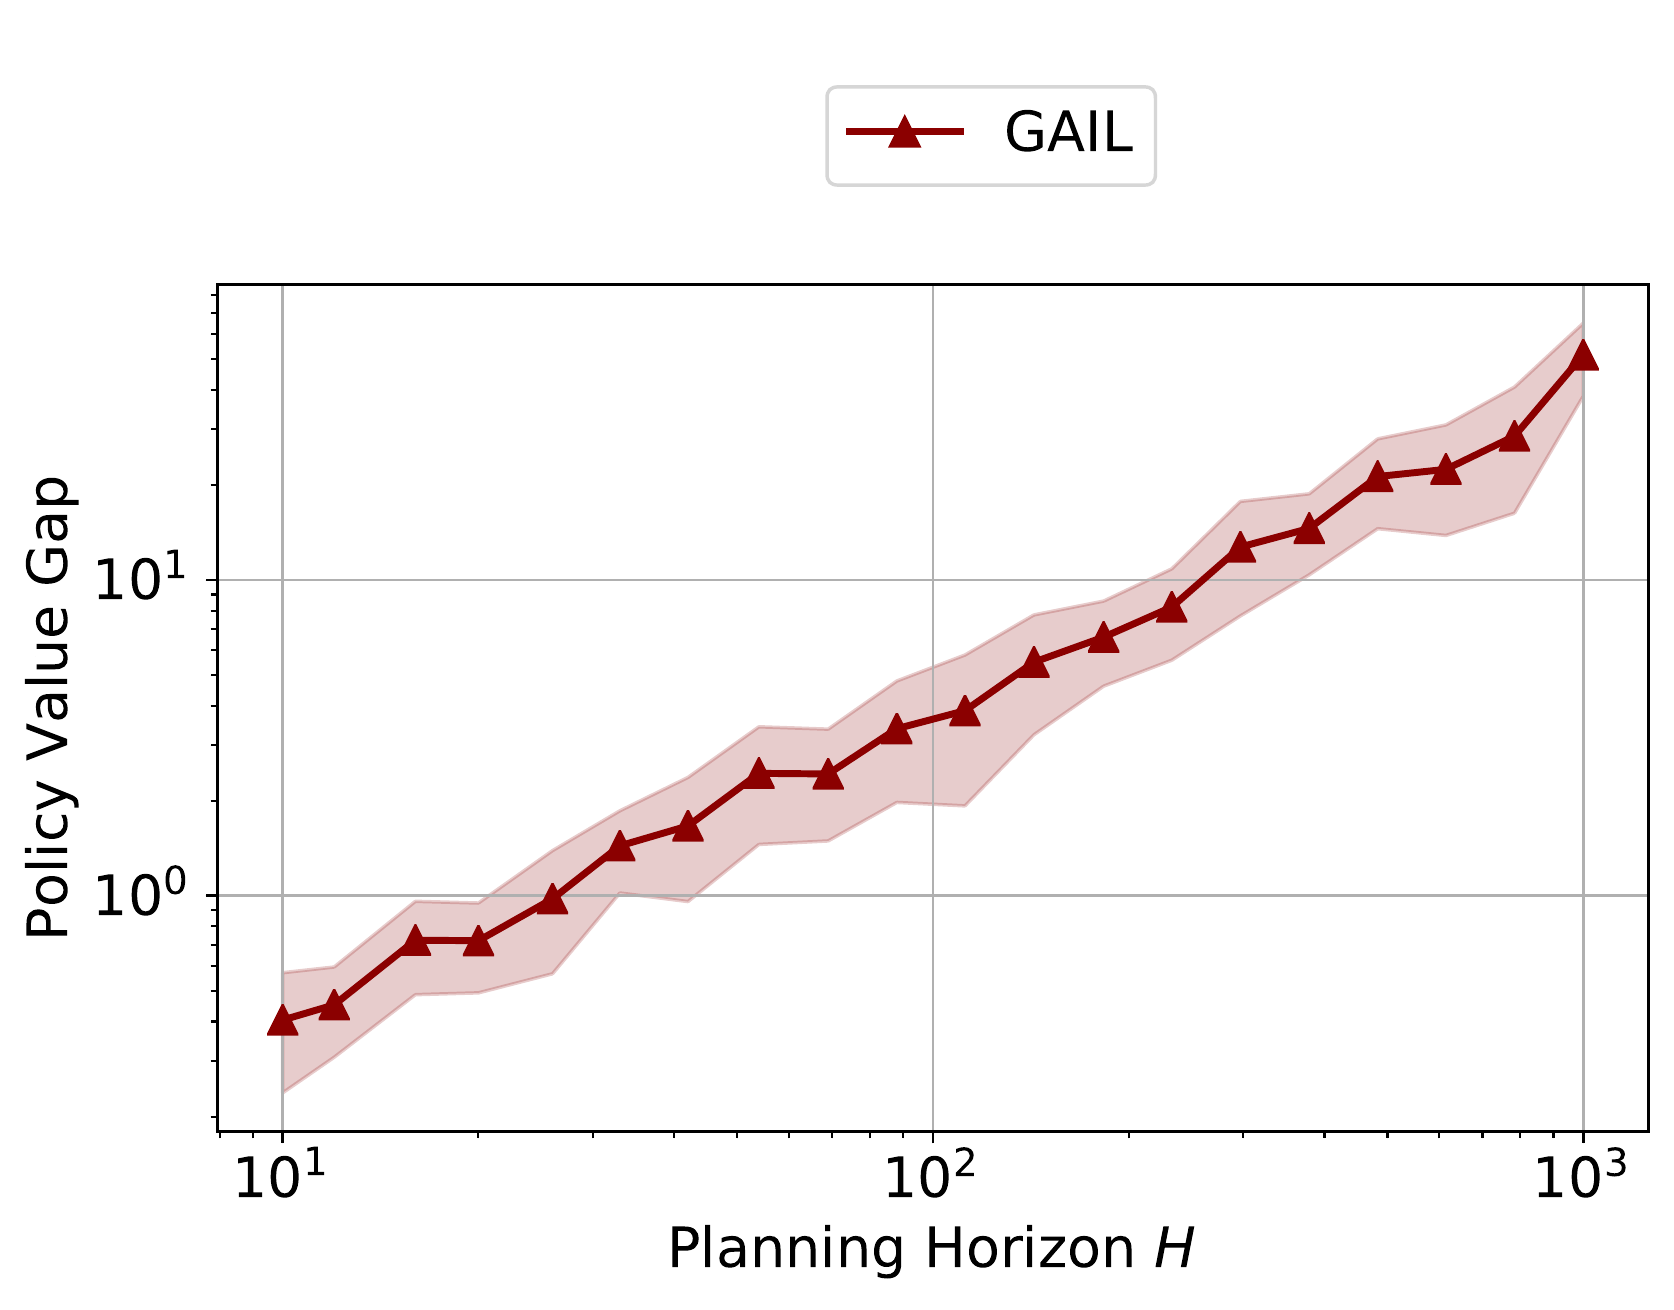}
         \caption{On the planning horizon on Standard Imitation.}
         \label{fig:gail_bandit_h_log_result}
     \end{subfigure}
     \hfill
     \begin{subfigure}[b]{0.23\textwidth}
         \centering
         \includegraphics[width=\textwidth]{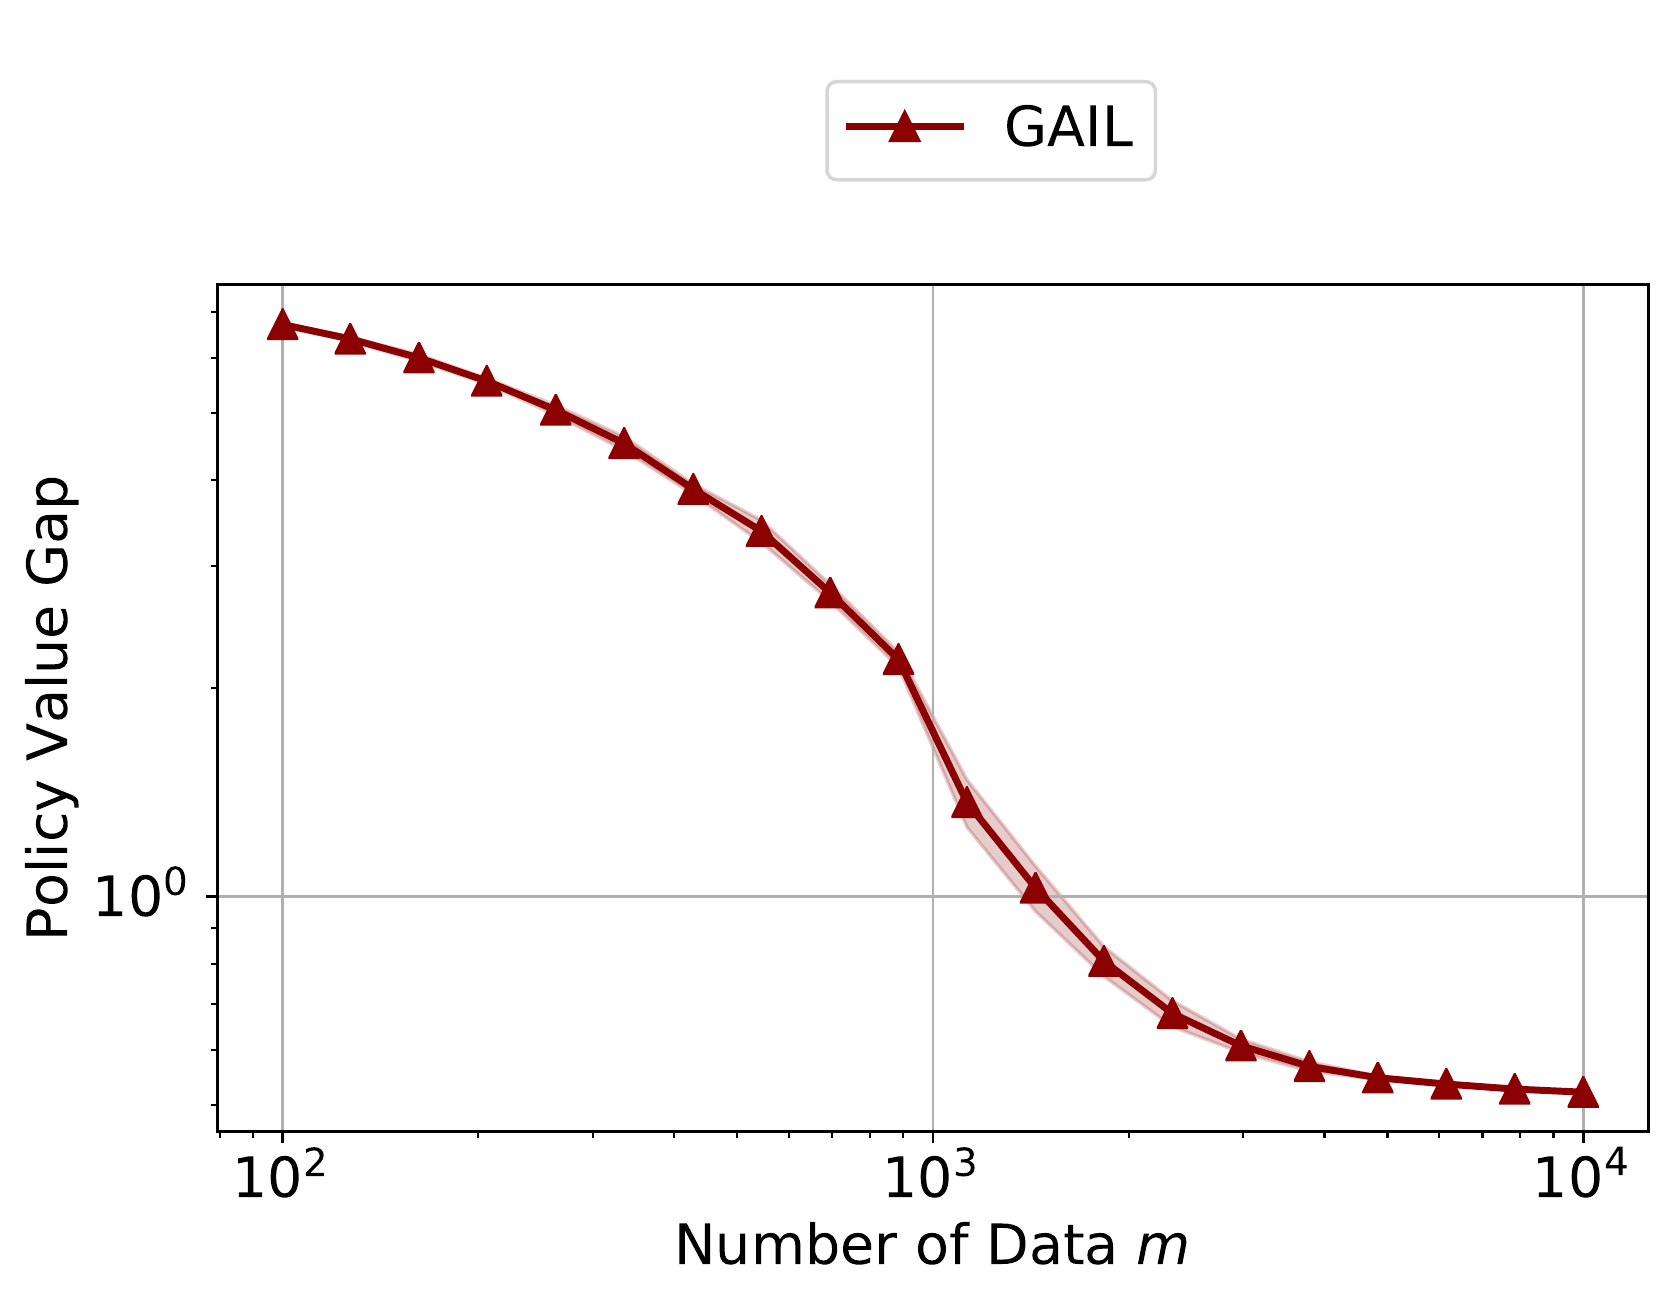}
         \caption{On the expert sample size on Standard Imitation.}
         \label{fig:gail_bandit_m_log_result}
     \end{subfigure}
     \hfill
     \begin{subfigure}[b]{0.23\textwidth}
         \centering
         \includegraphics[width=\textwidth]{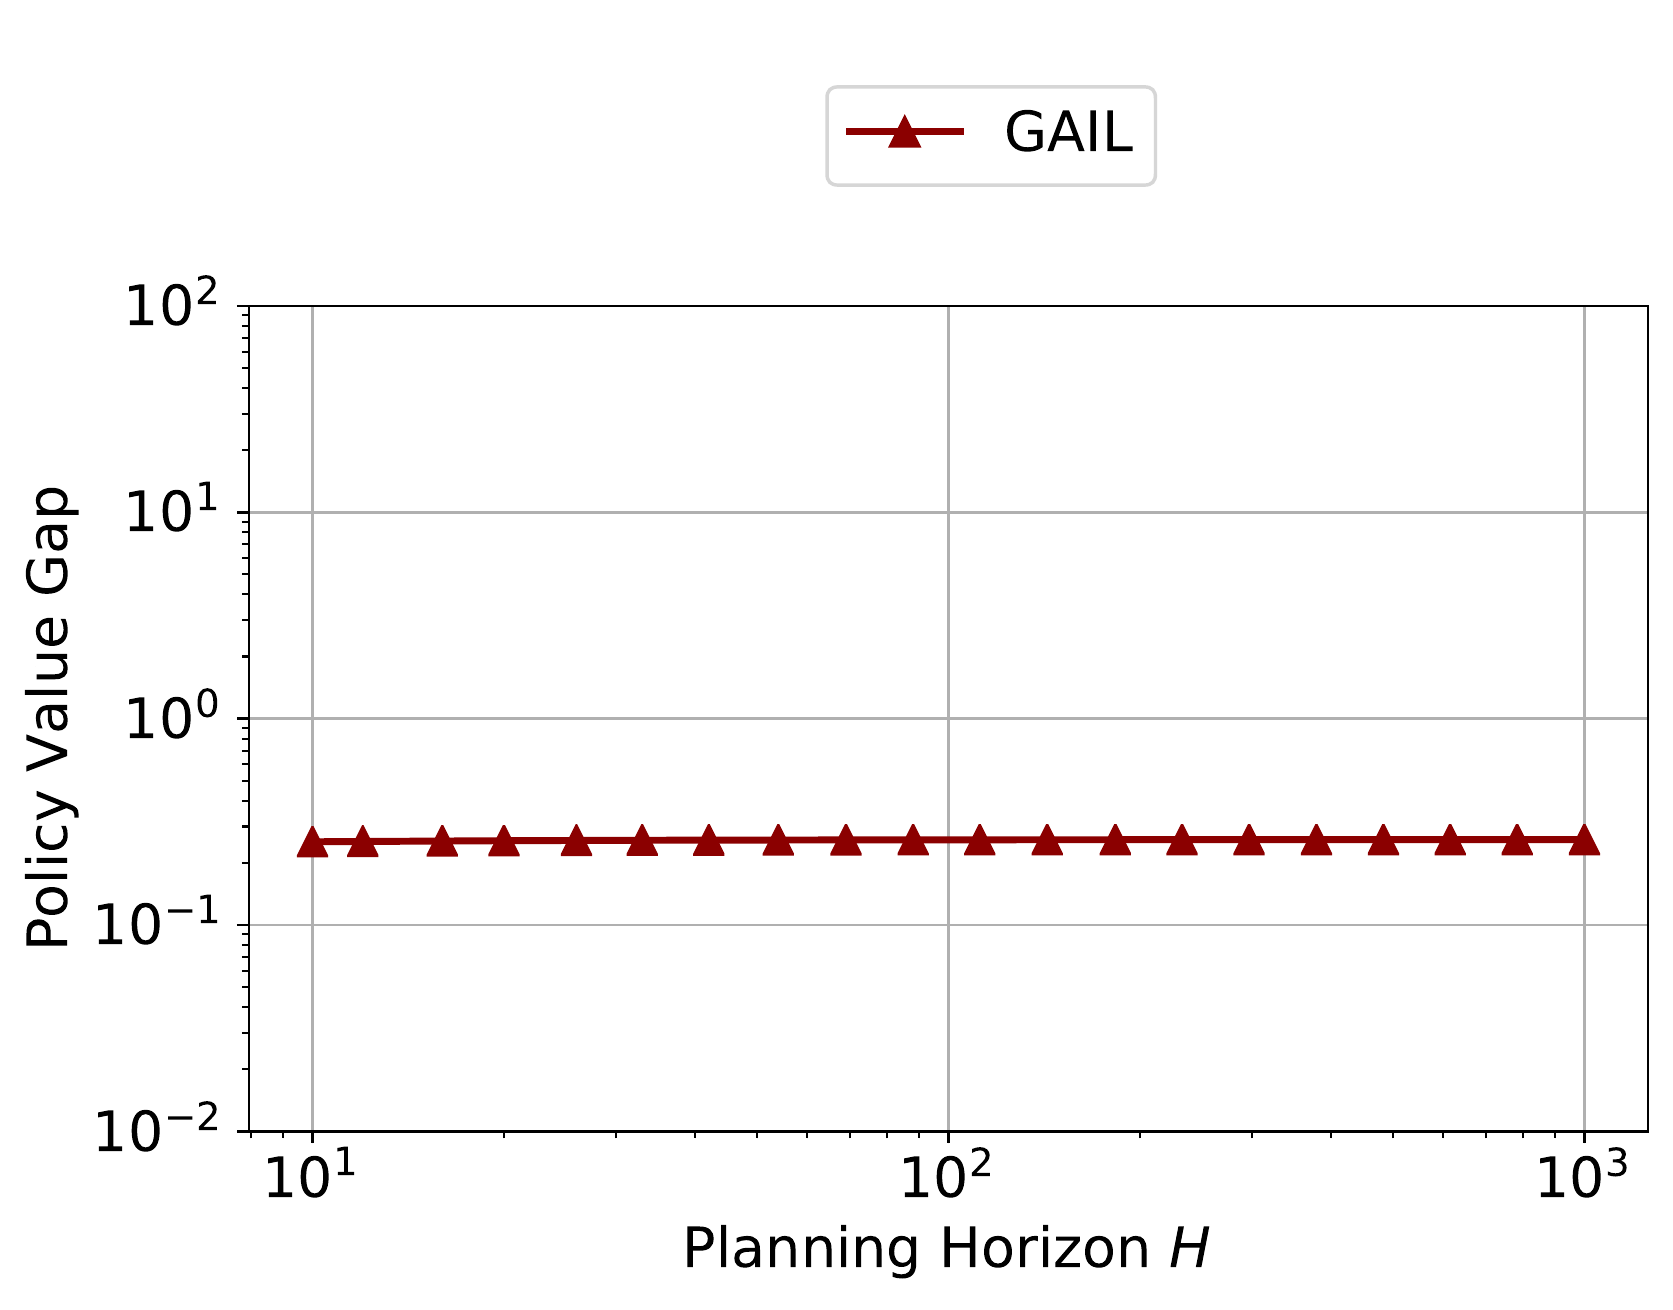}
         \caption{On the planning horizon on Reset Cliff.}
         \label{fig:gail_cliffwalking_h_log_result}
     \end{subfigure}
     \hfill
    \begin{subfigure}[b]{0.23\textwidth}
      \centering
      \includegraphics[width=\textwidth]{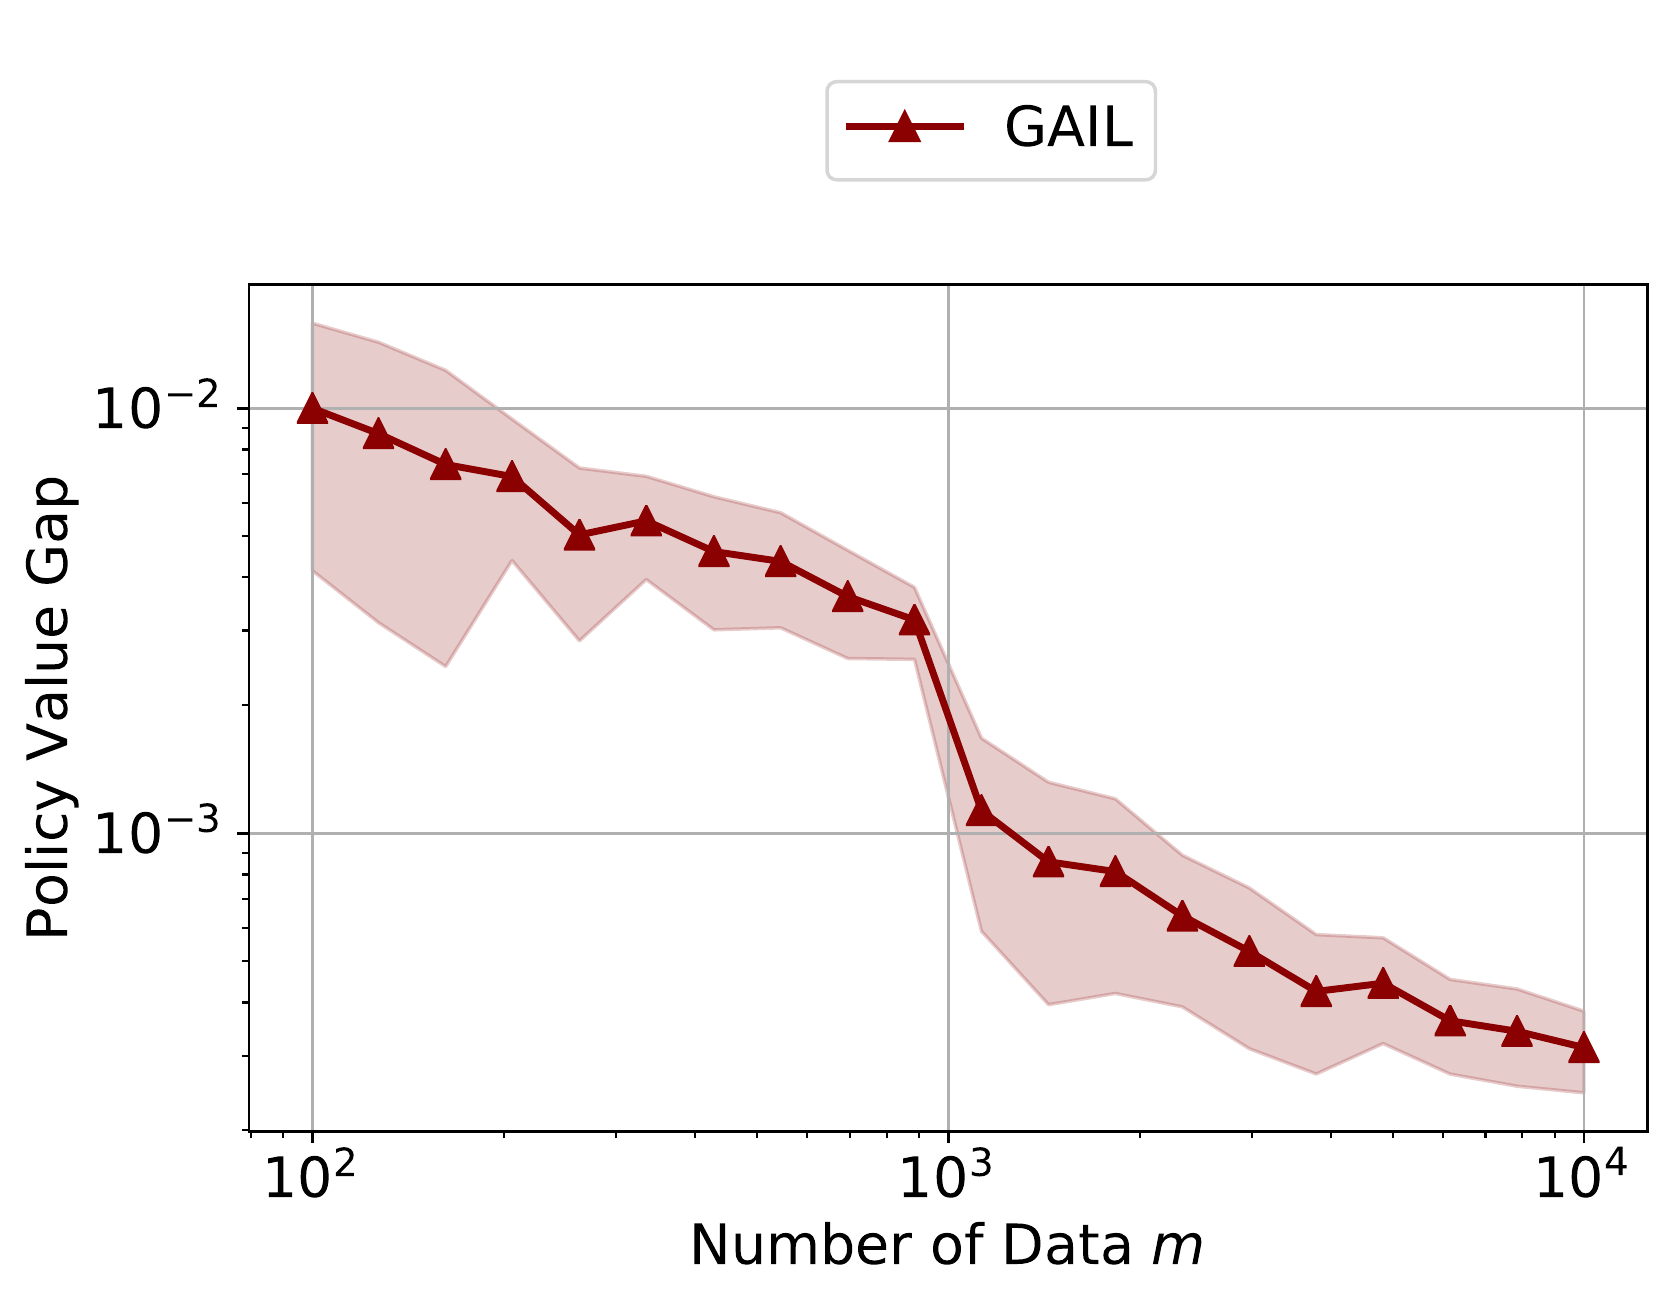}
      \caption{On the expert sample size on Reset Cliff.}
      \label{fig:gail_cliffwalking_m_log_result}
    \end{subfigure}

     \caption{The policy value gap (i.e., $V^{\piE} - V^{\pi}$) of GAIL on Standard Imitation and Reset Cliff. The solid lines are mean of results and the shaded region corresponds to the standard deviation over $20$ random seeds.}
     \label{figure:gail_results}
\end{figure*}

Under the known transition setting, we also test a famous practical AIL method named GAIL~\citep{ho2016gail}. Let $D = (D_1, \cdots, D_H)$ with $D_h: \gS \times \gA \rar [0, 1]$ for $h \in [H]$. The min-max objective of GAIL is shown as follows.
\begin{align}
    \min_{\pi \in \Pi} \max_{D} \sum_{h=1}^H \expect_{(s, a) \sim P^{\piE}_h} \ls \log \lp 1 - D_h (s, a) \rp \rs + \sum_{h=1}^H \expect_{(s, a) \sim P^{\pi}_h} \ls \log \lp D_h (s, a) \rp \rs.
    \label{eq:gail_objective}
\end{align}
\citet{ho2016gail} provided a practical implementation of GAIL under the unknown transition setting. Specifically, GAIL uses stochastic gradient descent ascent (SGDA) to update the policy and reward function alternatively. It is well-known even the full-batch version of SGDA (i.g., GDA) may not converge properly \citep{benaim1999mixed, lin2020gda}. As such, GAIL has no theoretical guarantee about the convergence or sample complexity.

To study the sample complexity of GAIL under the known transition setting, we make a small modification. In particular, we use the closed-form solution to the inner loop problem in \eqref{eq:gail_objective}:
\begin{align*}
    D^*_h (s, a) = \frac{P^{\pi^{(t)}}_h (s, a)}{P^{\pi^{(t)}}_h (s, a) + P^{\piE}_h (s, a)}.
\end{align*}
Then the recovered reward function is 
\begin{align*}
    w^{(t+1)}_h (s, a) = - \log \lp D^*_h (s, a) \rp.
\end{align*}
As for the policy, we use the mirror descent update~\citep{shalev12online-learning}, which is widely applied to solving a saddle point problem:
\begin{align*}
    \pi^{(t+1)}_h (a|s) = \frac{\pi^{(t)}_h (a|s) \exp \lp \eta Q^{\pi^{(t)}}_h (s, a) \rp}{\sum_{a^\prime \in \gA} \pi^{(t)}_h (a^\prime|s) \exp \lp \eta Q^{\pi^{(t)}}_h (s, a^\prime) \rp },
\end{align*}
where $\eta$ is the stepsize and $Q^{\pi^{(t)}}_h (s, a)$ is the action value function of $\pi^{(t)}$ with reward $w^{(t)}$.

The results of GAIL on Standard Imitation and Reset Cliff are plotted in Figure \ref{figure:gail_results}. Compared with results in Figure \ref{figure:main_results}, we see that the performance of GAIL is comparative with other conventional AIL methods such as FEM and GTAL. In particular, there is no  difference in the order dependence of the planning horizon and the expert sample size between GAIL and conventional AIL methods. This is reasonable since all of them follow the state-action distribution matching principle and use the naive estimation in \eqref{eq:estimate_by_count}.
