# Supplementary material for: A Note on Target Q-learning For Solving Finite MDPs with A Generative Oracle
Source: arXiv:2203.11489 source file (2022-03-22)
Supplement: Supplementary file 3 [file extension.tex]

\section{Extension of MIMIC-MD}
\label{appendix:extension_of_mimic_md}

In this section, we develop an extension of MIMIC-MD under the unknown transition setting. Before presentation, we note that the exact optimal solutions of the original MIMIC-MD formulation cannot be solved in a polynomial time as stated in \citep{rajaraman2020fundamental}. To this end, we will first establish an adversarial formulation for MIMIC-MD, which allows us to use gradient based methods to efficiently obtain an approximate solution. We call such a method TAIL (Transition-aware AIL). Then, we show how to combine TAIL with reward-free exploration methods in the unknown transition scenario. 

\subsection{TAIL}

With the improved estimator in \eqref{eq:new_estimator}, we arrive at the following state-action distribution matching problem:
\begin{align} \label{eq:l1_norm_imitation_with_estimator} 
   \min_{\pi \in \Pi} \sum_{h=1}^{H} \lnorm P^{\pi}_h - \widetilde{P}^{\piE}_h \rnorm_1.
\end{align}
We highlight that \eqref{eq:l1_norm_imitation_with_estimator} is slightly different from MIMIC-MD's objective in \citep{rajaraman2020fundamental}. Specifically, MIMIC-MD restricts candidate policies to $\Pi_{\text{BC}} (\gD_1) = \{ \pi \in \Pi: \pi_h (s) = \piE_h (s), \forall h \in [H], s \in \gS_h (\gD_1) \}$, which is the set of BC policies on $\gD_1$. The intuition in MIMIC-MD is that the expert actions are known on $\gD_1$ so that direct projection is feasible.

Now, we would like to develop an adversarial formulation for \eqref{eq:l1_norm_imitation_with_estimator}.  With the famous min-max theorem~\citep{bertsekas2016nonlinear}, we transform \eqref{eq:l1_norm_imitation_with_estimator} to:
\begin{align}   \label{eq:new_algo_max_min}
     \max_{w \in \gW} \min_{\pi \in \Pi} \sum_{h=1}^H \sum_{(s, a)} w_h (s, a) \lp \widetilde{P}^{\piE}_h (s, a) -  P^{\pi}_h (s, a)  \rp.
\end{align}
where $\gW = \{w: \lnorm w \rnorm_\infty \leq 1 \}$ is the unit ball. We see that the inner problem in \eqref{eq:new_algo_max_min} is to maximize the policy value of $\pi$ given the reward function $w_h(s, a)$. For the outer optimization problem, we can use online gradient descent methods \citep{shalev12online-learning} so that we can finally reach an approximate saddle point. Formally, let us define the objective $f^{(t)}(w)$:
\begin{align}   
    & \sum_{h=1}^{H} \sum_{(s, a)} w_h(s, a) \lp P^{\pi^{(t)}}_h (s, a) - \widetilde{P}^{\piE}_h (s, a)  \rp, \label{eq:objective_w}
\end{align}
where $\pi^{(t)}$ is the optimized policy at iteration $t$. Then the update rule for $w$ is:
\begin{align*}   
    w^{(t+1)} := \gP_{\gW}\lp w^{(t)} - \eta^{(t)}  \nabla f^{(t)}(w^{(t)}) \rp, 
\end{align*}
where $\eta^{(t)} > 0$ is the stepsize to be chosen later, and $\gP_{\gW}$ is the Euclidean projection on the unit  ball $\gW$, i.e., $\gP_{\gW}(w) := \argmin_{z \in \gW} \lnorm z- w \rnorm_2$. The procedure for solving \eqref{eq:new_algo_max_min} is outlined in \cref{algo:main_aglorithm}.

\begin{algorithm}[htbp]
\caption{\textsf{TAIL}}
\label{algo:main_aglorithm}
{
\begin{algorithmic}[1]
\REQUIRE{expert demonstrations $\gD$, number of iterations $T$, step size $\eta^{(t)}$, and initialization $w^{(1)}$.}
\STATE{Randomly split $\gD$ into two equal parts: $\gD = \gD_1 \cup \gD_1^{c}$ and obtain the estimation $\widetilde{P}_h^{\piE}$ in \eqref{eq:new_estimator}.}
\FOR{$t = 1, 2, \cdots, T$}
\STATE{$\pi^{(t)} \lar $ solve the optimal policy with the reward function $w^{(t)}$ up to an error of $\varepsilon_{\mathrm{opt}}$.}
\STATE{Compute the state-action distribution $P^{\pi^{(t)}}_h$ for $\pi^{(t)}$.}
\STATE{Update $ w^{(t+1)} := \gP_{\gW}\lp w^{(t)} - \eta^{(t)}  \nabla f^{(t)}(w^{(t)}) \rp$ with $f^{(t)}(w)$ defined in \eqref{eq:objective_w}.}
\ENDFOR
\STATE{Compute the mean state-action distribution $\widebar{P}_h(s, a) = \sum_{t=1}^{T} P^{\pi^{(t)}}_h(s, a) / T$.}
\STATE{Derive $\widebar{\pi}_h (a|s) \lar \widebar{P}_h(s, a) / \sum_{a} \widebar{P}_h(s, a)$.}
\ENSURE{policy $\widebar{\pi}$.}
\end{algorithmic}
}
\end{algorithm}

\begin{thm} \label{theorem:final_sample_complexity} 
Fix $\varepsilon \in \lp 0, H \rp$ and $\delta \in (0, 1)$; suppose $H \geq 5$. Consider the approach \textsf{TAIL} in Algorithm \ref{algo:main_aglorithm} with $\widebar{\pi}$ being the output policy. Assume that the optimization error $\varepsilon_{\mathrm{opt}} \leq \varepsilon / 2$, the number of iterations $T \succsim  |\gS|  |\gA| H^2 / \varepsilon^2$, and the step size $\eta^{(t)} :=  \sqrt{|\gS||\gA| / (8T)}$. If the number of expert trajectories ($m$) satisfies
\begin{align*}
m \succsim  \frac{  |\gS| H^{3/2}}{\varepsilon} \log\lp\frac{ |\gS| H}{\delta} \rp,
\end{align*}
then with probability at least $1-\delta$, we have $V^{\piE} - V^{\widebar{\pi}} \leq \varepsilon$.
\end{thm}
See \cref{appendix:proof_of_theorem:final_sample_complexity} for the proof. Let us briefly discuss the computation details of \textsf{TAIL}. For the optimization problem in Line 3 of \cref{algo:main_aglorithm}, we can use value iteration or policy gradient methods \citep{agarwal2020pg}. Specifically, if we use value iteration, it is clear that $\varepsilon_{\opt} = 0$ and this procedure can be done in $H$ iterations. For each iteration of the value iteration algorithm, the computation complexity is $\gO(|\gS||\gA| \times |\gS| + |\gS| |\gA|)$ for computing the target $Q$-values and  greedy actions for each state-action pairs. Since the total number of iterations of \cref{algo:main_aglorithm} is $\gO( |\gS| |\gA| H^2/\varepsilon^2)$, we have the following total computation complexity:
\begin{align*}
    \gO(|\gS|^2|\gA|) \times H  \times \gO( |\gS| |\gA| H^2/\varepsilon^2) = \gO(|\gS|^3 |\gA|^2 H^{3}/\varepsilon^2).
\end{align*}
On the other hand, the space complexity of \cref{algo:main_aglorithm} is $\gO(|\gS||\gA|H)$ for storing $w^{(t)}, \pi^{(t)}$ and $P^{\pi^{(t)}}_h$.

We notice that in \citep{nived2021provably}, a linear programming (LP) formulation is proposed to solve the exactly optimal solutions of MIMIC-MD. The computation complexity of this method is about $\widetilde{\gO}(d^{2.5})$ where $d = 2|\gS| |\gA| H$. However, the space complexity of this method is $\gO(|\gS|^2 |\gA|^2 H^2)$, which is unbearable in practice; see the evidence in \cref{appendix:experiments}.

\subsection{MB-TAIL}
\label{subsection:mb-tail}

In the following part, we present how to apply \textsf{TAIL} in Algorithm \ref{algo:main_aglorithm} under our framework. As mentioned, the main challenge is that the refined estimation in \eqref{eq:new_estimator} requires the knowledge of the true transition function. Unfortunately, we cannot utilize the biased empirical model instead of the true transition, since the induced estimation error is difficult to control.

Technically, the term ${\sum_{\tr_h \in \Tr_h^{\gD_1} } \sP^{\piE}(\tr_h) \indict \{ \tr_h(s_h, a_h) = (s, a)\}}$ in \eqref{eq:new_estimator} relies on the exact transition function. To address the mentioned issue, we present a key observation in \cref{lemma:unknown-transition-unbiased-estimation} in \cref{subsection:proof-of-theorem-sample-complexity-unknown-transition}. In particular, for a BC policy $\pi \in \Pi_{\text{BC}} \lp \gD_{1} \rp$, for all trajectories $\tr_h \in \Tr_h^{\gD_1}$, the trajectory probabilities induced by $\pi$ and $\piE$ are identical up to time step $h$. Based on this observation, we can estimate this term with a dataset $\gD^{\prime}_{\text{env}}$ collected by rolling out a BC policy $\pi \in \Pi_{\text{BC}} \lp \gD_{1} \rp$ with the environment. The new estimator is formulated as
\begin{align}
  \widetilde{P}_h^{\piE} (s, a) = {\frac{\sum_{\tr_h \in \gD_{\text{env}}^\prime} \indict \{ \tr_h (s_h, a_h) = (s, a), \tr_h \in \Tr_h^{\gD_1} \}}{|\gD^\prime_{\text{env}}|}} + {\frac{  \sum_{\tr_h \in \gD_1^c}  \indict\{ \tr_h (s_h, a_h) = (s, a), \tr_h \not\in \Tr_h^{\gD_1}  \} }{|\gD_1^c|}}. \label{eq:new_estimator_unknown_transition}
\end{align}
With the estimator in \eqref{eq:new_estimator_unknown_transition}, we develop an extension of TAIL named \textsf{MB-TAIL} presented in Algorithm \ref{algo:mbtail-abstract}. 

\begin{algorithm}[htbp]
\caption{\textsf{MB-TAIL}}
\label{algo:mbtail-abstract}
\begin{algorithmic}[1]
\REQUIRE{expert demonstrations $\gD$.}
\STATE{Randomly split $\gD$ into two equal parts: $\gD = \gD_1 \cup \gD_1^{c}$.}
\STATE{Learn $\pi \in \Pi_{\text{BC}} \lp \gD_{1} \rp$ by BC and roll out $\pi$ to obtain dataset $\gD_{\text{env}}^\prime$ with $|\gD_{\text{env}}^\prime| = n^{\prime}$}.
\STATE{Obtain the estimator $\widetilde{P}_h^{\piE}$ in \eqref{eq:new_estimator_unknown_transition} with $\gD$ and $\gD_{\text{env}}^\prime$.}
\STATE{Invoke \textnormal{RF-Express} to collect $n$ trajectories and learn an empirical transition function $\widehat{\gP}$.}
\STATE{$\widebar{\pi} \lar$ apply TAIL to perform imitation with the estimation $\widetilde{P}_h^{\piE}$ under transition model $\widehat{\gP}$.}
\ENSURE{policy $\widebar{\pi}$.}
\end{algorithmic}
\end{algorithm}

\begin{thm}\label{theorem:sample-complexity-unknown-transition}
Fix $\varepsilon \in \lp 0, 1 \rp$ and $\delta \in (0, 1)$; suppose $H \geq 5$. Under the unknown transition setting, consider \textsf{MB-TAIL} displayed in Algorithm \ref{algo:mbtail-abstract} and $\widebar{\pi}$ is output policy, assume that the optimization error $\varepsilon_{\mathrm{opt}} \leq \varepsilon / 2$, the number of iterations and the step size are the same as in Theorem \ref{theorem:final_sample_complexity}, if the number of expert trajectories ($m$), the number of interaction trajectories for estimation ($n^\prime$), and the number of interaction trajectories for reward-free exploration ($n$) satisfy
\begin{align*}
&m \succsim  \frac{  |\gS| H^{3/2}}{\varepsilon} \log\lp\frac{ |\gS| H}{\delta} \rp, n^{\prime} \succsim  \frac{  |\gS| H^2}{\varepsilon^2} \log \lp \frac{ |\gS| H }{\delta} \rp,
\\
& n \succsim \frac{ |\gS| |\gA| H^3}{\varepsilon^2} \lp |\gS| + \log \lp \frac{ |\gS| |\gA| H}{\delta \varepsilon} \rp \rp
\end{align*}
Then with probability at least $1-\delta$, we have $V^{\piE} - V^{\widebar{\pi}} \leq \varepsilon $.
\end{thm}
See \cref{subsection:proof-of-theorem-sample-complexity-unknown-transition} for the proof.
