# Supplementary material for: A Note on Target Q-learning For Solving Finite MDPs with A Generative Oracle
Source: arXiv:2203.11489 source file (2022-03-22)
Supplement: Supplementary file 4 [file lemmas.tex]

\section{Technical Lemmas and Proofs}
\label{appendix:technical_lemmas}

\subsection{Basic Technical Lemmas}

\begin{lem}   \label{lemma:policy_dual_value}
For tabular and episodic MDP, we have that 
\begin{align*}
    V^{\pi} = \sum_{h=1}^{H} \sum_{(s, a) \in \gS \times \gA} P^{\pi}_h(s, a) r_h(s, a).
\end{align*}
\end{lem}

\begin{proof}
The proof is direct from the definition. 
\end{proof}

\begin{lem}   \label{lemma:state_dist_discrepancy}
For any tabular and episodic MDP, considering two policies $\pi$ and $\pi^\prime$, let $P^{\pi}_h (\cdot)$ and $P^{\pi}_h (\cdot, \cdot)$ denote the state distribution and state-action distribution induced by $\pi$ in time step $h$, respectively. Then we have that
\begin{itemize}
    \item 
    $
    \lnorm P^{\pi}_h (\cdot) - P^{\pi^\prime}_h (\cdot)  \rnorm_{1} \leq \sum_{\ell=1}^{h-1} \expect_{s \sim P^{\pi^\prime}_{\ell} (\cdot)} [\lnorm \pi_{\ell} (\cdot|s) - \pi^\prime_{\ell} (\cdot|s)   \rnorm_1]
    $ when $h \geq 2$.
    \item $\lnorm P^{\pi}_h (\cdot, \cdot) - P^{\pi^\prime}_h (\cdot, \cdot)  \rnorm_{1} \leq \lnorm P^{\pi}_h (\cdot) - P^{\pi^\prime}_h (\cdot)  \rnorm_{1} + \expect_{s \sim P^{\pi^\prime}_h (\cdot)} \ls \lnorm \pi_h (\cdot|s)  - \pi^\prime_h (\cdot|s) \rnorm_1 \rs $.
\end{itemize}
\end{lem}

\begin{proof}
We prove the first statement. It is direct to obtain that $\lnorm P^{\pi}_1 (\cdot) - P^{\pi^\prime}_1 (\cdot)  \rnorm_{1} = \lnorm \rho (\cdot) - \rho (\cdot)  \rnorm_{1}= 0$.

When $h \geq 2$, for any $\ell $ where $1 < \ell \leq h$, we prove the following recursion format.

\begin{align*}
    \lnorm P^{\pi}_\ell (\cdot) - P^{\pi^\prime}_\ell (\cdot)  \rnorm_{1} \leq \lnorm P^{\pi}_{\ell-1} (\cdot) - P^{\pi^\prime}_{\ell-1} (\cdot)  \rnorm_{1} +  \expect_{s \sim P^{\pi^\prime}_{\ell-1} (\cdot)} \ls \lnorm \pi_{\ell-1} (\cdot|s) - \pi^\prime_{\ell-1} (\cdot|s)   \rnorm_1 \rs.
\end{align*}
With the \dquote{transition flow equation}, we have
\begin{align*}
    &\quad \lnorm P^{\pi}_\ell (\cdot) - P^{\pi^\prime}_\ell (\cdot)  \rnorm_{1}
    \\
    &= \sum_{s \in \gS} \labs P^{\pi}_\ell (s) - P^{\pi^\prime}_\ell (s)  \rabs
    \\
    &= \sum_{s \in \gS} \labs \sum_{(s^\prime, a^\prime) \in \gS \times \gA} P^{\pi}_{\ell-1} (s^\prime) \pi_{\ell-1} (a^\prime|s^\prime) P_{\ell}(s|s^\prime, a^\prime) - \sum_{(s^\prime, a^\prime) \in \gS \times \gA} P^{\pi^\prime}_{\ell-1} (s^\prime) \pi^\prime_{\ell-1} (a^\prime|s^\prime) P_{\ell}(s|s^\prime, a^\prime)  \rabs
    \\
    &= \sum_{s \in \gS} \Bigg| \sum_{(s^\prime, a^\prime) \in \gS \times \gA} \lp P^{\pi}_{\ell-1} (s^\prime) - P^{\pi^\prime}_{\ell-1} (s^\prime) \rp \pi_{\ell-1} (a^\prime|s^\prime) P_{\ell}(s|s^\prime, a^\prime) 
    \\
    &\quad + \sum_{(s^\prime, a^\prime) \in \gS \times \gA} P^{\pi^\prime}_{\ell-1} (s^\prime) \lp \pi_{\ell-1} (a^\prime|s^\prime) -\pi^\prime_{\ell-1} (a^\prime|s^\prime) \rp  P_{\ell}(s|s^\prime, a^\prime)  \Bigg|
    \\
    &\leq \sum_{s \in \gS} \sum_{(s^\prime, a^\prime) \in \gS \times \gA} \labs P^{\pi}_{\ell-1} (s^\prime) - P^{\pi^\prime}_{\ell-1} (s^\prime) \rabs \pi_{\ell-1} (a^\prime|s^\prime) P_{\ell}(s|s^\prime, a^\prime)
    \\
    &\quad + \sum_{s \in \gS} \sum_{(s^\prime, a^\prime) \in \gS \times \gA} P^{\pi^\prime}_{\ell-1} (s^\prime) \labs \pi_{\ell-1} (a^\prime|s^\prime) -\pi^\prime_{\ell-1} (a^\prime|s^\prime) \rabs  P_{\ell}(s|s^\prime, a^\prime)
    \\
    &= \lnorm P^{\pi}_{\ell-1} (\cdot) - P^{\pi^\prime}_{\ell-1} (\cdot)  \rnorm_{1} + \expect_{s \sim P^{\pi^\prime}_{\ell-1} (\cdot)} \ls \lnorm \pi_{\ell-1} (\cdot|s) - \pi^\prime_{\ell-1} (\cdot|s)   \rnorm_1 \rs,  
\end{align*}
where we obtain the recursion format. Applying the recursion format with $\lnorm P^{\pi}_1 (\cdot) - P^{\pi^\prime}_1 (\cdot)  \rnorm_{1}=0$ finishes the proof of the first statement.

We continue to prove the second statement.
\begin{align*}
    &\quad \lnorm P^{\pi}_h (\cdot, \cdot) - P^{\pi^\prime}_h (\cdot, \cdot)  \rnorm_{1} 
    \\
    &= \sum_{(s, a) \in \gS \times \gA} \labs P^{\pi}_h (s, a) - P^{\pi^\prime}_h (s, a) \rabs
    \\
    &= \sum_{(s, a) \in \gS \times \gA} \labs P^{\pi}_h (s) \pi_h (a|s) - P^{\pi^\prime}_h (s) \pi^\prime_h (a|s) \rabs
    \\
    &= \sum_{(s, a) \in \gS \times \gA} \labs \lp P^{\pi}_h (s) - P^{\pi^\prime}_h (s) \rp \pi_h (a|s) + P^{\pi^\prime}_h (s) \lp \pi_h (a|s) -   \pi^\prime_h (a|s) \rp \rabs
    \\
    &\leq \sum_{(s, a) \in \gS \times \gA} \labs  P^{\pi}_h (s) - P^{\pi^\prime}_h (s) \rabs \pi_h (a|s) + \sum_{(s, a) \in \gS \times \gA} P^{\pi^\prime}_h (s) \labs \pi_h (a|s) -   \pi^\prime_h (a|s) \rabs
    \\
    &= \lnorm P^{\pi}_h (\cdot) - P^{\pi^\prime}_h (\cdot)  \rnorm_{1} + \expect_{s \sim P^{\pi^\prime}_h (\cdot)} \ls \lnorm \pi_h (\cdot|s)  - \pi^\prime_h (\cdot|s) \rnorm_1 \rs, 
\end{align*}
which proves the second statement.
\end{proof}

\begin{lem}
\label{lem:unique_opt_solution_condition}
Consider the optimization problem: $\min_{x \in [0, 1]^n} f (x) := \sum_{i=1}^m f_i (x)$, where $f_i : [0, 1]^n \rightarrow \reals, \forall i \in [m]$. Suppose that 1) there exists $k \in [m]$ such that $x^*$ is the unique optimal solution to $\min_{x \in [0, 1]^n} f_k (x)$; 2) for each $j \in [m], j \not= k$, $x^*$ is the optimal solution to $\min_{x \in [0, 1]^n} f_j (x)$. Then, $x^*$ is the unique optimal solution to $\min_{x \in [0, 1]^n} f (x)$.
\end{lem}

\begin{proof}
Since $x^*$ is the unique optimal solution to $\min_{x \in [0, 1]^n} f_k (x)$, we have that $\forall x \in [0, 1]^n, x \not= x^*$, $f_k (x^*) < f_k (x)$. Furthermore, for each $j \in [m], j \not= k$, recall that $x^*$ is the optimal solution to $\min_{x \in [0, 1]^n} f_j (x)$. We have that
\begin{align*}
    \forall j \in [m], j \not= k, \forall x \in [0, 1]^n, x \not= x^*, f_j (x^*) \leq f_j (x).  
\end{align*}
Then we derive that $\forall x \in [0, 1]^n, x \not= x^*$, $f(x^*) < f(x)$ and $x$ is the unique optimal solution to $\min_{x \in [0, 1]^n} f (x)$.
\end{proof}

\begin{lem}
\label{lem:n_vars_opt_greedy_structure}
Consider the optimization problem $\min_{x_1, \cdots, x_n} f (x_1, \cdots, x_n)$. Suppose that $x^* = (x^*_1, \cdots, x^*_n)$ is the optimal solution, then $\forall i \in [n]$, $x^*_i$ is the optimal solution to $\min_{x_i} F (x_i) := f (x^*_1, \cdots, x_i, \cdots, x^*_n)$. 
\end{lem}

\begin{proof}
The proof is based on contradiction. Suppose that the original statement is not true. There exists $\widetilde{x}_i \not= x^*_i$ such that
\begin{align*}
    F (\widetilde{x}_i) < F (x^*_i). 
\end{align*}
Consider $\widetilde{x} = (x^*_1, \cdots,\widetilde{x}_i, \cdots, x^*_n)$ which differs from $x^*$ on the $i$-th component. Then we have that
\begin{align*}
    f (x^*_1, \cdots,\widetilde{x}_i, \cdots, x^*_n) = F (\widetilde{x}_i) < F (x^*_i) = f (x^*_1, \cdots, x^*_i, \cdots, x^*_n), 
\end{align*}
which contradicts with the fact that $x^* = (x^*_1, \cdots, x^*_n)$ is the optimal solution to $\min_{x_1, \cdots, x_n} f (x_1, \cdots, x_n)$. Hence, the original statement is true.  
\end{proof}

\begin{lem}
\label{lem:single_variable_opt}
For any constants $a, c \geq 0$, we define the function $f(x) = \vert c - ax \vert - ax$. Consider the optimization problem $\min_{x \in [0, 1]} f(x) $, then $x^* = 1$ is the optimal solution. 
\end{lem}

\begin{proof}
We assume that $x^* = 1$ is not the optimal solution. There exists $\widetilde{x}^* \in [0, 1)$ such that $f(\widetilde{x}^*) < f (x^*)$. That is
\begin{align*}
    \vert c - a\widetilde{x}^* \vert - a\widetilde{x}^* - \vert c - a \vert + a < 0, 
\end{align*}
which implies that $\vert c - a \vert - \vert c - a\widetilde{x}^* \vert > a - a \widetilde{x}^*$. On the other hand, according to the inequality that $\labs p \rabs - \labs q \rabs \leq \labs p-q \rabs$ for $p, q \in \reals$, we have
\begin{align*}
    \vert c - a \vert - \vert c - a\widetilde{x}^* \vert \leq \vert a\widetilde{x}^* - a \vert = a- a\widetilde{x}^*,
\end{align*}
where the last equality follows that $\widetilde{x}^* < 1$. We construct a contradiction. Therefore, the original statement is true.

\end{proof}

\begin{lem}
\label{lem:single_variable_opt_condition}
For any constants $a, c > 0$, we define the function $f(x) = \vert c - ax \vert - ax$. Consider the optimization problem $\min_{x \in [0, 1]} f(x) $, If $x^*$ is the optimal solution, then $x^* > 0$. Furthermore, if $c < a$, then the optimal solutions are $x^* \in [c/a, 1]$.  
\end{lem}

\begin{proof}
To begin with, we prove the first statement. The proof is based on contradiction. We assume that $x = 0$ is the optimal solution. We compare the function value on $x=1$ and $x=0$.
\begin{align*}
    f (0) - f(1) &= c +a - \labs c-a \rabs > 0,
\end{align*}
where the strict inequality follows that $a, c>0$. We obtain that $f(1) < f(0)$, which contradicts with the assumption that $x=0$ is the optimal solution. Therefore, the original statement is true and we finish the proof.

Then we prove the second statement. It is easy to see that
\begin{align*}
    f (x) = \begin{cases}
      c-2ax & x \in [0, \frac{c}{a}), \\
      -c & x \in [\frac{c}{a}, 1].
    \end{cases}
\end{align*}
$f(x)$ is continuous piece-wise linear function. $f(x)$ is strictly decreasing when $x \in [0, c / a)$ and is constant when $x \in [c / a, 1]$. Therefore, we can get that the optimal solutions are $x^* \in [c / a, 1]$. 
\end{proof}

\begin{lem}
\label{lem:single_variable_regularity}
For any constants $a > 0$ and $c \geq 0$, we define the function $f(x) = \vert c - ax \vert - ax$. For any $x \leq \min\{ c/a, 1 \}$, we have $f(x) - f(1) = 2 a ( \min\{ c/a, 1 \} - x)$. 
\end{lem}

\begin{proof}
We consider two cases: $c \geq a$ and $c < a$. When $c \geq a$, the function $f (x)$ at $[0, 1]$ is formulated as $f(x) = c - 2ax$. For any $x \leq \min\{ c/a, 1 \} = 1 $, $f(x) - f(1) = 2a (1-x) = 2 a ( \min\{ c/a, 1 \} - x)$. On the other hand, when $c < a$, the function $f (x)$ at $[0, 1]$ is formulated as
\begin{align*}
    f(x) = \begin{cases}
      c-2ax & x \in [0, \frac{c}{a}), \\
      -c & x \in [\frac{c}{a}, 1].
    \end{cases}
\end{align*}
For any $x \leq \min\{ c/a, 1 \} = c/a$, $f(x) - f(1) = 2 a (c/a-x) = 2 a ( \min\{ c/a, 1 \} - x) $. Therefore, we finish the proof.
\end{proof}

\begin{lem}
\label{lem:mn_variables_opt_unique}
Consider that $A = (a_{ij}) \in \reals^{m \times n}, c \in \reals^{m}, d \in \reals^{n}$ where $a_{ij} > 0$, $\sum_{i=1}^m c_i \geq \sum_{i=1}^m \sum_{j=1}^n a_{ij}$ and for each $j \in [n]$, $\sum_{i=1}^m a_{ij} = d_j$. Consider the following optimization problem:
\begin{align*}
    \min_{x \in [0, 1]^n}f (x) := \lnorm c - A x \rnorm_{1} - d^{\top} x = \sum_{i=1}^m \labs c_i - \sum_{j=1}^n a_{ij} x_j \rabs - \sum_{j=1}^n d_j x_j.
\end{align*}
Then $x^* = \mathbf{1}$ is the unique optimal solution, where $\mathbf{1}$ is the vector that each element is 1. 
\end{lem}

\begin{proof}
For $x = (x_1, \cdots, x_n)$, the function $f(x)$ is formulated as
\begin{align*}
    f (x) = \sum_{i=1}^m \labs c_i - \sum_{j=1}^n a_{ij} x_j \rabs - \sum_{j=1}^n d_j x_j.
\end{align*}
The proof is based on contradiction. We assume that the original statement is not true and there exists $x = (x_1, \cdots, x_n) \not= \mathbf{1}$ such that $x$ is the optimal solution. Let $k \in [n]$ denote some index where $x_k \not= 1$. We construct $\widetilde{x} = \lp \widetilde{x}_1, \cdots, \widetilde{x}_n  \rp \in [0, 1]^n$ in the following way.
\begin{align*}
    \widetilde{x}_j = x_j, \forall j \in [n] \setminus \{k\}, \quad \widetilde{x}_k = 1. 
\end{align*}
We compare the function value of $x$ and $\widetilde{x}$.
\begin{align*}
    f(\widetilde{x}) - f(x) &= \sum_{i=1}^m \lp \labs c_i - \sum_{j=1}^n a_{ij} \widetilde{x}_j \rabs - \labs c_i - \sum_{j=1}^n a_{ij} x_j  \rabs  \rp - d_k (1-x_k)
    \\
    &< \sum_{i=1}^m \lp a_{ik} (1-x_k) \rp - d_k (1-x_k) = 0.
\end{align*}
Here the strict inequality follows the statement that there exists $i^* \in [m]$ such that
\begin{align*}
    \labs c_{i^*} - \sum_{j=1}^n a_{i^* j} \widetilde{x}_j \rabs - \labs c_{i^*} - \sum_{j=1}^n a_{i^* j} x_j  \rabs  <  \labs \lp c_{i^*} - \sum_{j=1}^n a_{i^* j} \widetilde{x}_j \rp - \lp c_{i^*} - \sum_{j=1}^n a_{i^* j} x_j \rp  \rabs=  a_{i^* k} (1-x_k).
\end{align*}
We will prove this statement later. As for $i \in [m], i \not= i^*$, with the inequality that $\labs a \rabs - \labs b \rabs \leq \labs a-b \rabs$ for $a, b \in \reals$, we obtain that
\begin{align*}
    \labs c_i - \sum_{j=1}^n a_{ij} \widetilde{x}_j \rabs - \labs c_i - \sum_{j=1}^n a_{ij} x_j  \rabs  \leq \labs \lp c_i - \sum_{j=1}^n a_{ij} \widetilde{x}_j \rp - \lp c_i - \sum_{j=1}^n a_{ij} x_j \rp  \rabs=  a_{ik} (1-x_k) .
\end{align*}
Hence the strict inequality holds and we construct $\widetilde{x}$ such that $f(\widetilde{x}) < f(x) $, which contradicts with the assumption that $x$ is the optimal solution. Therefore, we prove that the original statement is true and finish the proof.

Now we proceed to prove the statement that there exists $i^* \in [m]$ such that
\begin{align*}
    \labs c_{i^*} - \sum_{j=1}^n a_{i^* j} \widetilde{x}_j \rabs - \labs c_{i^*} - \sum_{j=1}^n a_{i^* j} x_j  \rabs  <  \labs \lp c_{i^*} - \sum_{j=1}^n a_{i^* j} \widetilde{x}_j \rp - \lp c_{i^*} - \sum_{j=1}^n a_{i^* j} x_j \rp  \rabs
\end{align*}
We also prove this statement by contradiction. We assume that for all $i \in [m]$,
\begin{align*}
    \labs c_i - \sum_{j=1}^n a_{ij} \widetilde{x}_j \rabs - \labs c_i - \sum_{j=1}^n a_{ij} x_j  \rabs  \geq \labs \lp c_i - \sum_{j=1}^n a_{ij} \widetilde{x}_j \rp - \lp c_i - \sum_{j=1}^n a_{ij} x_j \rp  \rabs
\end{align*}
According to the inequality that $\labs a \rabs - \labs b \rabs \leq \labs a-b \rabs$ for $a, b \in \reals$, we have
\begin{align*}
    \forall i \in [m], \labs c_i - \sum_{j=1}^n a_{ij} \widetilde{x}_j \rabs - \labs c_i - \sum_{j=1}^n a_{ij} x_j  \rabs  = \labs \lp c_i - \sum_{j=1}^n a_{ij} \widetilde{x}_j \rp - \lp c_i - \sum_{j=1}^n a_{ij} x_j \rp  \rabs
\end{align*}
Furthermore, consider the inequality $\labs a \rabs - \labs b \rabs \leq \labs a-b \rabs$ for $a, b \in \reals$. Notice that the equality holds iff $(b-a) b \leq 0$. Hence we have that
\begin{align*}
     \forall i \in [m], \lp a_{ik} (1-x_k)  \rp  \lp  c_i - \sum_{j=1}^n a_{ij} x_j \rp   \leq 0. 
\end{align*}
Since $\lp a_{ik} (1-x_k)  \rp > 0$, we obtain that
\begin{align*}
    \forall i \in [m], c_i - \sum_{j=1}^n a_{ij} x_j \leq 0. 
\end{align*}
This implies that
\begin{align*}
    \sum_{i=1}^m c_i \leq \sum_{i=1}^m \sum_{j=1}^n a_{ij} x_j < \sum_{i=1}^m \sum_{j=1}^n a_{ij} \leq \sum_{i=1}^m c_i,  
\end{align*}
where the strict inequality follows that $x_k < 1$ and $a_{ij} > 0$. The last inequality follows the assumption of \cref{lem:mn_variables_opt_unique}. Here we find a contradiction that $\sum_{i=1}^m c_i < \sum_{i=1}^m c_i$ and hence the original statement is true.
\end{proof}

\begin{lem}
\label{lem:mn_variables_opt_regularity}
Under the same conditions in \cref{lem:mn_variables_opt_unique}, for any $x \in [0,1]^{n}$, we have that
\begin{align*}
    f (x) - f(x^*) \geq \sum_{j=1}^n \min_{i \in [m]} \{a_{ij} \} (1-x_{j}),
\end{align*}
where $x^* = \mathbf{1}$, which is the vector that each element is 1. 
\end{lem}

\begin{proof}
Recall that $f (x) = \sum_{i=1}^m \vert c_i - \sum_{j=1}^n a_{ij} x_j \vert - \sum_{j=1}^n d_j x_j$. We first claim that when $x \in [0, 1]^n$, $c_i - \sum_{j=1}^n a_{ij} x_j < 0$ does not hold simultaneously for all $i \in [m]$. We prove this claim via contradiction. Assume that there exists $x \in [0, 1]^n$ such that $c_i - \sum_{j=1}^n a_{ij} x_j < 0, \forall i \in [m]$. Then we have that
\begin{align*}
    \sum_{i=1}^m c_i < \sum_{i=1}^m \sum_{j=1}^n a_{ij} x_j \overset{(1)}{\leq} \sum_{i=1}^m \sum_{j=1}^n a_{ij} \overset{(2)}{\leq} \sum_{i=1}^m c_i.   
\end{align*}
The inequality $(1)$ follows that $A > 0$ and $x \in [0, 1]^n$ and the inequality $(2)$ follows that original assumption of \cref{lem:mn_variables_opt_regularity}. Thus we constructs a contradiction, which implies that the original claim is true.

Let $x_{p:q}$ be the shorthand of $(x_p, x_{p+1}, \cdots, x_{q})$ for any $1 \leq p \leq q \leq n$. With telescoping, we have that
\begin{align*}
    f(x) - f(x^*) = \sum_{j=1}^n f(x^*_{1:j-1}, x_{j:n}) - f(x^*_{1:j}, x_{j+1:n}).
\end{align*}
Note that $f(x^*_{1:j-1}, x_{j:n}) $ and $f(x^*_{1:j}, x_{j+1:n})$ only differ in the $j$-th variable. For each $j \in [n]$, with fixed $x^*_1, \cdots, x^*_{j-1}, x_{j+1}, \cdots, x_n \in [0, 1]$, we define one-variable function $F_j (t) = f (x^*_{1:j-1}, t, x_{j+1:n}), \forall t \in [0, 1]$. Notice that $F_j (t)$ is also a continuous piece-wise linear function.

On the one hand, $F_j (t)$ is differentiable at any interior point $t_0$ and it holds that 
\begin{align*}
    F_j^\prime (t_0) = -d_j + \sum_{i=1}^m \indict \lb \lp c_i - \sum_{k=1}^{j-1} a_{ik} x^*_k - a_{ij} t_0 - \sum_{k=j+1}^n a_{ik} x_k \rp < 0  \rb a_{ij} \leq - \min_{i \in [m]} \{ a_{ij} \}.
\end{align*}

The last inequality follows that $\forall x \in [0, 1]^n, c_i - \sum_{j=1}^n a_{ij} x_j \leq 0$ does not hold simultaneously for all $i \in [m]$ and $d_j = \sum_{i=1}^m a_{ij}$. On the other hand, the number of boundary points of $F_j (t)$ is $m$ at most. Let $b_j^1, b_j^2, \cdots, b_j^{n_j}$ denote the boundary point of $F_j (t)$ when $t \in [x_j, x_j^*]$. With fundamental theorem of calculus, we have that
\begin{align*}
   f(x) - f(x^*) &= \sum_{j=1}^n f(x^*_{1:j-1}, x_{j:n}) - f(x^*_{1:j}, x_{j+1:n})
   \\
   &= \sum_{j=1}^n F_j (x_j) - F_j (x_j^*)
   \\
   &= \sum_{j=1}^n \lp F_j (x_j) - F_j (b_j^1) + \sum_{k=1}^{n_j-1} F_j (b_j^k) - F_j (b_j^{k+1}) + F_j (b_j^{n_j}) - F(x_j^*)   \rp  
   \\
   &= - \sum_{j=1}^n \lp \int_{x_j}^{b_j^1} F_j^\prime (t) dt + \sum_{k=1}^{n_j-1} \int_{b_j^k}^{b_j^{k+1}} F_j^\prime (t) dt + \int_{b_j^{n_j}}^{x_j^*} F_j^\prime (t) dt    \rp 
   \\
   &\geq  \sum_{j=1}^n \min_{i \in [m]} \{ a_{ij} \} \lp x_j^* - x_j  \rp =  \sum_{j=1}^n \min_{i \in [m]} \{ a_{ij}\} \lp 1 - x_j  \rp.
\end{align*}

\end{proof}

\subsection{Proof of Technical Lemmas in Appendix \ref{appendix:proof_generalization_ail}, \ref{appendix:proof_beyond_vanilla_ail}, and \ref{appendix:discussion} }

\subsubsection{Proof of Lemma \ref{lemma:regret_of_ogd}}
\label{appendix:proof_lemma_regret_of_ogd}
\begin{proof}

Lemma \ref{lemma:regret_of_ogd} is a direct consequence of the regret bound of online gradient descend \citep{shalev12online-learning}. To apply such a regret bound, we need to verify that 1) the iterate norm $\lnorm w \rnorm_2$ has an upper bound; 2) the gradient norm $\Vert \nabla_{w}  f^{(t)}(w) \Vert_2$ also has an upper bound. The first point is easy to show, i.e., $\lnorm w \rnorm_2 \leq \sqrt{H |\gS| |\gA|}$ by the condition that $w \in \gW = \{ w: \Vert w \Vert_{\infty} \leq 1 \}$. For the second point, let $\widetilde{P}^{1}_h$ and $\widetilde{P}^{2}_h$ be the first and the second part in $\widetilde{P}^{\piE}_h$ defined in \eqref{eq:new_estimator}. Then, 
\begin{align*}
    \lnorm \nabla_{w} f^{(t)} (w) \rnorm_{2} &= \sqrt{\sum_{h=1}^H \sum_{(s, a) \in \gS \times \gA} \lp P^{\pi^{(t)}}_h (s, a) - \widetilde{P}^{\piE}_h (s, a) \rp^2 }
    \\
    &= \sqrt{\sum_{h=1}^H \sum_{(s, a) \in \gS \times \gA} \lp P^{\pi^{(t)}}_h (s, a) - \widetilde{P}^{1}_h(s, a) - \widetilde{P}^{2}_h(s, a) \rp^2 } 
    \\
    &\leq \sqrt{\sum_{h=1}^H  3 \sum_{(s, a) \in \gS \times \gA}   \lp P^{\pi^{(t)}}_h (s, a) \rp^2 + \lp \widetilde{P}^{1}_h(s, a) \rp^2 + \lp \widetilde{P}^{2}_h(s, a)  \rp^2 }
    \\
     &\leq \sqrt{\sum_{h=1}^H  3  \lp \lnorm P^{\pi^{(t)}}_h \rnorm_1 + \lnorm \widetilde{P}^{1}_h \rnorm_1 + \lnorm \widetilde{P}^{2}_h \rnorm_1  \rp }
    \\
    &\leq 2\sqrt{ H },
\end{align*}
where the first inequality follows $(a+b+c)^2 \leq 3(a^2+b^2+c^2)$ and the second inequality is based on that $ x ^2 \leq \vert x \vert$ if $0 \leq x \leq 1$.

Invoking Corollary 2.7 in \citep{shalev12online-learning} with $B = \sqrt{H |\gS| |\gA|}$ and $L = 2 \sqrt{H}$ finishes the proof. 
\end{proof}

\subsubsection{Proof of Lemma \ref{lemma:approximate-minimax}}
\label{appendix:proof_lemma_approximate_minimax}

\begin{proof}
With the dual representation of $\ell_1$-norm, we have
\begin{align*}
    \min_{\pi \in \Pi} \sum_{h=1}^H \lnorm P^{\pi}_h - \widetilde{P}^{\piE}_h \rnorm_{1} = \min_{\pi \in \Pi} \max_{w \in \gW} \sum_{h=1}^H \sum_{(s, a) \in \gS \times \gA} w_{h} (s, a) \lp \widetilde{P}^{\piE}_h(s, a) - P^{\pi}_h (s, a) \rp. 
\end{align*}
Since the above objective is linear w.r.t both $w$ and $P^\pi_h$, invoking the minimax theorem \citep{bertsekas2016nonlinear} yields
\begin{align*}
    &\quad \min_{\pi \in \Pi} \max_{w \in \gW} \sum_{h=1}^H \sum_{(s, a) \in \gS \times \gA} w_{h} (s, a) \lp \widetilde{P}^{\piE}_h(s, a) - P^{\pi}_h (s, a) \rp
    \\
    &= \max_{w \in \gW} \min_{\pi \in \Pi} \sum_{h=1}^H \sum_{(s, a) \in \gS \times \gA} w_{h} (s, a) \lp \widetilde{P}^{\piE}_h(s, a) - P^{\pi}_h (s, a) \rp
    \\
    &= - \min_{w \in \gW} \max_{\pi \in \Pi} \sum_{h=1}^H \sum_{(s, a) \in \gS \times \gA} w_h (s, a) \lp P^{\pi}_h (s, a) -  \widetilde{P}^{\piE}_h(s, a) \rp, 
\end{align*}
where the last step follows the property that for a function $f$, $- \max_{x} f(x) = \min_{x} - f(x)$. Therefore, we have
\begin{align} \label{eq:l1_dual_representation}
    \min_{\pi \in \Pi} \sum_{h=1}^H \lnorm P^{\pi}_h  - \widetilde{P}^{\piE}_h \rnorm_{1} = - \min_{w \in \gW} \max_{\pi \in \Pi} \sum_{h=1}^H \sum_{(s, a) \in \gS \times \gA} w_h (s, a) \lp P^{\pi}_h (s, a) -  \widetilde{P}^{\piE}_h(s, a) \rp.
\end{align}
Then we consider the term $\min_{w \in \gW} \max_{\pi \in \Pi} \sum_{h=1}^H \sum_{(s, a) \in \gS \times \gA} w_h (s, a) \lp P^{\pi}_h (s, a) -  \widetilde{P}^{\piE}_h(s, a) \rp$.
\begin{align*}
    &\quad \min_{w \in \gW} \max_{\pi \in \Pi} \sum_{h=1}^H \sum_{(s, a) \in \gS \times \gA} w_h (s, a) \lp P^{\pi}_h (s, a) -  \widetilde{P}^{\piE}_h(s, a) \rp
    \\
    &\leq \max_{\pi \in \Pi} \sum_{h=1}^H \sum_{(s, a) \in \gS \times \gA} \lp \frac{1}{T} \sum_{t=1}^T w^{(t)}_h (s, a) \rp \lp P^{\pi}_h (s, a) -  \widetilde{P}^{\piE}_h(s, a) \rp
    \\
    &\leq \frac{1}{T} \sum_{t=1}^T \max_{\pi \in \Pi} \sum_{h=1}^H \sum_{(s, a) \in \gS \times \gA} w^{(t)}_h (s, a) \lp P^{\pi}_h (s, a) -  \widetilde{P}^{\piE}_h(s, a) \rp. 
\end{align*}
At iteration $t$, $\pi^{(t)}$ is the approximately optimal policy regarding reward function $w^{(t)}$ with an optimization error of $\varepsilon_{\mathrm{opt}}$. Then we obtain that
\begin{align*}
    &\quad \frac{1}{T} \sum_{t=1}^T \max_{\pi \in \Pi} \sum_{h=1}^H \sum_{(s, a) \in \gS \times \gA} w^{(t)}_h (s, a) \lp P^{\pi}_h (s, a) -  \widetilde{P}^{\piE}_h(s, a) \rp
    \\
    &\leq \frac{1}{T} \sum_{t=1}^T \sum_{h=1}^H \sum_{(s, a) \in \gS \times \gA} w^{(t)}_h (s, a) \lp P^{\pi^{(t)}}_h (s, a) -  \widetilde{P}^{\piE}_h(s, a) \rp + \varepsilon_{\mathrm{opt}}.
\end{align*}
Applying Lemma \ref{lemma:regret_of_ogd} yields that
\begin{align*}
    &\quad \frac{1}{T} \sum_{t=1}^T \sum_{h=1}^H \sum_{(s, a) \in \gS \times \gA} w^{(t)}_h (s, a) \lp P^{\pi^{(t)}}_h (s, a) -  \widetilde{P}^{\piE}_h(s, a) \rp
    \\
    & \leq \min_{w \in \gW} \frac{1}{T} \sum_{t=1}^T \sum_{h=1}^H \sum_{(s, a) \in \gS \times \gA} w_h (s, a) \lp P^{\pi^{(t)}}_h (s, a) -  \widetilde{P}^{\piE}_h(s, a) \rp + 2H \sqrt{ \frac{2 |\gS| |\gA|}{T} }
    \\
    &= \min_{w \in \gW}  \sum_{h=1}^H \sum_{(s, a) \in \gS \times \gA} w_h (s, a) \lp \frac{1}{T} \sum_{t=1}^T P^{\pi^{(t)}}_h (s, a) -  \widetilde{P}^{\piE}_h(s, a) \rp + 2H \sqrt{ \frac{2 |\gS| |\gA|}{T} }
    \\
    &= \min_{w \in \gW}  \sum_{h=1}^H \sum_{(s, a) \in \gS \times \gA} w_h (s, a) \lp P^{\widebar{\pi}}_h (s, a) -  \widetilde{P}^{\piE}_h(s, a) \rp + 2H \sqrt{ \frac{2 |\gS| |\gA|}{T} }.
\end{align*}
Note that $\widebar{\pi}$ is induced by the mean state-action distribution, i.e., $\widebar{\pi}_h (a|s) = \widebar{P}_h(s, a) / \sum_{a} \widebar{P}_h(s, a)$, where $\widebar{P}_h (s, a) = {1}/{T} \cdot \sum_{t=1}^T P^{\pi^{(t)}}_h (s, a)$. Based on Proposition 3.1 in \citep{ho2016gail}, we have that $P^{\widebar{\pi}}_h (s, a) = \widebar{P}_h (s, a)$, and hence the last equation holds. Combined with \eqref{eq:l1_dual_representation}, we have that
\begin{align*}
    &\quad \min_{\pi \in \Pi} \sum_{h=1}^H \lnorm P^{\pi}_h - \widetilde{P}^{\piE}_h \rnorm_{1}
    \\
    &\geq - \min_{w \in \gW}  \sum_{h=1}^H \sum_{(s, a) \in \gS \times \gA} w_h (s, a) \lp P^{\widebar{\pi}}_h (s, a) -  \widetilde{P}^{\piE}_h(s, a) \rp - 2H \sqrt{ \frac{2 |\gS| |\gA|}{T} } - \varepsilon_{\mathrm{opt}}
    \\
    &= \max_{w \in \gW} \sum_{h=1}^H \sum_{(s, a) \in \gS \times \gA} w_h (s, a) \lp  \widetilde{P}^{\piE}_h(s, a) - P^{\widebar{\pi}}_h (s, a)  \rp - 2H \sqrt{ \frac{2 |\gS| |\gA|}{T} } - \varepsilon_{\mathrm{opt}}
    \\
    &= \sum_{h=1}^H \lnorm \widetilde{P}^{\piE}_h - P^{\widebar{\pi}}_h \rnorm_{1} - 2H \sqrt{ \frac{2 |\gS| |\gA|}{T}} - \varepsilon_{\mathrm{opt}},
\end{align*}
where the last step again utilizes the dual representation of $\ell_1$-norm. We complete the proof.

\end{proof}

\subsubsection{Proof of Lemma \ref{lemma:sample_complexity_of_new_estimator_known_transition}}
\label{appendix:proof_lemma_sample_complexity_of_new_estimator_known_transition}

\begin{proof}
Recall the definition of the estimator $\widetilde{P}_h^{\piE}$
\begin{align*} 
\widetilde{P}_h^{\piE}  (s, a) =   { \sum_{\tr_h \in \Tr_h^{\gD_1} } \sP^{\piE}(\tr_h) \indict\lb \tr_h(s_h, a_h) = (s, a)\rb} + {\frac{  \sum_{\tr_h \in \gD_1^c}  \indict\{ \tr_h (s_h, a_h) = (s, a), \tr_h \not\in \Tr_h^{\gD_1}  \} }{|\gD_1^c|}}.
\end{align*}
Our target is to upper bound the estimation error of $\widetilde{P}_h^{\piE} \in \real^{|\gS| \times |\gA|}$:
\begin{align*}
    \sum_{h=1}^H \lnorm \widetilde{P}^{\piE}_h - P^{\piE}_h  \rnorm_{1} = \sum_{h=1}^{H} \sum_{(s, a) \in \gS \times \gA} \labs \widetilde{P}_h^{\pi_E}(s, a) - P_h^{\piE}(s, a) \rabs,
\end{align*}
where $\widetilde{P}_h^{\piE}$ is defined in \eqref{eq:new_estimator}:
\begin{align*}
  \widetilde{P}_h^{\piE}(s, a) =   { \sum_{\tr_h \in \Tr_h^{\gD_1} } \sP^{\piE}(\tr_h) \indict\lb \tr_h(s_h, a_h) = (s, a)\rb}  + {\frac{  \sum_{\tr_h \in \gD_1^c}  \indict\{ \tr_h (s_h, a_h) = (s, a), \tr_h \not\in \Tr_h^{\gD_1}  \} }{|\gD_1^c|}}.
\end{align*}
Recall that $\Tr_h^{\gD_1}$ is the set of trajectories along which each state has been visited in $\gD_1$ up to time step $h$. Similarly, for $P_h^{\piE}$, we have the following decomposition in \eqref{eq:key_decomposition}:
\begin{align*}
    P_h^{\piE}(s, a) = \sum_{\tr_h \in \Tr_h^{\gD_1}} \sP^{\piE}(\tr_h) \indict\lb  \tr_h (s_h, a_h) = (s, a)  \rb + \sum_{\tr_h \notin \Tr_h^{\gD_1}} \sP^{\piE}(\tr_h) \indict\lb  \tr_h (s_h, a_h) = (s, a)  \rb.
\end{align*}

Consequently, we obtain for any $(s, a) \in \gS \times \gA, h \in [H]$, 
\begin{align}
     &\quad  \labs \widetilde{P}_h^{\pi_E}(s, a) - P_h^{\piE}(s, a) \rabs \nonumber \\
     &=   \labs \widetilde{P}_h^{\pi_E}(s, a) - \lp \sum_{\tr_h \in \Tr_h^{\gD_1}} \sP^{\piE}(\tr_h) \indict\lb  \tr_h (s_h, a_h) = (s, a)  \rb + \sum_{\tr_h \notin \Tr_h^{\gD_1}} \sP^{\piE}(\tr_h) \indict\lb  \tr_h (s_h, a_h) = (s, a)  \rb \rp  \rabs \nonumber \\
     &= \labs \frac{  \sum_{\tr_h \in \gD_1^c}  \indict\{ \tr_h (s_h, a_h) = (s, a), \tr_h \not\in \Tr_h^{\gD_1}  \} }{|\gD_1^c|} - \sum_{\tr_h \notin \Tr_h^{\gD_1}} \sP^{\piE}(\tr_h) \indict\lb  \tr_h (s_h, a_h) = (s, a)  \rb  \rabs, \label{eq:new_estimation_probability_error}
\end{align}
where the last equation is based on the fact that the first term in $\widetilde{P}_h^{\pi_E}(s, a)$ and $P_h^{\piE}(s, a)$ is identical. As a result, the estimation error is caused by the unknown expert actions in trajectories that does not fully match with any trajectory in $\gD_1$. Then we obtain that
\begin{align*}
    &\quad \sum_{h=1}^H \lnorm \widetilde{P}^{\piE}_h - P^{\piE}_h  \rnorm_{1}
    \\
    &\leq \sum_{h=1}^H \sum_{(s, a) \in \gS \times \gA} \labs \frac{  \sum_{\tr_h \in \gD_1^c}  \indict\{ \tr_h (s_h, a_h) = (s, a), \tr_h \not\in \Tr_h^{\gD_1}  \} }{|\gD_1^c|} - \sum_{\tr_h \notin \Tr_h^{\gD_1}} \sP^{\piE}(\tr_h) \indict\lb  \tr_h (s_h, a_h) = (s, a)  \rb  \rabs. 
\end{align*}
Next, we invoke Lemma A.12 in \cite{rajaraman2020fundamental} to upper bound the term in RHS. 
\begin{lem}[Lemma A.12 in \cite{rajaraman2020fundamental}]
Fix $\delta \in (0, \min\{1, H/5 \})$, with probability at least $1-\delta$,
\begin{align*}
    & \quad \sum_{h=1}^H \sum_{(s, a) \in \gS \times \gA} \labs \frac{  \sum_{\tr_h \in \gD_1^c}  \indict\{ \tr_h (s_h, a_h) = (s, a), \tr_h \not\in \Tr_h^{\gD_1}  \} }{|\gD_1^c|} - \sum_{\tr_h \notin \Tr_h^{\gD_1}} \sP^{\piE}(\tr_h) \indict\lb  \tr_h (s_h, a_h) = (s, a)  \rb  \rabs
    \\
    &\precsim \frac{\vert \gS \vert H^{3/2}}{m} \lp 1 + \frac{3 \log \lp 2 \vert \gS \vert H / \delta \rp}{\sqrt{\vert \gS \vert}} \rp \sqrt{\log \lp \frac{2 \vert \gS \vert H}{\delta} \rp}. 
\end{align*}
\end{lem}

Then, for any fixed $\delta \in (0, \min\{1, H/5 \})$, with probability at least $1-\delta$,
\begin{align*}
    \sum_{h=1}^H \lnorm \widetilde{P}^{\piE}_h - P^{\piE}_h  \rnorm_{1} \leq \frac{\vert \gS \vert H^{3/2}}{m} \lp 1 + \frac{3 \log \lp 2 \vert \gS \vert H / \delta \rp}{\sqrt{\vert \gS \vert}} \rp \sqrt{\log \lp \frac{2 \vert \gS \vert H }{\delta} \rp}, 
\end{align*}
When $m \succsim \vert \gS \vert H^{3/2} \log \lp H \vert \gS \vert / \delta \rp / \varepsilon$, we have that $\sum_{h=1}^H \Vert \widetilde{P}^{\piE}_h - P^{\piE}_h  \Vert_{1} \leq \varepsilon$. 

\end{proof}

\subsubsection{Proof of Lemma \ref{lemma:sample_complexity_of_new_estimator_unknown_transition}}
\label{appendix:proof_lemma_sample_complexity_of_new_estimator_unknown_transition}

\begin{proof}
We aim to upper bound the estimation error.
\begin{align*}
    \sum_{h=1}^H \lnorm \widetilde{P}^{\piE}_h - P^{\piE}_h  \rnorm_{1}.
\end{align*}
Recall the definition of the estimator $\widetilde{P}^{\piE}_h(s, a)$.
\begin{align*}
    \widetilde{P}_h^{\piE} (s, a) := \frac{\sum_{\tr_h \in \gD^\prime_{\mathrm{env}}} \indict \lb \tr_h (s_h, a_h) = (s, a), \tr_h \in \Tr_h^{\gD_1} \rb }{ | \gD^\prime_{\mathrm{env}} |} + \frac{\sum_{\tr_h \in \gD_1^{c}} \indict \lb \tr_h (s_h, a_h) = (s, a), \tr_h \notin \Tr_h^{\gD_1} \rb}{| \gD_1^{c} |}.
\end{align*}

Similarly, we utilize the decomposition of $P_h^{\piE}(s, a)$ as we have done in the proof of Lemma \ref{lemma:sample_complexity_of_new_estimator_known_transition}.  
\begin{align*}
    P_h^{\piE}(s, a) = \sum_{\tr_h \in \Tr_h^{\gD_1}} \sP^{\piE}(\tr_h) \indict\lb  \tr_h (s_h, a_h) = (s, a)  \rb + \sum_{\tr_h \notin \Tr_h^{\gD_1}} \sP^{\piE}(\tr_h) \indict\lb  \tr_h (s_h, a_h) = (s, a)  \rb.
\end{align*}
Then, for any $h \in [H]$ and $(s, a) \in \gS \times \gA$, we have
\begin{align*}
    &\quad \labs \widetilde{P}^{\piE}_h(s, a) - P^{\piE}_h (s, a)  \rabs
    \\
    &\leq \labs \frac{\sum_{\tr_h \in \gD^\prime_{\mathrm{env}}} \indict \lb \tr_h (s_h, a_h) = (s, a), \tr_h \in \Tr_h^{\gD_1} \rb }{ | \gD^\prime_{\mathrm{env}} |} - \sum_{\tr_h \in \Tr_h^{\gD_1}} \sP^{\piE}(\tr_h) \indict\lb  \tr_h (s_h, a_h) = (s, a)  \rb  \rabs 
    \\
    & \quad + \labs \frac{\sum_{\tr_h \in \gD_1^{c}} \indict \lb \tr_h (s_h, a_h) = (s, a), \tr_h \notin \Tr_h^{\gD_1} \rb}{| \gD_1^{c} |} - \sum_{\tr_h \notin \Tr_h^{\gD_1}} \sP^{\piE}(\tr_h) \indict\lb  \tr_h (s_h, a_h) = (s, a)  \rb  \rabs .
\end{align*}
Thus, we can upper bound the estimation error.
\begin{align*}
    &\quad \sum_{h=1}^H \lnorm \widetilde{P}^{\piE}_h - P^{\piE}_h  \rnorm_{1}
    \\
    &\leq \underbrace{\sum_{h=1}^H \sum_{(s, a) \in \gS \times \gA} \labs \frac{\sum_{\tr_h \in \gD^\prime_{\mathrm{env}}} \indict \lb \tr_h (s_h, a_h) = (s, a), \tr_h \in \Tr_h^{\gD_1} \rb }{ | \gD^\prime_{\mathrm{env}} |} - \sum_{\tr_h \in \Tr_h^{\gD_1}} \sP^{\piE}(\tr_h) \indict\lb  \tr_h (s_h, a_h) = (s, a)  \rb  \rabs}_{\text{Error A}}
    \\
    &\quad + \underbrace{\sum_{h=1}^H \sum_{(s, a) \in \gS \times \gA} \labs \frac{\sum_{\tr_h \in \gD_1^{c}} \indict \lb \tr_h (s_h, a_h) = (s, a), \tr_h \notin \Tr_h^{\gD_1} \rb}{| \gD_1^{c} |} - \sum_{\tr_h \notin \Tr_h^{\gD_1}} \sP^{\piE}(\tr_h) \indict\lb  \tr_h (s_h, a_h) = (s, a)  \rb  \rabs}_{\text{Error B}}. 
\end{align*}
We first analyze the term $\text{Error A}$. Recall that dataset $\gD^\prime_{\mathrm{env}}$ is collected by the policy $\pi \in \Pi_{\text{BC}} \lp \gD_{1} \rp$ with $|\gD^\prime_{\mathrm{env}}| = n^\prime$, and $\sum_{\tr_h \in \gD^\prime_{\mathrm{env}}} \indict \{ \tr_h (s_h, a_h) = (s, a), \tr_h \in \Tr_h^{\gD_1} \} /  | \gD^\prime_{\mathrm{env}} |$ is a maximum likelihood estimator for $\sum_{\tr_h \in \Tr_h^{\gD_1}} \sP^{\piE}(\tr_h) \indict \lb  \tr_h (s_h, a_h) = (s, a)  \rb $. Let ${E^\prime}^{s}_h$ be the event that $\tr_h$ agrees with expert policy at state $s$ in time step $h$ and appears in $\Tr_h^{\gD_1}$. Formally, 
\begin{align*}
    {E^\prime}_h^{s} = \indict\{\tr_h (s_h, a_h) = (s, \piE_h (s)) \cap \tr_h \in \mathbf{Tr}^{\gD_1}_h \}.
\end{align*}
Then we apply Chernoff's bound to upper bound the term $\text{Error A}$.

\begin{lem}[Chernoff's bound \citep{vershynin2018high}]   \label{lemma:chernoff_bound}
Let $\widebar{X} = {1}/{n} \cdot \sum_{i=1}^{n} X_i$, where $X_i$ is a Bernoulli random variable with $\sP(X_i = 1) = p_i$ and $\sP(X_i = 0) = 1 - p_i$ for $i \in [n]$. Furthermore, assume these random variables are independent. Let $\mu = \expect[\widebar{X}] = {1}/{n} \cdot \sum_{i=1}^{n} p_i$. Then for $0 < t \leq 1$, 
\begin{align*}
    \sP\lp  \labs  \widebar{X} - \mu \rabs  \geq t \mu  \rp \leq 2 \exp\lp -\frac{\mu n t^2}{3}  \rp.
\end{align*}
\end{lem}

By Lemma \ref{lemma:chernoff_bound}, for each $s \in \gS$ and $h \in [H]$, with probability at least $1 - \frac{\delta}{2 |\gS| H}$ over the randomness of $\gD ^\prime$, we have
\begin{align*}
    &\quad \labs \frac{\sum_{\tr_h \in \gD^\prime_{\mathrm{env}}} \indict \lb \tr_h (s_h, a_h) = (s, \piE_h(s)), \tr_h \in \Tr_h^{\gD_1} \rb }{ | \gD^\prime_{\mathrm{env}} |}  - \sum_{\tr_h \in \Tr_h^{\gD_1}} \sP^{\piE}(\tr_h) \indict\lb  \tr_h (s_h, a_h) = (s, \piE_h (s))  \rb  \rabs
    \\
    &\leq \sqrt{ \sP^{\piE} \lp {E^\prime}^{s}_h  \rp  \frac{3 \log \lp 4 |\gS| H / \delta \rp}{n^\prime}}.
\end{align*}
By union bound, with probability at least $1-{\delta}/{2}$ over the randomness of $\gD^\prime_{\mathrm{env}}$, we have
\begin{align*}
    \text{Error A} &\leq  \sum_{h=1}^H \sum_{s \in \gS} \sqrt{ \sP^{\piE} \lp {E^\prime}^{s}_h  \rp  \frac{3 \log \lp 4 |\gS| H / \delta \rp}{n^\prime}}
    \\
    &\leq \sum_{h=1}^H \sqrt{|\gS|} \sqrt{\sum_{s \in \gS} \sP^{\piE} \lp {E^\prime}^{s}_h  \rp  \frac{3 \log \lp 4 |\gS| H / \delta \rp}{n^\prime} }
\end{align*}
The last inequality follows the Cauchy-Schwartz inequality. It remains to upper bound $\sum_{s \in \gS}  \sP^{\piE}(E_{h}^{s})$ for all $h \in [H]$. To this end, we define the event ${G^\prime}_h^{\gD_1}$ that expert policy $\piE$ visits states covered in $\gD_1$ up to time step $h$. Formally, ${G^\prime}_h^{\gD_1} = \indict\{ \forall h^{\prime} \leq h,  s_{h^{\prime}} \in \gS_{h^{\prime}} (\gD_1) \}$, where $\gS_{h}(\gD_1)$ is the set of states in $\gD_1$ in time step $h$. Then, for all $h \in [H]$, we have \begin{align*}
    \sum_{s \in \gS} \sP^{\piE} \lp {E^\prime}_h^{s}  \rp = \sP^{\piE}({G^\prime}_h^{\gD_1}) \leq \sP({G^\prime}_1^{\gD_1}).
\end{align*}
The last inequality holds since ${G^\prime}_h^{\gD_1} \subseteq {G^\prime}_1^{\gD_1}$ for all $h \in [H]$. Then we have that
\begin{align*}
    \text{Error A} \leq H \sqrt{\frac{3 |\gS| \log \lp 4 |\gS| H / \delta \rp}{n^\prime}}.
\end{align*}
When the interaction complexity satisfies that $n^\prime \succsim \frac{| \gS | H^{2}}{\varepsilon^2} \log\lp  \frac{|\gS| H}{\delta} \rp$, with probability at least $1-\frac{\delta}{2}$ over the randomness of $\gD^\prime$, we have $\text{Error A} \leq \frac{\varepsilon}{2}$. For the term $\text{Error B}$, we have analyzed it in the proof of Lemma \ref{lemma:sample_complexity_of_new_estimator_known_transition}. When the expert sample complexity satisfies that $m \succsim \frac{|\gS| H^{3/2}}{\varepsilon} \log \lp \frac{|\gS| H}{\delta} \rp$, with probability at least $1-\frac{\delta}{2}$ over the randomness of $\gD$, we have $\text{Error B} \leq \frac{\varepsilon}{2}$. Applying union bound finishes the proof.
\end{proof}

\subsubsection{Proof of Lemma \ref{lemma:ail_policy_ail_objective_equals_expert_policy_ail_objective}}
\label{appendix:proof_lemma:ail_policy_ail_objective_equals_expert_policy_ail_objective}

\begin{proof}
For $h, h^\prime \in [H], h \leq h^\prime$, we use $\pi_{h:h^\prime}$ denote the shorthand of $\lp \pi_h, \pi_{h+1}, \cdots, \pi_{h^\prime} \rp$. From \cref{prop:ail_general_reset_cliff}, we have that $\forall h \in [H-1], s \in \goodS, \piail_{h} (a^{1}|s) = \piE_{h} (a^{1}|s) = 1$. Hence, $\piail$ and $\piE$ never visit bad states. Furthermore, notice that for any time step $h \in [H]$, $\text{Loss}_{h} (\pi)$ only depends on $\pi_{1:h}$. Therefore, we have
\begin{align*}
    \sum_{h=1}^{H-1} \text{Loss}_{h} (\piail) = \sum_{h=1}^{H-1} \text{Loss}_{h} (\piE).
\end{align*}
It remains to prove that $\text{Loss}_{H} (\piail) = \text{Loss}_{H} (\piE)$. From \cref{lem:n_vars_opt_greedy_structure}, fixing $\piail_{1:H-1}$, $\piail_{H}$ is the optimal solution to \textsf{VAIL}'s objective. With fixed $\piail_{1:H-1}$, $\sum_{h=1}^{H-1} \text{Loss}_{h} (\piail)$ is independent of $\piail_{H}$ and thus
\begin{align*}
    \piail_{H} &\in \argmin_{\pi_H}  \text{Loss}_{H} (\piail_{1:H-1}, \pi_H)
    \\
    &=  \argmin_{\pi_H}  \text{Loss}_{H} (\piE_{1:H-1}, \pi_H)
    \\
    &= \argmin_{\pi_H} \sum_{s \in \gS} \sum_{a \in \gA} \labs \widehat{P}^{\piE}_h(s, a) - P^{\piE}_H (s) \pi_H (a|s)  \rabs
    \\
    &= \argmin_{\pi_H} \sum_{s \in \goodS} \labs \widehat{P}^{\piE}_h(s) - P^{\piE}_H (s) \pi_H (a^{1}|s)  \rabs + P^{\piE}_H (s) \lp 1 - \pi_{H} (a^{1}|s) \rp
    \\
    &= \argmin_{\pi_H} \sum_{s \in \goodS} \labs \widehat{P}^{\piE}_h(s) - P^{\piE}_H (s) \pi_H (a^{1}|s)  \rabs - P^{\piE}_H (s) \pi_{H} (a^{1}|s). 
\end{align*}
In the penultimate equality, we use the facts that 1) for each $s \in \goodS$, we have $\widehat{P}^{\piE}_h(s, a^{1}) = \widehat{P}^{\piE}_h(s)$, and $\widehat{P}^{\piE}_h(s, a) = 0, \forall a \in \gA \setminus \{a^{1}\}$; 2) for each $s \in \badS$, $\widehat{P}^{\piE}_h(s) = P^{\piE}_h (s) = 0$. The last equality follows that $P^{\piE}_H (s)$ is independent of $\pi_H$. Since the optimization variables $\pi_H (a^{1}|s)$ for different $s \in \goodS$ are independent, we can view the above optimization problem for each $\pi_H (a^{1}|s)$ individually.
\begin{align*}
    \piail_{H}(a^{1}|s) = \argmin_{\pi_H (a^{1}|s) \in [0, 1]} \labs \widehat{P}^{\piE}_h(s) - P^{\piE}_H (s) \pi_H (a^{1}|s)  \rabs - P^{\piE}_H (s) \pi_{H} (a^{1}|s).
\end{align*}
By \cref{lem:single_variable_opt}, we have that $\piE_H(a^{1}|s) = 1$ is also the optimal solution like $\piail_{H} (a^{1}|s)$. Therefore, we have that 
\begin{align*}
    \text{Loss}_{H} (\piail_{1:H-1}, \piail_H) = \min_{\pi_H} \text{Loss}_{H} (\piail_{1:H-1}, \pi_H)  = \min_{\pi_H} \text{Loss}_{H} (\piE_{1:H-1}, \pi_H) = \text{Loss}_{H} (\piE_{1:H-1}, \piE_H).  
\end{align*}
Finally, we prove that $f (\piail) = f(\piE)$.
\end{proof}

\subsubsection{Proof of Proposition \ref{prop:ail_general_reset_cliff_approximate_solution}}
\label{appendix:proof_prop:ail_general_reset_cliff_approximate_solution}

\begin{proof}
Suppose that $\piail$ is the optimal solution to \eqref{eq:ail}. Since $\widebar{\pi}$ is $\varepsilon_{\ail}$ optimal, we have that
\begin{align*}
    f (\widebar{\pi}) - f(\piail) \leq \varepsilon_{\ail}.
\end{align*}
By \cref{lemma:ail_policy_ail_objective_equals_expert_policy_ail_objective}, it holds that $f(\piail) = f(\piE)$. Furthermore, with the decomposition of $f(\pi)$, we have 
\begin{align}
\label{eq:ail_objective_pi_bar_minus_piE}
    f (\widebar{\pi}) - f(\piail) = f (\widebar{\pi}) - f(\piE) =  \sum_{h=1}^{H} \text{Loss}_{h} (\widebar{\pi}) - \text{Loss}_{h} (\piE) \leq \varepsilon_{\ail}. 
\end{align}
For any $h, h^\prime \in [H]$ with $h \leq h^\prime$, we use $\pi_{h:h^\prime}$ denote the shorthand of $\lp \pi_h, \pi_{h+1}, \cdots, \pi_{h^\prime} \rp$. Note that $\text{Loss}_{h} (\pi)$ only depends on $\pi_{1:h}$ and thus we have
\begin{align*}
    \sum_{h=1}^{H} \text{Loss}_{h} (\widebar{\pi}_{1:h}) - \text{Loss}_{h} (\piE_{1:h}) \leq \varepsilon_{\ail}.
\end{align*}
We defined a policy set $\Pi^{\text{opt}} = \{ \pi \in \Pi: \forall h \in [H], \exists s \in \goodS, \pi_h (a^{1}|s) > 0 \}$ and note that $\widebar{\pi} \in \Pi^{\text{opt}}$. In the following part, we analyze $\sum_{h=1}^{H} \text{Loss}_{h} (\pi_{1:h}) - \text{Loss}_{h} (\piE_{1:h})$ where $\pi \in \Pi^{\text{opt}}$. For each $h \in [H]$, we have the following key composition by telescoping: 
\begin{align}
\label{eq:sum_telescoping}
\boxed{
    \text{Loss}_{h} (\pi_{1:h}) - \text{Loss}_{h} (\piE_{1:h}) = \sum_{\ell=1}^{h} \text{Loss}_{h} (\pi_{1:\ell}, \piE_{\ell+1:h}) - \text{Loss}_{h} (\pi_{1:\ell-1}, \piE_{\ell:h}). 
}
\end{align}
In the following part, we consider two cases: Case I: $ h<H$ and Case II: $ h = H$.

First, we consider Case I and focus on the term $\text{Loss}_{h} (\pi_{1:\ell}, \piE_{\ell+1:h}) - \text{Loss}_{h} (\pi_{1:\ell-1}, \piE_{\ell:h})$. Under Case I, we consider two situations: $\ell = h$ and $\ell < h$.

\begin{itemize}
    \item When $\ell = h$, we consider the term $\text{Loss}_{h} (\pi_{1:h}) - \text{Loss}_{h} (\pi_{1:h-1}, \piE_{h})$. Note that $\pi_{1:h}$ and $(\pi_{1:h-1}, \piE_{h})$ differ in the policy in time step $h$. Take the policy in time step $h$ as variable and we focus on
    \begin{align*}
        g (\pi_{h}) - g(\piE_{h}),
    \end{align*}
    where $g (\pi_{h}) = \text{Loss}_{h} (\pi_{1:h})$ and $g(\piE_{h}) = \text{Loss}_{h} (\pi_{1:h-1}, \piE_{h})$. We formulate $g (\pi_{h}) = \text{Loss}_{h} (\pi_{1:h})$ as
    \begin{align*}
        g (\pi_{h}) &=  \sum_{(s, a) \in \gS \times \gA} | \widehat{P}^{\piE}_h(s, a) - P^{\pi}_h(s, a)  |
        \\
        &= \sum_{s \in \goodS} \sum_{a \in \gA} \labs \widehat{P}^{\piE}_{h} (s, a) - P^{\pi}_{h} (s) \pi_{h} (a|s)  \rabs + \sum_{s \in \badS} \sum_{a \in \gA} P^{\pi}_{h} (s, a)
        \\
        &= \sum_{s \in \goodS} \lp \labs \widehat{P}^{\piE}_{h} (s, a^1) - P^{\pi}_{h} (s) \pi_h(a^1|s) \rabs + P^{\pi}_{h} (s) \lp 1 - \pi_h(a^1|s)  \rp  \rp + \sum_{s \in \badS} P^{\pi}_{h} (s)  
        \\
        &= \sum_{s \in \goodS}\lp \labs \widehat{P}^{\piE}_{h} (s) - P^{\pi}_{h} (s) \pi_h(a^1|s) \rabs + P^{\pi}_{h} (s) \lp 1 - \pi_h(a^1|s)  \rp   \rp + \sum_{s \in \badS} P^{\pi}_{h} (s). 
    \end{align*}
    Note that $P^{\pi}_{h} (s)$ is independent of the policy in time step $h$. Then we have that
    \begin{align*}
       g (\pi_{h}) - g(\piE_{h})  &= \sum_{s \in \goodS}\lp \labs \widehat{P}^{\piE}_{h} (s) - P^{\pi}_{h} (s) \pi_h(a^1|s) \rabs - P^{\pi}_{h} (s)   \pi_h(a^1|s)     \rp \\
       &\quad - \lp \labs \widehat{P}^{\piE}_{h} (s) 
        \quad - P^{\pi}_{h} (s) \piE_h(a^1|s) \rabs - P^{\pi}_{h} (s)   \piE_h(a^1|s)     \rp. 
    \end{align*}
    For each $s \in \goodS$, we apply \cref{lem:single_variable_opt} and obtain that 
    \begin{align}
    \label{eq:case_one_situation_one_result}
        g (\pi_{h}) - g(\piE_{h}) = \text{Loss}_{h} (\pi_{1:h}) - \text{Loss}_{h} (\pi_{1:h-1}, \piE_{h}) \geq 0.
    \end{align}
    \item When $\ell < h$, we consider the term $\text{Loss}_{h} (\pi_{1:\ell}, \piE_{\ell+1:h}) - \text{Loss}_{h} (\pi_{1:\ell-1}, \piE_{\ell:h})$. Notice that $(\pi_{1:\ell}, \piE_{\ell+1:h})$ and $(\pi_{1:\ell-1}, \piE_{\ell:h})$ only differ in the policy in time step $\ell$. Take the policy in time step $\ell$ as variable and we focus on
    \begin{align*}
        g (\pi_{\ell}) - g(\piE_{\ell}),
    \end{align*}
    where $g (\pi_{\ell}) = \text{Loss}_{h} (\pi_{1:\ell}, \piE_{\ell+1:h})$ and $g (\piE_{\ell}) = \text{Loss}_{h} (\pi_{1:\ell-1}, \piE_{\ell:h})$. We can calculate $g (\pi_{\ell})$ as
    \begin{align*}
    g (\pi_{\ell}) &=  \sum_{(s, a) \in \gS \times \gA} | \widehat{P}^{\piE}_h(s, a) - P^{\pi}_h(s, a)  |
    \\
    &= \sum_{s \in \goodS} \sum_{a \in \gA} \labs \widehat{P}^{\piE}_{h} (s, a) - P^{\pi}_{h} (s) \pi_{h} (a|s)  \rabs + \sum_{s \in \badS} \sum_{a \in \gA} P^{\pi}_{h} (s, a)
    \\
    &= \sum_{s \in \goodS} \labs \widehat{P}^{\piE}_{h} (s, a^1) - P^{\pi}_{h} (s, a^1) \rabs + \sum_{s \in \badS} P^{\pi}_{h} (s)  
    \\
    &= \sum_{s \in \goodS} \labs \widehat{P}^{\piE}_{h} (s) - P^{\pi}_{h} (s) \rabs + \sum_{s \in \badS} P^{\pi}_{h} (s).
    \end{align*}
    With a little abuse of notation, we use $P^{\pi}_h(s, a)$ and $P^{\pi}_{h} (s)$ to denote the distributions induced by $(\pi_{1:\ell}, \piE_{\ell+1:h})$. Similar to the proof of \cref{prop:ail_general_reset_cliff}, with the \dquote{transition flow equation}, we have
    \begin{align*}
        \forall s \in \goodS, P^{\pi}_{h} (s) &= \sum_{s^\prime \in \gS} \sum_{a \in \gA} P^{\pi}_{\ell} (s^\prime) \pi_\ell (a|s^\prime) \sP^{\pi} \lp s_{h} = s |s_\ell = s^\prime, a_\ell = a \rp  
        \\
        &= \sum_{s^\prime \in \goodS} P^{\pi}_{\ell} (s^\prime) \pi_{\ell} (a^{1}|s^\prime) \sP^{\pi} \lp s_{h} = s |s_{\ell} = s^\prime, a_{h} = a^{1} \rp.
    \end{align*}
    Notice that the conditional probability $\sP^{\pi} \lp s_{h} = s |s_{\ell} = s^\prime, a_{h} = a^{1} \rp$ is independent of $\pi_\ell$. Besides, for the visitation probability on bad states in time step $h$, we have
    \begin{align*}
        \sum_{s \in \badS} P^{\pi}_{h} (s) &= \sum_{s \in \badS} P^{\pi}_{\ell} (s) + \sum_{s^\prime \in \goodS} \sum_{a \in \gA \setminus \{a^1 \}} P^{\pi}_{\ell} (s^\prime)  \pi_{\ell} (a|s^\prime)
        \\
        &= \sum_{s \in \badS} P^{\pi}_{\ell} (s) + \sum_{s^\prime \in \goodS} P^{\pi}_{\ell} (s^\prime) \lp 1 - \pi_{\ell} (a^{1}|s^\prime) \rp .
    \end{align*}
    Plugging the above two equations into $g (\pi_{\ell})$ yields that
    \begin{align*}
        g (\pi_{\ell})  &= \sum_{s \in \goodS} \labs \widehat{P}^{\piE}_{h} (s) - \sum_{s^\prime \in \goodS} P^{\pi}_{\ell} (s^\prime) \pi_{\ell} (a^{1}|s^\prime) \sP^{\pi} \lp s_{h} = s |s_{\ell} = s^\prime, a_{\ell} = a^{1} \rp \rabs
        \\
        &\quad + \sum_{s \in \badS} P^{\pi}_{\ell} (s) + \sum_{s^\prime \in \goodS} P^{\pi}_{\ell} (s^\prime) \lp 1 - \pi_{\ell} (a^{1}|s^\prime) \rp. 
    \end{align*}
    Notice that $P^{\pi}_{\ell} (s)$ is independent of the policy in time step $\ell$ and we have
    \begin{align*}
    &\quad g (\pi_{\ell}) - g (\piE_{\ell}) \\
    &= \lp \sum_{s \in \goodS} \labs \widehat{P}^{\piE}_{h} (s) - \sum_{s^\prime \in \goodS} P^{\pi}_{\ell} (s^\prime)  \sP^{\pi} \lp s_{h} = s |s_{\ell} = s^\prime, a_{\ell} = a^{1} \rp \pi_{\ell} (a^{1}|s^\prime) \rabs - \sum_{s^\prime \in \goodS} P^{\pi}_{\ell} (s^\prime) \pi_{\ell} (a^{1}|s^\prime)   \rp
    \\
    &\quad - \lp \sum_{s \in \goodS} \labs \widehat{P}^{\piE}_{h} (s) - \sum_{s^\prime \in \goodS} P^{\pi}_{\ell} (s^\prime)  \sP^{\pi} \lp s_{h} = s |s_{\ell} = s^\prime, a_{\ell} = a^{1} \rp \piE_{\ell} (a^{1}|s^\prime) \rabs - \sum_{s^\prime \in \goodS} P^{\pi}_{\ell} (s^\prime) \piE_{\ell} (a^{1}|s^\prime)   \rp .
    \end{align*}
    For this type function, we can use \cref{lem:mn_variables_opt_regularity} to prove that
    \begin{align*}
    g (\pi_{\ell}) - g (\piE_{\ell}) &\geq \sum_{s^\prime \in \goodS} \min_{s \in \goodS} \{ P^{\pi}_{\ell} (s^\prime) \sP^{\pi} \lp s_{h} = s |s_{\ell} = s^\prime, a_{\ell} = a^{1} \rp \} \lp 1 - \pi_{\ell} (a^{1}|s^\prime)  \rp
    \\
    &= \sum_{s^\prime \in \goodS} \min_{s \in \goodS} \{  \sP^{\pi} \lp s_{h} = s |s_{\ell} = s^\prime, a_{\ell} = a^{1} \rp \} P^{\pi}_{\ell} (s^\prime) \lp 1 - \pi_{\ell} (a^{1}|s^\prime)  \rp.
    \end{align*}
    To check conditions in \cref{lem:mn_variables_opt_regularity}, we define
    \begin{align*}
        & m = n = \labs \goodS \rabs, \forall s \in \goodS, c(s) = \widehat{P}^{\piE}_{h} (s), \\
        & \forall s, s^\prime \in \goodS, A (s, s^\prime) = P^{\pi}_{\ell} (s^\prime)  \sP^{\pi} \lp s_{h} = s |s_{\ell} = s^\prime, a_{\ell} = a^{1} \rp,
        \\
        & \forall s^\prime \in \goodS, d(s^\prime) = P^{\pi}_{\ell} (s^\prime). 
    \end{align*}
    Note that $\pi \in \Pi^{\text{opt}} = \{ \pi \in \Pi: \forall h \in [H], \exists s \in \goodS, \pi_h (a^{1}|s) > 0 \}$. Combined with the reachable assumption that $\forall h \in [H], s, s^\prime \in \goodS, P_h (s^\prime |s, a^1) > 0$, we have that
    \begin{align*}
        \forall s, s^\prime \in \goodS, P^{\pi}_{\ell} (s^\prime)  > 0, \sP^{\pi} \lp s_{h} = s |s_\ell = s^\prime, a_\ell = a^{1} \rp > 0.
    \end{align*}
    Then we can obtain that $A > 0$ where $>$ means element-wise comparison. Besides, we have that
    \begin{align*}
        & \sum_{s \in \goodS} c (s) = 1 \geq \sum_{s \in \goodS} \sum_{s^\prime \in \goodS} P^{\pi}_\ell (s^\prime)  \sP^{\pi} \lp s_{h} = s |s_\ell = s^\prime, a_\ell = a^{1} \rp = \sum_{s \in \goodS} \sum_{s^\prime \in \goodS} A (s, s^\prime).
    \end{align*}
    For each $s^\prime \in \goodS$, we further have that 
    \begin{align*}
        \sum_{s \in \goodS} A (s, s^\prime) = \sum_{s \in \goodS} P^{\pi}_\ell (s^\prime)  \sP^{\pi} \lp s_{h} = s |s_\ell = s^\prime, a_\ell = a^{1} \rp = P^{\pi}_\ell (s^\prime) = d(s^\prime).  
    \end{align*}
    Thus, we have verified conditions in \cref{lem:mn_variables_opt_regularity}. By \cref{lem:mn_variables_opt_regularity}, we have that
    \begin{align*}
    g (\pi_{\ell}) - g (\piE_{\ell}) &\geq \sum_{s^\prime \in \goodS} \min_{s \in \goodS} \{  \sP^{\pi} \lp s_{h} = s |s_{\ell} = s^\prime, a_{\ell} = a^{1} \rp \} P^{\pi}_{\ell} (s^\prime) \lp 1 - \pi_{\ell} (a^{1}|s^\prime)  \rp
    \\
    &\geq \min_{s, s^\prime \in \goodS} \{  \sP^{\pi} \lp s_{h} = s |s_{\ell} = s^\prime, a_{\ell} = a^{1} \rp \} \sum_{s^\prime \in \goodS} P^{\pi}_{\ell} (s^\prime) \lp 1 - \pi_{\ell} (a^{1}|s^\prime)  \rp
    \\
    &= c_{\ell, h} \sum_{s^\prime \in \goodS} P^{\pi}_{\ell} (s^\prime) \lp 1 - \pi_{\ell} (a^{1}|s^\prime)  \rp.   
    \end{align*}
    Here $c_{\ell, h} = \min_{s, s^\prime \in \goodS} \{ \sP^{\pi} \lp s_{h} = s |s_{\ell} = s^\prime, a_{\ell} = a^{1} \rp \} > 0$. In conclusion, we prove that for each $\ell < h$,
    \begin{align}
        \text{Loss}_{h} (\pi_{1:\ell}, \piE_{\ell+1:h}) - \text{Loss}_{h} (\pi_{1:\ell-1}, \piE_{\ell:h}) \geq c_{\ell, h} \sum_{s^\prime \in \goodS} P^{\pi}_{\ell} (s^\prime) \lp 1 - \pi_{\ell} (a^{1}|s^\prime)  \rp, \label{eq:case_one_situation_two_result} 
    \end{align}
    where $c_{\ell, h} = \min_{s, s^\prime \in \goodS} \{ \sP^{\pi} \lp s_{h} = s |s_{\ell} = s^\prime, a_{\ell} = a^{1} \rp \} > 0$.
\end{itemize}

Then for Case I where $h < H$, we combine the results in \eqref{eq:case_one_situation_one_result} and \eqref{eq:case_one_situation_two_result} to obtain 
\begin{align}
    \text{Loss}_{h} (\pi_{1:h}) - \text{Loss}_{h} (\piE_{1:h}) &= \sum_{\ell=1}^{h} \text{Loss}_{h} (\pi_{1:\ell}, \piE_{\ell+1:h}) - \text{Loss}_{h} (\pi_{1:\ell-1}, \piE_{\ell:h}) \nonumber
    \\
    &= \text{Loss}_{h} (\pi_{1:h}) - \text{Loss}_{h} (\pi_{1:h-1}, \piE_{h}) + \sum_{\ell=1}^{h-1} \text{Loss}_{h} (\pi_{1:\ell}, \piE_{\ell+1:h}) - \text{Loss}_{h} (\pi_{1:\ell-1}, \piE_{\ell:h}) \nonumber
    \\
    &\geq \sum_{\ell=1}^{h-1} \text{Loss}_{h} (\pi_{1:\ell}, \piE_{\ell+1:h}) - \text{Loss}_{h} (\pi_{1:\ell-1}, \piE_{\ell:h}) \nonumber
    \\
    &\geq \sum_{\ell=1}^{h-1} c_{\ell, h} \sum_{s^\prime \in \goodS} P^{\pi}_{\ell} (s^\prime) \lp 1 - \pi_{\ell} (a^{1}|s^\prime)  \rp, \label{eq:case_one_result} 
\end{align}
where $c_{\ell, h} = \min_{s, s^\prime \in \goodS} \{ \sP^{\pi} \lp s_{h} = s |s_{\ell} = s^\prime, a_{\ell} = a^{1} \rp \}$. The penultimate inequality follows \eqref{eq:case_one_situation_one_result} and the last inequality follows \eqref{eq:case_one_situation_two_result}. 

Second, we consider Case II where $h = H$. By telescoping, we have that
\begin{align}
    &\quad \text{Loss}_{H} (\pi_{1:H}) - \text{Loss}_{H} (\piE_{1:H}) \nonumber
    \\
    &= \sum_{\ell=1}^{H} \text{Loss}_{H} (\pi_{1:\ell}, \piE_{\ell+1:H}) - \text{Loss}_{H} (\pi_{1:\ell-1}, \piE_{\ell:H}) \nonumber
    \\
    &= \text{Loss}_{H} (\pi_{1:H}) - \text{Loss}_{H} (\pi_{1:H-1}, \piE_{H}) + \sum_{\ell=1}^{H-1} \text{Loss}_{H} (\pi_{1:\ell}, \piE_{\ell+1:H}) - \text{Loss}_{H} (\pi_{1:\ell-1}, \piE_{\ell:H}). \label{eq:case_two_telescoping}
\end{align}
Similar to Case I, we also consider two situations: $\ell=H$ and $\ell<H$. We first consider the situation where $\ell<H$, which is similar to the corresponding part under Case I.

\begin{itemize}
    \item When $\ell<H$, we consider $\text{Loss}_{H} (\pi_{1:\ell}, \piE_{\ell+1:H}) - \text{Loss}_{H} (\pi_{1:\ell-1}, \piE_{\ell:H})$. The following analysis is similar to that under Case I. Note that $(\pi_{1:\ell}, \piE_{\ell+1:H})$ and $(\pi_{1:\ell-1}, \piE_{\ell:H})$ only differ in the policy in time step $\ell$. We take the policy in time step $\ell$ as variable and focus on
    \begin{align*}
        g (\pi_{\ell}) - g(\piE_{\ell}),
    \end{align*}
    where $g (\pi_{\ell}) = \text{Loss}_{H} (\pi_{1:\ell}, \piE_{\ell+1:h})$ and $g (\piE_{\ell}) = \text{Loss}_{H} (\pi_{1:\ell-1}, \piE_{\ell:h})$. Similarly, we have 
    \begin{align*}
        g (\pi_{\ell}) = \sum_{s \in \goodS} \labs \widehat{P}^{\piE}_{H} (s) - P^{\pi}_{H} (s) \rabs + \sum_{s \in \badS} P^{\pi}_{H} (s).
    \end{align*}
    With a little abuse of notation, we use $P^{\pi}_h(s)$ to denote the distributions induced by $(\pi_{1:\ell}, \piE_{\ell+1:h})$. With the \dquote{transition flow equation}, it holds that
    \begin{align*}
        &\forall s \in \goodS, P^{\pi}_{H} (s) = \sum_{s^\prime \in \goodS} P^{\pi}_{\ell} (s^\prime) \pi_{\ell} (a^{1}|s^\prime) \sP^{\pi} \lp s_{H} = s |s_{\ell} = s^\prime, a_{h} = a^{1} \rp,
        \\
        & \sum_{s \in \badS} P^{\pi}_{H} (s) = \sum_{s \in \badS} P^{\pi}_{\ell} (s) + \sum_{s^\prime \in \goodS} P^{\pi}_{\ell} (s^\prime) \lp 1 - \pi_{\ell} (a^{1}|s^\prime) \rp .
    \end{align*}
    Plugging the above two equations into $g (\pi_{\ell})$ yields that
    \begin{align*}
        g (\pi_{\ell})  &= \sum_{s \in \goodS} \labs \widehat{P}^{\piE}_{H} (s) - \sum_{s^\prime \in \goodS} P^{\pi}_{\ell} (s^\prime) \pi_{\ell} (a^{1}|s^\prime) \sP^{\pi} \lp s_{H} = s |s_{\ell} = s^\prime, a_{\ell} = a^{1} \rp \rabs
        \\
        &\quad + \sum_{s \in \badS} P^{\pi}_{\ell} (s) + \sum_{s^\prime \in \goodS} P^{\pi}_{\ell} (s^\prime) \lp 1 - \pi_{\ell} (a^{1}|s^\prime) \rp. 
    \end{align*}
    Notice that $P^{\pi}_{\ell} (s)$ is independent of the policy in time step $\ell$ and we have
    \begin{align*}
    &\quad g (\pi_{\ell}) - g (\piE_{\ell})
    \\
    &= \lp \sum_{s \in \goodS} \labs \widehat{P}^{\piE}_{H} (s) - \sum_{s^\prime \in \goodS} P^{\pi}_{\ell} (s^\prime)  \sP^{\pi} \lp s_{H} = s |s_{\ell} = s^\prime, a_{\ell} = a^{1} \rp \pi_{\ell} (a^{1}|s^\prime) \rabs - \sum_{s^\prime \in \goodS} P^{\pi}_{\ell} (s^\prime) \pi_{\ell} (a^{1}|s^\prime)   \rp
    \\
    &- \lp \sum_{s \in \goodS} \labs \widehat{P}^{\piE}_{H} (s) - \sum_{s^\prime \in \goodS} P^{\pi}_{\ell} (s^\prime)  \sP^{\pi} \lp s_{H} = s |s_{\ell} = s^\prime, a_{\ell} = a^{1} \rp \piE_{\ell} (a^{1}|s^\prime) \rabs - \sum_{s^\prime \in \goodS} P^{\pi}_{\ell} (s^\prime) \piE_{\ell} (a^{1}|s^\prime)   \rp .
    \end{align*}
    For this type function in RHS, we can use \cref{lem:mn_variables_opt_regularity} to prove that
    \begin{align*}
    g (\pi_{\ell}) - g (\piE_{\ell}) &\geq \sum_{s^\prime \in \goodS} \min_{s \in \goodS} \{ P^{\pi}_{\ell} (s^\prime) \sP^{\pi} \lp s_{H} = s |s_{\ell} = s^\prime, a_{\ell} = a^{1} \rp \} \lp 1 - \pi_{\ell} (a^{1}|s^\prime)  \rp
    \\
    &= \sum_{s^\prime \in \goodS} \min_{s \in \goodS} \{  \sP^{\pi} \lp s_{H} = s |s_{\ell} = s^\prime, a_{\ell} = a^{1} \rp \} P^{\pi}_{\ell} (s^\prime) \lp 1 - \pi_{\ell} (a^{1}|s^\prime)  \rp.
    \end{align*}
    To check conditions in \cref{lem:mn_variables_opt_regularity}, we define
    \begin{align*}
        & m = n = \labs \goodS \rabs, \forall s \in \goodS, c(s) = \widehat{P}^{\piE}_{H} (s), \\
        & \forall s, s^\prime \in \goodS, A (s, s^\prime) = P^{\pi}_{\ell} (s^\prime)  \sP^{\pi} \lp s_{H} = s |s_{\ell} = s^\prime, a_{\ell} = a^{1} \rp,
        \\
        & \forall s^\prime \in \goodS, d(s^\prime) = P^{\pi}_{\ell} (s^\prime). 
    \end{align*}
    Similar to the analysis under Case I, we obtain that $A > 0$ and
    \begin{align*}
         & \sum_{s \in \goodS} c (s) = 1 \geq \sum_{s \in \goodS} \sum_{s^\prime \in \goodS} P^{\pi}_\ell (s^\prime)  \sP^{\pi} \lp s_{H} = s |s_\ell = s^\prime, a_\ell = a^{1} \rp = \sum_{s \in \goodS} \sum_{s^\prime \in \goodS} A (s, s^\prime),
         \\
         & \forall s^\prime \in \goodS, \sum_{s \in \goodS} A (s, s^\prime) = \sum_{s \in \goodS} P^{\pi}_\ell (s^\prime)  \sP^{\pi} \lp s_{h} = s |s_\ell = s^\prime, a_\ell = a^{1} \rp = P^{\pi}_\ell (s^\prime) = d(s^\prime).
    \end{align*}
    Thus, we have verified conditions in \cref{lem:mn_variables_opt_regularity} and prove that
    \begin{align*}
    g (\pi_{\ell}) - g (\piE_{\ell}) &\geq \sum_{s^\prime \in \goodS} \min_{s \in \goodS} \{  \sP^{\pi} \lp s_{H} = s |s_{\ell} = s^\prime, a_{\ell} = a^{1} \rp \} P^{\pi}_{\ell} (s^\prime) \lp 1 - \pi_{\ell} (a^{1}|s^\prime)  \rp
    \\
    &\geq \min_{s, s^\prime \in \goodS} \{  \sP^{\pi} \lp s_{H} = s |s_{\ell} = s^\prime, a_{\ell} = a^{1} \rp \} \sum_{s^\prime \in \goodS} P^{\pi}_{\ell} (s^\prime)  \lp 1 - \pi_{\ell} (a^{1}|s^\prime)  \rp 
    \\
    &= c_{\ell, H} \sum_{s^\prime \in \goodS} P^{\pi}_{\ell} (s^\prime)  \lp 1 - \pi_{\ell} (a^{1}|s^\prime) \rp. 
    \end{align*}
    Here $c_{\ell, H} = \min_{s, s^\prime \in \goodS} \{ \sP^{\pi} \lp s_{H} = s |s_{\ell} = s^\prime, a_{\ell} = a^{1} \rp \} $. In summary, for $\ell < H$, we prove that
    \begin{align}
    \label{eq:case_two_situation_one_result}
        \text{Loss}_{H} (\pi_{1:\ell}, \piE_{\ell+1:H}) - \text{Loss}_{H} (\pi_{1:\ell-1}, \piE_{\ell:H}) \geq c_{\ell, H} \sum_{s^\prime \in \goodS} P^{\pi}_{\ell} (s^\prime)  \lp 1 - \pi_{\ell} (a^{1}|s^\prime) \rp. 
    \end{align}
    \item When $\ell = H$, we consider the term $\text{Loss}_{H} (\pi_{1:H}) - \text{Loss}_{H} (\pi_{1:H-1}, \piE_{H})$. The analysis under this situation is more complex. Note that $\pi_{1:H}$ and $(\pi_{1:H-1}, \piE_{H})$ only differs in the policy in the last time step $H$. Take the policy in time step $H$ as variable and we focus on
    \begin{align*}
        g (\pi_{H}) - g(\piE_{H}),
    \end{align*}
    where $g (\pi_{H}) = \text{Loss}_{H} (\pi_{1:H})$ and $g(\piE_{H}) = \text{Loss}_{H} (\pi_{1:H-1}, \piE_{H})$. Similarly, we can formulate $g (\pi_{H}) = \text{Loss}_{H} (\pi_{1:H})$ as
    \begin{align*}
        g (\pi_{H}) = \sum_{s \in \goodS}\lp \labs \widehat{P}^{\piE}_{H} (s) - P^{\pi}_{H} (s) \pi_H(a^1|s) \rabs + P^{\pi}_{H} (s) \lp 1 - \pi_H(a^1|s)  \rp   \rp + \sum_{s \in \badS} P^{\pi}_{H} (s).
    \end{align*}
    Note that $P^{\pi}_{H} (s)$ is independent of the policy in time step $H$ and we have that
    \begin{align*}
        g (\pi_{H}) - g(\piE_{H}) &= \sum_{s \in \goodS} \lp \labs \widehat{P}^{\piE}_{H} (s) - P^{\pi}_{H} (s) \pi_H (a^1|s) \rabs - P^{\pi}_{H} (s)   \pi_H (a^1|s)     \rp \\
        &\quad - \lp \labs \widehat{P}^{\piE}_{H} (s) - P^{\pi}_{H} (s) \piE_H (a^1|s) \rabs - P^{\pi}_{H} (s)   \piE_H (a^1|s)     \rp.
    \end{align*}
    Given estimation $\widehat{P}^{\piE}_{H} (s)$, we divide the set of good states into two parts. That is $\goodS = \gS^{\pi}_H \cup  \lp \gS^{\pi}_H \rp^c$ and $\gS^{\pi}_H \cap \lp \gS^{\pi}_H \rp^c = \emptyset$. Here $\gS^{\pi}_H  = \{s \in \goodS, \pi_H (a^1|s) \leq \min\{1, \widehat{P}^{\piE}_{H} (s) / P^{\piE}_H (s) \}  \}$. Therefore, we have that
    \begin{align*}
     g (\pi_{H}) - g(\piE_{H}) &= \sum_{s \in  \gS^{\pi}_H} \lp \labs \widehat{P}^{\piE}_{H} (s) - P^{\pi}_{H} (s) \pi_H (a^1|s) \rabs - P^{\pi}_{H} (s)   \pi_H (a^1|s)     \rp \\
     &\quad - \lp \labs \widehat{P}^{\piE}_{H} (s) - P^{\pi}_{H} (s) \piE_H (a^1|s) \rabs - P^{\pi}_{H} (s)   \piE_H (a^1|s)     \rp
        \\
        &\quad \underbrace{+  \sum_{s \in  \lp \gS^{\pi}_H \rp^c} \lp \labs \widehat{P}^{\piE}_{H} (s) - P^{\pi}_{H} (s) \pi_H (a^1|s) \rabs - P^{\pi}_{H} (s)   \pi_H (a^1|s)     \rp}_{\text{Term I}} \\
        &\quad \underbrace{- \lp \labs \widehat{P}^{\piE}_{H} (s) - P^{\pi}_{H} (s) \piE_H (a^1|s) \rabs - P^{\pi}_{H} (s)   \piE_H (a^1|s)     \rp}_{\text{Term I}}. 
    \end{align*}
    By \cref{lem:single_variable_opt}, we that $\text{Term I} + \text{Term II} \geq 0$. Then we have that
    \begin{align*}
       g (\pi_{H}) - g(\piE_{H})  &\geq \sum_{s \in  \gS^{\pi}_H} \lp \labs \widehat{P}^{\piE}_{H} (s) - P^{\pi}_{H} (s) \pi_H (a^1|s) \rabs - P^{\pi}_{H} (s)   \pi_H (a^1|s)     \rp \\
       &\quad - \lp \labs \widehat{P}^{\piE}_{H} (s) - P^{\pi}_{H} (s) \piE_H (a^1|s) \rabs - P^{\pi}_{H} (s)   \piE_H (a^1|s)     \rp.
    \end{align*}
    For each $s \in  \gS^{\pi}_H$, we consider
    \begin{align*}
        \lp \labs \widehat{P}^{\piE}_{H} (s) - P^{\pi}_{H} (s) \pi_H (a^1|s) \rabs - P^{\pi}_{H} (s)   \pi_H (a^1|s)     \rp - \lp \labs \widehat{P}^{\piE}_{H} (s) - P^{\pi}_{H} (s) \piE_H (a^1|s) \rabs - P^{\pi}_{H} (s)   \piE_H (a^1|s)     \rp.
    \end{align*}
    We aim to apply \cref{lem:single_variable_regularity} to prove that
    \begin{align*}
        &\quad \lp \labs \widehat{P}^{\piE}_{H} (s) - P^{\pi}_{H} (s) \pi_H (a^1|s) \rabs - P^{\pi}_{H} (s)   \pi_H (a^1|s)     \rp - \lp \labs \widehat{P}^{\piE}_{H} (s) - P^{\pi}_{H} (s) \piE_H (a^1|s) \rabs - P^{\pi}_{H} (s)   \piE_H (a^1|s)     \rp
        \\
        &\geq 2 P^{\pi}_{H} (s) \lp \min\{1,  \widehat{P}^{\piE}_{H} (s) / P^{\piE}_H (s)\} -  \pi_H (a^1|s)  \rp.
    \end{align*}
    To check the conditions in \cref{lem:single_variable_regularity}, we define
    \begin{align*}
        c = \widehat{P}^{\piE}_{H} (s), a = P^{\pi}_{H} (s), x = \pi_H (a^1|s).   
    \end{align*}
    It is easy to see that $c \geq 0$. Since $\pi \in \Pi^{\text{opt}} := \{ \pi \in \Pi: \forall h \in [H], \exists s \in \goodS, \pi_h (a^{1}|s) > 0 \}$, combined with the reachable assumption that $\forall h \in [H-1], \forall s, s^\prime \in \goodS, P_{h} (s^\prime|s, a^{1}) > 0$, we have that $a = P^{\pi}_{H} (s) > 0$. According to the definition of $\gS^{\pi}_H$, we have that $x =  \pi_H (a^1|s) \leq \min\{ 1,  \widehat{P}^{\piE}_{H} (s) / P^{\piE}_H (s) \} \leq  \min\{ 1,  \widehat{P}^{\piE}_{H} (s) / P^{\pi}_H (s) \} = \min\{ 1,  c / a \}$. We have verified the conditions in \cref{lem:single_variable_regularity} and obtain that
    \begin{align*}
        &\quad \lp \labs \widehat{P}^{\piE}_{H} (s) - P^{\pi}_{H} (s) \pi_H (a^1|s) \rabs - P^{\pi}_{H} (s)   \pi_H (a^1|s)     \rp - \lp \labs \widehat{P}^{\piE}_{H} (s) - P^{\pi}_{H} (s) \piE_H (a^1|s) \rabs - P^{\pi}_{H} (s)   \piE_H (a^1|s)     \rp
        \\
        &= 2 P^{\pi}_{H} (s) \lp \min\{1,  \widehat{P}^{\piE}_{H} (s) / P^{\pi}_H (s)\} -  \pi_H (a^1|s)  \rp
        \\
        &\geq 2 P^{\pi}_{H} (s) \lp \min\{1,  \widehat{P}^{\piE}_{H} (s) / P^{\piE}_H (s)\} -  \pi_H (a^1|s)  \rp, 
    \end{align*}
    where the last inequality follows that $\forall s \in \goodS, P^{\piE}_H (s) \geq P^{\pi}_H (s)$. Plugging the above inequality into $g (\pi_{H}) - g(\piE_{H})$ yields that
    \begin{align*}
        g (\pi_{H}) - g(\piE_{H}) \geq 2 \sum_{s \in  \gS^{\pi}_H}  P^{\pi}_{H} (s) \lp \min\{1,  \widehat{P}^{\piE}_{H} (s) / P^{\piE}_H (s)\} -  \pi_H (a^1|s)  \rp .
    \end{align*}
    In summary, under this situation, we prove that 
    \begin{align}
    \label{eq:case_two_situation_two_result}
        \text{Loss}_{H} (\pi_{1:H}) - \text{Loss}_{H} (\pi_{1:H-1}, \piE_{H}) \geq  2 \sum_{s \in  \gS^{\pi}_H}  P^{\pi}_{H} (s) \lp \min\{1,  \widehat{P}^{\piE}_{H} (s) / P^{\piE}_H (s)\} -  \pi_H (a^1|s)  \rp . 
    \end{align}
\end{itemize}

Under Case II where $h=H$, with \eqref{eq:case_two_telescoping}, \eqref{eq:case_two_situation_one_result}, and \eqref{eq:case_two_situation_two_result},   we have that
\begin{align}
    &\quad \text{Loss}_{H} (\pi_{1:H}) - \text{Loss}_{H} (\piE_{1:H}) \nonumber
    \\
    &= \text{Loss}_{H} (\pi_{1:H}) - \text{Loss}_{H} (\pi_{1:H-1}, \piE_{H}) + \sum_{\ell=1}^{H-1} \text{Loss}_{H} (\pi_{1:\ell}, \piE_{\ell+1:H}) - \text{Loss}_{H} (\pi_{1:\ell-1}, \piE_{\ell:H}) \nonumber
    \\
    &\geq 2 \sum_{s \in  \gS^{\pi}_H}  P^{\pi}_{H} (s) \lp \min\{1,  \widehat{P}^{\piE}_{H} (s) / P^{\piE}_H (s)\} -  \pi_H (a^1|s)  \rp + \sum_{\ell=1}^{H-1} c_{\ell, H} \sum_{s \in \goodS} P^{\pi}_{\ell} (s)  \lp 1 - \pi_{\ell} (a^{1}|s) \rp, \label{eq:case_two_result} 
\end{align}
where $c_{\ell, H} = \min_{s, s^\prime \in \goodS} \{ \sP^{\pi} \lp s_{H} = s |s_{\ell} = s^\prime, a_{\ell} = a^{1} \rp \} $. The last inequality follows $\eqref{eq:case_two_situation_one_result}$ and $\eqref{eq:case_two_situation_two_result}$.

Finally, we combine the results in \eqref{eq:case_one_result} and $\eqref{eq:case_two_result}$ to obtain that 
\begin{align*}
    f (\pi) - f(\piE) &= \sum_{h=1}^{H} \text{Loss}_{h} (\pi_{1:h}) - \text{Loss}_{h} (\piE_{1:h})
    \\
    &=  \sum_{h=1}^{H-1} \text{Loss}_{h} (\pi_{1:h}) - \text{Loss}_{h} (\piE_{1:H}) + \text{Loss}_{H} (\pi_{1:h}) - \text{Loss}_{H} (\piE_{1:H})
    \\
    &\geq \sum_{h=1}^{H-1} \sum_{\ell=1}^{h-1} c_{\ell, h} \sum_{s \in \goodS} P^{\pi}_{\ell} (s) \lp 1 - \pi_{\ell} (a^{1}|s)  \rp 
    \\
    &\quad + 2 \sum_{s \in  \gS^{\pi}_H}  P^{\pi}_{H} (s) \lp \min\{1,  \widehat{P}^{\piE}_{H} (s) / P^{\piE}_H (s)\} -  \pi_H (a^1|s)  \rp + \sum_{\ell=1}^{H-1} c_{\ell, H} \sum_{s \in \goodS} P^{\pi}_{\ell} (s)  \lp 1 - \pi_{\ell} (a^{1}|s) \rp
    \\
    &= \sum_{h=1}^{H} \sum_{\ell=1}^{h-1} c_{\ell, h} \sum_{s \in \goodS} P^{\pi}_{\ell} (s) \lp 1 - \pi_{\ell} (a^{1}|s)  \rp + 2 \sum_{s \in  \gS^{\pi}_H}  P^{\pi}_{H} (s) \lp \min\{1,  \widehat{P}^{\piE}_{H} (s) / P^{\piE}_H (s)\} -  \pi_H (a^1|s)  \rp, 
\end{align*}
where $c_{\ell, h}  = \min_{s, s^\prime \in \goodS} \{ \sP^{\pi} \lp s_{h} = s |s_{\ell} = s^\prime, a_{\ell} = a^{1} \rp \} $. The penultimate inequality follows \eqref{eq:case_one_result} and \eqref{eq:case_two_result}. In summary, we prove that for any $\pi \in \Pi^{\mathrm{opt}}$, we have
\begin{align*}
    &\quad f (\pi) - f(\piE) \\
    &\geq \sum_{h=1}^{H} \sum_{\ell=1}^{h-1} c_{\ell, h} \sum_{s \in \goodS} P^{\pi}_{\ell} (s) \lp 1 - \pi_{\ell} (a^{1}|s)  \rp + 2 \sum_{s \in  \gS^{\pi}_H}  P^{\pi}_{H} (s) \lp \min\{1,  \widehat{P}^{\piE}_{H} (s) / P^{\piE}_H (s)\} -  \pi_H (a^1|s)  \rp
    \\
    &\geq c (\pi) \lp \sum_{h=1}^{H} \sum_{\ell=1}^{h-1} \sum_{s \in \goodS} P^{\pi}_{\ell} (s) \lp 1 - \pi_{\ell} (a^{1}|s)  \rp + \sum_{s \in  \gS^{\pi}_H}  P^{\pi}_{H} (s) \lp \min\{1,  \widehat{P}^{\piE}_{H} (s) / P^{\piE}_H (s)\} -  \pi_H (a^1|s)  \rp  \rp.
\end{align*}
Here $c (\pi) = \min_{1 \leq \ell < h \leq H} c_{\ell, h} =  \min_{1 \leq \ell < h \leq H, s, s^\prime \in \goodS} \{ \sP^{\pi} \lp s_{h} = s |s_{\ell} = s^\prime, a_{\ell} = a^{1} \rp \}$. Since $\widebar{\pi} \in \Pi^{\mathrm{opt}}$, it holds that
\begin{align*}
    &\quad f (\widebar{\pi}) - f(\piE) \\
    &\geq c (\widebar{\pi}) \lp \sum_{h=1}^{H} \sum_{\ell=1}^{h-1} \sum_{s \in \goodS} P^{\widebar{\pi}}_{\ell} (s) \lp 1 - \widebar{\pi}_{\ell} (a^{1}|s)  \rp + \sum_{s \in  \gS^{\widebar{\pi}}_H}  P^{\widebar{\pi}}_{H} (s) \lp \min\{1,  \widehat{P}^{\piE}_{H} (s) / P^{\piE}_H (s)\} -  
    \widebar{\pi}_H (a^1|s)  \rp  \rp. 
\end{align*}
Combined with \eqref{eq:ail_objective_pi_bar_minus_piE}, we obtain
\begin{align*}
    c (\widebar{\pi}) \lp \sum_{h=1}^{H} \sum_{\ell=1}^{h-1} \sum_{s \in \goodS} P^{\widebar{\pi}}_{\ell} (s) \lp 1 - \widebar{\pi}_{\ell} (a^{1}|s)  \rp + \sum_{s \in  \gS^{\widebar{\pi}}_H}  P^{\widebar{\pi}}_{H} (s) \lp \min\{1,  \widehat{P}^{\piE}_{H} (s) / P^{\piE}_H (s)\} -  
    \widebar{\pi}_H (a^1|s)  \rp  \rp \leq \varepsilon_{\ail},
\end{align*}
which completes the whole proof.

\end{proof}
