# Supplementary material for: A Note on Target Q-learning For Solving Finite MDPs with A Generative Oracle
Source: arXiv:2203.11489 source file (2022-03-22)
Supplement: Supplementary file 6 [file open_problem.tex]

\section{Open Problem}
\label{appendix:open_problem}

To better understand the role of our research, we discuss the following related open problems.

\textbf{Function Approximation.} In this paper, we focus on the tabular MDPs, in which the one-hot feature is used. As a result, the lower bounds in \citep{rajaraman2020fundamental} imply that the dependence of $|\gS|$ is inevitable for all imitation learning algorithms if no additional information is provided. We note that MDPs with \dquote{low-rank} structures allow algorithms (including BC and AIL) to use function approximation to obtain better sample complexity; refer to the related work discussed in \cref{appendix:review_of_previous_work}. Typically, the refined sample complexity is expected to depend on the inherent dimension $d$ rather than $|\gS|$. This direction is orthogonal to our research since we mainly compare algorithms in terms of the horizon $H$, which is usually unrelated to function approximation. Nevertheless, it is interesting to extend our results under the function approximation setting; see the discussion in \cref{appendix:discussion_of_function_approximation}. 

\textbf{Representation Learning.} We firmly believe that GAIL beats FEM and GTAL for MuJoCo tasks because the former uses deep neural networks to learn a good feature representation while the latter uses pre-specified features. However, these methods do not make a big difference under the tabular MDPs in terms of the sample complexity. It would be valuable to investigate this direction under the feature learning framework (see e.g., \citep{uehara2021representation}).
