# Supplementary material for: A Note on Target Q-learning For Solving Finite MDPs with A Generative Oracle
Source: arXiv:2203.11489 source file (2022-03-22)
Supplement: Supplementary file 7 [file proof_tail.tex]

\section{Proof of Results in Section \ref{sec:beyond_vanilla_ail}}
\label{appendix:proof_beyond_vanilla_ail}

\subsection{Proof of Theorem \ref{theorem:final_sample_complexity}}
\label{appendix:proof_of_theorem:final_sample_complexity}

Before we prove Theorem \ref{theorem:final_sample_complexity}, we first state three key lemmas: Lemma \ref{lemma:regret_of_ogd}, and Lemma \ref{lemma:approximate-minimax}, and \cref{lemma:sample_complexity_of_new_estimator_known_transition}.
\begin{lem}\label{lemma:regret_of_ogd}
Consider the adversarial imitation learning approach displayed in Algorithm \ref{algo:main_aglorithm}, then we have
\begin{align*}
    \sum_{t=1}^T f^{(t)} \lp w^{(t)} \rp - \min_{w \in \gW} \sum_{t=1}^T f^{(t)} (w) \leq 2H \sqrt{2 |\gS| |\gA| T},
\end{align*}
where $f^{(t)}(w) = \sum_{h=1}^{H} \sum_{(s, a) \in \gS \times \gA} w_h(s, a) ( P^{\pi^{(t)}}_h (s, a) - \widetilde{P}^{\piE}_h (s, a) )$.
\end{lem}

Refer to \cref{appendix:proof_lemma_regret_of_ogd} for the proof. Basically, \cref{lemma:regret_of_ogd} is a direct consequence of the regret bound of online gradient descent \citep{shalev12online-learning}.

\begin{lem} \label{lemma:approximate-minimax}
Consider the transition-aware adversarial imitation learning approach displayed in Algorithm \ref{algo:main_aglorithm} and $\widebar{\pi}$ is the output policy, then we have
\begin{align*}
\sum_{h=1}^H \lnorm P^{\widebar{\pi}}_h - \widetilde{P}^{\piE}_h \rnorm_{1} \leq \min_{\pi \in \Pi} \sum_{h=1}^H \lnorm P^{\pi}_h - \widetilde{P}^{\piE}_h \rnorm_{1} + 2 H \sqrt{\frac{2 |\gS| |\gA|}{T}} + \varepsilon_{\mathrm{opt}}. 
\end{align*}
\end{lem}

Refer to \cref{appendix:proof_lemma_approximate_minimax} for the proof. In particular, \cref{lemma:approximate-minimax} provides the guarantee of online gradient descent for the approximate saddle point optimization (i.e., the min-max optimization in \eqref{eq:new_algo_max_min}).

\begin{lem}
\label{lemma:sample_complexity_of_new_estimator_known_transition}
Consider $\gD$ is randomly divided into two subsets, i.e., $\gD = \gD_{1} \cup \gD_{1}^c$ with $\labs \gD_1 \rabs = \labs \gD_1^{c} \rabs = m / 2$. Fix $\varepsilon \in (0, H)$ and $\delta \in (0, 1)$; suppose $H \geq 5$. Consider the estimator in \eqref{eq:new_estimator}, if the number of trajectories ($m$) satisfies
\begin{align*}
  m \succsim   \frac{  | \gS | H^{3/2}}{\varepsilon} \log\lp  \frac{ |\gS| H}{\delta} \rp ,
\end{align*}
then with probability at least $1-\delta$, we have $\sum_{h=1}^H \Vert \widetilde{P}^{\piE}_h - P^{\piE}_h  \Vert_1 \leq \varepsilon$.
\end{lem}

Refer to \cref{appendix:proof_lemma_sample_complexity_of_new_estimator_known_transition} for the proof. The proof relies on the fine-grained analysis of \citep[Lemma A.12]{rajaraman2020fundamental}. Specifically, \cref{lemma:sample_complexity_of_new_estimator_known_transition} indicates a better sample complexity of the new estimator in \eqref{eq:new_estimator}.

\begin{proof}[Proof of Theorem \ref{theorem:final_sample_complexity}]
Let $\widebar{\pi}$ be the policy output by Algorithm \ref{algo:main_aglorithm}. With Lemma \ref{lemma:approximate-minimax}, we establish the upper bound on the $\ell_1$ deviation between $P^{\widebar{\pi}}_h (s, a)$ and $\widetilde{P}^{\piE}_h(s, a)$. 
\begin{align*}
    \sum_{h=1}^H \lnorm P^{\widebar{\pi}}_h  - \widetilde{P}^{\piE}_h \rnorm_{1} \leq \min_{\pi \in \Pi} \sum_{h=1}^H \lnorm P^{\pi}_h  - \widetilde{P}^{\piE}_h \rnorm_{1} + 2 H \sqrt{\frac{2 |\gS| |\gA|}{T}} + \varepsilon_{\mathrm{opt}}. 
\end{align*}
Since $\piE \in \Pi$, we further obtain that
\begin{align*}
    \sum_{h=1}^H \lnorm P^{\widebar{\pi}}_h  - \widetilde{P}^{\piE}_h \rnorm_{1} \leq \sum_{h=1}^H \lnorm P^{\piE}_h - \widetilde{P}^{\piE}_h \rnorm_{1} + 2 H \sqrt{\frac{2 |\gS| |\gA|}{T}} + \varepsilon_{\mathrm{opt}}.
\end{align*}
By \cref{lemma:sample_complexity_of_new_estimator_known_transition}, fix $\varepsilon \in (0, H)$ and $\delta \in (0, 1)$, when the number of trajectories in $\gD$ satisfies that $m \succsim | \gS | H^{3/2} \log\lp  |\gS| H / \delta \rp / \varepsilon $, with probability at least $1-\delta$, we have
\begin{align*}
    \sum_{h=1}^H \lnorm P^{\piE}_h - \widetilde{P}^{\piE}_h \rnorm_{1} \leq \frac{\varepsilon}{8}.
\end{align*}
Moreover, with $T \succsim |\gS| |\gA| H^2 / \varepsilon^2$ and $\varepsilon_{\mathrm{opt}} \leq \varepsilon / 2$, we can obtain that
\begin{align*}
    \sum_{h=1}^H \lnorm P^{\widebar{\pi}}_h - \widetilde{P}^{\piE}_h \rnorm_{1} \leq \frac{\varepsilon}{8} + \frac{\varepsilon}{4} + \varepsilon_{\mathrm{opt}} \leq \frac{7\varepsilon}{8}.
\end{align*}
Finally, with the dual representation of policy value, we can upper bound the policy value gap by the state-action distribution error.
\begin{align*}
    \left\vert V^{\piE} - V^{\bar{\pi}} \right\vert &= \left\vert \sum_{h=1}^H \sum_{(s, a) \in \gS \times \gA} \lp P^{\piE}_h (s, a) - P^{\widebar{\pi}}_h (s, a) \rp r_h (s, a) \right\vert
    \\
    &\leq \sum_{h=1}^H \lnorm P^{\piE}_h - P^{\widebar{\pi}}_h \rnorm_1
    \\
    &\leq \sum_{h=1}^H \lnorm P^{\piE}_h - \widetilde{P}^{\piE}_h \rnorm_1 + \sum_{h=1}^H \lnorm \widetilde{P}^{\piE}_h - P^{\widebar{\pi}}_h \rnorm_1
    \\
    &\leq \frac{\varepsilon}{8} + \frac{7\varepsilon}{8} = \varepsilon.
\end{align*}
\end{proof}

\subsection{Proof of Proposition \ref{prop:connection}}
\label{subsec:proof_of_proposition_connection}

\begin{proof}

Let $\widetilde{P}^{\piE}_h(s, a)$ be an expert state-action distribution estimator and $\widehat{\gP}$ be a transition model learned by a reward-free method. We define the following two events.
\begin{align*}
    &E_{\mathrm{EST}}:= \lb \sum_{h=1}^H \lnorm \widetilde{P}^{\piE}_h - P^{\piE}_h  \rnorm_{1} \leq \varepsilon_{\mathrm{EST}} \rb,
    \\
    & E_{\mathrm{RFE}}:= \lb \forall r: \gS \times \gA \rar [0, 1], \pi \in \Pi, \left\vert V^{\pi, \gP, r} - V^{\pi, \widehat{\gP}, r} \right\vert \leq \varepsilon_{\mathrm{RFE}} \rb. 
\end{align*}
According to assumption $(a)$ and $(b)$, we have that $\sP \lp E_{\mathrm{EST}}  \rp \geq 1 - \delta_{\mathrm{EST}}$ and $\sP \lp E_{\mathrm{RFE}}  \rp \geq 1 - \delta_{\mathrm{RFE}}$. Applying union bound yields
\begin{align*}
    \sP \lp E_{\mathrm{EST}}  \cap E_{\mathrm{RFE}} \rp \geq 1 - \delta_{\mathrm{EST}} -  \delta_{\mathrm{RFE}}.
\end{align*}
The following analysis is established on the event $E_{\mathrm{EST}}  \cap E_{\mathrm{RFE}}$. Let $\widebar{\pi}$ be the output of Algorithm \ref{algo:framework}.
\begin{align*}
    \left\vert V^{\piE, \gP} - V^{\widebar{\pi}, \gP} \right\vert \leq \left\vert V^{\piE, \gP} - V^{\widebar{\pi}, \widehat{\gP}} \right\vert + \left\vert V^{\widebar{\pi}, \widehat{\gP}} - V^{\widebar{\pi}, \gP} \right\vert \leq \left\vert V^{\piE, \gP} - V^{\widebar{\pi}, \widehat{\gP}} \right\vert + \varepsilon_{\mathrm{RFE}}. 
\end{align*}
The last inequality follows the event $E_{\mathrm{RFE}}$. Then we consider the error $\vert V^{\piE, \gP} - V^{\widebar{\pi}, \widehat{\gP}} \vert$. From the dual form of the policy value in \cref{lemma:policy_dual_value}, we have that
\begin{align*}
    \left\vert V^{\piE, \gP} - V^{\widebar{\pi}, \widehat{\gP}} \right\vert &= \left\vert \sum_{h=1}^H \sum_{(s, a) \in \gS \times \gA} \lp P^{\piE, \gP}_h (s, a) - P^{\widebar{\pi}, \widehat{\gP}}_h (s, a) \rp r_h (s, a)  \right\vert \leq \sum_{h=1}^H \lnorm P^{\piE, \gP}_h - P^{\widebar{\pi}, \widehat{\gP}}_h   \rnorm_1,
\end{align*}
where $P^{\widebar{\pi}, \widehat{\gP}}_h (s, a)$ is the state-action distribution of the policy $\widebar{\pi}$ under the transition model $\widehat{\gP}$. Then we get that
\begin{align*}
    \sum_{h=1}^H \lnorm P^{\piE, \gP}_h - P^{\widebar{\pi}, \widehat{\gP}}_h   \rnorm_1 & \leq \sum_{h=1}^H \lnorm P^{\piE, \gP}_h - \widetilde{P}^{\piE}_h   \rnorm_1 + \sum_{h=1}^H \lnorm \widetilde{P}^{\piE}_h - P^{\widebar{\pi}, \widehat{\gP}}_h   \rnorm_1
    \\
    &\leq \varepsilon_{\mathrm{EST}} + \sum_{h=1}^H \lnorm \widetilde{P}^{\piE}_h - P^{\widebar{\pi}, \widehat{\gP}}_h   \rnorm_1. 
\end{align*}
The last inequality follows the event $E_{\mathrm{EST}}$. Combining the above three inequalities yields
\begin{align*}
    \left\vert V^{\piE, \gP} - V^{\widebar{\pi}, \gP} \right\vert \leq \sum_{h=1}^H \lnorm \widetilde{P}^{\piE}_h - P^{\widebar{\pi}, \widehat{\gP}}_h   \rnorm_1 + \varepsilon_{\mathrm{EST}} +  \varepsilon_{\mathrm{RFE}}.
\end{align*}
According to assumption $(c)$, with the estimator $\widetilde{P}^{\piE}_h (s, a)$ and transition model $\widehat{\gP}$, algorithm B solves the projection problem in \eqref{eq:l1_norm_imitation_with_estimator} up to an error $\varepsilon_{\mathrm{AIL}}$ and $\widebar{\pi}$ is the output of the algorithm B. Formally,
\begin{align*}
    \sum_{h=1}^H \lnorm \widetilde{P}^{\piE}_h - P^{\widebar{\pi}, \widehat{\gP}}_h   \rnorm_1 \leq \min_{\pi \in \Pi} \sum_{h=1}^H \lnorm \widetilde{P}^{\piE}_h - P^{\pi, \widehat{\gP}}_h   \rnorm_1 + \varepsilon_{\mathrm{AIL}}.
\end{align*}
Then we get that
\begin{align*}
    \left\vert V^{\piE, \gP} - V^{\widebar{\pi}, \gP} \right\vert &\leq \sum_{h=1}^H \lnorm \widetilde{P}^{\piE}_h - P^{\widebar{\pi}, \widehat{\gP}}_h   \rnorm_1 + \varepsilon_{\mathrm{EST}} +  \varepsilon_{\mathrm{RFE}}
    \\
    &\leq \min_{\pi \in \Pi} \sum_{h=1}^H \lnorm \widetilde{P}^{\piE}_h - P^{\pi, \widehat{\gP}}_h  \rnorm_1 +  \varepsilon_{\mathrm{AIL}} + \varepsilon_{\mathrm{EST}} +  \varepsilon_{\mathrm{RFE}}
    \\
    &\overset{(1)}{\leq} \sum_{h=1}^H \lnorm \widetilde{P}^{\piE}_h - P^{\piE, \widehat{\gP}}_h   \rnorm_1 +  \varepsilon_{\mathrm{AIL}} + \varepsilon_{\mathrm{EST}} +  \varepsilon_{\mathrm{RFE}}
    \\
    &\leq \sum_{h=1}^H \lnorm \widetilde{P}^{\piE}_h - P^{\piE, \gP}_h   \rnorm_1 + \sum_{h=1}^H \lnorm P^{\piE, \gP}_h - P^{\piE, \widehat{\gP}}_h   \rnorm_1  +  \varepsilon_{\mathrm{AIL}} + \varepsilon_{\mathrm{EST}} +  \varepsilon_{\mathrm{RFE}}
    \\
    &\overset{(2)}{\leq} \sum_{h=1}^H \lnorm P^{\piE, \gP}_h - P^{\piE, \widehat{\gP}}_h   \rnorm_1  +  \varepsilon_{\mathrm{AIL}} + 2\varepsilon_{\mathrm{EST}} +  \varepsilon_{\mathrm{RFE}},
\end{align*}
where inequality $(1)$ holds since $\piE \in \Pi$ and inequality $(2)$ follows the event $E_{\mathrm{EST}}$. With the dual representation of $\ell_1$-norm, we have that
\begin{align*}
    \sum_{h=1}^H \lnorm P^{\piE, \gP}_h - P^{\piE, \widehat{\gP}}_h \rnorm_1 &= \max_{w \in \gW} \sum_{h=1}^H w_h (s, a) \lp P^{\piE, \gP}_h (s, a) - P^{\piE, \widehat{\gP}}_h (s, a)  \rp
    \\
    &= \max_{w \in \gW} V^{\piE, \gP, w} - V^{\piE, \widehat{\gP}, w} \leq \varepsilon_{\mathrm{RFE}},
\end{align*}
where $\gW = \{w: \|w \|_{\infty} \leq 1 \}$, $V^{\piE, \widehat{\gP}, w}$ is the value of policy $\piE$ with the transition model $\widehat{\gP}$ and reward function $w$. The last inequality follows the event $E_{\mathrm{RFE}}$. Then we prove that
\begin{align*}
    \left\vert V^{\piE, \gP} - V^{\widebar{\pi}, \gP} \right\vert \leq  2\varepsilon_{\mathrm{EST}} + 2 \varepsilon_{\mathrm{RFE}} + \varepsilon_{\mathrm{AIL}}. 
\end{align*}

\end{proof}

\subsection{Proof of Theorem \ref{theorem:sample-complexity-unknown-transition}}
\label{subsection:proof-of-theorem-sample-complexity-unknown-transition}

Before we prove \cref{theorem:sample-complexity-unknown-transition}, we first explain the modified estimator in \eqref{eq:new_estimator_unknown_transition}. In particular, we demonstrate it is an unbiased estimator under the unknown transition setting and present its sample complexity and interaction complexity. Then, we review the theoretical guarantee of the RF-Express algorithm.

We consider the decomposition of $P_h^{\piE} (s, a)$.
\begin{align*} 
P_h^{\piE}(s, a) &= {\sum_{\tr_h \in \Tr_h^{\gD_1}} \sP^{\piE}(\tr_h) \indict\lb \tr_h(s_h, a_h) = (s, a) \rb} + {\sum_{\tr_h \notin \Tr_h^{\gD_1}} \sP^{\piE}(\tr_h) \indict\lb \tr_h(s_h, a_h) = (s, a) \rb}
\\
&= {\sum_{\tr_h \in \Tr_h^{\gD_1}} \sP^{\pi}(\tr_h) \indict\lb \tr_h(s_h, a_h) = (s, a) \rb} + {\sum_{\tr_h \notin \Tr_h^{\gD_1}} \sP^{\piE}(\tr_h) \indict\lb \tr_h(s_h, a_h) = (s, a) \rb},
\end{align*}
where $\pi \in \Pi_{\text{BC}} \lp \gD_1 \rp$ and the last equality follows Lemma \ref{lemma:unknown-transition-unbiased-estimation}. Recall the definition of the new estimator.
\begin{align*}
\widetilde{P}_h^{\piE} (s, a) = {\frac{\sum_{\tr_h \in \gD^\prime_{\mathrm{env}}} \indict \{ \tr_h (s_h, a_h) = (s, a), \tr_h \in \Tr_h^{\gD_1} \}}{|\gD^\prime_{\mathrm{env}}|}} + {\frac{  \sum_{\tr_h \in \gD_1^c}  \indict\{ \tr_h (s_h, a_h) = (s, a), \tr_h \not\in \Tr_h^{\gD_1}  \} }{|\gD_1^c|}},
\end{align*}
where $\gD^\prime_{\mathrm{env}}$ is the dataset collected by the policy $\pi \in \Pi_{\text{BC}} (\gD_1)$. Notice that the two terms in RHS are Monte Carlo estimations of ${\sum_{\tr_h \in \Tr_h^{\gD_1}} \sP^{\pi}(\tr_h) \indict\lb \tr_h(s_h, a_h) = (s, a) \rb}$ and ${\sum_{\tr_h \notin \Tr_h^{\gD_1}} \sP^{\piE}(\tr_h) \indict\lb \tr_h(s_h, a_h) = (s, a) \rb}$ based on the dataset $\gD^\prime_{\mathrm{env}}$ and $\gD_1^c$, respectively. Therefore, $\widetilde{P}_h^{\piE} (s, a)$ is an unbiased estimation of $P_h^{\piE}(s, a)$.

\begin{lem} \label{lemma:unknown-transition-unbiased-estimation}
We define $\Pi_{\text{BC}} \lp \gD_1 \rp$ as the set of policies, each of which takes expert action on states contained in $\gD_{1}$. For each $\pi \in \Pi_{\text{BC}} \lp \gD_{1} \rp$, $\forall h \in [H]$ and $(s, a) \in \gS \times \gA$, we have
\begin{align*}
    &\sum_{\tr_h \in \Tr_h^{\gD_1}} \sP^{\piE}(\tr_h) \indict\lb \tr_h(s_h, a_h) = (s, a) \rb = \sum_{\tr_h \in \Tr_h^{\gD_1}} \sP^{\pi}(\tr_h) \indict\lb \tr_h(s_h, a_h) = (s, a) \rb.
\end{align*}
\end{lem}

\begin{proof}
Let $\Pi_{\text{BC}} \lp \gD_1 \rp$ denote the set of policies, each of which exactly takes expert action on states contained in $\gD_{1}$. Fix $\pi \in \Pi_{\text{BC}} \lp \gD_{1} \rp$, $h \in [H]$ and $(s, a) \in \gS \times \gA$, we consider the probability $\sP^{\piE} \lp \tr_h \rp$ of a truncated trajectory $\tr_h \in \Tr^{\gD_{1}}_h$. Since $\pi$ exactly takes expert action on states contained in $\gD_{1}$, we have
\begin{align*}
    &\quad \sP^{\piE}(\tr_h) \\
    &= \rho (\tr_h(s_1)) \piE_1 \lp \tr_h(a_1)| \tr(s_1) \rp \prod_{\ell=1}^{h-1}  P_{\ell} \lp \tr_h(s_{\ell+1}) | \tr_h(s_{\ell}), \tr_h(a_{\ell}) \rp \piE_{\ell+1} \lp \tr_h(a_{\ell+1}) | \tr_h(s_{\ell+1}) \rp
    \\
    &= \rho (\tr_h(s_1)) \pi_1 \lp \tr_h(a_1)| \tr(s_1) \rp \prod_{\ell=1}^{h-1}  P_{\ell} \lp \tr_h(s_{\ell+1}) | \tr_h(s_{\ell}), \tr_h(a_{\ell}) \rp \pi_{\ell+1} \lp \tr_h(a_{\ell+1}) | \tr_h(s_{\ell+1}) \rp
    \\
    &= \sP^{\pi}(\tr_h).
\end{align*}
Therefore, we obtain that
\begin{align*}
    \sum_{\tr_h \in \Tr_h^{\gD_1}} \sP^{\piE}(\tr_h) \indict\lb \tr_h(s_h, a_h) = (s, a) \rb = \sum_{\tr_h \in \Tr_h^{\gD_1}} \sP^{\pi}(\tr_h) \indict\lb \tr_h(s_h, a_h) = (s, a) \rb,
\end{align*}
which completes the proof.
\end{proof}

The sample complexity and interaction complexity of the estimator \eqref{eq:new_estimator_unknown_transition} are given in the following \cref{lemma:sample_complexity_of_new_estimator_unknown_transition}.

\begin{lem} \label{lemma:sample_complexity_of_new_estimator_unknown_transition}
Given expert dataset $\gD$ and $\gD$ is divided into two equal subsets, i.e., $\gD = \gD_{1} \cup \gD_{1}^c$ with $\labs \gD_1 \rabs = \labs \gD_1^{c} \rabs = m / 2$. Fix $\pi \in \Pi_{\text{BC}} \lp \gD_1 \rp$, let $\gD^\prime_{\mathrm{env}}$ be the dataset collected by $\pi$ and $|\gD^\prime_{\mathrm{env}} | = n^\prime$. Fix $\varepsilon \in (0, 1)$ and $\delta \in (0, 1)$; suppose $H \geq 5$. Consider the estimator $\widetilde{P}^{\piE}_h$ shown in \eqref{eq:new_estimator_unknown_transition}, if the number of expert trajectories ($m$) and the number of interaction trajectories in $\gD^\prime_{\mathrm{env}}$ for estimation ($n^\prime$) satisfy
\begin{align*}
    m \succsim   \frac{| \gS | H^{3/2}  }{\varepsilon} \log\lp  \frac{|\gS| H}{\delta} \rp, \; n^\prime \succsim \frac{ | \gS |H^{2}}{\varepsilon^2} \log\lp  \frac{|\gS| H}{\delta} \rp,
\end{align*}
then with probability at least $1-\delta$, we have
\begin{align*}
    \sum_{h=1}^H \lnorm \widetilde{P}^{\piE}_h - P^{\piE}_h  \rnorm_{1} \leq \varepsilon.
\end{align*}
\end{lem}

Refer to \cref{appendix:proof_lemma_sample_complexity_of_new_estimator_unknown_transition} for the proof. The proof is based on \cref{lemma:sample_complexity_of_new_estimator_known_transition} and \cref{lemma:unknown-transition-unbiased-estimation}.

Next, we state the theoretical guarantee of \textnormal{RF-Express} algorithm~\citep{menard20fast-active-learning}, which corresponds to assumption $(a)$ in Proposition \ref{prop:connection}.

\begin{thm}[Theorem 1 in ~\citep{menard20fast-active-learning}] \label{theorem:rf_express_sample_complexity}
Fix $\varepsilon \in \lp 0, 1 \rp$ and $\delta \in (0, 1)$. Consider the RF-Express algorithm and $\widehat{\gP}$ is the empirical transition function built on the collected trajectories, if the number of trajectories collected by RF-Express ($n$) satisfies 
\begin{align*}
    n \succsim  \frac{ |\gS| |\gA| H^{3} }{\varepsilon^2}    \lp |\gS| + \log\lp\frac{|\gS| H}{\delta} \rp \rp.
\end{align*}
Then with probability at least $1-\delta$, for any policy $\pi$ and any bounded reward function $w$ between $[-1, 1]$, we have\footnote{This is implied by the stopping rule in RF-Express algorithm and Lemma 1 in \citep{menard20fast-active-learning}.} $| V^{\pi, \gP, w} - V^{\pi, \widehat{\gP}, w} | \leq {\varepsilon}/{2}$; furthermore, for any bounded reward function $w$ between $[-1, 1]$, we have $ \max_{\pi \in \Pi} V^{\pi, w} \leq V^{\widehat{\pi}_{w}^{*}, w} + \varepsilon$, where $\widehat{\pi}_{w}^{*}$ is the optimal policy under empirical transition function $\widehat{\gP}$ and reward function $w$.
\end{thm}

In the following part, we formally prove \cref{theorem:sample-complexity-unknown-transition}. The proof combines \cref{prop:connection}, \cref{lemma:sample_complexity_of_new_estimator_unknown_transition}, and \cref{theorem:rf_express_sample_complexity}.

\begin{proof}[Proof of \cref{theorem:sample-complexity-unknown-transition}]
When the number of trajectories collected by \textnormal{RF-Express} satisfies
\begin{align*}
    n \succsim  \frac{ |\gS| |\gA| H^{3} }{\varepsilon^2}    \lp |\gS| + \log\lp\frac{|\gS| H}{\delta} \rp \rp,
\end{align*}
for any policy $\pi \in \Pi$ and reward function $w : \gS \times \gA \rar [0, 1]$, with probability at least $1-\delta/2$, $| V^{\pi, \gP, w} - V^{\pi, \widehat{\gP}, w} | \leq \varepsilon / 16 = \varepsilon_{\text{RFE}}$. In a word, the assumption $(a)$ in Proposition \ref{prop:connection} holds with $\delta_{\mathrm{RFE}} = \delta / 2$ and $\varepsilon_{\mathrm{RFE}} = \varepsilon / 16$.

Secondly, we note that the ku $(b)$ in Proposition \ref{prop:connection} holds by Lemma \ref{lemma:sample_complexity_of_new_estimator_unknown_transition}. More concretely, if the expert sample complexity and interaction complexity satisfies
\begin{align*}
    m \succsim   \frac{ | \gS | H^{3/2} }{\varepsilon} \log\lp  \frac{|\gS| H}{\delta} \rp, \; n^\prime \succsim \frac{ | \gS | H^{2}}{\varepsilon^2} \log\lp  \frac{|\gS| H}{\delta} \rp,
\end{align*}
with probability at least $1-\delta/2$, $\sum_{h=1}^H \Vert \widetilde{P}^{\piE}_h - P^{\piE}_h  \Vert_{1} \leq \varepsilon / 16 = \varepsilon_{\text{EST}}$. Hence, the assumption $(b)$ in Proposition \ref{prop:connection} holds with $\delta_{\mathrm{EST}} = \delta / 2$ and $\varepsilon_{\mathrm{EST}} = \varepsilon / 16$.

Thirdly, we aim to verify that the assumption $(c)$ in Proposition \ref{prop:connection} holds with $\widetilde{P}^{\piE}_h (s, a)$ and $\widehat{\gP}$. With the dual representation of $\ell_1$-norm and the minimax theorem, we get that
\begin{align*}
    \min_{\pi \in \Pi} \sum_{h=1}^H \lnorm P^{\pi, \widehat{\gP}}_h - \widetilde{P}^{\piE}_h \rnorm_{1} = - \min_{w \in \gW} \max_{\pi \in \Pi} \sum_{h=1}^H \sum_{(s, a) \in \gS \times \gA} w_h (s, a) \lp P^{\pi, \widehat{\gP}}_h (s, a) -  \widetilde{P}^{\piE}_h(s, a) \rp.
\end{align*}
Recall that $w^{(t)}$ is the reward function inferred by MB-TAIL in the iteration $t$. Then we have
\begin{align*}
    &\quad \min_{w \in \gW} \max_{\pi \in \Pi} \sum_{h=1}^H \sum_{(s, a) \in \gS \times \gA} w_h (s, a) \lp P^{\pi, \widehat{\gP}}_h (s, a) -  \widetilde{P}^{\piE}_h(s, a) \rp
    \\
    &\leq \max_{\pi \in \Pi} \sum_{h=1}^H \sum_{(s, a) \in \gS \times \gA} \lp \frac{1}{T} \sum_{t=1}^T w_h^{(t)} (s, a) \rp \lp P^{\pi, \widehat{\gP}}_h (s, a) -  \widetilde{P}^{\piE}_h(s, a) \rp
    \\
    &=  \max_{\pi \in \Pi} \frac{1}{T} \sum_{t=1}^T \sum_{h=1}^H \sum_{(s, a) \in \gS \times \gA}   w_h^{(t)} (s, a) \lp P^{\pi, \widehat{\gP}}_h (s, a) -  \widetilde{P}^{\piE}_h(s, a) \rp
    \\
    &\leq  \frac{1}{T} \sum_{t=1}^T \max_{\pi \in \Pi} \sum_{h=1}^H \sum_{(s, a) \in \gS \times \gA}   w_h^{(t)} (s, a) \lp P^{\pi, \widehat{\gP}}_h (s, a) -  \widetilde{P}^{\piE}_h(s, a) \rp
    \\
    &\leq \frac{1}{T} \sum_{t=1}^T \sum_{h=1}^H \sum_{(s, a) \in \gS \times \gA}   w_h^{(t)} (s, a) \lp P^{\pi^{(t)}, \widehat{\gP}}_h (s, a) -  \widetilde{P}^{\piE}_h(s, a) \rp + \varepsilon_{\text{opt}}.
\end{align*}
In the last inequality, the policy $\pi^{(t)}$ is the nearly optimal policy w.r.t $w^{(t)}$ and $\widehat{\gP}$ up to an error of $\varepsilon_{\text{opt}}$. Then we have that
\begin{align*}
    &\quad \min_{\pi \in \Pi} \sum_{h=1}^H \lnorm P^{\pi, \widehat{\gP}}_h - \widetilde{P}^{\piE}_h \rnorm_{1}
    \\
    &\geq -\frac{1}{T} \sum_{t=1}^T \sum_{h=1}^H \sum_{(s, a) \in \gS \times \gA}   w_h^{(t)} (s, a) \lp P^{\pi^{(t)}, \widehat{\gP}}_h (s, a) -  \widetilde{P}^{\piE}_h(s, a) \rp - \varepsilon_{\text{opt}}
    \\
    &\geq \frac{1}{T} \max_{w \in \gW} \sum_{t=1}^T \sum_{h=1}^H \sum_{(s, a) \in \gS \times \gA}   w_h (s, a) \lp P^{\pi^{(t)}, \widehat{\gP}}_h (s, a) -  \widetilde{P}^{\piE}_h(s, a) \rp - \varepsilon_{\text{opt}} - 2H \sqrt{\frac{2 \vert \gS \vert \vert \gA \vert}{T}}. 
\end{align*}
Note that the reward function $w^{(t)}$ is updated by online projected gradient descent with objective function $f^{(t)} (w) = \sum_{h=1}^H \sum_{(s, a) \in \gS \times \gA}   w_h (s, a) ( P^{\pi^{(t)}, \widehat{\gP}}_h (s, a) -  \widetilde{P}^{\piE}_h(s, a) )$. Hence, the last inequality follows Lemma \ref{lemma:regret_of_ogd}. Then we have that
\begin{align*}
    &\quad \min_{\pi \in \Pi} \sum_{h=1}^H \lnorm P^{\pi, \widehat{\gP}}_h - \widetilde{P}^{\piE}_h \rnorm_{1}
    \\
    &\geq \frac{1}{T} \max_{w \in \gW} \sum_{t=1}^T \sum_{h=1}^H \sum_{(s, a) \in \gS \times \gA}   w_h (s, a) \lp P^{\pi^{(t)}, \widehat{\gP}}_h (s, a) -  \widetilde{P}^{\piE}_h(s, a) \rp - \varepsilon_{\text{opt}} - 2H \sqrt{\frac{2 \vert \gS \vert \vert \gA \vert}{T}}
    \\
    &=  \max_{w \in \gW}  \sum_{h=1}^H \sum_{(s, a) \in \gS \times \gA}   w_h (s, a) \lp \frac{1}{T} \sum_{t=1}^T P^{\pi^{(t)}, \widehat{\gP}}_h (s, a) -  \widetilde{P}^{\piE}_h(s, a) \rp - \varepsilon_{\text{opt}} - 2H \sqrt{\frac{2 \vert \gS \vert \vert \gA \vert}{T}}
    \\
    &= \max_{w \in \gW}  \sum_{h=1}^H \sum_{(s, a) \in \gS \times \gA}   w_h (s, a) \lp P^{\widebar{\pi}, \widehat{\gP}}_h (s, a) -  \widetilde{P}^{\piE}_h(s, a) \rp - \varepsilon_{\text{opt}} - 2H \sqrt{\frac{2 \vert \gS \vert \vert \gA \vert}{T}}
    \\
    &= \sum_{h=1}^H \lnorm P^{\widebar{\pi}, \widehat{\gP}}_h - \widetilde{P}^{\piE}_h \rnorm_{1} - \varepsilon_{\text{opt}} - 2H \sqrt{\frac{2 \vert \gS \vert \vert \gA \vert}{T}}.
\end{align*}
When $\varepsilon_{\text{opt}} \leq \varepsilon / 2$ and $T \succsim |\gS| |\gA| H^2 / \varepsilon^2$ such that $2 H \sqrt{2 |\gS| |\gA| / T} \leq \varepsilon / 4$, we have that
\begin{align*}
    \sum_{h=1}^H \lnorm P^{\widebar{\pi}, \widehat{\gP}}_h - \widetilde{P}^{\piE}_h \rnorm_{1} - \min_{\pi \in \Pi} \sum_{h=1}^H \lnorm P^{\pi, \widehat{\gP}}_h - \widetilde{P}^{\piE}_h \rnorm_{1} \leq \frac{3\varepsilon}{4}  = \varepsilon_{\mathrm{AIL}}.
\end{align*}
Therefore, the assumption $(c)$ in Proposition \ref{prop:connection} holds with $\varepsilon_{\mathrm{AIL}} = 3\varepsilon / 4H$. Now, we summarize the conditions what we have obtained.
\begin{itemize}
    \item The assumption $(a)$ in Proposition \ref{prop:connection} holds with $\delta_{\mathrm{RFE}} = \delta / 2$ and $\varepsilon_{\mathrm{RFE}} = \varepsilon / 16$.
    \item The assumption $(b)$ in Proposition \ref{prop:connection} holds with $\delta_{\mathrm{EST}} = \delta / 2$ and $\varepsilon_{\mathrm{EST}} = \varepsilon / 16$.
    \item The assumption $(c)$ in Proposition \ref{prop:connection} holds with $\varepsilon_{\mathrm{AIL}} = 3\varepsilon / 4$. 
\end{itemize}
Applying Proposition \ref{prop:connection} finishes the proof. With probability at least $1-\delta$,
\begin{align*}
    V^{\piE} - V^{\widebar{\pi}} \leq 2 \varepsilon_{\mathrm{RFE}} + 2 \varepsilon_{\mathrm{EST}} + \varepsilon_{\mathrm{AIL}} = \varepsilon.  
\end{align*}

\end{proof}
