# Supplementary material for: A Note on Target Q-learning For Solving Finite MDPs with A Generative Oracle
Source: arXiv:2203.11489 source file (2022-03-22)
Supplement: Supplementary file 8 [file proof_vail.tex]

\section{Proof of Results in Section \ref{sec:generalization_of_ail}}
\label{appendix:proof_generalization_ail}

\subsection{Proof of Theorem \ref{theorem:worst_case_sample_complexity_of_vail}}

First, we formally state the result on the worst-case sample complexity for \textsf{VAIL} to achieve a small policy value gap \emph{with high probability}. Notice that this result does not change too much compared with that \emph{in expectation}.

\begin{thm}[High Probability Version of \cref{theorem:worst_case_sample_complexity_of_vail}] \label{theorem:worst_case_sample_complexity_of_vail_high_prob}
For any tabular and episodic MDP, with probability at least $1-\delta$, to obtain an $\varepsilon$-optimal policy (i.e., $V^{\piE} -  V^{\piail} \leq \varepsilon$), \textsf{VAIL} in \eqref{eq:ail} requires at most $\widetilde{\gO} ( |\gS| H^2/\varepsilon^2)$ expert trajectories. 
\end{thm}

\begin{proof}[Proof of \cref{theorem:worst_case_sample_complexity_of_vail} and \cref{theorem:worst_case_sample_complexity_of_vail_high_prob}]

In the following part, we provide proof for both \cref{theorem:worst_case_sample_complexity_of_vail} and \cref{theorem:worst_case_sample_complexity_of_vail_high_prob}. To prove \cref{theorem:worst_case_sample_complexity_of_vail} and \cref{theorem:worst_case_sample_complexity_of_vail_high_prob}, we take two steps. For the first step, we extend \citep[Lemma 1]{xu2020error} from infinite-horizon MDPs to episodic MDPs. Suppose that $\piail$ is the optimal solution of the \textsf{VAIL} objective in \eqref{eq:ail}. We have the following re-formulation for policy value (see \cref{lemma:policy_dual_value}): 
\begin{align*}
    V^{\piail} = \sum_{h=1}^{H} \sum_{(s, a) \in \gS \times \gA} P^{\piail}_h(s, a) r_h(s, a).
\end{align*}
Then, we obtain the following decomposition for the policy value gap:
\begin{align*}
    V^{\piE} - V^{\piail} &= \sum_{h=1}^{H} \sum_{(s, a) \in \gS \times \gA} \lp P^{\piE}_h(s, a) - P^{\piail}_h(s, a) \rp r_h(s, a).
\end{align*}
Recall that $r_h(s, a) \in [0, 1]$ by assumption. It is straightforward to see that for the optimal solution $\piail$ to \textsf{VAIL}'s objective in \eqref{eq:ail}, we have 
\begin{align*}
    \labs  V^{\piE} - V^{\piail} \rabs &\leq \sum_{h=1}^{H}  \sum_{(s, a) \in \gS \times \gA} \labs P^{\piE}_h(s, a) - P^{\piail}_h(s, a) \rabs \\
    &\leq \sum_{h=1}^{H}  \sum_{(s, a) \in \gS \times \gA} \labs P^{\piE}_h(s, a) - \widehat{P}^{\piE}_h(s, a) \rabs + \sum_{h=1}^{H}  \sum_{(s, a) \in \gS \times \gA} \labs  \widehat{P}^{\piE}_h(s, a) - P^{\piail}_h(s, a) \rabs \\
    &\leq 2 \sum_{h=1}^{H}  \sum_{(s, a) \in \gS \times \gA} \labs P^{\piE}_h(s, a) - \widehat{P}^{\piE}_h(s, a) \rabs,
\end{align*}
where the last inequality holds because  
\begin{align*}
 \sum_{h=1}^{H}  \sum_{(s, a) \in \gS \times \gA} \labs  \widehat{P}^{\piE}_h(s, a) - P^{\piail}_h(s, a) \rabs &= \min_{\pi} \sum_{h=1}^{H}  \sum_{(s, a) \in \gS \times \gA} \labs P^{\pi}_h(s, a) - \widehat{P}^{\piE}_h(s, a) \rabs \\
 &\leq \sum_{h=1}^{H}  \sum_{(s, a) \in \gS \times \gA} \labs P^{\piE}_h(s, a) - \widehat{P}^{\piE}_h(s, a) \rabs.
\end{align*}
Notice that $\piE$ is deterministic and hence $P^{\piE}_h (s, a) = \widehat{P}^{\piE}_h (s, a) = 0$ for $a \not= \piE_h(s)$. Then we have that
\begin{align*}
    \labs  V^{\piE} - V^{\piail} \rabs &\leq 2\sum_{h=1}^{H}  \sum_{(s, a) \in \gS \times \gA} \labs P^{\piE}_h(s, a) - \widehat{P}^{\piE}_h(s, a) \rabs
    \\
    &= 2\sum_{h=1}^{H}  \sum_{s \in \gS } \labs P^{\piE}_h(s, \piE_h (s)) - \widehat{P}^{\piE}_h(s, \piE_h (s)) \rabs
    \\
    &= 2\sum_{h=1}^{H}  \sum_{s \in \gS } \labs P^{\piE}_h(s) - \widehat{P}^{\piE}_h(s) \rabs 
\end{align*}
For the second step, we upper bound the estimation error between $P^{\piE}_h(s)$ and $\widehat{P}^{\piE}_h(s)$. We first prove the sample complexity to achieve a small policy value gap with \emph{high probability}. 

\begin{lem}[Concentration Inequality for Total Variation Distance \citep{weissman2003inequalities}]  \label{lemma:l1_concentration}
Let $\gX = \{1, 2, \cdots, |\gX|\}$ be a finite set. Let $P$ be a distribution on $\gX$. Futhermore, let $\widehat{P}$ be the empirical distribution given $m$ i.i.d. samples $x_1, x_2, \cdots, x_m$ from $P$, i.e.,
\begin{align*}
    \widehat{P}(j) = \frac{1}{m} \sum_{i=1}^{m} \mathbb{I} \lb x_i = j \rb.
\end{align*}
Then, with probability at least $1-\delta$, we have that 
\begin{align*}
    \lnorm P - \widehat{P} \rnorm_1 := \sum_{x \in \gX} \labs P(x) - \widehat{P}(x) \rabs \leq \sqrt{\frac{2 |\gX| \ln(1/\delta) }{m}}.
\end{align*}
\end{lem}

It is clear that each $\widehat{P}^{\piE}_h(s)$ is an empirical estimation for $P^{\piE}_h(s)$. By \cref{lemma:l1_concentration}, for any fixed $h$, with probability at least $1-\delta$, we have that 
\begin{align*}
    \sum_{s \in \gS } \labs P^{\piE}_h(s) - \widehat{P}^{\piE}_h(s) \rabs \leq \sqrt{\frac{2 |\gS| \ln(1/\delta) }{m}},
\end{align*}
where $m$ is the number of expert trajectories in the dataset $\gD$. By a union bound over $h = 1, \cdots, H$, with probability at least $1-\delta$,  we have that 
\begin{align*}
    \sum_{h=1}^{H} \sum_{s \in \gS } \labs P^{\piE}_h(s) - \widehat{P}^{\piE}_h(s) \rabs \leq H\sqrt{\frac{2 |\gS| \ln(H/\delta) }{m}}.
\end{align*}
As a result, we obtain that with probability at least $1-\delta$ 
\begin{align*}
     \labs  V^{\piE} - V^{\piail} \rabs \leq 2H\sqrt{\frac{2 |\gS| \ln(H/\delta) }{m}},
\end{align*}
which translates to a sample complexity $\widetilde{\gO}( |\gS| H^2/\varepsilon^2)$ with high probability.

Second, we prove the corresponding sample complexity to achieve a small policy value gap \emph{in expectation}. With \citep[Theorem 1]{han2015minimax}, we can upper bound the expected $\ell-1$ risk of the maximum likelihood estimation.
\begin{align*}
    \forall h \in [H], \, \expect\ls \lnorm \widehat{P}^{\piE}_h - P^{\piE}_h   \rnorm_{1} \rs \leq \sqrt{ \frac{|\gS| - 1}{m}},
\end{align*}
where the expectation is taken w.r.t the randomness of expert demonstrations. For the expected policy value gap, we have 
\begin{align*}
     \expect \ls V^{\piE} - V^{\piail} \rs \leq H \sqrt{ \frac{|\gS| - 1}{m}}, 
\end{align*}
which translates to a sample complexity $\gO ( |\gS| H^2/\varepsilon^2)$ in expectation as in \cref{theorem:worst_case_sample_complexity_of_vail}.

\end{proof}

\subsection{Proof of Claim in Example \ref{example:ail_fail}}

In this part, we formally state and prove the theoretical result in \cref{example:ail_fail}.

\begin{claim} \label{claim:ail_standard_imitation}
Consider the MDP and expert demonstration configuration in \cref{example:ail_fail}. We have that $\piail (a^{1}|s^{1}) \in [0.8, 1.0], \piail (a^{1}|s^{2}) = 1$ are all globally optimal solutions of \eqref{eq:ail}. The largest policy value gap among all optimal solutions is $0.1$.  
\end{claim}

\begin{proof}[Proof of \cref{claim:ail_standard_imitation}]
The empirical distribution is calculated as
\begin{align*}
    \widehat{P}^{\piE} (s^{1}, a^{1}) = 0.4, \widehat{P}^{\piE} (s^{1}, a^{2}) = 0.0,
    \widehat{P}^{\piE} (s^{2}, a^{1}) = 0.6, \widehat{P}^{\piE} (s^{2}, a^{2}) = 0.0.
\end{align*}
With the above empirical distribution, we can obtain \textsf{VAIL}'s objective.
\begin{align*}
    &\quad \labs \widehat{P}^{\piE} (s^{1}, a^{1})  - \rho (s^{1}) \pi (a^{1}|s^{1})  \rabs + \labs \widehat{P}^{\piE} (s^{1}, a^{2}) - \rho (s^{1}) \lp 1-\pi (a^{1}|s^{1}) \rp \rabs
    \\
    &+ \labs \widehat{P}^{\piE} (s^{2}, a^{1}) - \rho (s^{2}) \pi (a^{1}|s^{2}) \rabs + \labs \widehat{P}^{\piE} (s^{2}, a^{2}) - \rho (s^{2}) \lp 1-\pi (a^{1}|s^{2}) \rp \rabs
    \\
    &= \labs 0.4 - 0.5 \pi (a^{1}|s^{1})  \rabs + \labs 0 - 0.5 \lp 1-\pi (a^{1}|s^{1}) \rp  \rabs + \labs 0.6 - 0.5 \pi (a^{1}|s^{2}) \rabs + \labs 0 - 0.5 \lp 1-\pi (a^{1}|s^{2}) \rp \rabs
    \\
    &= \labs 0.4 - 0.5 \pi (a^{1}|s^{1})  \rabs + 0.5 \lp 1-\pi (a^{1}|s^{1}) \rp + 1.1 -  \pi (a^{1}|s^{2}). 
\end{align*}
Notice that the optimization variables $\pi (a^{1}|s^{1}), \pi (a^{1}|s^{2})$ are independent and we can consider the optimization problem for each optimization variable. For $\pi (a^{1}|s^{1})$, we have that
\begin{align*}
    \piail (a^{1}|s^{1}) \in \argmin_{\pi (a^{1}|s^{1}) \in [0, 1]} \labs 0.4 - 0.5 \pi (a^{1}|s^{1})  \rabs - 0.5 \pi (a^{1}|s^{1}). 
\end{align*}
We apply \cref{lem:single_variable_opt_condition} with $a = 0.5$ and $c = 0.4$. We get that $\piail (a^{1}|s^{1}) \in [0.8, 1.0]$ is the optimal solution. For $\pi (a^{1}|s^{2})$, we have that
\begin{align*}
    \piail (a^{1}|s^{2}) \in \argmin_{\pi (a^{1}|s^{2}) \in [0, 1]} - \pi (a^{1}|s^{2}). 
\end{align*}
It is easy to see that $\piail (a^{1}|s^{2}) = 1$ is the optimal solution, which completes the proof.
\end{proof}

\subsection{Proof of Proposition \ref{proposition:ail_policy_value_gap_standard_imitation}}

In this part, we extend the result in \cref{claim:ail_standard_imitation} to the Standard Imitation MDPs shown in \cref{fig:bandit}. In Standard Imitation, all states are absorbing, $a^{1}$ is the expert action (in green) and $a^{2}$ is the non-expert action (in blue). The initial state distribution is denoted as $\rho$.    \cref{proposition:ail_policy_value_gap_standard_imitation} indicates that the largest policy value gap of \textsf{VAIL} \emph{equals} half of the estimation error and formally demonstrates the weak convergence issue of \textsf{VAIL}.

\begin{figure}[htbp]
\centering
\includegraphics[width=0.7\linewidth]{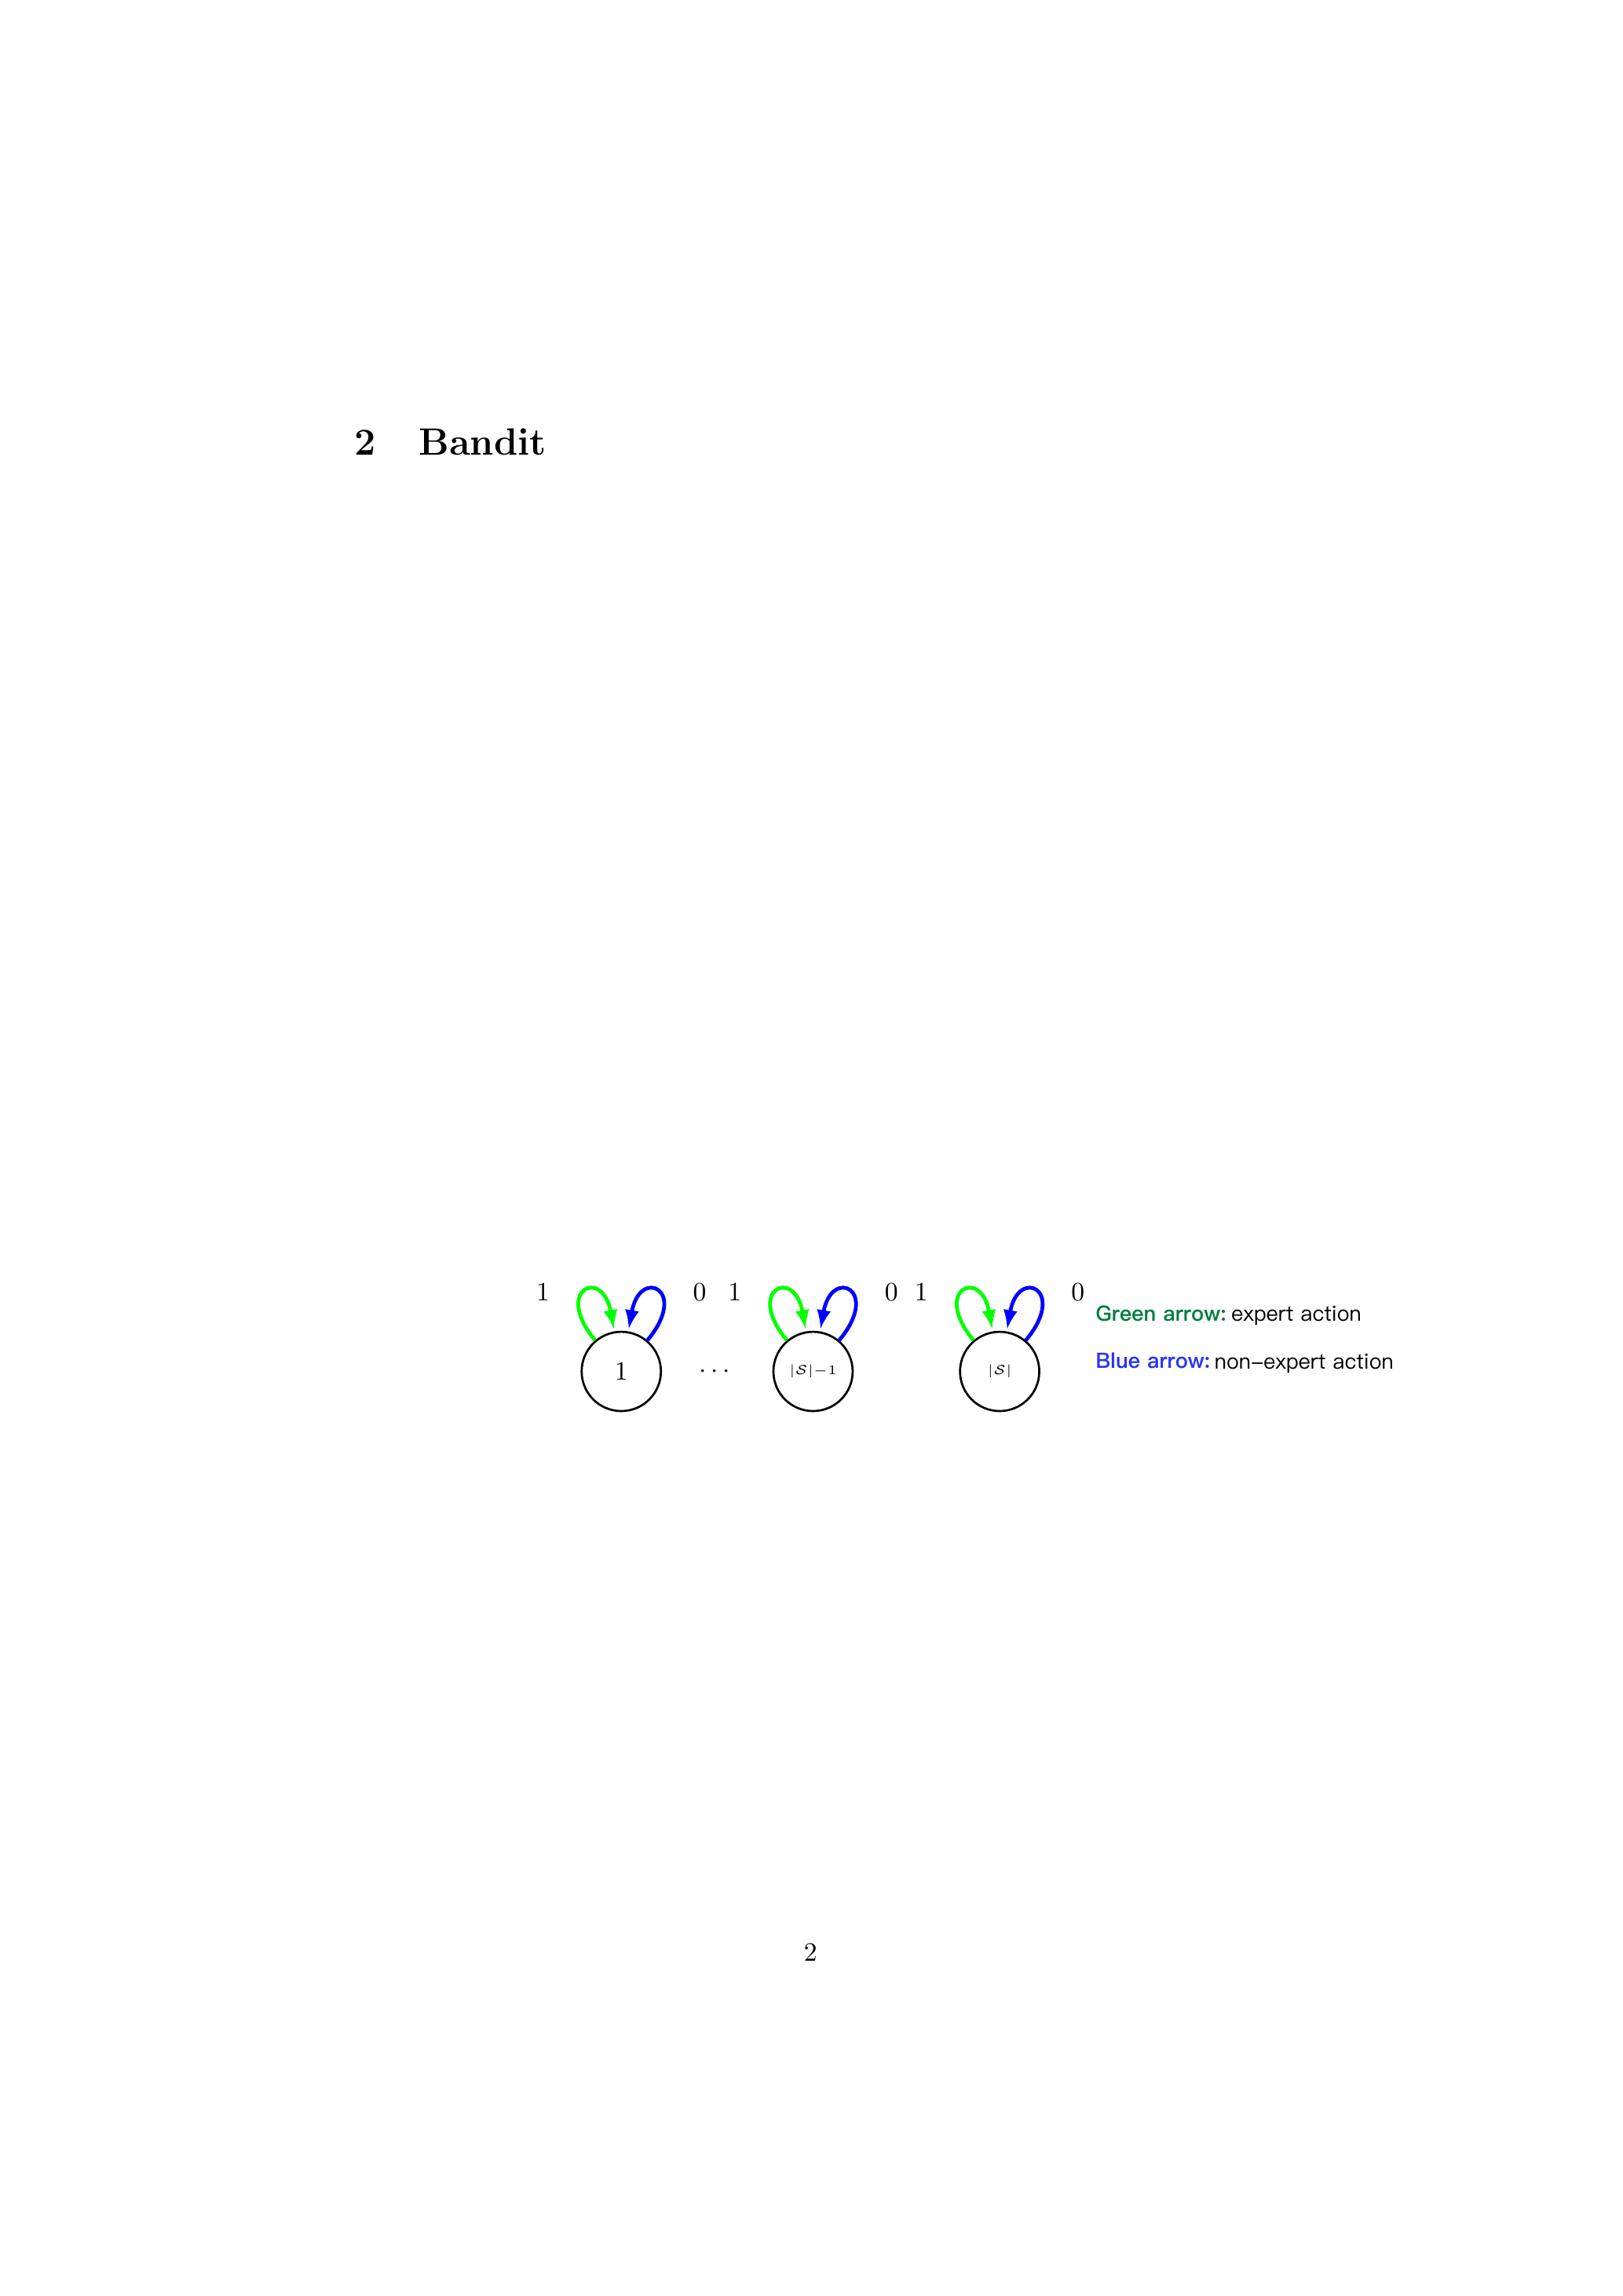}  
\caption{\textsf{Standard Imitation} MDPs corresponding to \cref{asmp:standard_imitation}.}
\label{fig:bandit}
\end{figure}

\begin{proof}[Proof of \cref{proposition:ail_policy_value_gap_standard_imitation}]
Notice that each state is absorbing in Standard Imitation and thus, $P^{\pi}_h (s) = \rho (s), \forall s \in \gS, h \in [H]$. Then we obtain
\begin{align*}
  &\quad \min_{\pi \in \Pi} \sum_{h=1}^{H} \sum_{(s, a) \in \gS \times \gA} | P^{\pi}_h(s, a) - \widehat{P}^{\piE}_h(s, a) |
  \\
  &= \min_{\pi \in \Pi} \sum_{h=1}^{H} \sum_{(s, a) \in \gS \times \gA} | \rho (s) \pi_h (a|s) - \widehat{P}^{\piE}_h(s, a) |
  \\
  &= \min_{\pi \in \Pi} \sum_{h=1}^{H} \sum_{s \in \gS } \lp | \rho (s) \pi_h (a^{1}|s) - \widehat{P}^{\piE}_h(s, a^{1}) | + \rho (s) \pi_h (a^{2}|s) \rp
  \\
  &= \min_{\pi \in \Pi} \sum_{h=1}^{H} \sum_{s \in \gS } \lp | \rho (s) \pi_h (a^{1}|s) - \widehat{P}^{\piE}_h(s) | + \rho (s) \lp 1- \pi_h (a^{1}|s) \rp \rp
  \\
  &= \min_{\pi \in \Pi} \sum_{h=1}^{H} \sum_{s \in \gS } \lp | \rho (s) \pi_h (a^{1}|s) - \widehat{P}^{\piE}_h(s) | - \rho (s) \pi_h (a^{1}|s) \rp. 
\end{align*}
Since the optimization variables $\pi_h (a^{1}|s)$ for different $s \in \gS, h \in [H]$ are independent, we can consider the optimization problem for each $s \in \gS, h \in [H]$ individually. For each $h \in [H]$ and $s \in \gS$,
\begin{align*}
    \min_{\pi_h (a^{1}|s) \in [0, 1]} | \rho (s) \pi_h (a^{1}|s) - \widehat{P}^{\piE}_h(s) | - \rho (s) \pi_h (a^{1}|s). 
\end{align*}
For any state $s \in \gS^1_h = \{s \in \gS: \widehat{P}^{\piE}_h (s) < \rho (s) \} $, with \cref{lem:single_variable_opt_condition}, we have that $\piail_h (a^{1}|s) \in [\widehat{P}^{\piE}_h (s) / \rho (s), 1]$ are all optimal solutions. On the other hand, for any state $s \in \lp \gS^1_h \rp^c$, the optimization problem is reduced to
\begin{align*}
    \min_{\pi_h (a^{1}|s) \in [0, 1]}  \widehat{P}^{\piE}_h(s) - 2\rho (s) \pi_h (a^{1}|s).
\end{align*}
It is easy to see that the optimal solution is $\pi_h (a^{1}|s) = 1$. Therefore, for each time step $h$, $\piail_h (a^1|s) \in [\widehat{P}^{\piE}_h(s) / \rho (s), 1], \forall s \in \gS_h^1$ and $\piail_h (a^1|s) = 1, \forall s \in (\gS_h^1)^c$ are all optimal solutions of \eqref{eq:ail}.

For the policy value gap, according to the dual representation of policy value, we have that
\begin{align*}
    V^{\piE} - V^{\piail} &= \sum_{h=1}^{H} \sum_{(s, a) \in \gS \times \gA}  \lp P^{\piE}_h(s, a) - P^{\piail}_h(s, a) \rp r_h (s, a)
    \\
    &= \sum_{h=1}^{H} \sum_{s \in \gS}  P^{\piE}_h(s, a^{1}) - P^{\piail}_h(s, a^{1}) 
    \\
    &= \sum_{h=1}^{H} \sum_{s \in \gS } P^{\piE}_h(s)  - \rho(s) \piail_h( a^{1}|s).
\end{align*}
Among all optimal solutions, the largest policy value gap is obtained at $\forall h \in [H], \piail_h (a^1|s) = \widehat{P}^{\piE}_h(s) / \rho (s), \forall s \in \gS_h^1; \piail_h (a^1|s) = 1, \forall s \in (\gS_h^1)^c$. The largest policy value gap is
\begin{align*}
    V^{\piE} - V^{\piail} &= \sum_{h=1}^{H} \sum_{s \in \gS_h^1} P^{\piE}_h(s)  - \rho(s) \piail_h( a^{1}|s) = \sum_{h=1}^{H} \sum_{s \in \gS_h^1} P^{\piE}_h(s)  - \widehat{P}^{\piE}_h(s). 
\end{align*}
Next, we connect the term $\sum_{s \in \gS_h^1} P^{\piE}_h(s)  - \widehat{P}^{\piE}_h(s)$ with the $\ell_1$-norm estimation error. Notice that for each time step $h \in [H]$, $\sum_{s \in \gS} P^{\piE}_h(s) = \sum_{s \in \gS} \widehat{P}^{\piE}_h(s)$ = 1. Then we have that
\begin{align*}
    \sum_{s \in \gS^1_h} P^{\piE}_h(s)  - \widehat{P}^{\piE}_h(s) = \sum_{s \in (\gS^1_h)^c} \widehat{P}^{\piE}_h(s) - P^{\piE}_h(s).  
\end{align*}
Furthermore, we obtain
\begin{align}
     \sum_{h=1}^H \lnorm \widehat{P}^{\piE}_h - P^{\piE}_h   \rnorm_1 &= \sum_{h=1}^H \sum_{s \in \gS} \labs P^{\piE}_h(s) - \widehat{P}^{\piE}_h (s)  \rabs \nonumber
     \\
     &= \sum_{h=1}^H \sum_{s \in \gS^1_h} P^{\piE}_h(s)  - \widehat{P}^{\piE}_h(s) + \sum_{s \in (\gS^1_h)^c} \widehat{P}^{\piE}_h(s) - P^{\piE}_h(s) \nonumber
     \\
     &= 2 \sum_{h=1}^H \sum_{s \in \gS^1_h} P^{\piE}_h(s)  - \widehat{P}^{\piE}_h(s), \label{eq:vail_standard_imitation_policy_value_gap_half_estimation_error}
\end{align}
where the penultimate equality follows that $\gS^1_h = \{s \in \gS: \widehat{P}^{\piE}_h (s) < \rho (s) \}$. Finally, we get that
\begin{align*}
    V^{\piE} - V^{\piail} = \sum_{h=1}^{H} \sum_{s \in \gS_h^1} P^{\piE}_h(s)  - \widehat{P}^{\piE}_h(s) = \frac{1}{2}  \sum_{h=1}^H \lnorm \widehat{P}^{\piE}_h - P^{\piE}_h   \rnorm_1.
\end{align*}
\end{proof}

\subsection{Proof of Proposition \ref{prop:lower_bound_vail}}

\begin{proof}

To prove \cref{prop:lower_bound_vail}, we make two steps. First, we connect the policy value gap with the estimation error with the help of \cref{proposition:ail_policy_value_gap_standard_imitation}. Consider the Standard Imitation MDP in \cref{asmp:standard_imitation}, given estimation $\widehat{P}^{\piE}_h$, for each time step $h \in [H]$, recall the definition of $\gS_h^1 := \{s \in \gS: \widehat{P}^{\piE}_h (s) < \rho (s)   \}$. We construct a policy set $\Pi^{\ail}$ defined as
\begin{align*}
   \Pi^{\ail}: = \lb \pi \in \Pi: \forall h \in [H], \forall s \in \gS_h^1, \piail_h (a^1|s) \in [\widehat{P}^{\piE}_h(s) / \rho (s), 1]; \forall s \in (\gS_h^1)^c,  \piail_h (a^1|s) =1  \rb. 
\end{align*}
With \cref{proposition:ail_policy_value_gap_standard_imitation}, we have that $\Pi^{\ail}$ is the set of all globally optimal solutions of \textsf{VAIL}'s objective \eqref{eq:ail}. Note that \textsf{VAIL} outputs a policy $\piail$ uniformly sampled from $\Pi^{\ail}$. Same with the proof of \cref{proposition:ail_policy_value_gap_standard_imitation}, we have that
\begin{align*}
    V^{\piE} - V^{\piail} &= \sum_{h=1}^{H} \sum_{s \in \gS } P^{\piE}_h(s)  - \rho(s) \piail_h( a^{1}|s)
    \\
    &= \sum_{h=1}^{H} \sum_{s \in \gS_h^1 } P^{\piE}_h(s)  - \rho(s) \piail_h( a^{1}|s) .
\end{align*}
Taking expectation w.r.t the uniformly random selection of $\piail$ on both sides yields that
\begin{align*}
    V^{\piE} - \expect_{\piail \sim \text{Unif} (\Pi^{\ail})} \ls V^{\piail} \rs &= \expect_{\piail \sim \text{Unif} (\Pi^{\ail})} \ls \sum_{h=1}^{H} \sum_{s \in \gS_h^1 } P^{\piE}_h(s)  - \rho(s) \piail_h( a^{1}|s) \rs 
    \\
    &=  \sum_{h=1}^{H} \sum_{s \in \gS_h^1 } P^{\piE}_h(s) - \rho (s) \expect_{\piail_h( a^{1}|s) \sim \text{Unif} \lp [\widehat{P}^{\piE}_h(s) / \rho (s), 1] \rp } \ls \piail_h( a^{1}|s) \rs
    \\
    &= \frac{1}{2} \sum_{h=1}^{H} \sum_{s \in \gS_h^1} P^{\piE}_h(s)  - \widehat{P}^{\piE}_h(s).
\end{align*}
Combined with \eqref{eq:vail_standard_imitation_policy_value_gap_half_estimation_error}, we have that
\begin{align*}
    V^{\piE} - \expect_{\piail \sim \text{Unif} (\Pi^{\ail})} \ls V^{\piail} \rs = \frac{1}{2} \sum_{h=1}^{H} \sum_{s \in \gS_h^1} P^{\piE}_h(s)  - \widehat{P}^{\piE}_h(s) = \frac{1}{4} \sum_{h=1}^H \lnorm \widehat{P}^{\piE}_h - P^{\piE}_h   \rnorm_1.
\end{align*}
We further take the expectation over the randomness of expert demonstrations on both sides.
\begin{align*}
    V^{\piE} - \expect \ls \expect_{\piail \sim \text{Unif} (\Pi^{\ail})} \ls V^{\piail} \rs \rs = \frac{1}{4} \sum_{h=1}^H \expect \ls \lnorm \widehat{P}^{\piE}_h - P^{\piE}_h   \rnorm_1 \rs.
\end{align*}
Second, we apply the lower bound of expected $\ell_1$ risk of \citep[Corollary 9]{kamath2015learning} and have that
\begin{align*}
    V^{\piE} - \expect \ls \expect_{\piail \sim \text{Unif} (\Pi^{\ail})} \ls V^{\piail} \rs \rs \geq \frac{1}{4} H \sqrt{\frac{2 \lp \vert \gS \vert - 1 \rp}{\pi m}}.
\end{align*}
To obtain an $\varepsilon$-optimal policy (i.e., $V^{\piE} - \expect[ V^{\piail}] \leq \varepsilon$), in expectation, \textsf{VAIL} requires at least $\Omega(|\gS| H^2/\varepsilon^2)$ expert trajectories.

\end{proof}

\subsection{Proof of Theorem \ref{theorem:bc_deterministic}}

First, we formally state the result on the sample complexity for BC to achieve an $\varepsilon$-optimal policy \emph{with high probability}. This result is similar to \emph{in expectation} bound.

\begin{thm}[High Probability Version of \cref{theorem:bc_deterministic}]  \label{theorem:bc_deterministic_high_prob}
For any tabular and episodic MDP with deterministic transitions, with probability at least $1-\delta$, to obtain an $\varepsilon$-optimal policy (i.e., $V^{\piE} - V^{\pibc} \leq \varepsilon$), BC as in \eqref{eq:bc} requires at most ${\widetilde{\gO}}(|\gS| H/\varepsilon)$ expert trajectories.  
\end{thm}

\begin{proof}[Proof of \cref{theorem:bc_deterministic} and \cref{theorem:bc_deterministic_high_prob}]

In the following part, we provide proof for both \cref{theorem:bc_deterministic} and \cref{theorem:bc_deterministic_high_prob}. To prove \cref{theorem:bc_deterministic} and \cref{theorem:bc_deterministic_high_prob}, we make two steps. First, we show that when the transition function is deterministic, the policy value gap of BC comes from non-visited states in the first step.

Suppose that $\pibc$ is the minimizer of BC objective in \cref{eq:bc}. Then we have that
\begin{align*}
    &\quad V^{\piE} - V^{\pibc}
    \\
    &= \expect_{s_1 \sim \rho (\cdot)} \ls V^{\piE}_1 (s_1) - V^{\pibc}_1 (s_1)   \rs
    \\
    &= \expect_{s_1 \sim \rho (\cdot)} \ls \indict \lp s_1 \notin \gS_1 (\gD) \rp \lp V^{\piE}_1 (s_1) - V^{\pibc}_1 (s_1) \rp   \rs + \expect_{s_1 \sim \rho (\cdot)} \ls \indict \lp s_1 \in \gS_1 (\gD) \rp \lp V^{\piE}_1 (s_1) - V^{\pibc}_1 (s_1) \rp   \rs
    \\
    &= \expect_{s_1 \sim \rho (\cdot)} \ls \indict \lp s_1 \notin \gS_1 (\gD) \rp \lp V^{\piE}_1 (s_1) - V^{\pibc}_1 (s_1) \rp   \rs. 
\end{align*}
Since the expert policy and transition function are deterministic, the trajectories, started with the visited initial states, are fully covered in the expert demonstrations. Hence, the policy value gap on these trajectories is zero. This is our key observation for deterministic MDPs. Recall that $\gS_1(\gD)$ is the set of visited states in time step $1$ from expert dataset $\gD$. Then we have that
\begin{align*}
  V^{\piE} - V^{\pibc} &= \expect_{s_1 \sim \rho (\cdot)} \ls \indict \lp s_1 \notin \gS_1 (\gD) \rp \lp V^{\piE}_1 (s_1) - V^{\pibc}_1 (s_1) \rp   \rs
    \\
    &\leq H \expect_{s_1 \sim \rho (\cdot)} \ls \indict \lp s_1 \notin \gS_1 (\gD) \rp   \rs, 
\end{align*}
which is tighter than the result in \citep{rajaraman2020fundamental} since their result holds for general MDPs with stochastic transitions. Notice that $\expect_{s_1 \sim \rho (\cdot)} \ls \indict \lp s_1 \notin \gS_1 (\gD) \rp   \rs = \sum_{s \in \gS} \rho (s) \indict \lp s_1 \notin \gS_1 (\gD) \rp $ is the \emph{missing mass} of the distribution of $\rho$ given $m$ i.i.d. samples; see \cref{defn:missing_mass} for the definition of missing mass, which is from \citep[Defintion A.1]{rajaraman2020fundamental}.

\begin{defn}[Missing Mass \citep{rajaraman2020fundamental}] \label{defn:missing_mass}
Let $\gX = \{1, 2, \cdots, |\gX|\}$ be a finite set. Let $P$ be some distribution on $\gX$. Furthermore, let $X^{m} = (X_1, \cdots, X_m)$ be $m$ i.i.d. random variables from $P$.  Let $\mathfrak{n}_x(X^{m}) = \sum_{i=1}^{m} \mathbb{I}\{ X_i =  x\}$ be the number of times the element $x$ was observed in these random variables. Then, $\mathfrak{m}_0(P, X^{m}) = \sum_{x \in \gX} P(x) \mathbb{I} \{ n_x(X^{m}) = 0 \}$ is called missing mass, which means the probability mass contributed by elements never observed in $X^{m}$.
\end{defn}

Second, we need to upper bound the missing mass in the first time step. We first prove the sample complexity to achieve a small policy value gap \emph{with high probability}. To this end, we leverage the following concentration inequality \citep[Lemma A.3]{rajaraman2020fundamental}.
\begin{lem}[Concentration Inequality for Missing Mass \citep{rajaraman2020fundamental}]  \label{lemma:missing_mass_one_step}
Let $\gX = \{1, 2, \cdots, |\gX|\}$ be a finite set. Let $P$ be some distribution on $\gX$. Furthermore, let $X^{m} = (X_1, \cdots, X_m)$ be $m$ i.i.d. random variables from $P$. For any $\delta \in (0, 1/10]$, with probability at least $1-\delta$, we have 
\begin{align*}
\mathfrak{m}_0(P, X^{m}) := \sum_{x \in \gX} P(x) \mathbb{I} \{ n_x(X^{m}) = 0 \} \leq \frac{4|\gX|}{9m}  + \frac{3\sqrt{|\gX|} \log (1/\delta)}{m}.
\end{align*}
\end{lem}
With \cref{lemma:missing_mass_one_step}, we obtain that with probability at least $1-\delta$, 
\begin{align*}
    V^{\piE} - V^{\pibc} \leq H \lp \frac{4|\gS|}{9m}  + \frac{3\sqrt{|\gS|} \log (1/\delta)}{m} \rp,
\end{align*}
which translates to the sample complexity $\widetilde{\gO}(|\gS| H/\varepsilon)$ with high probability.

We continue to prove the sample complexity to achieve a small policy value gap \emph{in expectation}. We have that
\begin{align*}
    \expect \ls V^{\piE} - V^{\pibc} \rs \leq H \expect \ls \expect_{s_1 \sim \rho (\cdot)} \ls \indict \lp s_1 \notin \gS_1 (\gD) \rp   \rs \rs. 
\end{align*}
The outer expectation is taken w.r.t the randomness of expert demonstrations. For RHS, we have 
\begin{align}
    \expect \ls \expect_{s_1 \sim \rho (\cdot)} \ls \indict \lp s_1 \notin \gS_1 (\gD) \rp   \rs \rs &= \expect_{s_1 \sim \rho (\cdot)} \ls \expect \ls \indict \lp s_1 \notin \gS_1 (\gD) \rp \rs   \rs \nonumber
    \\
    &= \sum_{s \in \gS } \rho (s) \sP \lp  s \notin \gS_1 (\gD) \rp \nonumber
    \\
    &=  \sum_{s \in \gS } \rho (s) \lp 1 - \rho (s) \rp^m \nonumber
    \\
    &\leq \vert \gS \vert \max_{x \in [0, 1]} x (1-x)^m \nonumber
    \\
    &\leq \frac{|\gS|}{em}. \label{eq:expected_missing_mass_upper_bound} 
\end{align}
In the last inequality, we consider the optimization problem $\max_{x \in [0, 1]} f(x) = x (1-x)^m$. Here $f'(x) = (1-x)^{m-1} (1- (m+1)x)$. It is easy to see that the maximum is achieved at $x = 1/(m+1)$. Hence,
\begin{align*}
  \max_{x \in [0, 1]} x (1-x)^m = \frac{1}{m} \lp 1 - \frac{1}{m+1} \rp^{m+1} \leq \frac{1}{em}.   
\end{align*}
Finally, we have $ V^{\piE} - \expect [ V^{\pibc}] \leq (|\gS|H) / (em)$, which translates to the sample complexity $\gO(|\gS| H/\varepsilon)$ as in \cref{theorem:bc_deterministic}.

\end{proof}

\subsection{Reset Cliff and Useful Properties}
\label{appendix:reset_cliff_and_ail_properties}
In this part, we first give a detailed introduction of a family of MDPs called Reset Cliff shown in \cref{subsec:ail_generalize_well}. Then we present some properties of \textsf{VAIL}, which are useful in proving the results in \cref{subsec:ail_generalize_well}.

The Reset Cliff MDPs (refer to \cref{asmp:reset_cliff}) are illustrated in \cref{fig:reset_cliff}. Their properties are re-stated as follows.
\begin{itemize}
    \item In Reset Cliff, the state space is divided into the set of good states (shown in black circle) and the set of bad states (shown in red circle). That is $\gS = \goodS \cup \badS, \goodS \cap \badS = \emptyset$.
    \item The action space is denoted as $\gA$, in which $a^1$ is expert action (shown in green arrow) and the others are non-expert actions (shown in blue arrow).
    \item The agent gets $+1$ reward only by taking expert action $a^1$ on good states. For other cases, the agents gets 0 reward.
    \item On a good state, when the agent takes expert action $a^1$, then it transits into good states. Otherwise, the agent transits into bad states. Formally, $\forall h \in [H], s \in \goodS, a \in \gA \setminus \{a^1\}, \sum_{s^\prime \in \goodS} P_h (s^\prime|s, a^1) = 1, \sum_{s^\prime \in \badS} P_h (s^\prime|s, a) = 1$. Besides, we assume that $\forall h \in [H], \forall s, s^\prime \in \goodS, P_h (s^\prime |s, a^1) > 0 $.
    
    \item On a bad state, no matter which action is taken, the agent always goes to bad states. That is, $\forall h \in [H], s \in \badS, a \in \gA, \sum_{s^\prime \in \badS} P_h (s^\prime |s, a) = 1$.
\end{itemize}
       
\begin{figure}[htbp]
\centering
\includegraphics[width=0.9\linewidth]{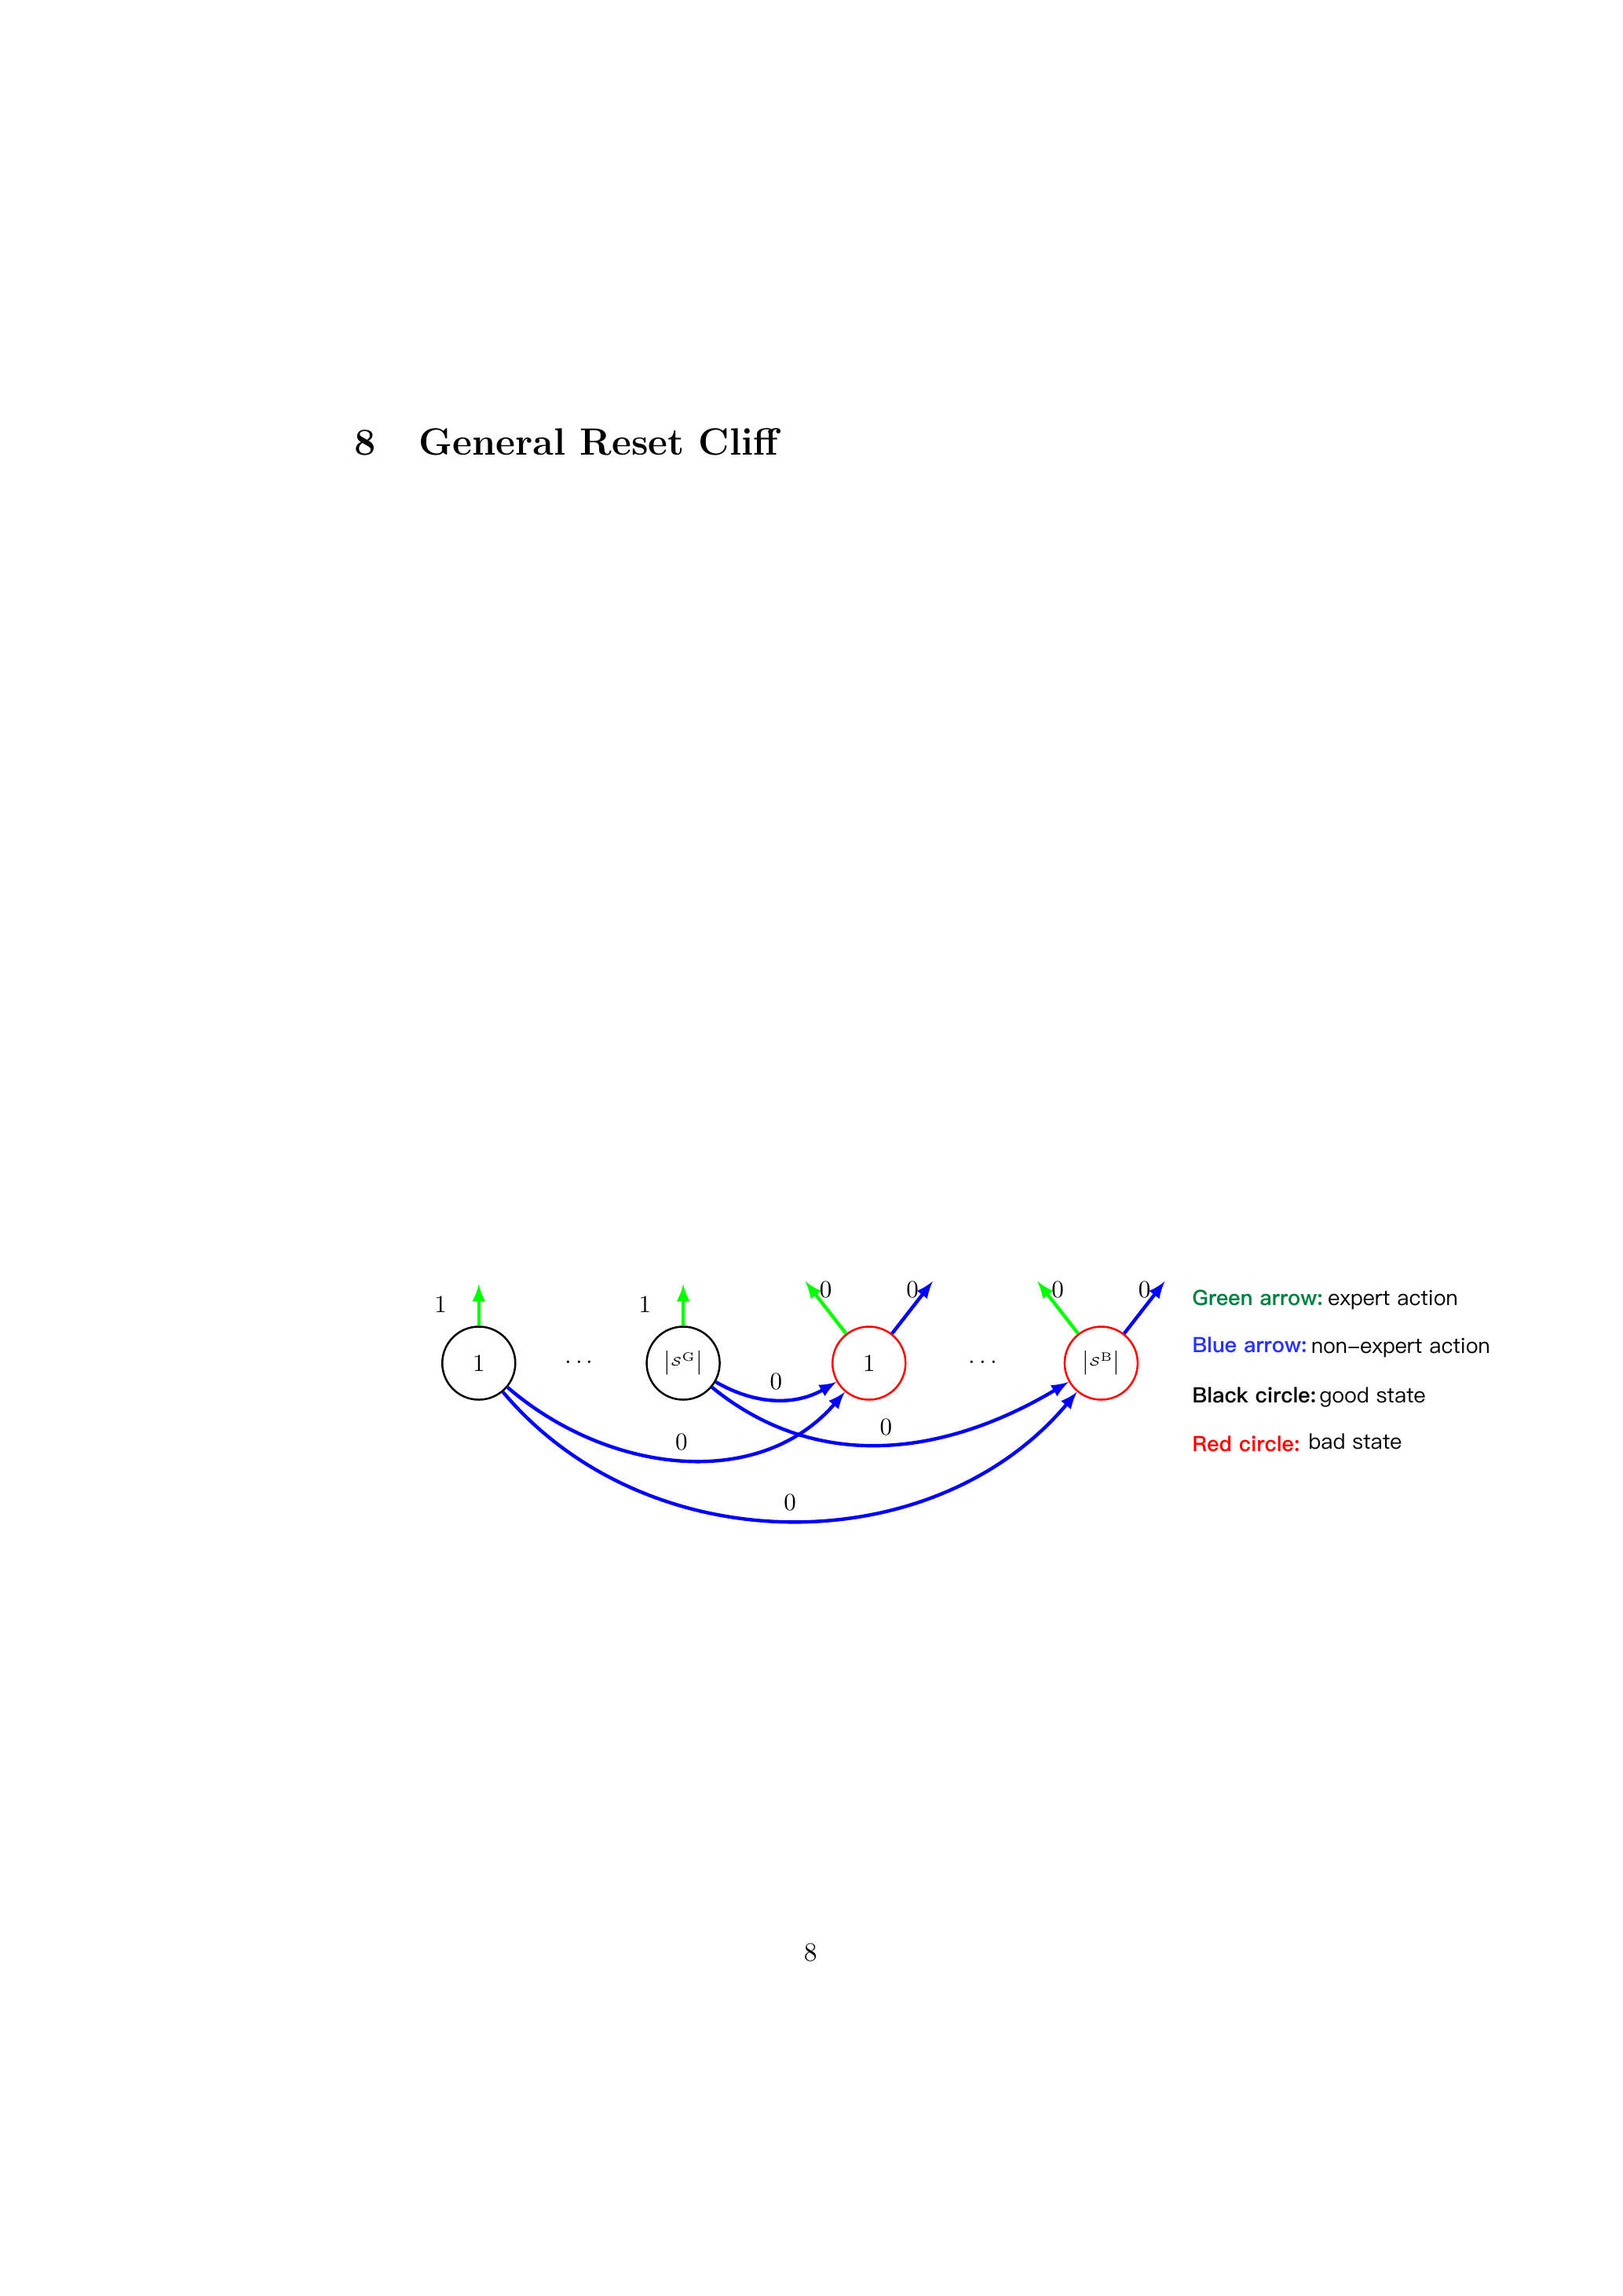}
\caption{\textsf{Reset Cliff} MDPs corresponding to \cref{asmp:reset_cliff}.}
\label{fig:reset_cliff}
\end{figure}

For Reset Cliff MDPs, we know the expert policy never visits bad states. Thus, we have the following fact. 
\begin{fact}    \label{fact:ail_estimation}
For any tabular and episodic MDP satisfying \cref{asmp:reset_cliff}, considering any unbiased estimation $\widehat{P}^{\piE}_h (s, a)$, we have that 
\begin{align*}
   &\forall h \in [H], \forall s \in \badS, \forall a \in \gA, \quad  \widehat{P}^{\piE}_h(s) = 0,  \widehat{P}^{\piE}_h(s, a) = 0, \\
   &\forall h \in [H], \quad \sum_{s \in \goodS} \widehat{P}^{\piE}_h(s, a^{1}) = 1.0, \\
   &\forall h \in [H], \forall s \in \goodS, \forall a \ne a^{1}, \quad  \widehat{P}^{\piE}_h(s, a) = 0.0. 
\end{align*}
\end{fact}

Then we continue to present some useful properties of \textsf{VAIL} on Reset Cliff MDPs, which will be applied in the proof of results in \cref{subsec:ail_generalize_well}. Recall that 
\begin{align*}
  \piail = \argmin_{\pi} \sum_{h=1}^{H} \sum_{(s, a) \in \gS \times \gA} | P^{\pi}_h(s, a) - \widehat{P}^{\piE}_h(s, a) |.
\end{align*}
The first lemma states that on Reset Cliff, in each time step, $\piail$ takes the expert action on some good state with a positive probability.
\begin{lem}
\label{lem:condition_for_ail_optimal_solution}
For any tabular and episodic MDP satisfying \cref{asmp:reset_cliff}, suppose that $\piail$ is the optimal solution of \eqref{eq:ail}. Then $\forall h \in [H]$, $\exists s \in \goodS$, $\piail_h (a^{1} |s) > 0$.
\end{lem}

\begin{proof}
This proof is based on contradiction. Assume that the original statement is false: there exists a policy $\piail$, which is the optimal solution of \eqref{eq:ail}, such that $\exists h \in [H]$, $\forall s \in \goodS$, $\piail_h (a^{1}|s) = 0$. Let $h$ denote the smallest time step index such that $\forall s \in \goodS, \piail_{h} (a^{1}|s) = 0$. It also implies that $\forall s \in \goodS, \sum_{a \in \gA \setminus \{a^1 \}} \piail_{h} (a|s) = 1$.

We construct another policy $\widetilde{\pi}^{\operatorname{AIL}}$. $\widetilde{\pi}^{\operatorname{AIL}}$ is the same as $\piail$ in the first $h-1$ steps. In time step $h$, $\widetilde{\pi}^{\operatorname{AIL}} (a^{1}|s) = 1, \forall s \in \goodS$. Here we compare objective values of $\piail$ and $\widetilde{\pi}^{\operatorname{AIL}}$. Since $\piail$ is the same as $\widetilde{\pi}^{\operatorname{AIL}}$ in the first $h-1$ steps, their objective values are the same in the first $h-1$ steps. We only need to compare VAIL's objectives of $\piail$ and $\widetilde{\pi}^{\operatorname{AIL}}$ from time step $h$.

In time step $h$, notice that $P^{\widetilde{\pi}^{\operatorname{AIL}}}_h (s) =P^{\piail}_h (s)$, we obtain
\begin{align*}
    &\quad \text{Loss}_{h}(\piail) \\
    &= \sum_{(s, a)} \labs \widehat{P}^{\piE}_h (s, a) - P^{\piail}_h (s, a)  \rabs \\
    &= \sum_{s \in \goodS} \ls \labs \widehat{P}^{\piE}_h (s, a^{1}) - P^{\piail}_h (s, a^{1})  \rabs + \sum_{a \ne a^{1}} \labs \widehat{P}^{\piE}_h (s, a) - P^{\piail}_h (s, a)  \rabs \rs   + \sum_{s \in \badS} \sum_{a} \labs \widehat{P}^{\piE}_h (s, a) - P^{\piail}_h (s, a)  \rabs  \\
    &= \sum_{s \in \goodS} \ls \labs \widehat{P}^{\piE}_h (s, a^{1}) - 0  \rabs + \sum_{a \ne a^{1}} \labs 0 - P^{\piail}_h (s, a)  \rabs \rs   + \sum_{s \in \badS} \sum_{a} \labs 0 - P^{\piail}_h (s, a)  \rabs \\
    &=  \sum_{s \in \goodS} \lp \widehat{P}^{\piE}_h (s) + P^{\piail}_h (s) \rp + \sum_{s \in \badS}  P^{\piail}_h (s),
    \\
    &\quad \text{Loss}_{h}(\widetilde{\pi}^{\operatorname{AIL}}) \\
    &= \sum_{(s, a)} \labs \widehat{P}^{\piE}_h (s, a) - P^{\widetilde{\pi}^{\operatorname{AIL}}}_h (s, a)  \rabs \\
    &= \sum_{s \in \goodS} \ls \labs \widehat{P}^{\piE}_h (s, a^{1}) - P^{\widetilde{\pi}^{\operatorname{AIL}}}_h (s, a^{1})  \rabs + \sum_{a \ne a^{1}} \labs \widehat{P}^{\piE}_h (s, a) - P^{\widetilde{\pi}^{\operatorname{AIL}}}_h (s, a)  \rabs \rs   + \sum_{s \in \badS} \sum_{a} \labs \widehat{P}^{\piE}_h (s, a) - P^{\widetilde{\pi}^{\operatorname{AIL}}}_h (s, a)  \rabs  \\
    &=  \sum_{s \in \goodS} \ls \labs \widehat{P}^{\piE}_h (s, a^{1}) - P^{\widetilde{\pi}^{\operatorname{AIL}}}_h (s, a^{1})  \rabs + \sum_{a \ne a^{1}} \labs 0 - 0 \rabs \rs + \sum_{s \in \badS} \sum_{a} \labs 0 - P^{\piail}_h (s, a)  \rabs \\
    &= \sum_{s \in \goodS} \labs \widehat{P}^{\piE}_h (s) - P^{\piail}_h (s) \rabs + \sum_{s \in \badS}  P^{\piail}_h (s).
\end{align*}
Then we have
\begin{align*}
    \text{Loss}_{h}(\widetilde{\pi}^{\operatorname{AIL}}) - \text{Loss}_{h}(\piail) = \sum_{s \in \goodS} \labs \widehat{P}^{\piE}_h (s) - P^{\piail}_h (s) \rabs - \widehat{P}^{\piE}_h (s) - P^{\piail}_h (s) < 0,  
\end{align*}
where the last strict inequality follows that there always exists $s \in \goodS$ such that $\widehat{P}^{\piE}_h (s)>0, P^{\piail}_h (s) >0$. This is because $h$ is the smallest time step index such that $\forall s \in \goodS, \piail_{h} (a^1|s) = 0$ and $\forall h \in [H], \forall s, s^\prime \in \goodS, P_h (s^\prime |s, a^1) > 0$. Hence, $\forall s \in \goodS, P^{\piail}_h (s) >0$. For time step $h^\prime$ where $h+1 \leq h^\prime \leq H$,
\begin{align*}
    &\quad \text{Loss}_{h^\prime}(\piail) \\
    &=  \sum_{(s, a)} \labs \widehat{P}^{\piE}_{h^\prime} (s, a) - P^{\piail}_{h^\prime} (s, a)  \rabs  \\
    &= \sum_{s \in \goodS} \sum_{a}  \labs \widehat{P}^{\piE}_{h^\prime} (s, a) - P^{\piail}_{h^\prime} (s, a)  \rabs   + \sum_{s \in \badS} \sum_{a} \labs \widehat{P}^{\piE}_{h^\prime} (s, a) - P^{\piail}_{h^\prime} (s, a)  \rabs  \\
    &=  \sum_{s \in \goodS} \sum_{a}  \labs \widehat{P}^{\piE}_{h^\prime} (s, a) - 0 \rabs   + \sum_{s \in \badS} \sum_{a} \labs 0 - P^{\piail}_{h^\prime} (s, a)  \rabs \\
    &= \sum_{s \in \goodS} \widehat{P}^{\piE}_{h^\prime} (s) + \sum_{s \in \badS}  P^{\piail}_{h^\prime} (s) = 2,
\end{align*}
which is the maximal value of VAIL's objective at each time step. Thus, we have that $\text{Loss}_{h^\prime}(\widetilde{\pi}^{\operatorname{AIL}}) < \text{Loss}_{h^\prime}(\piail)$.

To summarize, we construct a policy $\widetilde{\pi}^{\operatorname{AIL}}$ whose VAIL's objective is strictly smaller than that of $\piail$. It contradicts with the fact that $\piail$ is the optimal solution of VAIL's objective. Hence the original statement is true and we finish the proof. 

\end{proof}

For any fixed unbiased estimation $\widehat{P}^{\piE}_h (s, a)$, we define a set of states $\gS ( \widehat{P}^{\piE}_H  ) := \{ s \in \gS, \widehat{P}^{\piE}_H (s) > 0  \}$. The following lemma states that in the last time step, \textsf{VAIL}'s policy takes the expert action on each $s \in \gS ( \widehat{P}^{\piE}_H  )$ with a positive probability. Note this positive probability may not be 1 due to the \dquote{weak convergence} issue.

\begin{lem}
\label{lem:general_condition_ail_policy_at_last_step}
Consider any tabular and episodic MDP satisfying \cref{asmp:reset_cliff}. For any fixed unbiased estimation $\widehat{P}^{\piE}_h (s, a)$, we define a set of states $\gS ( \widehat{P}^{\piE}_H  ) := \{ s \in \gS, \widehat{P}^{\piE}_H (s) > 0  \}$. Suppose that $\piail = (\piail_1, \cdots, \piail_H)$ is the optimal solution of \eqref{eq:ail}, then $\forall s \in \gS ( \widehat{P}^{\piE}_H  ), \piail_{H} \lp a^{1} |s \rp > 0$. 
\end{lem}

\begin{proof}
With \cref{lem:n_vars_opt_greedy_structure}, if $\piail = (\piail_1, \cdots, \piail_{H-1}, \piail_{H})$ is the optimal solution, then fixing $(\piail_1, \cdots, \piail_{H-1})$, $\piail_{H}$ is also optimal w.r.t VAIL's objective. Furthermore, since $P^{\piail}_{H} (s)$ is independent of $\piail_H$, we have
\begin{align*}
    \piail_{H} & \in \argmin_{\pi_{H}}  \sum_{(s, a)} \labs P^{\piail}_H(s) \pi_{H}(a|s) - \widehat{P}^{\piE}_H(s, a) \rabs.
\end{align*}
Recall that $\gS ( \widehat{P}^{\piE}_H  ) := \{ s \in \gS, \widehat{P}^{\piE}_H (s) > 0  \}$, we have 
\begin{align*}
   \piail_{H} &\in \argmin_{\pi_{H}}  \sum_{s \in \gS ( \widehat{P}^{\piE}_H  )} \sum_{a \in \gA} \labs P^{\piail}_H(s) \pi_{H}(a|s) - \widehat{P}^{\piE}_H(s, a) \rabs + \sum_{s \notin \gS ( \widehat{P}^{\piE}_H  )} \sum_{a \in \gA} \labs P^{\piail}_H(s) \pi_H(a|s) - \widehat{P}^{\piE}_H(s, a) \rabs
   \\
   &= \argmin_{\pi_{H}}  \sum_{s \in \gS ( \widehat{P}^{\piE}_H  )} \lp \labs P^{\piail}_H(s) \pi_H ( a^{1} |s) - \widehat{P}^{\piE}_H(s, a^{1} ) \rabs + \sum_{a \ne a^{1} } \labs P^{\piail}_H(s) \pi_H (a|s) - \widehat{P}^{\piE}_H(s, a) \rabs \rp
   \\
   &\quad + \sum_{s \notin \gS ( \widehat{P}^{\piE}_H  )} \sum_{a \in \gA } \labs P^{\piail}_H(s) \pi_H(a|s) - \widehat{P}^{\piE}_H(s, a) \rabs.
\end{align*}
Since $\widehat{P}^{\piE}_H(s, a) = 0$ for $a \not= a^{1}$, we obtain
\begin{align*}
\piail_{H} &\in \argmin_{\pi_{H}}  \sum_{s \in \gS ( \widehat{P}^{\piE}_H  )} \lp \labs P^{\piail}_H(s) \pi_H ( a^{1} |s) - \widehat{P}^{\piE}_H(s, a^{1}) \rabs +   P^{\piail}_H(s) \lp 1 - \pi_H (a^{1} |s) \rp \rp
   \\
   &\quad + \sum_{s \notin \gS ( \widehat{P}^{\piE}_H  )} \sum_{a \in \gA } \labs P^{\piail}_H(s) \pi_H(a|s) - \widehat{P}^{\piE}_H(s, a) \rabs
   \\
   &= \argmin_{\pi_{H}}  \sum_{s \in \gS ( \widehat{P}^{\piE}_H  )} \lp \labs P^{\piail}_H(s) \pi_H ( a^{1} |s) - \widehat{P}^{\piE}_H(s, a^{1} ) \rabs -   P^{\piail}_H(s) \pi_H ( a^{1} |s)  \rp
   \\
   &\quad + \sum_{s \notin \gS ( \widehat{P}^{\piE}_H  )} \sum_{a \in \gA } \labs P^{\piail}_H(s) \pi_H(a|s) - \widehat{P}^{\piE}_H(s, a) \rabs.
\end{align*}
The last equation follows that $P^{\piail}_H(s)$ is independent of $\pi_H$. Note that for different $s \in \gS ( \widehat{P}^{\piE}_H  )$, $\pi_H (a^{1} |s)$ are independent by the tabular formulation. Thus, we can consider the optimization problem for each $s \in \gS ( \widehat{P}^{\piE}_H  )$ separately. For each $s \in \gS ( \widehat{P}^{\piE}_H  )$, we have
\begin{align*}
    \piail_{H} (a^{1} |s) = \argmin_{\pi_H (a^{1} |s) \in [0, 1]} \labs P^{\piail}_H(s) \pi_H ( a^{1} |s) - \widehat{P}_H(s, a^{1}) \rabs -   P^{\piail}_H(s) \pi_H ( a^{1} |s).
\end{align*}
For the above one-dimension optimization problem, \cref{lem:single_variable_opt_condition} claims that the optimal solution must be positive, i.e., $\piail_{H} (a^{1} |s)  > 0$. Thus, we finish the proof if we can verify the conditions in \cref{lem:single_variable_opt_condition}. 

In the following part, we verify the conditions of \cref{lem:single_variable_opt_condition} by setting $a = P^{\piail}_H(s), c = \widehat{P}_H(s, a^{1})$. Since $\piail$ is the optimal solution of VAIL's objective, with \cref{lem:condition_for_ail_optimal_solution}, we have that $\forall h \in [H]$, $\exists s \in \goodS$, $\piail_h (a^1 |s) > 0$. Combined with the assumption that $\forall h \in [H], s, s^\prime \in \goodS, P_h (s^\prime |s, a^1) > 0$, we have that $P^{\piail}_H(s) > 0, \forall s \in \goodS$. Based on the definition, for each $s \in \gS ( \widehat{P}^{\piE}_H  )$, $\widehat{P}_H^{\piE}(s, a^{1}) > 0$. Now the conditions of \cref{lem:single_variable_opt_condition} are verified and we obtain that $\piail_H (a^{1} |s) > 0, \forall s \in \gS ( \widehat{P}^{\piE}_H  )$. 
\end{proof}

\subsection{Proof of Claim in Example \ref{example:ail_success}}
\label{appendix:warm_up_of_proposition_reset_cliff}

In this part, we formally state and prove the theoretical result in \cref{example:ail_success}, which is a simplified version of \cref{prop:ail_general_reset_cliff}. 

\begin{claim} \label{claim:ail_reset_cliff}
Consider the MDP and expert demonstration configuration in \cref{example:ail_success}. Suppose that $\piail$ is the optimal solution of \eqref{eq:ail}, then for each time step $h \in [2]$, $\piail_{h} (a^{1}|s) = \piE_h (a^{1}|s) = 1, \forall s \in \{s^{1}, s^{2} \}$.  
\end{claim}

Let us briefly discuss the proof idea. Since the objective in \eqref{eq:ail} involves multi-stage optimization problems, it is common to use the dynamic programming (DP) technique to show the structure of the optimal solutions; see examples in the famous book \citep{bertsekas2012dynamic}.  

\begin{proof}
First of all, recall that there are three states $(s^{1}, s^{2}, s^{3})$ and two actions $(a^{1}, a^{2})$. In particular, $s^{1}$ and $s^{2}$ are good states while $s^{3}$ is a bad absorbing state. Suppose $H=2$ and $\rho = (0.5, 0.5, 0.0)$.  Moreover, the expert policy always takes action $a^{1}$. The agent is provided only 2 expert trajectories: $\tr_1 = (s^{1}, a^{1}) \rar (s^{1}, a^{1}) $ and $\tr_2 = (s^{1}, a^{1}) \rar (s^{2}, a^{1})$.  

Let us compute the empirical state-action distribution:
\begin{align*}
    \widehat{P}^{\piE}_{1}(s^{1}, a^{1}) = \RED{1.0}, \widehat{P}^{\piE}_{1}(s^{2}, a^{1}) = 0.0, \widehat{P}^{\piE}_{1}(s^{3}, a^{1}) = 0.0, \\
    \widehat{P}^{\piE}_{1}(s^{1}, a^{2}) = 0.0, \widehat{P}^{\piE}_{1}(s^{2}, a^{2}) = 0.0, \widehat{P}^{\piE}_{1}(s^{3}, a^{2}) = 0.0, \\
    \widehat{P}^{\piE}_{2}(s^{1}, a^{1}) = \RED{0.5}, \widehat{P}^{\piE}_{2}(s^{2}, a^{1}) = \RED{0.5}, \widehat{P}^{\piE}_{2}(s^{3}, a^{1}) = 0.0, \\
    \widehat{P}^{\piE}_{2}(s^{1}, a^{2}) = 0.0, \widehat{P}^{\piE}_{2}(s^{2}, a^{2}) = 0.0, \widehat{P}^{\piE}_{2}(s^{3}, a^{2}) = 0.0.
\end{align*}
Define the single-stage loss function in time step $h$ as 
\begin{align*}
    \text{Loss}_h (\pi) = \sum_{(s, a) \in \gS \times \gA} \labs P^{\pi}_h(s, a)  - \widehat{P}^{\piE}_h(s, a) \rabs .
\end{align*}
Then, we can define the \dquote{cost-to-go} function:
\begin{align*}
    \ell_h (\pi) = \sum_{t=h}^{H} \text{Loss}_t (\pi)  = \sum_{t=h}^{H} \sum_{(s, a) \in \gS \times \gA} \labs P^{\pi}_t(s, a)  - \widehat{P}^{\piE}_t(s, a) \rabs .
\end{align*}
As $\piail = (\piail_1, \piail_2)$ is the optimal solution of \eqref{eq:ail}, with \cref{lem:n_vars_opt_greedy_structure}, fixing $\piail_1$, $\piail_2$ is optimal w.r.t to VAIL's objective. Notice that $P^{\piail}_1$ and $\text{Loss}_1$ are independent of $\piail_2$, we have that
\begin{align*}
    \piail_2 \in \argmin_{\pi_2} \ell_2 (\pi_2)
\end{align*}
With a slight abuse of notation, we use $P^{\pi}_2$ denote the distribution induce by $(\piail_1, \pi_2)$ for any optimization variable $\pi_2$. For \cref{example:ail_success}, in the last time step $h = 2$, we have that 
\begin{align*}
    \ell_2 (\pi_2) &= \sum_{(s, a) \in \gS \times \gA} \labs P^{\pi}_2(s, a)  - \widehat{P}^{\piE}_2(s, a) \rabs  \\
    &= \labs P^{\pi}_2(s^{1}, a^{1}) - \widehat{P}^{\piE}_2(s^{1}, a^{1}) \rabs + \labs P^{\pi}_2(s^{2}, a^{1}) - \widehat{P}^{\piE}_2(s^{2}, a^{1}) \rabs + \labs P^{\pi}_2(s^{3}, a^{1}) - \widehat{P}^{\piE}_2(s^{3}, a^{1}) \rabs  \\
    &\quad + \labs P^{\pi}_2(s^{1}, a^{2}) - \widehat{P}^{\piE}_2(s^{1}, a^{2}) \rabs  + \labs P^{\pi}_2(s^{2}, a^{2}) - \widehat{P}^{\piE}_2(s^{2}, a^{2}) \rabs  + \labs P^{\pi}_2(s^{3}, a^{2}) - \widehat{P}^{\piE}_2(s^{3}, a^{2}) \rabs \\
    &= \labs P^{\pi}_2(s^{1}) \pi_2(a^{1}|s^{1}) - 0.5 \rabs +  \labs P^{\pi}_2(s^{2}) \pi_2(a^{1}|s^{2}) - 0.5 \rabs + \labs P^{\pi}_2(s^{3}) \pi_2(a^{1}|s^{3}) - 0.0 \rabs \\
    &\quad + \labs P^{\pi}_2(s^{1}) \pi_2(a^{2}|s^{1}) - 0.0 \rabs +  \labs P^{\pi}_2(s^{2}) \pi_2(a^{2}|s^{2}) - 0.0 \rabs + \labs P^{\pi}_2(s^{3}) \pi_2(a^{2}|s^{3}) - 0.0 \rabs \\
    &= \labs P^{\pi}_2(s^{1}) \pi_2(a^{1} | s^{1}) - 0.5 \rabs +  \labs P^{\pi}_2(s^{2}) \pi_2(a^{1}|s^{2}) - 0.5 \rabs + P^{\pi}_2(s^{3})  \\
    &\quad +  P^{\pi}_2(s^{1}) (1 - \pi_2(a^{1} | s^{1}))  + P^{\pi}_2(s^{2}) (1 - \pi_2(a^{1} | s^{2})).
\end{align*}
Note that $\pi_2$ is the optimization variable for $\ell_2 (\pi_2)$ while $P_2^{\pi}(s^{1}) = P_2^{\piail}(s^{1}), P_2^{\pi}(s^{2}) = P_2^{\piail}(s^{2}), P_2^{\pi}(s^{3}) = P_2^{\piail}(s^{3})$ are independent of $\pi_2$. We obtain
\begin{align*}
    \piail_2 &\in \argmin_{\pi_2} \ell_2 (\pi_2)
    \\
    &= \argmin_{\pi_2} \labs P_2^{\piail}(s^{1}) \pi_2(a^{1} | s^{1}) - 0.5 \rabs +  \labs P_2^{\piail}(s^{2}) \pi_2(a^{1}|s^{2}) - 0.5 \rabs + P^{\piail}_2(s^{3})  \\
    &\quad +  P^{\piail}_2(s^{1}) (1 - \pi_2(a^{1} | s^{1}))  + P^{\piail}_2(s^{2}) (1 - \pi_2(a^{1} | s^{2}))
    \\
    &= \argmin_{\pi_2} \labs P_2^{\piail}(s^{1}) \pi_2(a^{1} | s^{1}) - 0.5 \rabs - P^{\piail}_2(s^{1}) \pi_2(a^{1} | s^{1})  +  \labs P_2^{\piail}(s^{2}) \pi_2(a^{1}|s^{2}) - 0.5 \rabs \\
    &\quad - P^{\piail}_2(s^{2})  \pi_2(a^{1} | s^{2}). 
\end{align*}

Note that we only have two free optimization variables: $\pi_2(a^{1}|s^{1})$ and $\pi_2(a^{1}|s^{2})$ and they are independent. Then we obtain
\begin{align*}
    & \piail_2 (a^1|s^1) \in \argmin_{\pi_2 (a^1|s^1) \in [0, 1]} \labs P_2^{\piail}(s^{1}) \pi_2(a^{1} | s^{1}) - 0.5 \rabs - P^{\piail}_2(s^{1}) \pi_2(a^{1} | s^{1}),
    \\
    &\piail_2 (a^1|s^2) \in \argmin_{\pi_2 (a^1|s^2) \in [0, 1]} \labs P_2^{\piail}(s^{2}) \pi_2(a^{1}|s^{2}) - 0.5 \rabs - P^{\piail}_2(s^{2})  \pi_2(a^{1} | s^{2}).
\end{align*}
We first consider $\piail_2 (a^1|s^1)$ and we want to argue that $\pi_2(a^{1} | s^{1}) = 1$ is the optimal solution. We can directly prove this claim for this specific example but we have a more powerful lemma in \cref{appendix:technical_lemmas}. In particular, \cref{lem:mn_variables_opt_unique} claims that $\pi_2(a^{1} | s^{1}) = 1$ is the unique globally optimal solution. Similarly, we also have that $\piail_2 (a^1|s^2) = 1$. This finishes the proof in time step $h=2$.

 In the following part, we check the conditions of \cref{lem:mn_variables_opt_unique}. We apply \cref{lem:mn_variables_opt_unique} with $m = n = 1$, $c_1 = 0.5$, $a_{11} = P_2^{\piail}(s^{1})$ and $d_1 = P^{\piail}_2(s^{1})$.  \cref{lem:condition_for_ail_optimal_solution} implies that $\exists s \in \{s^1, s^2 \}$, $\piail_1 (a^1|s) > 0$ and hence we have $a_{11} = P_2^{\piail}(s^{1}) > 0$. Besides, $P_2^{\piail}(s^{1}) \leq 0.5 = c_1$, where the equality holds if and only if $\piail_2 (a^1|s^1) = 1, \piail_2 (a^1|s^2) = 1$. By \cref{lem:mn_variables_opt_unique}, we have that $\piail_2 (a^1|s^1) = 1$.

Then we consider the policy optimization in time step $h=1$. With \cref{lem:single_variable_opt_condition}, we have that fixing $\piail_2$, $\piail_1$ is optimal w.r.t VAIL's objective.
\begin{align*}
    \piail_1 \in \argmin_{\pi_1} \ell_1 (\pi_1) = \argmin_{\pi_1} \text{Loss}_1 (\pi_1) + \text{Loss}_2 (\pi_1). 
\end{align*}
We have proved that $\piail_2 (a^1|s^1) = 1, \piail_2 (a^1|s^2) = 1$ and plug it into $\text{Loss}_2 (\pi_1)$.
\begin{align*}
    \text{Loss}_2 (\pi_1) &= \labs P^{\pi}_2(s^{1}) - 0.5 \rabs + \labs P^{\pi}_2(s^{2})  - 0.5 \rabs + P^{\pi}_2(s^{3}) \\
    &= \labs P^{\pi}_1(s^{1}) \pi_1(a^{1}|s^{1}) P_1(s^{1}|s^{1}, a^{1})  + P^{\pi}_1(s^{2}) \pi_1(a^{1}|s^{2}) P_1(s^{1}|s^{2}, a^{1})  -0.5 \rabs  \\
    &\quad + \labs P^{\pi}_1(s^{1}) \pi_1(a^{1}|s^{1}) P_1(s^{2}|s^{1}, a^{1})  + P^{\pi}_1(s^{2}) \pi_1(a^{1}|s^{2}) P_1(s^{2}|s^{2}, a^{1})  -0.5 \rabs \\
    &\quad + P^{\pi}_1(s^{1}) \pi_1(a^{2}|s^{1})  P_1(s^{3}|s^{1}, a^{2}) + P^{\pi}_1(s^{2}) \pi_1(a^{2}|s^{2})  P_1(s^{3}|s^{2}, a^{2}) \\
    &= 2 \labs 0.25 \pi_1(a^{1} | s^{1}) + 0.25 \pi_1(a^{1} | s^{2}) - 0.5 \rabs + 0.5(1- \pi_1(a^{1} |s^{1})) + 0.5(1- \pi_1(a^{1} |s^{2})) \\
    &=  (1.0 - 0.5 \pi_1(a^{1} | s^{1}) - 0.5 \pi_1(a^{1} | s^{2}) ) - 0.5 \pi_1(a^{1} | s^{2}) - 0.5 \pi_1(a^{1} | s^{2}) + 1.0 \\
    &= 2.0 - \pi_1(a^{1} | s^{1}) - \pi_1(a^{1} | s^{2}),
\end{align*}
which has a unique globally optimal solution at $\pi_1(a^{1} | s^{1}) = 1.0$ and $\pi_1(a^{1} | s^{2}) = 1.0$. For $\text{Loss}_1 (\pi_1)$, 
\begin{align*}
    \text{Loss}_1 (\pi_1) &= \labs P^{\pi}_1 (s^{1}) - \rho (s^{1}) \pi_1 (a^1|s^1) \rabs + \rho (s^{1}) \lp 1 - \pi_1 (a^1|s^1) \rp + \rho (s^{2})
    \\
    &= \labs 1 - 0.5 \pi_1 (a^1|s^1) \rabs + 0.5 (1-\pi_1 (a^1|s^1)) + 0.5
    \\
    &= 2 - \pi_1 (a^1|s^1),
\end{align*}
which has a globally optimal solution at $\pi_1(a^{1} | s^{1}) = 1.0$ and $\pi_1(a^{1} | s^{2}) = 1.0$. By \cref{lem:unique_opt_solution_condition}, we have that $\pi_1(a^{1} | s^{1}) = \pi_1(a^{1} | s^{2}) = 1.0$ is the unique globally optimal solution of the joint objective $ \text{Loss}_1 (\pi_1) + \text{Loss}_2 (\pi_1)$. Recall that $\piail_1 \in \argmin_{\pi_1} \text{Loss}_1 (\pi_1) + \text{Loss}_2 (\pi_1)$. Hence it holds that $\piail_1(a^{1} | s^{1}) = \piail_1(a^{1} | s^{2}) = 1.0$. This finishes the proof in time step $h=1$. 
\end{proof}
In \cref{example:ail_success}, the estimator in the last time step happens to equal the true distribution, i.e., $\widehat{P}^{\piE}_{2}(s^{1}, a^{1}) = P^{\piE}_{2}(s^{1}, a^{1})$ and $\widehat{P}^{\piE}_{2}(s^{2}, a^{1}) = P^{\piE}_{2}(s^{2}, a^{1})$. Therefore, we can prove that $\piE_H$ is the unique globally optimal solution of \eqref{eq:ail}. We remark that in general, we cannot prove that in the last time step $h=H$, $\piE_H$ is the unique globally optimal solution of \eqref{eq:ail} due to the \dquote{weak convergence} issue discussed in \cref{sec:generalization_of_ail}.

\subsection{Proof of Proposition \ref{prop:ail_general_reset_cliff}}

Since the objective in \eqref{eq:ail} is a multi-stage optimization problem, we leverage backward induction to analyze its optimal solution step by step. In particular, we generalize the proof idea in \cref{claim:ail_reset_cliff} in \cref{example:ail_success}. The main intuition is that if the agent does not select the expert action, it goes to a bad absorbing state and suffers a huge loss for future state-action distribution matching. This implies the expert action is expected to be the optimal solution. With assumed transitions, we further prove that the optimal solution is unique in the first $H-1$ time steps.

\begin{proof}
The proof is based on backward induction. Suppose that $\piail = (\piail_1, \cdots, \piail_{H})$ is the optimal solution of \eqref{eq:ail}.  Define the single-stage loss function in time step $h$ as 
\begin{align*}
    \text{Loss}_h (\pi) = \sum_{(s, a) \in \gS \times \gA} \labs P^{\pi}_h(s, a)  - \widehat{P}^{\piE}_h(s, a) \rabs .
\end{align*}
\RED{First, we consider the base case (3 pages).} We aim to prove that $\piail_{H-1} (a^{1}|s) =  1, \forall s \in \goodS$. By \cref{lem:n_vars_opt_greedy_structure}, with fixed $(\piail_1, \cdots, \piail_{H-2}, \piail_{H})$, $\piail_{H-1}$ is optimal w.r.t the \textsf{VAIL} objective in \eqref{eq:ail}. This is direct from the global optimality condition. Furthermore, with fixed $(\piail_1, \cdots, \piail_{H-2}, \piail_{H})$, the state-action distribution losses from time step $1$ to $H-2$ are independent of $\pi_{H-1}$. Therefore, we have
\begin{align*}
\piail_{H-1} \in \argmin_{\pi_{H-1}} \text{Loss}_{H-1} (\pi_{H-1}) + \text{Loss}_{H} (\pi_{H-1}).
\end{align*}
In the following part, we will prove that $\piail_{H-1} (a^{1}|s) =  1, \forall s \in \goodS$ is the \emph{unique} optimal solution of the optimization problem $\min_{\pi_{H-1}} \text{Loss}_{H-1} (\pi_{H-1}) + \text{Loss}_{H} (\pi_{H-1})$. Our strategy is to prove that $\piail_{H-1} (a^{1}|s) =  1, \forall s \in \goodS$ is the optimal solution of $\min_{\pi_{H-1}} \text{Loss}_{H-1} (\pi_{H-1})$ and the \emph{unique} optimal solution of $\min_{\pi_{H-1}} \text{Loss}_{H} (\pi_{H-1})$. As a consequence, $\piail_{H-1} (a^{1}|s) =  1, \forall s \in \goodS$ is the unique optimal solution in time step $H-1$; see also \cref{lem:unique_opt_solution_condition}. We prove two terms separately. 
\begin{itemize}
    \item \BLUE{Term 1.}  We consider $\text{Loss}_{H-1} (\pi_{H-1})$. 
    \begin{align*}
        &\quad \text{Loss}_{H-1} (\pi_{H-1})
        \\
        &= \sum_{s \in \gS} \sum_{a \in \gA} \labs \widehat{P}^{\piE}_{H-1} (s, a) - P^{\piail}_{H-1} (s) \pi_{H-1} (a|s) \rabs
        \\
        &= \sum_{s \in \goodS}  \ls \labs \widehat{P}^{\piE}_{H-1} (s, a^{1}) - P^{\piail}_{H-1} (s) \pi_{H-1} (a|s^{1}) \rabs +  \sum_{a \ne a^{1}} \labs \widehat{P}^{\piE}_{H-1} (s, a) - P^{\piail}_{H-1} (s) \pi_{H-1} (a|s)  \rabs \rs \\
        &\quad +  \sum_{s \in \badS} \sum_{a \in \gA} \labs \widehat{P}^{\piE}_{H-1} (s, a) - P^{\piail}_{H-1} (s) \pi_{H-1} (a|s) \rabs \\
        &= \sum_{s \in \goodS} \lp \labs \widehat{P}^{\piE}_{H-1} (s) - P^{\piail}_{H-1} (s) \pi_{H-1} (a^{1}|s)  \rabs + P^{\piail}_{H-1} (s) \lp 1 - \pi_{H-1} (a^{1}|s) \rp \rp + \sum_{s \in \badS} P^{\piail}_{H-1} (s). 
    \end{align*}
    The last equation follows that the expert policy is deterministic and hence 1) $\forall s \in \goodS, \widehat{P}^{\piE}_{H-1} (s, a^{1}) = \widehat{P}^{\piE}_{H-1} (s)$; 2) $\forall a \in \gA \setminus \{a^{1} \}, \widehat{P}^{\piE}_{H-1} (s, a) = 0$; 3) $\forall s \in \badS, \widehat{P}^{\piE}_{H-1} (s) = 0$. Notice that $P^{\piail}_{H-1} (s)$ is fixed and independent of $\pi_{H-1}$, so we can obtain the following optimization problem: 
    \begin{align*}
        &\quad \argmin_{\pi_{H-1}} \mathrm{Loss}_{H-1} (\pi_{H-1})
        \\
        &= \argmin_{\pi_{H-1}} \sum_{s \in \goodS} \labs \widehat{P}^{\piE}_{H-1} (s) - P^{\piail}_{H-1} (s) \pi_{H-1} (a^{1}|s)  \rabs - P^{\piail}_{H-1} (s) \pi_{H-1} (a^{1}|s).
    \end{align*}
    Since the optimization variables $\pi_{H-1} (a^{1}|s)$ for different $s \in \goodS$ are independent, we can consider the above optimization problem for each $s \in \goodS$ individually.
    \begin{align*}
        \argmin_{\pi_{H-1} (a^{1}|s) \in [0, 1]} \labs \widehat{P}^{\piE}_{H-1} (s) - P^{\piail}_{H-1} (s) \pi_{H-1} (a^{1}|s)  \rabs - P^{\piail}_{H-1} (s) \pi_{H-1} (a^{1}|s).
    \end{align*}
    For this one-dimension optimization problem, we can use \cref{lem:single_variable_opt} to show that $\piail_{H-1} (a^{1}|s) = 1$ is the optimal solution. Consequently, we obtain that $\piail_{H-1} (a^{1}|s) = 1, \forall s \in \goodS$ is the optimal solution of $\mathrm{Loss}_{H-1} (\pi_{H-1})$.
    \item \BLUE{Term 2.} We consider the \textsf{VAIL}'s loss in step $H$. Recall the definition of $\gS (\widehat{P}^{\piE}_H) := \{ s \in \gS: \widehat{P}^{\piE}_H (s) > 0  \}$. Note that on non-visited state $s \notin \gS (\widehat{P}^{\piE}_H)$, we have that $\widehat{P}^{\piE}_{H} (s) = 0$. Then we obtain
    \begin{align*}
        &\quad \text{Loss}_{H} (\pi_{H-1})
        \\
        &= \sum_{s \in \gS} \sum_{a \in \gA} \labs \widehat{P}^{\piE}_{H} (s, a) - P^{\piail}_{H} (s, a) \rabs
        \\
        &= \sum_{s \in \goodS} \sum_{a \in \gA} \labs \widehat{P}^{\piE}_{H} (s, a) - P^{\piail}_{H} (s, a) \rabs + \sum_{s \in \badS} P^{\piail}_H (s)  
        \\
        &= \sum_{s \in \gS (\widehat{P}^{\piE}_H)} \lp \labs \widehat{P}^{\piE}_{H} (s) - P^{\piail}_{H} (s, a^{1}) \rabs + \sum_{a\in \gA \setminus \{a^1\}} P^{\piail}_H (s, a) \rp + \sum_{s \in \goodS \text{ and } s \notin \gS (\widehat{P}^{\piE}_H)} P^{\piail}_H (s)
        \\
        &\quad + \sum_{s \in \badS} P^{\piail}_H (s).
    \end{align*}
    Readers may notice that here we slightly abuse the notation: we use $P^{\piail}_{H} (s, a), P^{\piail}_{H} (s)$ to denote the distributions induced by $(\piail_1, \cdots, \piail_{H-2}, \pi_{H-1}, \piail_{H})$ for optimization variable $\pi_{H-1}$.  With the \dquote{transition flow equation}, we have that
    \begin{align*}
        \forall s \in \goodS, P^{\piail}_{H} (s) &= \sum_{s^\prime \in \gS} \sum_{a \in \gA} P^{\piail}_{H-1} (s^\prime) \pi_{H-1} (a|s^\prime) P_{H-1} (s | s^\prime, a)
        \\
        &=  \sum_{s^\prime \in \goodS} P^{\piail}_{H-1} (s^\prime) \pi_{H-1} (a^{1}|s^\prime) P_{H-1} (s | s^\prime, a^{1}).
    \end{align*}
    Recall that when the agent takes a non-expert action,  it transits into bad states. Therefore, the probability of visiting bad states in time step $H$ arises from two parts. One is the probability of visiting bad states in time step $H-1$ and the other is the probability of visiting good states and taking non-expert actions in time step $H-1$. Accordingly, we obtain 
    \begin{align*}
        \sum_{s \in \badS} P^{\piail}_H (s) &= \sum_{s \in \badS} P^{\piail}_{H-1} (s) + \sum_{s^\prime \in \goodS} P^{\piail}_{H-1} (s^\prime) \lp \sum_{a \in \gA \setminus \{a^{1}\}} \pi_{H-1} (a|s^\prime) \rp
        \\
        &= \sum_{s \in \badS} P^{\piail}_{H-1} (s) + \sum_{s^\prime \in \goodS} P^{\piail}_{H-1} (s^\prime) \lp 1 - \pi_{H-1} (a^{1}|s^\prime) \rp.
    \end{align*}
    Plugging the above two equations into $\text{Loss}_{H} (\pi_{H-1})$ yields
    \begin{align*}
        &\quad \text{Loss}_{H} (\pi_{H-1})
        \\
        &= \sum_{s \in \gS (\widehat{P}^{\piE}_H)} \labs \widehat{P}^{\piE}_{H} (s) - \lp \sum_{s^\prime \in \goodS} P^{\piail}_{H-1} (s^\prime) \pi_{H-1} (a^{1}|s^\prime) P_{H-1} (s | s^\prime, a^{1})  \rp \piail_{H} (a^{1}|s) \rabs
        \\
        &\quad + \sum_{s \in \gS (\widehat{P}^{\piE}_H)} \lp \sum_{s^\prime \in \goodS} P^{\piail}_{H-1} (s^\prime) \pi_{H-1} (a^{1}|s^\prime) P_{H-1} (s | s^\prime, a^{1})  \rp \lp 1- \piail_{H} (a^{1}|s) \rp 
        \\
        &\quad + \sum_{s \in \goodS \text{ and } s \notin \gS (\widehat{P}^{\piE}_H)} \lp \sum_{s^\prime \in \goodS} P^{\piail}_{H-1} (s^\prime) \pi_{H-1} (a^{1}|s^\prime) P_{H-1} (s | s^\prime, a^{1}) \rp
        \\
        &\quad +  \sum_{s \in \badS} P^{\piail}_{H-1} (s) + \sum_{s^\prime \in \goodS} P^{\piail}_{H-1} (s^\prime) \lp 1 - \pi_{H-1} (a^{1}|s^\prime) \rp
        \\
        &= \sum_{s \in \gS (\widehat{P}^{\piE}_H)} \labs \widehat{P}^{\piE}_{H} (s) - \sum_{s^\prime \in \goodS} P^{\piail}_{H-1} (s^\prime)  P_{H-1} (s | s^\prime, a^{1}) \piail_{H} (a^{1}|s) \pi_{H-1} (a^{1}|s^\prime) \rabs
        \\
        &\quad + \sum_{s^\prime \in \goodS} \lp \sum_{s \in \gS (\widehat{P}^{\piE}_H)} P^{\piail}_{H-1} (s^\prime) P_{H-1} (s | s^\prime, a^{1}) \lp 1- \piail_{H} (a^{1}|s) \rp    \rp \pi_{H-1} (a^{1}|s^\prime)
        \\
        &\quad + \sum_{s^\prime \in \goodS} \lp \sum_{s \in \goodS \text{ and } s \notin \gS (\widehat{P}^{\piE}_H)} P^{\piail}_{H-1} (s^\prime) P_{H-1} (s | s^\prime, a^{1}) \rp \pi_{H-1} (a^{1}|s^\prime) - \sum_{s^\prime \in \goodS} P^{\piail}_{H-1} (s^\prime) \pi_{H-1} (a^{1}|s^\prime)
        \\
        &\quad + \sum_{s \in \badS} P^{\piail}_{H-1} (s) + \sum_{s^\prime \in \goodS} P^{\piail}_{H-1} (s^\prime)
    \end{align*}
    Then, we merge the terms that are linear w.r.t $\pi_{H-1} (a^{1}|s^\prime)$, i.e., the second, third and forth terms in RHS.
    \begin{align*}
        & \quad \sum_{s^\prime \in \goodS} \lp \sum_{s \in \gS (\widehat{P}^{\piE}_H)} P^{\piail}_{H-1} (s^\prime) P_{H-1} (s | s^\prime, a^{1}) \lp 1- \piail_{H} (a^{1}|s) \rp    \rp \pi_{H-1} (a^{1}|s^\prime)
        \\
        &\quad + \sum_{s^\prime \in \goodS} \lp \sum_{s \in \goodS \text{ and } s \notin \gS (\widehat{P}^{\piE}_H)} P^{\piail}_{H-1} (s^\prime) P_{H-1} (s | s^\prime, a^{1}) \rp \pi_{H-1} (a^{1}|s^\prime) - \sum_{s^\prime \in \goodS} P^{\piail}_{H-1} (s^\prime) \pi_{H-1} (a^{1}|s^\prime)
        \\
        &= \sum_{s^\prime \in \goodS} \Bigg( \sum_{s \in \gS (\widehat{P}^{\piE}_H)} P^{\piail}_{H-1} (s^\prime) P_{H-1} (s | s^\prime, a^{1}) - \sum_{s \in \gS (\widehat{P}^{\piE}_H)} P^{\piail}_{H-1} (s^\prime) P_{H-1} (s | s^\prime, a^{1}) \piail_{H} (a^{1}|s)
        \\
        &\quad + \sum_{s \in \goodS \text{ and } s \notin \gS (\widehat{P}^{\piE}_H)} P^{\piail}_{H-1} (s^\prime) P_{H-1} (s | s^\prime, a^{1}) - P^{\piail}_{H-1} (s^\prime)   \Bigg) \pi_{H-1} (a^{1}|s^\prime)
        \\
        &= \sum_{s^\prime \in \goodS} \Bigg( \sum_{s \in \goodS} P^{\piail}_{H-1} (s^\prime) P_{H-1} (s | s^\prime, a^{1}) - \sum_{s \in \gS (\widehat{P}^{\piE}_H)} P^{\piail}_{H-1} (s^\prime) P_{H-1} (s | s^\prime, a^{1}) \piail_{H} (a^{1}|s)
        \\
        &\quad - P^{\piail}_{H-1} (s^\prime)   \Bigg) \pi_{H-1} (a^{1}|s^\prime)
        \\
        &= - \sum_{s^\prime \in \goodS} \lp \sum_{s \in \gS (\widehat{P}^{\piE}_H)} P^{\piail}_{H-1} (s^\prime) P_{H-1} (s | s^\prime, a^{1}) \piail_{H} (a^{1}|s)  \rp \pi_{H-1} (a^{1}|s^\prime),
    \end{align*}
    where in the last equation we use the fact that $\sum_{s \in \goodS} P_{H-1}(s|s^\prime, a^\prime) = 1$ so that the first term and the third term are canceled. Plugging the above equation into $\text{Loss}_{H} (\pi_{H-1})$ yields
    \begin{equation}    \label{eq:proof_vail_reset_cliff_1}
    \begin{split}
        &\quad \text{Loss}_{H} (\pi_{H-1})
        \\
        &= \sum_{s \in \gS (\widehat{P}^{\piE}_H)} \labs \widehat{P}^{\piE}_{H} (s) - \sum_{s^\prime \in \goodS} P^{\piail}_{H-1} (s^\prime)  P_{H-1} (s | s^\prime, a^{1}) \piail_{H} (a^{1}|s) \pi_{H-1} (a^{1}|s^\prime) \rabs
        \\
        & \quad - \sum_{s^\prime \in \goodS} \lp \sum_{s \in \gS (\widehat{P}^{\piE}_H)} P^{\piail}_{H-1} (s^\prime) P_{H-1} (s | s^\prime, a^{1}) \piail_{H} (a^{1}|s) \rp \pi_{H-1} (a^{1}|s^\prime)
        \\
        & \quad + \sum_{s \in \badS} P^{\piail}_{H-1} (s) + \sum_{s^\prime \in \goodS} P^{\piail}_{H-1} (s^\prime).     
    \end{split}
    \end{equation}
    Notice that $P^{\piail}_{H-1} (s)$ is independent of $\pi_{H-1}$ and then we have
    \begin{align*}
        &\quad \argmin_{\pi_{H-1}} \text{Loss}_{H} (\pi_{H-1})
        \\
        &= \argmin_{\pi_{H-1}} \sum_{s \in \gS (\widehat{P}^{\piE}_H)} \labs \widehat{P}^{\piE}_{H} (s) - \sum_{s^\prime \in \goodS} P^{\piail}_{H-1} (s^\prime)  P_{H-1} (s | s^\prime, a^{1}) \piail_{H} (a^{1}|s) \pi_{H-1} (a^{1}|s^\prime) \rabs
        \\
        &\qquad - \sum_{s^\prime \in \goodS} \lp \sum_{s \in \gS (\widehat{P}^{\piE}_H)} P^{\piail}_{H-1} (s^\prime) P_{H-1} (s | s^\prime, a^{1}) \piail_{H} (a^{1}|s) \rp \pi_{H-1} (a^{1}|s^\prime).
    \end{align*}
    For this type optimization problem, we apply \cref{lem:mn_variables_opt_unique} to show that $\forall s \in \goodS, \pi_{H-1}(a^{1} | s) = 1$ is the unique optimal solution. In particular, we verify the conditions of \cref{lem:mn_variables_opt_unique} by defining the following terms:
    \begin{align*}
        &m = \labs \gS (\widehat{P}^{\piE}_H)  \rabs, n = \labs \goodS \rabs, \forall s \in \gS (\widehat{P}^{\piE}_H), c(s) = \widehat{P}^{\piE}_{H} (s),
        \\
        & \forall s \in \gS (\widehat{P}^{\piE}_H), s^\prime \in \goodS, A (s, s^\prime) = P^{\piail}_{H-1} (s^\prime)  P_{H-1} (s | s^\prime, a^{1}) \piail_{H} (a^{1}|s),
        \\
        & \forall s^\prime \in \goodS, d(s^\prime) = \sum_{s \in \gS (\widehat{P}^{\piE}_H)} P^{\piail}_{H-1} (s^\prime) P_{H-1} (s | s^\prime, a^{1}) \piail_{H} (a^{1}|s). 
    \end{align*}
    To help us verify the conditions in \cref{lem:mn_variables_opt_unique}, we note that 
    \cref{lem:condition_for_ail_optimal_solution} implies that if $\piail$ is the optimal solution, then $\forall h \in [H]$, $\exists s \in \goodS$, $\piail_{h} (a^{1}|s) > 0$. Intuitively, in each time step, $\piail$ always takes the expert action on some good state with a positive probability. Combined with the reachable assumption that $\forall h \in [H], s, s^\prime \in \goodS, P_h (s^\prime| s, a^1) > 0$, we have that 
    \begin{align*}
        \forall s^\prime \in \goodS, s \in \gS (\widehat{P}^{\piE}_H), P^{\piail}_{H-1} (s^\prime)  > 0, P_{H-1} (s | s^\prime, a^{1}) > 0.
    \end{align*}
    With \cref{lem:general_condition_ail_policy_at_last_step}, we have that $\forall s \in \gS (\widehat{P}^{\piE}_H), \piail_{H} (a^{1}|s) > 0$. Hence we have that $A > 0$, where $>$ means element-wise comparison. Besides, we have that
    \begin{align*}
         & \sum_{s \in  \gS (\widehat{P}^{\piE}_H) } \sum_{s^\prime \in \goodS} A (s, s^\prime)  \leq \sum_{s \in  \gS (\widehat{P}^{\piE}_H) } \sum_{s^\prime \in \goodS} P^{\piail}_{H-1} (s^\prime)  P_{H-1} (s | s^\prime, a^{1}) \leq  1
         \\
         & \quad = \sum_{s \in  \gS (\widehat{P}^{\piE}_H) } \widehat{P}^{\piE}_{H} (s) = \sum_{s \in  \gS (\widehat{P}^{\piE}_H) } c(s) .
    \end{align*}
    For each $s^\prime \in \goodS$, it holds that 
    \begin{align*}
        \sum_{s \in \gS (\widehat{P}^{\piE}_H)} A (s, s^\prime) =  \sum_{s \in \gS (\widehat{P}^{\piE}_H)} P^{\piail}_{H-1} (s^\prime)  P_{H-1} (s | s^\prime, a^{1}) \piail_{H} (a^{1}|s) = d (s^\prime). 
    \end{align*}
    Thus, we have verified conditions in \cref{lem:mn_variables_opt_unique}. With \cref{lem:mn_variables_opt_unique}, we obtain that $\piail_{H-1} (a^{1}|s) = 1, \forall s \in \goodS$ is the \emph{unique} optimal solution of $\mathrm{Loss}_{H} (\pi_{H-1})$. 
\end{itemize}
Therefore, $\piail_{H-1} (a^{1}|s) = 1, \forall s \in \goodS$ is the \emph{unique} globally optimal solution of $\min_{\pi_{H-1}} \text{Loss}_{H-1} (\pi_{H-1}) + \text{Loss}_{H} (\pi_{H-1})$ and we finish the proof of the base case.

\RED{Second, we prove the induction step (3 pages).} The main proof strategy is similar to what we have used in the proof of the base case but is more tricky. We assume that for step $h^\prime = h+1, h+2, \cdots, H-1$, $\piail_{h^\prime} (a^{1}|s) = 1, \forall s \in \goodS$. We aim to prove that for step $h$, $\piail_{h} (a^{1}|s) = 1, \forall s \in \goodS$. By \cref{lem:n_vars_opt_greedy_structure}, we have that with fixed $(\piail_1, \cdots, \piail_{h-1}, \piail_{h+1}, \cdots, \piail_{H})$, $\piail_h$ is the optimal solution of the \textsf{VAIL}'s objective in \eqref{eq:ail}. This is direct from the global optimality condition. Moreover, note that $P^{\piail}_{t} (s, a)$ for $t \in [h-1]$ is fixed and independent of $\piail_{h}$ under this case. Therefore, we only need to consider the \textsf{VAIL}'s  state-action distribution matching losses from step $h$ to $H$. That is, we only need to prove that $\piail_{h} (a^{1}|s) = 1, \forall s \in \goodS$ is the \emph{unique} optimal solution of the losses from step $h$ to $H$.

Recall that the single-stage loss function in time step $h$ is
\begin{align*}
    \text{Loss}_h (\pi) = \sum_{(s, a) \in \gS \times \gA} \labs P^{\pi}_h(s, a)  - \widehat{P}^{\piE}_h(s, a) \rabs .
\end{align*}
By backward induction, we have three types of losses: 1) the single-stage loss in time step $h$; 2) the single-stage loss in time step $h < h^\prime \leq H-1$; 3) the single-stage loss in time step $H$. We need to prove that $\forall s \in \goodS, \pi_{h}(a^{1} | s) = 1$ is optimal for each cases. Furthermore, we will show that $\forall s \in \goodS, \pi_{h}(a^{1} | s) = 1$ is the unique optimal solution for case 2) and case 3), which proves the uniqueness of the optimal solution of the total losses. 

\begin{itemize}
    \item \BLUE{Term 1.}  For time step $h$, we have that
    \begin{align*}
        \text{Loss}_{h} (\pi_{h}) &= \sum_{s \in \gS} \sum_{a \in \gA} \labs \widehat{P}^{\piE}_{h} (s, a) - P^{\piail}_{h} (s, a) \rabs
        \\
        &= \sum_{s \in \goodS}  \lp \labs \widehat{P}^{\piE}_{h} (s, a^1) - P^{\piail}_{h} (s, a^1) \rabs + \sum_{a \in \gA \setminus \{ a^1\}} P^{\piail}_{h} (s, a)  \rp + \sum_{s \in \badS} P^{\piail}_{h} (s)  
        \\
        &= \sum_{s \in \goodS} \lp \labs \widehat{P}^{\piE}_{h} (s) - P^{\piail}_{h} (s) \pi_{h} (a^{1}|s)  \rabs + P^{\piail}_{h} (s) \lp 1 - \pi_{h} (a^{1}|s) \rp \rp + \sum_{s \in \badS} P^{\piail}_{h} (s). 
    \end{align*}
    Readers may notice that here we slightly abuse the notation and use $P^{\piail}_{h} (s, a)$ to denote the distribution induced by $(\piail_1, \piail_2, \cdots, \pi_h)$. Notice that $P^{\piail}_{h} (s)$ is independent of $\pi_{h}$, then we have that
    \begin{align*}
        &\quad \argmin_{\pi_{h}} \mathrm{Loss}_{h} (\pi_{h})
        \\
        &= \argmin_{\pi_{h}} \sum_{s \in \goodS} \labs \widehat{P}^{\piE}_{h} (s) - P^{\piail}_{h} (s) \pi_{h} (a^{1}|s)  \rabs - P^{\piail}_{h} (s) \pi_{h} (a^{1}|s).
    \end{align*}
    Since the optimization variables $\pi_{h} (a^{1}|s)$ for different $s \in \goodS$ are independent, we can consider the above optimization problem for each $s \in \goodS$ individually.
    \begin{align*}
        \argmin_{\pi_{h} (a^{1}|s) \in [0, 1]} \labs \widehat{P}^{\piE}_{h} (s) - P^{\piail}_{h} (s) \pi_{h} (a^{1}|s)  \rabs - P^{\piail}_{h} (s) \pi_{h} (a^{1}|s).
    \end{align*}
    For this one-dimension optimization problem, we can show that $\pi_h(a^{1}|s) = 1$ is the optimal solution by \cref{lem:single_variable_opt}. Thus, we obtain that $\piail_{h} (a^{1}|s) = 1, \forall s \in \goodS$ is the optimal solution of $\mathrm{Loss}_{h} (\pi_{h})$.
    \item \BLUE{Term 2.} Next, we consider \textsf{VAIL}'s objective values in time step $h^\prime$ where $h+1 \leq h^\prime \leq H-1$. Since $\piail_{h^\prime} (a^{1}|s) = 1, \forall s \in \goodS$, \textsf{VAIL}'s objective value regarding $\pi_h$ in time step $h^\prime$ is formulated as
    \begin{align*}
        \text{Loss}_{h^\prime} (\pi_{h}) &= \sum_{s \in \gS} \sum_{a \in \gA} \labs \widehat{P}^{\piE}_{h^\prime} (s, a) - P^{\piail}_{h^\prime} (s, a) \rabs
        \\
        &= \sum_{s \in \goodS} \sum_{a \in \gA} \labs \widehat{P}^{\piE}_{h^\prime} (s, a) - P^{\piail}_{h^\prime} (s) \piail_{h^\prime} (a|s)  \rabs + \sum_{s \in \badS} \sum_{a \in \gA} P^{\piail}_{h^\prime} (s, a)
        \\
        &= \sum_{s \in \goodS} \labs \widehat{P}^{\piE}_{h^\prime} (s, a^1) - P^{\piail}_{h^\prime} (s, a^1) \rabs + \sum_{s \in \badS} P^{\piail}_{h^\prime} (s)  
        \\
        &= \sum_{s \in \goodS} \labs \widehat{P}^{\piE}_{h^\prime} (s) - P^{\piail}_{h^\prime} (s) \rabs + \sum_{s \in \badS} P^{\piail}_{h^\prime} (s).
    \end{align*}
    With a little abuse of notation, we use $P^{\piail}_{h^\prime} (s)$ to denote the distribution induced by $(\piail_1, \piail_2, \cdots, \pi_h, \piail_{h+1}, \cdots, \piail_{h^\prime})$. Note that only through taking the expert action on good states, the agent could transit into good states. With the \dquote{transition flow equation}, we have 
    \begin{align*}
        \forall s \in \goodS, P^{\piail}_{h^\prime} (s) &= \sum_{s^\prime \in \gS} \sum_{a \in \gA} P^{\piail}_h (s^\prime) \pi_h (a|s^\prime) \sP^{\piail} \lp s_{h^\prime} = s |s_h = s^\prime, a_h = a^{1} \rp  
        \\
        &= \sum_{s^\prime \in \goodS} P^{\piail}_h (s^\prime) \pi_h (a^{1}|s^\prime) \sP^{\piail} \lp s_{h^\prime} = s |s_h = s^\prime, a_h = a^{1} \rp.
    \end{align*}
    Notice that the conditional probability $\sP^{\piail} \lp s_{h^\prime} = s |s_h = s^\prime, a_h = a^{1} \rp$ is independent of $\pi_h$. Besides, as for each $h^\prime = h+1, h+2, \cdots, H-1$, $\piail_{h^\prime} (a^{1}|s) = 1, \forall s \in \goodS$, the visitation probability of bad states in step $h^\prime$ comes from two parts in step $h$. One is the visitation probability of bad states in step $h$. The other is the probability of visiting good states and taking non-expert actions in step $h$. We obtain
    \begin{align*}
        \sum_{s \in \badS} P^{\piail}_{h^\prime} (s) &= \sum_{s \in \badS} P^{\piail}_{h} (s) + \sum_{s^\prime \in \goodS} \sum_{a \in \gA \setminus \{a^1 \}} P^{\piail}_h (s^\prime)  \pi_h (a|s^\prime)
        \\
        &= \sum_{s \in \badS} P^{\piail}_{h} (s) + \sum_{s^\prime \in \goodS} P^{\piail}_h (s^\prime) \lp 1 - \pi_h (a^{1}|s^\prime) \rp .
    \end{align*}
    Plugging the above two equations into $\text{Loss}_{h^\prime} (\pi_{h})$ yields
    \begin{align*}
        \text{Loss}_{h^\prime} (\pi_{h}) &= \sum_{s \in \goodS} \labs \widehat{P}^{\piE}_{h^\prime} (s) - \sum_{s^\prime \in \goodS} P^{\piail}_h (s^\prime) \pi_h (a^{1}|s^\prime) \sP^{\piail} \lp s_{h^\prime} = s |s_h = s^\prime, a_h = a^{1} \rp \rabs
        \\
        &\quad + \sum_{s \in \badS} P^{\piail}_{h} (s) + \sum_{s^\prime \in \goodS} P^{\piail}_h (s^\prime) \lp 1 - \pi_h (a^{1}|s^\prime) \rp. 
    \end{align*}
    This equation is similar to \eqref{eq:proof_vail_reset_cliff_1} in the proof of the base case. Note that $P^{\piail}_h (s)$ is independent of $\pi_h$ and then we have that
    \begin{align*}
        & \quad \argmin_{\pi_h} \text{Loss}_{h^\prime} (\pi_{h})
        \\
        &= \argmin_{\pi_h} \sum_{s \in \goodS} \labs \widehat{P}^{\piE}_{h^\prime} (s) - \sum_{s^\prime \in \goodS} P^{\piail}_h (s^\prime)  \sP^{\piail} \lp s_{h^\prime} = s |s_h = s^\prime, a_h = a^{1} \rp \pi_h (a^{1}|s^\prime) \rabs
        \\
        & \quad - \sum_{s^\prime \in \goodS} P^{\piail}_h (s^\prime) \pi_h (a^{1}|s^\prime).   
    \end{align*}
    For this type optimization problem, we can again use \cref{lem:mn_variables_opt_unique} to prove that $\forall s \in \goodS, \pi_h(a^{1} | s) = 1$ is the unique global optimal solution. To check the conditions in \cref{lem:mn_variables_opt_unique}, we define 
    \begin{align*}
        & m = n = \labs \goodS \rabs, \forall s \in \goodS, c(s) = \widehat{P}^{\piE}_{h^\prime} (s), \\
        & \forall s, s^\prime \in \goodS, A (s, s^\prime) = P^{\piail}_h (s^\prime)  \sP^{\piail} \lp s_{h^\prime} = s |s_h = s^\prime, a_h = a^{1} \rp,
        \\
        & \forall s^\prime \in \goodS, d(s^\prime) = P^{\piail}_h (s^\prime). 
    \end{align*}
    To help verify \cref{lem:mn_variables_opt_unique}, we note that  \cref{lem:condition_for_ail_optimal_solution} implies that if $\piail$ is the optimal solution, then $\forall h \in [H]$, $\exists s \in \goodS$, $\piail_{h} (a^{1}|s) > 0$. Combined with the reachable assumption that $\forall h \in [H], s, s^\prime \in \goodS, P_h (s^\prime |s, a^1) > 0$, we have that 
    \begin{align*}
        \forall s, s^\prime \in \goodS, P^{\piail}_{h} (s^\prime)  > 0, \sP^{\piail} \lp s_{h^\prime} = s |s_h = s^\prime, a_h = a^{1} \rp > 0.
    \end{align*}
    Then we can obtain that $A > 0$ where $>$ means element-wise comparison. Besides, we have that
    \begin{align*}
        & \sum_{s \in \goodS} c (s) = 1 \geq \sum_{s \in \goodS} \sum_{s^\prime \in \goodS} P^{\piail}_h (s^\prime)  \sP^{\piail} \lp s_{h^\prime} = s |s_h = s^\prime, a_h = a^{1} \rp = \sum_{s \in \goodS} \sum_{s^\prime \in \goodS} A (s, s^\prime).
    \end{align*}
    For each $s^\prime \in \goodS$, we further have that 
    \begin{align*}
        \sum_{s \in \goodS} A (s, s^\prime) = \sum_{s \in \goodS} P^{\piail}_h (s^\prime)  \sP^{\piail} \lp s_{h^\prime} = s |s_h = s^\prime, a_h = a^{1} \rp = P^{\piail}_h (s^\prime) = d(s^\prime).  
    \end{align*}
    Thus, we have verified conditions in \cref{lem:mn_variables_opt_unique}. By Lemma \ref{lem:mn_variables_opt_unique}, we obtain that $\piail_{h} (a^{1}|s) = 1, \forall s \in \goodS$ is the \emph{unique} optimal solution of $\mathrm{Loss}_{h^\prime} (\pi_{h})$ for each time step $h^\prime$, where $h+1 \leq h^\prime \leq H-1$.
    \item \BLUE{Term 3.} Finally, we consider the last time step $H$. Recall the definition that $\gS (\widehat{P}^{\piE}_H) = \{s \in \gS, \widehat{P}^{\piE}_H (s) > 0  \}$. \textsf{VAIL}'s loss in step $H$ is formulated as 
    \begin{align*}
        &\quad \text{Loss}_{H} (\pi_h)
        \\
        &= \sum_{s \in \gS} \sum_{a \in \gA} \labs \widehat{P}^{\piE}_{H} (s, a) - P^{\piail}_{H} (s, a) \rabs
        \\
        &= \sum_{s \in \goodS} \sum_{a \in \gA} \labs \widehat{P}^{\piE}_{H} (s, a) - P^{\piail}_{H} (s, a) \rabs + \sum_{s \in \badS} P^{\piail}_H (s)
        \\
        &=\sum_{s \in \gS (\widehat{P}^{\piE}_H)} \lp \labs \widehat{P}^{\piE}_{H} (s, a^1) - P^{\piail}_{H} (s, a^1) \rabs + \sum_{a \ne a^{1}} P^{\piail}_{H} (s, a) \rp + \sum_{s \in \goodS \text{ and } s \notin \gS (\widehat{P}^{\piE}_H)} \sum_{a \in \gA} P^{\piail}_{H} (s, a)
        \\
        &\quad  + \sum_{s \in \badS} P^{\piail}_H (s)
        \\
        &= \sum_{s \in \gS (\widehat{P}^{\piE}_H)} \lp \labs \widehat{P}^{\piE}_{H} (s) - P^{\piail}_{H} (s, a^{1}) \rabs + P^{\piail}_H (s) (1 - \piail_{H} (a^{1}|s)) \rp + \sum_{s \in \goodS \text{ and } s \notin \gS (\widehat{P}^{\piE}_H)} P^{\piail}_H (s)
        \\
        &\quad + \sum_{s \in \badS} P^{\piail}_H (s), 
    \end{align*}
    where we slightly abuse the notation and use $P^{\piail}_{H} (s, a), P^{\piail}_{H} (s)$ to denote the distributions induced by $(\piail_1, \piail_2, \cdots, \pi_h, \piail_{h+1}, \cdots, \piail_{H})$. Similarly, with the \dquote{transition flow equation}, we have
    \begin{align*}
         \forall s \in \goodS, P^{\piail}_{H} (s) &= \sum_{s^\prime \in \gS} \sum_{a \in \gA} P^{\piail}_{h} (s^\prime) \pi_{h} (a|s^\prime) \sP^{\piail} (s_H = s | s_h = s^\prime, a_h = a)
        \\
        &= \sum_{s^\prime \in \goodS} P^{\piail}_{h} (s^\prime) \pi_{h} (a^{1}|s^\prime) \sP^{\piail} (s_H = s | s_h = s^\prime, a_h = a^{1}).  
    \end{align*}
    Notice that for time step $h^\prime = h+1, h+2, \cdots, H-1$, $\piail_{h^\prime} (a^{1}|s) = 1, \forall s \in \goodS$. Then we have 
    \begin{align*}
        \sum_{s \in \badS} P^{\piail}_H (s) &= \sum_{s \in \badS} P^{\piail}_{h} (s) + \sum_{s^\prime \in \goodS} \sum_{a \in \gA \setminus \{a^1\}} P^{\piail}_{h} (s^\prime)  \pi_{h} (a|s^\prime)
        \\
        &= \sum_{s \in \badS} P^{\piail}_{h} (s) + \sum_{s^\prime \in \goodS} P^{\piail}_{h} (s^\prime) \lp 1 - \pi_{h} (a^{1}|s^\prime) \rp.
    \end{align*}
   
    Plugging the above equation into $\text{Loss}_{H} (\pi_h)$ yields that
    \begin{align*}
        \text{Loss}_{H} (\pi_h) &= \sum_{s \in \gS (\widehat{P}^{\piE}_H)} \labs \widehat{P}^{\piE}_{H} (s) - \sum_{s^\prime \in \goodS} P^{\piail}_{h} (s^\prime) \sP^{\piail} (s_H = s | s_h = s^\prime, a_h = a^{1}) \piail_H (a^{1}|s) \pi_h (a^{1}|s^\prime)    \rabs
        \\
        &\quad - \sum_{s^\prime \in \goodS} \lp \sum_{s \in \gS (\widehat{P}^{\piE}_H)} P^{\piail}_{h} (s^\prime) \sP^{\piail} (s_H = s | s_h = s^\prime, a_h = a^{1}) \piail_H (a^{1}|s) \rp \pi_h (a^{1}|s^\prime)
        \\
        &\quad + \sum_{s \in \badS} P^{\piail}_{h} (s) + \sum_{s^\prime \in \goodS} P^{\piail}_h (s^\prime). 
    \end{align*}
    This equation is similar to \eqref{eq:proof_vail_reset_cliff_1} in the proof of the base case.  Since $P^{\piail}_h (s)$ is independent of $\pi_h$, we have that
    \begin{align*}
        & \quad \argmin_{\pi_h} \text{Loss}_{H} (\pi_h)
        \\
        &= \argmin_{\pi_h} \sum_{s \in \gS (\widehat{P}^{\piE}_H)} \labs \widehat{P}^{\piE}_{H} (s) - \sum_{s^\prime \in \goodS} P^{\piail}_{h} (s^\prime) \sP^{\piail} (s_H = s | s_h = s^\prime, a_h = a^{1}) \piail_H (a^{1}|s) \pi_h (a^{1}|s^\prime)    \rabs
        \\
        &\quad - \sum_{s^\prime \in \goodS} \lp \sum_{s \in \gS (\widehat{P}^{\piE}_H)} P^{\piail}_{h} (s^\prime) \sP^{\piail} (s_H = s | s_h = s^\prime, a_h = a^{1}) \piail_H (a^{1}|s) \rp \pi_h (a^{1}|s^\prime).
    \end{align*}
    For this type optimization problem, we can again use \cref{lem:mn_variables_opt_unique} to prove that $\forall s \in \goodS, \piail_h(a^{1} | s) = 1$ is the unique globally optimal solution. To check conditions in \cref{lem:mn_variables_opt_unique}, we define 
    \begin{align*}
        & m = \labs \gS (\widehat{P}^{\piE}_H) \rabs, n = \labs \goodS \rabs, \forall s \in \gS (\widehat{P}^{\piE}_H), c(s) = \widehat{P}^{\piE}_{H} (s), 
        \\
        & \forall s \in \gS (\widehat{P}^{\piE}_H), s^\prime \in \goodS, A (s, s^\prime) = P^{\piail}_{h} (s^\prime) \sP^{\piail} (s_H = s | s_h = s^\prime, a_h = a^{1}) \piail_H (a^{1}|s),
        \\
        & \forall s^\prime \in \goodS, d(s^\prime) =  \sum_{s \in \gS (\widehat{P}^{\piE}_H)} P^{\piail}_{h} (s^\prime) \sP^{\piail} (s_H = s | s_h = s^\prime, a_h = a^{1}) \piail_H (a^{1}|s). 
    \end{align*}
    Similarly, we have that
    \begin{align*}
        & A > 0, \sum_{s \in \gS (\widehat{P}^{\piE}_H)} \sum_{s^\prime \in \goodS} A (s, s^\prime) \leq \sum_{s \in \gS (\widehat{P}^{\piE}_H)} \sum_{s^\prime \in \goodS} P^{\piail}_{h} (s^\prime) \sP^{\piail} (s_H = s | s_h = s^\prime, a_h = a^{1}) \leq 1
        \\
        & \qquad \qquad =  \sum_{s \in \gS (\widehat{P}^{\piE}_H)} c(s),
        \\
        &\forall s^\prime \in \goodS, \sum_{s \in \gS (\widehat{P}^{\piE}_H)} A (s, s^\prime) =  \sum_{s \in \gS (\widehat{P}^{\piE}_H)} P^{\piail}_{h} (s^\prime) \sP^{\piail} (s_H = s | s_h = s^\prime, a_h = a^{1}) \piail_H (a^{1}|s) = d(s^\prime).  
    \end{align*}
    Thus we have verified conditions in \cref{lem:mn_variables_opt_unique}. By \cref{lem:mn_variables_opt_unique}, we obtain $\piail_h(a^{1} | s) = 1, \forall s \in \goodS$ is the unique optimal solution of $\min_{\pi_h} \text{Loss}_{H} (\pi_h)$.
\end{itemize}
Thus, we finish the induction proof and the whole proof is done. 

\end{proof}

\subsection{Proof of Theorem \ref{theorem:ail_reset_cliff}}

We first formally present the sample complexity of \textsf{VAIL} to achieve a small policy value gap \emph{with high probability} on Reset Cliff. This result is similar to Theorem \ref{theorem:ail_reset_cliff}.

\begin{thm}[High Probability Version of \cref{theorem:ail_reset_cliff}]     
\label{theorem:ail_reset_cliff_high_prob}
For each tabular and episodic MDP satisfying \cref{asmp:reset_cliff}, with probability at least $1-\delta$, to obtain an $\varepsilon$-optimal policy (i.e., $V^{\piE} - V^{\piail} \leq \varepsilon$), \textsf{VAIL} requires at most ${\widetilde{\gO}}(|\gS|/\varepsilon^2)$ expert trajectories.
\end{thm}

We discuss the proof idea here. \cref{prop:ail_general_reset_cliff} indicates \textsf{VAIL} exactly recovers the expert policy in the first $H-1$ time steps. Thus, we infer that the policy value gap of $\piail$ only arises from the decision errors in the last time step. Similar to the proof of \cref{theorem:worst_case_sample_complexity_of_vail}, we can utilize $\ell_1$-norm concentrations inequality to upper bound the policy value gap in the last time step.

\begin{proof}[Proof of \cref{theorem:ail_reset_cliff} and \cref{theorem:ail_reset_cliff_high_prob}]
Similar to the proof of \cref{theorem:worst_case_sample_complexity_of_vail}, we can upper bound the policy value gap with the state-action distribution discrepancy. 
\begin{align*}
    \labs  V^{\piE} - V^{\piail} \rabs &\leq \sum_{h=1}^{H}  \sum_{(s, a) \in \gS \times \gA} \labs P^{\piE}_h(s, a) - P^{\piail}_h(s, a) \rabs.
\end{align*}
We apply \cref{prop:ail_general_reset_cliff} with the maximum likelihood estimation $\widehat{P}^{\piE}_h (s, a)$. From \cref{prop:ail_general_reset_cliff}, we have that for any $h \in [H-1]$, $\piail_{h} (a^{1}|s) = \piE_h (a^{1}|s) = 1, \forall s \in \goodS$. Therefore, $\piE$ and $\piail$ never visit bad states and for any $h \in [H-1]$, $P^{\piE}_h(s, a) = P^{\piail}_h(s, a)$. As a result, the policy value gap is upper bounded by the state-action distribution discrepancy in the last time step.
\begin{align*}
    \labs  V^{\piE} - V^{\piail} \rabs &\leq \sum_{(s, a) \in \gS \times \gA} \labs P^{\piE}_H (s, a) - P^{\piail}_H (s, a) \rabs
    \\
    &\leq \sum_{(s, a) \in \gS \times \gA} \labs P^{\piE}_H (s, a) - \widehat{P}^{\piE}_H (s, a) \rabs + \labs \widehat{P}^{\piE}_H (s, a) - P^{\piail}_H (s, a)  \rabs.
\end{align*}
Since $\piail = (\piail_1, \cdots, \piail_H)$ is the optimal solution of VAIL's objective in \eqref{eq:ail}, by \cref{lem:n_vars_opt_greedy_structure}, it holds that with fixed $(\piail_1, \cdots, \piail_{H-1})$, $\piail_{H}$ is also optimal w.r.t VAIL's objective. From \cref{prop:ail_general_reset_cliff}, we know that $(\piail_1 (a^{1}|s), \cdots, \piail_{H-1} (a^{1}|s)) = (\piE_1 (a^{1}|s), \cdots, \piE_{H-1} (a^{1}|s)), \forall s \in \goodS$ and thus $P^{\piail}_H (s) = P^{\piE}_H (s), \forall s \in \gS$. Then with fixed $(\piail_1, \cdots, \piail_{H-1})$, VAIL's objective is formulated as
\begin{align*}
    \piail_{H} &\in \argmin_{\pi_H} \sum_{(s, a) \in \gS \times \gA} \labs \widehat{P}^{\piE}_H (s, a) - P^{\piail}_H (s, a) \rabs
    \\
    &= \argmin_{\pi_H} \sum_{(s, a) \in \gS \times \gA} \labs \widehat{P}^{\piE}_H (s, a) - P^{\piE}_H (s) \pi_H (a|s)  \rabs, 
\end{align*}
where we slightly abuse the notation and use $P^{\piail}_H (s, a)$ to denote the distribution induced by $(\piail_1, \cdots, \piail_{H-1}, \pi_H)$ temporally. Since $\piail_{H} \in  \argmin_{\pi_H} \sum_{(s, a) \in \gS \times \gA} \labs \widehat{P}^{\piE}_H (s, a) - P^{\piE}_H (s) \pi_H (a|s)  \rabs$, we have
\begin{align*}
    \sum_{(s, a) \in \gS \times \gA} \labs \widehat{P}^{\piE}_H (s, a) - P^{\piail}_H (s, a)  \rabs &=\sum_{(s, a) \in \gS \times \gA} \labs \widehat{P}^{\piE}_H (s, a) - P^{\piE}_H (s) \piail_H (a|s)  \rabs
    \\
    &\leq \sum_{(s, a) \in \gS \times \gA} \labs \widehat{P}^{\piE}_H (s, a) - P^{\piE}_H (s) \piE_H (a|s)  \rabs.
\end{align*}
Then we obtain
\begin{align}
    \labs  V^{\piE} - V^{\piail} \rabs &\leq \sum_{(s, a) \in \gS \times \gA} \labs P^{\piE}_H (s, a) - \widehat{P}^{\piE}_H (s, a) \rabs + \labs \widehat{P}^{\piE}_H (s, a) - P^{\piail}_H (s, a)  \rabs \nonumber
    \\
    &\leq 2 \sum_{(s, a) \in \gS \times \gA} \labs P^{\piE}_H (s, a) - \widehat{P}^{\piE}_H (s, a) \rabs = 2\sum_{s \in \gS} \labs \widehat{P}^{\piE}_H (s) - P^{\piE}_H (s)  \rabs. \label{eq:vail_reset_cliff_value_gap_last_step_estimation_error} 
\end{align}
First, we prove the sample complexity required to achieve a small policy value gap \emph{with high probability}. With \cref{lemma:l1_concentration}, with probability at least $1-\delta$, we have
\begin{align}
\label{eq:value_gap_ail_policy}
    \labs  V^{\piE} - V^{\piail} \rabs \leq 2 \sum_{s \in \gS} \labs  \widehat{P}^{\piE}_H (s) - P^{\piE}_H (s)  \rabs \leq 2\sqrt{\frac{2 \vert \gS \vert \ln (1/\delta)}{m}},
\end{align}
which translates to a sample complexity $\widetilde{\gO} \lp \vert \gS \vert / \varepsilon^2 \rp$.

Finally, we prove the sample complexity required to achieve a small policy value gap \emph{in expectation}. We apply \citep[Theorem 1]{han2015minimax} and have that
\begin{align*}
    V^{\piE} - \expect \ls V^{\piail} \rs \leq 2 \expect \ls \lnorm \widehat{P}^{\piE}_H (\cdot) - P^{\piE}_H (\cdot) \rnorm_{1} \rs \leq 2 \sqrt{ \frac{|\gS| - 1}{m}},
\end{align*}
which translates to a sample complexity $\gO \lp \vert \gS \vert / \varepsilon^2 \rp$ as in \cref{theorem:ail_reset_cliff}.
\end{proof}
