# Supplementary material for: A Note on Target Q-learning For Solving Finite MDPs with A Generative Oracle
Source: arXiv:2203.11489 source file (2022-03-22)
Supplement: Supplementary file 9 [file review.tex]

\section{Review of Previous Work}
\label{appendix:review_of_previous_work}

In addition to the related work discussed in \cref{sec:related_work}, we provide a more detailed overview of other works in this section. %

\textbf{Function Approximation.} Beyond the tabular setting, researchers also have considered the statistical guarantees for imitation learning algorithms with function approximation. For instance, \citet{cai2019lqr} and \citet{liu2021provably} considered GAIL with linear function approximation setting while the neural network approximation case is studied in \citep{wang2020computation, zhang2020generative, xu2021error}. In addition, \citet{rajaraman2021value} studied BC and MIMIC-MD with linear function approximation. The main message is that under mild assumptions, the dependence on $|\gS|$ can be improved to the inherent dimension $d$ with function approximation. This direction is orthogonal to us since we mainly focus on the improvement/comparison in the planning horizon $H$, which is usually unrelated to function approximation.

\textbf{Active Imitation Learning.} In this paper, we mainly focus on the case where the expert demonstrations are fixed over the learning process. There is another setting where the agent can actively query the expert policy to obtain guidance in an online way. For this setting, DAgger \citep{ross11dagger} and AggraVaTe \citep{ross2014reinforcement} are two famous methods using the no-regret online learning. For general tabular and episodic MDPs, DAgger cannot improve the sample complexity compared with BC; see the theoretical result and explanation in \citep{rajaraman2020fundamental}. However, under the $\mu$-recoverability assumption, \citet{rajaraman2021value} proved that there is a clear boundary between the active setting and offline setting. That is, under the $\mu$-recoverability assumption, the agent can improve its sample complexity if it can actively query the expert policy.

\textbf{Inverse Reinforcement Learning.} Given the expert demonstrations, one of the interesting questions is to recover the reward function used by the expert policy. This field is often called inverse reinforcement learning (IRL) \citep{ng00irl, ziebart2008maximum}. Adversarial imitation learning algorithms are closely related to IRL (see e.g., \citep{pieter04apprentice, ho2016gail, fu2018airl}). However, without any assumption, the recovered reward function by adversarial imitation learning algorithms is not the true environment reward function.

\textbf{Reward-free Exploration.} The reward-free exploration framework is firstly proposed in \citep{chi20reward-free} with the goal of 1) isolating the exploration issue and planning issue under a standard RL framework and 2) learning a \dquote{robust} environment to cover all possible training scenarios. Following \citep{chi20reward-free}, there are many advances in this direction \citep{wang2020rewardfree, menard20fast-active-learning, Kaufmann21adaptive-rfe, zhang2021reward, chen2021near}, in which the minimax rate under the tabular setting is achieved by \citep{menard20fast-active-learning}. Our framework in Section \ref{sec:beyond_vanilla_ail} connects the reward-free exploration and adversarial imitation learning.
